# Supplementary material for: CausalSim: A Causal Framework for Unbiased Trace-Driven Simulation
Source: arXiv:2201.01811 source file (2023-05-05)
Supplement: Supplementary file 1 [file new_bola_basic_v1_bola_basic_v2.tex]

\addplot[solid, green!70!black, thick, mark = none] coordinates{
(0.0, 0.5271745033150107)
(0.08024875595518914, 0.5360297753759454)
(0.16049751191037828, 0.5475526605379091)
(0.24074626786556744, 0.5632273946616249)
(0.32099502382075656, 0.5827631477473563)
(0.4012437797759457, 0.6118762335830227)
(0.4814925357311349, 0.6562528800945017)
(0.561741291686324, 0.718229755900364)
(0.6419900476415131, 0.8038440906503069)
(0.7222388035967022, 0.9200256612345975)
(0.8024875595518914, 1.0515209355981034)
(0.8827363155070805, 1.1898156147830292)
(0.9629850714622697, 1.3229254970761055)
(1.0432338274174588, 1.4536686248885695)
(1.123482583372648, 1.5779232351207109)
(1.203731339327837, 1.700252350182185)
(1.2839800952830263, 1.820706113176394)
(1.3642288512382155, 1.9460036999593138)
(1.4444776071934045, 2.0756135936348747)
(1.5247263631485937, 2.207239240067228)
(1.6049751191037829, 2.3498161402827527)
(1.685223875058972, 2.4910993484304855)
(1.765472631014161, 2.6364441479538456)
(1.8457213869693503, 2.79154679539939)
(1.9259701429245395, 2.9562869473189535)
(2.0062188988797285, 3.1444539571483054)
(2.0864676548349177, 3.344434682139358)
(2.166716410790107, 3.52849998611036)
(2.246965166745296, 3.6920367035482564)
(2.3272139227004853, 3.840229631344895)
(2.407462678655674, 3.9898265660368124)
(2.4877114346108633, 4.144126923827912)
(2.5679601905660525, 4.301957356098569)
(2.6482089465212417, 4.462956832504284)
(2.728457702476431, 4.627265753734583)
(2.80870645843162, 4.797882677372955)
(2.888955214386809, 4.974185828937204)
(2.969203970341998, 5.150137978777634)
(3.0494527262971873, 5.3340227675763865)
(3.1297014822523765, 5.523844499818031)
(3.2099502382075658, 5.722300874465637)
(3.290198994162755, 5.924036608075787)
(3.370447750117944, 6.131879771680398)
(3.450696506073133, 6.3484678925184586)
(3.530945262028322, 6.5720860764535916)
(3.6111940179835114, 6.802644065899671)
(3.6914427739387006, 7.042939846026575)
(3.77169152989389, 7.289393199251343)
(3.851940285849079, 7.54546399970877)
(3.9321890418042678, 7.808103546711961)
(4.012437797759457, 8.073821880264086)
(4.092686553714646, 8.344644781742614)
(4.172935309669835, 8.60877859322721)
(4.253184065625025, 8.876231878157073)
(4.333432821580214, 9.1402453461935)
(4.413681577535403, 9.40424878560925)
(4.493930333490592, 9.672163387090418)
(4.574179089445781, 9.94286594512078)
(4.654427845400971, 10.217900867285145)
(4.734676601356159, 10.499785337374332)
(4.814925357311348, 10.787506464699606)
(4.895174113266537, 11.08044247477877)
(4.975422869221727, 11.373859858650604)
(5.055671625176916, 11.675972056652482)
(5.135920381132105, 11.981193127065332)
(5.216169137087294, 12.291278078508256)
(5.2964178930424834, 12.609426040978347)
(5.376666648997673, 12.927443631379596)
(5.456915404952862, 13.2511574783274)
(5.537164160908051, 13.580326894925426)
(5.61741291686324, 13.913959047726307)
(5.6976616728184295, 14.250930731213812)
(5.777910428773618, 14.58923622125183)
(5.858159184728807, 14.932475792664684)
(5.938407940683996, 15.27784143166182)
(6.0186566966391855, 15.624881850312608)
(6.098905452594375, 15.97575320206337)
(6.179154208549564, 16.326273552090314)
(6.259402964504753, 16.677335447634004)
(6.339651720459942, 17.030984727313278)
(6.4199004764151315, 17.38647927319778)
(6.500149232370321, 17.742926538046934)
(6.58039798832551, 18.10608295013138)
(6.660646744280699, 18.47180668911005)
(6.740895500235888, 18.836507508779306)
(6.821144256191077, 19.20909082430348)
(6.901393012146266, 19.584783012238628)
(6.981641768101455, 19.959743110864096)
(7.061890524056644, 20.341973959482967)
(7.1421392800118335, 20.7191704405202)
(7.222388035967023, 21.103186383620216)
(7.302636791922212, 21.487713786374936)
(7.382885547877401, 21.869152373960045)
(7.46313430383259, 22.256206989126266)
(7.54338305978778, 22.645538101186975)
(7.623631815742969, 23.031449453595616)
(7.703880571698158, 23.420810651518366)
(7.784129327653347, 23.813060092197123)
(7.8643780836085355, 24.206161965633722)
(7.944626839563725, 24.5981406335541)
(8.024875595518914, 24.98910641078574)
(8.105124351474103, 25.378006292157185)
(8.185373107429292, 25.77182019766211)
(8.265621863384482, 26.163006604548723)
(8.34587061933967, 26.556639994881394)
(8.42611937529486, 26.954264776244923)
(8.50636813125005, 27.348389568990942)
(8.586616887205238, 27.743326680012085)
(8.666865643160428, 28.140500173444995)
(8.747114399115617, 28.537683695498583)
(8.827363155070806, 28.939470354444552)
(8.907611911025995, 29.337556452359387)
(8.987860666981184, 29.738771479926562)
(9.068109422936374, 30.135323198877277)
(9.148358178891563, 30.53250672093086)
(9.228606934846752, 30.932578485740454)
(9.308855690801941, 31.32793679883018)
(9.38910444675713, 31.730977035361217)
(9.469353202712318, 32.13078805603311)
(9.549601958667507, 32.527269574639064)
(9.629850714622696, 32.923510406348676)
(9.710099470577886, 33.320172440126875)
(9.790348226533075, 33.71502932218257)
(9.870596982488264, 34.11011686251393)
(9.950845738443453, 34.50310842112304)
(10.031094494398642, 34.89772461628241)
(10.111343250353832, 35.29329353040643)
(10.19159200630902, 35.687699124531505)
(10.27184076226421, 36.081894117622284)
(10.3520895182194, 36.47194729037199)
(10.432338274174588, 36.859142306227746)
(10.512587030129778, 37.248844477253634)
(10.592835786084967, 37.63754378621147)
(10.673084542040156, 38.02693506999626)
(10.753333297995345, 38.413769055507515)
(10.833582053950535, 38.80178641825907)
(10.913830809905724, 39.184438468946524)
(10.994079565860913, 39.5720847727329)
(11.074328321816102, 39.958748271692585)
(11.154577077771291, 40.34448913754966)
(11.23482583372648, 40.72891625409757)
(11.31507458968167, 41.112861996852814)
(11.395323345636859, 41.495002587885566)
(11.475572101592048, 41.87750420926282)
(11.555820857547236, 42.26077803443247)
(11.636069613502425, 42.64179541994899)
(11.716318369457614, 43.02369532408541)
(11.796567125412803, 43.39968837064097)
(11.876815881367992, 43.77865991753866)
(11.957064637323182, 44.15661857374762)
(12.037313393278371, 44.53934082477984)
(12.11756214923356, 44.91466195374981)
(12.19781090518875, 45.2904343706504)
(12.278059661143939, 45.667360078929256)
(12.358308417099128, 46.04477718962146)
(12.438557173054317, 46.42590488996547)
(12.518805929009506, 46.807082733412884)
(12.599054684964695, 47.1906373599616)
(12.679303440919885, 47.57624785374981)
(12.759552196875074, 47.96429530236341)
(12.839800952830263, 48.356955916490065)
(12.920049708785452, 48.749626559237406)
(13.000298464740641, 49.14821408818628)
(13.08054722069583, 49.54972997437386)
(13.16079597665102, 49.952088264698624)
(13.241044732606209, 50.359019606053714)
(13.321293488561398, 50.768137186717176)
(13.401542244516587, 51.181416644963065)
(13.481791000471777, 51.60192673871963)
(13.562039756426966, 52.03032935695181)
(13.642288512382153, 52.47000414482893)
(13.722537268337343, 52.91601702097617)
(13.802786024292532, 53.37554847780079)
(13.883034780247721, 53.85300107978159)
(13.96328353620291, 54.345596898990024)
(14.0435322921581, 54.85284453301277)
(14.123781048113289, 55.38006917943118)
(14.204029804068478, 55.934882561341816)
(14.284278560023667, 56.52732332804591)
(14.364527315978856, 57.17772952228365)
(14.444776071934045, 57.915495031269735)
(14.525024827889235, 58.81886315355393)
(14.605273583844424, 60.13474855891228)
(14.685522339799613, 62.24080904493333)
(14.765771095754802, 66.29194056919042)
(14.846019851709991, 86.76113761062697)
(14.92626860766518, 93.30335845469385)
(15.00651736362037, 95.3532386076624)
(15.08676611957556, 96.72010952056073)
(15.167014875530748, 97.55207386359933)
(15.247263631485938, 98.11996456687741)
(15.327512387441127, 98.63450300813493)
(15.407761143396316, 99.09249005737473)
(15.488009899351505, 99.44460495808988)
(15.568258655306694, 99.69419726958768)
(15.648507411261884, 99.85166667151383)
(15.728756167217071, 99.94469215694672)
(15.80900492317226, 99.98548858587523)
(15.88925367912745, 99.99914756724215)
(15.969502435082639, 99.99995988551727)
};
\addplot[solid, blue, thick, mark = none] coordinates{
(0.0, 0.5052548657047036)
(0.075, 0.5052751582872167)
(0.15, 0.5052853045784733)
(0.225, 0.5053055971609866)
(0.3, 0.5053055971609866)
(0.375, 0.5053360360347563)
(0.45, 0.5053461823260129)
(0.525, 0.5053766211997827)
(0.6, 0.5053867674910393)
(0.675, 0.5054172063648091)
(0.75, 0.5054273526560656)
(0.8250000000000001, 0.5054476452385789)
(0.9, 0.5054577915298355)
(0.975, 0.5054780841123487)
(1.05, 0.5055085229861185)
(1.125, 0.505518669277375)
(1.2, 0.5055288155686316)
(1.2750000000000001, 0.5055592544424014)
(1.35, 0.5055694007336581)
(1.425, 0.5056099858986844)
(1.5, 0.5056607173549674)
(1.575, 0.5056911562287372)
(1.6500000000000001, 0.5057114488112504)
(1.725, 0.5057621802675333)
(1.8, 0.5058534968888427)
(1.875, 0.5059346672188955)
(1.95, 0.5059955449664351)
(2.025, 3.5811334990155057)
(2.1, 3.688714625209191)
(2.1750000000000003, 3.8012065563710693)
(2.25, 3.9172091043077297)
(2.325, 4.038883429056827)
(2.4, 4.165681630890505)
(2.475, 4.295594744139959)
(2.5500000000000003, 4.431017293541744)
(2.625, 4.572497178823716)
(2.7, 4.718999478277704)
(2.775, 4.872959301805289)
(2.85, 5.033362020280813)
(2.9250000000000003, 5.198827738093378)
(3.0, 5.371223372834198)
(3.075, 5.553176813938732)
(3.15, 5.739990328555175)
(3.225, 5.934657072604222)
(3.3000000000000003, 6.1386482583180815)
(3.375, 6.346474742126934)
(3.45, 6.562570453309913)
(3.525, 6.78787899695388)
(3.6, 7.022938126495437)
(3.6750000000000003, 7.2740283962224135)
(3.75, 7.540601906406957)
(3.825, 7.831810611762514)
(3.9, 8.128650508765482)
(3.975, 8.374190757175102)
(4.05, 8.57788770044252)
(4.125, 8.781828154700097)
(4.2, 8.994281347321957)
(4.275, 9.206704101070049)
(4.3500000000000005, 9.42669598809556)
(4.425, 9.650827561953761)
(4.5, 9.87998154998398)
(4.575, 10.111367722090648)
(4.65, 10.349389568679129)
(4.7250000000000005, 10.592261342488264)
(4.8, 10.839222071673808)
(4.875, 11.08835410718826)
(4.95, 11.343147773223897)
(5.025, 11.606007740808526)
(5.1000000000000005, 11.874235096467894)
(5.175, 12.14833715476483)
(5.25, 12.428283476825566)
(5.325, 12.713921868281252)
(5.4, 13.00516101251058)
(5.4750000000000005, 13.303076416386746)
(5.55, 13.603528393077063)
(5.625, 13.912553985879203)
(5.7, 14.224613319767066)
(5.775, 14.540020929769604)
(5.8500000000000005, 14.846946240281628)
(5.925, 15.136430076123563)
(6.0, 15.420323305483116)
(6.075, 15.70457165503665)
(6.15, 15.99281764334528)
(6.2250000000000005, 16.28056646338234)
(6.3, 16.57281009044607)
(6.375, 16.870816810943545)
(6.45, 17.17218195384696)
(6.525, 17.47523138109896)
(6.6000000000000005, 17.782339324853606)
(6.675, 18.08991399800605)
(6.75, 18.400309340127833)
(6.825, 18.713078914403656)
(6.9, 19.03543673391696)
(6.9750000000000005, 19.35931649711876)
(7.05, 19.688817305676707)
(7.125, 20.01718172961392)
(7.2, 20.351177345198543)
(7.275, 20.68381335775478)
(7.3500000000000005, 21.021583393686853)
(7.425, 21.365339741460325)
(7.5, 21.707807510244205)
(7.575, 22.050802886173425)
(7.65, 22.395959422140304)
(7.7250000000000005, 22.74134932280608)
(7.8, 23.079362869728318)
(7.875, 23.412567074594925)
(7.95, 23.747699074800284)
(8.025, 24.08139030164721)
(8.1, 24.415619281930734)
(8.175, 24.75466775056114)
(8.25, 25.091027452008554)
(8.325, 25.432916882190803)
(8.4, 25.777353031478462)
(8.475, 26.122022545465022)
(8.55, 26.472576908380415)
(8.625, 26.823445806324752)
(8.700000000000001, 27.176607766093085)
(8.775, 27.527923100852714)
(8.85, 27.884910212424785)
(8.925, 28.244362872772204)
(9.0, 28.60302412240161)
(9.075000000000001, 28.969102310939586)
(9.15, 29.335606643710342)
(9.225, 29.69867138374511)
(9.3, 30.0664541492142)
(9.375, 30.43410501289695)
(9.450000000000001, 30.803318405433217)
(9.525, 31.169548788340045)
(9.6, 31.536144437732112)
(9.675, 31.905144758151987)
(9.75, 32.26684989515837)
(9.825000000000001, 32.63005668327074)
(9.9, 32.99408532097488)
(9.975, 33.357687814446244)
(10.05, 33.721564257781544)
(10.125, 34.08732791129057)
(10.200000000000001, 34.458763341612034)
(10.275, 34.82687078840133)
(10.35, 35.19507969810319)
(10.425, 35.56605854531811)
(10.5, 35.93774763292098)
(10.575000000000001, 36.305114400448545)
(10.65, 36.67833557803117)
(10.725, 37.051303098332376)
(10.8, 37.4227486749451)
(10.875, 37.79489434565452)
(10.950000000000001, 38.168754739586305)
(11.025, 38.54612575029287)
(11.1, 38.921771891485825)
(11.175, 39.29823988227055)
(11.25, 39.67633127965634)
(11.325000000000001, 40.05542715987653)
(11.4, 40.430637010545446)
(11.475, 40.80649622385478)
(11.55, 41.177383754448385)
(11.625, 41.55398364701946)
(11.700000000000001, 41.9265453156704)
(11.775, 42.30015205232077)
(11.85, 42.67658960423174)
(11.925, 43.05578694736449)
(12.0, 43.43395951508033)
(12.075000000000001, 43.80954477852574)
(12.15, 44.187331787173825)
(12.225, 44.56347509663835)
(12.3, 44.93966913755916)
(12.375, 45.32000286531265)
(12.450000000000001, 45.69727241310665)
(12.525, 46.075800101016476)
(12.6, 46.45420603343122)
(12.675, 46.834529614893455)
(12.75, 47.21663894361686)
(12.825000000000001, 47.59977304775717)
(12.9, 47.98309993143136)
(12.975, 48.3665790094744)
(13.05, 48.75257436774908)
(13.125, 49.138245044703545)
(13.200000000000001, 49.52227202247444)
(13.275, 49.91166638832007)
(13.35, 50.30139558177717)
(13.425, 50.69511226769813)
(13.5, 51.09185254841354)
(13.575000000000001, 51.49371670621353)
(13.65, 51.89643315247907)
(13.725, 52.304588010858154)
(13.8, 52.71666948395354)
(13.875, 53.133195032619305)
(13.950000000000001, 53.55984657995917)
(14.025, 53.99006962182135)
(14.1, 54.42673555863146)
(14.175, 54.874329051124924)
(14.25, 55.33023235615755)
(14.325000000000001, 55.79733716673745)
(14.4, 56.26958614698445)
(14.475, 56.759063529785145)
(14.55, 57.269148030127994)
(14.625, 57.79730307519883)
(14.700000000000001, 58.34731323163638)
(14.775, 58.92801591912513)
(14.85, 59.54216078259562)
(14.925, 60.190458062435816)
};
\addplot[solid, red, thick, mark = none] coordinates{
(0.0008284753172681492,0.5144582122920603)
(0.08367600704408307,0.5223808226297029)
(0.16652353877089798,0.5333120191715136)
(0.2493710704977129,0.5469409146763949)
(0.3322186022245278,0.5642402853503614)
(0.41506613395134273,0.5867946532609414)
(0.49791366567815765,0.6165595994408443)
(0.5807611974049726,0.6592714949193503)
(0.6636087291317875,0.7229231503788662)
(0.7464562608586024,0.8047566951322379)
(0.8293037925854173,0.9038394674561732)
(0.9121513243122323,1.0267502425171195)
(0.9949988560390473,1.187338545474931)
(1.0778463877658622,1.399062785282919)
(1.1606939194926769,1.5505451006627815)
(1.243541451219492,1.692861256740612)
(1.3263889829463067,1.8362905897139847)
(1.4092365146731218,1.9792385488946906)
(1.4920840463999365,2.1302996622059696)
(1.5749315781267517,2.288059894131863)
(1.6577791098535664,2.458977676390651)
(1.7406266415803815,2.6420501469142788)
(1.8234741733071964,2.8272286277808236)
(1.9063217050340113,3.022205071052276)
(1.9891692367608265,3.240207227406295)
(2.072016768487641,3.4890273351116754)
(2.154864300214456,3.7223833097276318)
(2.237711831941271,3.897643484741103)
(2.320559363668086,4.067789063207488)
(2.403406895394901,4.238716874086957)
(2.4862544271217155,4.410657575655162)
(2.5691019588485307,4.586539525150828)
(2.651949490575346,4.764036082576064)
(2.7347970223021605,4.945152972066982)
(2.817644554028975,5.132447491897126)
(2.9004920857557903,5.321527106208408)
(2.9833396174826055,5.514457710861026)
(3.06618714920942,5.711319534820424)
(3.149034680936235,5.915060992566686)
(3.23188221266305,6.124659164790396)
(3.314729744389865,6.342631235282373)
(3.39757727611668,6.570601840592868)
(3.4804248078434945,6.8058632531381305)
(3.5632723395703096,7.055355278429108)
(3.646119871297125,7.311325792679729)
(3.7289674030239395,7.574536971061713)
(3.8118149347507546,7.847435797021118)
(3.8946624664775698,8.131105361591445)
(3.9775099982043844,8.418676059606511)
(4.060357529931199,8.691314141428222)
(4.143205061658014,8.953552543604191)
(4.2260525933848285,9.20985400233727)
(4.308900125111644,9.469294419343365)
(4.39174765683846,9.730429673244473)
(4.474595188565274,9.996970353692403)
(4.557442720292089,10.26612850413796)
(4.640290252018904,10.544372584920103)
(4.7231377837457185,10.826888858112167)
(4.805985315472533,11.111862143370967)
(4.888832847199348,11.403825377244118)
(4.971680378926163,11.696089469737684)
(5.054527910652979,11.995173024294033)
(5.137375442379794,12.300975754706355)
(5.220222974106608,12.614791353042449)
(5.303070505833423,12.937381994474029)
(5.385918037560238,13.263793540384905)
(5.4687655692870525,13.594908509394962)
(5.551613101013867,13.933424600467273)
(5.634460632740683,14.275932082570447)
(5.717308164467498,14.620074229844555)
(5.800155696194313,14.966984276426492)
(5.883003227921128,15.308659383013183)
(5.965850759647942,15.644377488915618)
(6.048698291374757,15.97900247516387)
(6.131545823101572,16.313316574171026)
(6.2143933548283865,16.648673649728963)
(6.297240886555202,16.982526432184812)
(6.380088418282018,17.325535345322017)
(6.462935950008832,17.671442529835897)
(6.545783481735647,18.02247433951755)
(6.628631013462462,18.373977494371186)
(6.7114785451892764,18.731026476461174)
(6.794326076916091,19.09040209854905)
(6.877173608642906,19.453688882702345)
(6.960021140369721,19.819763623404835)
(7.042868672096537,20.191193647550744)
(7.125716203823352,20.564709624798212)
(7.208563735550166,20.941755676525236)
(7.291411267276981,21.32077736652633)
(7.374258799003796,21.700771832733437)
(7.4571063307306105,22.081939647560173)
(7.539953862457426,22.465053014798936)
(7.622801394184242,22.847384149624613)
(7.705648925911056,23.232553384102893)
(7.788496457637871,23.614272773067054)
(7.871343989364686,23.996844594789067)
(7.9541915210915,24.379155672373386)
(8.037039052818315,24.759511168924995)
(8.119886584545132,25.143095881335743)
(8.202734116271944,25.530200639605372)
(8.285581647998761,25.914718013739414)
(8.368429179725576,26.29983710511429)
(8.45127671145239,26.690802882345928)
(8.534124243179205,27.085017932678067)
(8.61697177490602,27.478210063700796)
(8.699819306632834,27.87408986506591)
(8.78266683835965,28.274352173668433)
(8.865514370086466,28.67631934778665)
(8.948361901813279,29.07663179949257)
(9.031209433540095,29.483914142571482)
(9.11405696526691,29.890173566340984)
(9.196904496993724,30.29591150183509)
(9.279752028720539,30.70209069663914)
(9.362599560447354,31.1088816373047)
(9.44544709217417,31.513285766248295)
(9.528294623900983,31.919876134500253)
(9.6111421556278,32.32350805965144)
(9.693989687354614,32.72758124411258)
(9.776837219081429,33.13238651788339)
(9.859684750808244,33.534022747519145)
(9.942532282535058,33.9377750161185)
(10.025379814261873,34.33935107403017)
(10.108227345988688,34.73829963332354)
(10.191074877715504,35.14254330433624)
(10.273922409442317,35.5502167636217)
(10.356769941169134,35.95911371463018)
(10.439617472895948,36.364029303228484)
(10.522465004622763,36.77308671216786)
(10.605312536349578,37.184380503518994)
(10.688160068076392,37.592334764183505)
(10.771007599803209,38.003708784500084)
(10.853855131530022,38.417168757918226)
(10.936702663256838,38.83234362547274)
(11.019550194983653,39.24693683302778)
(11.102397726710468,39.66034666334251)
(11.185245258437282,40.07431809641536)
(11.268092790164097,40.48203167018354)
(11.350940321890914,40.89912200428804)
(11.433787853617726,41.31175963081037)
(11.516635385344543,41.723715311126426)
(11.599482917071358,42.131378741791195)
(11.682330448798172,42.541088011074805)
(11.765177980524987,42.94777866553356)
(11.848025512251802,43.35140056206407)
(11.930873043978616,43.75988633962466)
(12.013720575705431,44.168582718219525)
(12.096568107432248,44.5759352616432)
(12.17941563915906,44.98328780506688)
(12.262263170885877,45.39516325641749)
(12.345110702612692,45.8063667901825)
(12.427958234339506,46.22121071325456)
(12.510805766066321,46.6347208297761)
(12.593653297793136,47.05083838767459)
(12.676500829519952,47.465993197987736)
(12.759348361246765,47.88672392139928)
(12.842195892973582,48.30728415825926)
(12.925043424700396,48.730060720289636)
(13.007890956427211,49.15313814094043)
(13.090738488154026,49.57742902469357)
(13.17358601988084,50.01005369223226)
(13.256433551607655,50.44527577252722)
(13.33928108333447,50.880909026270075)
(13.422128615061286,51.31993195380296)
(13.504976146788099,51.76396919167613)
(13.587823678514916,52.21191759161471)
(13.67067121024173,52.664328727756136)
(13.753518741968545,53.123218352857215)
(13.83636627369536,53.594493324498785)
(13.919213805422174,54.06938862820604)
(14.00206133714899,54.55302888914674)
(14.084908868875804,55.04834246455961)
(14.16775640060262,55.55843822685562)
(14.250603932329435,56.081561167415686)
(14.33345146405625,56.623237056234785)
(14.416298995783064,57.19899019812643)
(14.499146527509879,57.85791069132197)
(14.581994059236695,58.71015290537665)
(14.664841590963508,59.91309598463054)
(14.747689122690325,61.94534582244267)
(14.83053665441714,65.90978994953699)
(14.913384186143954,93.27463648506472)
(14.996231717870769,99.31404234544968)
(15.079079249597584,99.69905112199706)
(15.161926781324398,99.82576274429594)
(15.244774313051213,99.90168943146847)
(15.32762184477803,99.95160187659562)
(15.410469376504842,99.97681382898655)
(15.493316908231659,99.98635104725375)
(15.576164439958474,99.9915358441456)
(15.659011971685288,99.99492551793564)
(15.741859503412103,99.99685101310631)
(15.824707035138918,99.99800430448457)
(15.907554566865734,99.99882665138038)
(15.990402098592547,99.99936819689712)
(16.07324963031936,99.99964899827619)
(16.15609716204618,99.99984957068979)
(16.238944693772993,99.99991977103456)
(16.321792225499806,99.99993982827591)
(16.404639757226622,99.99997994275864)
(16.48748728895344,99.99997994275864)
};
\addplot[dashed, magenta, thick, mark = none] coordinates{
(0.0, 0.9132228167000467)
(0.075, 0.9406433190096234)
(0.15, 0.9704456021767475)
(0.225, 1.001518835633403)
(0.3, 1.0346836329523585)
(0.375, 1.070040068959561)
(0.45, 1.1073879940031162)
(0.525, 1.1485487699152657)
(0.6, 1.191460855281494)
(0.675, 1.2365745868185642)
(0.75, 1.2849407501989236)
(0.8250000000000001, 1.3361090087058094)
(0.9, 1.3918807092062735)
(0.975, 1.448933367478864)
(1.05, 1.5597362147677818)
(1.125, 1.8411466253317603)
(1.2, 1.9301131455989644)
(1.2750000000000001, 2.025114177870794)
(1.35, 2.1243383677976024)
(1.425, 2.2247634556357787)
(1.5, 2.328551057625787)
(1.575, 2.4406148477216414)
(1.6500000000000001, 2.5584229328268746)
(1.725, 2.68126478167726)
(1.8, 2.8120225492600817)
(1.875, 2.948104297583303)
(1.95, 3.091011149036134)
(2.025, 4.063898576965998)
(2.1, 4.281621368297076)
(2.1750000000000003, 4.439709570846122)
(2.25, 4.583757275314753)
(2.325, 4.728115211743821)
(2.4, 4.873443873984578)
(2.475, 5.022695469402472)
(2.5500000000000003, 5.176040125201613)
(2.625, 5.334608686915207)
(2.7, 5.497020121945178)
(2.775, 5.665466068979776)
(2.85, 5.8389958171725)
(2.9250000000000003, 6.014527061884171)
(3.0, 6.197413806302973)
(3.075, 6.392709829139247)
(3.15, 6.585894273148033)
(3.225, 6.779138762052386)
(3.3000000000000003, 6.975815817486734)
(3.375, 7.176936195193146)
(3.45, 7.380508406135268)
(3.525, 7.588483909419072)
(3.6, 7.805265997386246)
(3.6750000000000003, 8.028773113657081)
(3.75, 8.259815864321753)
(3.825, 8.503648177742498)
(3.9, 8.757077666971595)
(3.975, 9.041570382174752)
(4.05, 9.430371088462843)
(4.125, 9.651416364015375)
(4.2, 9.874753353082099)
(4.275, 10.102503641973103)
(4.3500000000000005, 10.336188368042786)
(4.425, 10.57376600484182)
(4.5, 10.814916312927176)
(4.575, 11.060279771184915)
(4.65, 11.312488347537455)
(4.7250000000000005, 11.564336654516582)
(4.8, 11.821649046992436)
(4.875, 12.086897373165916)
(4.95, 12.352355856473887)
(5.025, 12.620576404978001)
(5.1000000000000005, 12.903628042687517)
(5.175, 13.181305662243659)
(5.25, 13.462355803434228)
(5.325, 13.7460579275124)
(5.4, 14.03535423436103)
(5.4750000000000005, 14.326702075141585)
(5.55, 14.623574046314431)
(5.625, 14.926780753969743)
(5.7, 15.233800312493651)
(5.775, 15.547845123799064)
(5.8500000000000005, 15.86954565928945)
(5.925, 16.19391819263263)
(6.0, 16.524595440010494)
(6.075, 16.871424764296265)
(6.15, 17.17076858367001)
(6.2250000000000005, 17.47143339074626)
(6.3, 17.771537778797207)
(6.375, 18.075214838134475)
(6.45, 18.380553139582464)
(6.525, 18.689324007560455)
(6.6000000000000005, 18.999175683658674)
(6.675, 19.309587778782195)
(6.75, 19.623962837013234)
(6.825, 19.94306142702899)
(6.9, 20.2599583708739)
(6.9750000000000005, 20.58032791117919)
(7.05, 20.910855046318133)
(7.125, 21.23875021353466)
(7.2, 21.56734590453282)
(7.275, 21.899504259334705)
(7.3500000000000005, 22.233594058277372)
(7.425, 22.573268032507908)
(7.5, 22.913732597863422)
(7.575, 23.255348023717335)
(7.65, 23.602877871784735)
(7.7250000000000005, 23.948396215850593)
(7.8, 24.29987901954291)
(7.875, 24.647839189361886)
(7.95, 24.99294722664136)
(8.025, 25.361192563679865)
(8.1, 25.69646324556871)
(8.175, 26.03181398731832)
(8.25, 26.36762507326728)
(8.325, 26.705167453705137)
(8.4, 27.046902969350185)
(8.475, 27.388708537373397)
(8.55, 27.734867360325318)
(8.625, 28.079044701723475)
(8.700000000000001, 28.42402264172922)
(8.775, 28.772463170712744)
(8.85, 29.12335553293197)
(8.925, 29.475739010057822)
(9.0, 29.830674395245328)
(9.075000000000001, 30.189622780953318)
(9.15, 30.545138600131317)
(9.225, 30.905578100745927)
(9.3, 31.26446644155835)
(9.375, 31.62747786519981)
(9.450000000000001, 31.988117515466314)
(9.525, 32.34969786909672)
(9.6, 32.71727270480138)
(9.675, 33.081324906632695)
(9.75, 33.447478679808896)
(9.825000000000001, 33.81425291690597)
(9.9, 34.17380175156965)
(9.975, 34.53548218002601)
(10.05, 34.90890138556599)
(10.125, 35.26690906791007)
(10.200000000000001, 35.62822922699303)
(10.275, 35.98926917656332)
(10.35, 36.3522405702744)
(10.425, 36.71332054977507)
(10.5, 37.07424040955422)
(10.575000000000001, 37.43762211005169)
(10.65, 37.79999305480708)
(10.725, 38.16323465054822)
(10.8, 38.531850264442724)
(10.875, 38.897753850554054)
(10.950000000000001, 39.26676976375236)
(11.025, 39.63466483890004)
(11.1, 40.005061784696416)
(11.175, 40.376049171965875)
(11.25, 40.74973857953592)
(11.325000000000001, 41.11704321321052)
(11.4, 41.49265405743875)
(11.475, 41.86533270926672)
(11.55, 42.235419423102655)
(11.625, 42.60588642127719)
(11.700000000000001, 42.97633340448653)
(11.775, 43.34552945237154)
(11.85, 43.71889862049855)
(11.925, 44.089966067628765)
(12.0, 44.46026293859919)
(12.075000000000001, 44.84107767377668)
(12.15, 45.21267551748443)
(12.225, 45.58376297957983)
(12.3, 45.95780264904069)
(12.375, 46.32883006624053)
(12.450000000000001, 46.70458101522508)
(12.525, 47.07748983915273)
(12.6, 47.45247021197749)
(12.675, 47.83039278468511)
(12.75, 48.208685634248724)
(12.825000000000001, 48.59138177615403)
(12.9, 48.97563908534411)
(12.975, 49.362458310078445)
(13.05, 49.75161928573995)
(13.125, 50.144963389126055)
(13.200000000000001, 50.53743684152641)
(13.275, 50.929149725249566)
(13.35, 51.32481556459765)
(13.425, 51.72268305011657)
(13.5, 52.12825629723344)
(13.575000000000001, 52.53857309110022)
(13.65, 52.95027091756507)
(13.725, 53.37287690005817)
(13.8, 53.794241954709534)
(13.875, 54.22271232200316)
(13.950000000000001, 54.6604796406273)
(14.025, 55.169440190430386)
(14.1, 55.79581853351752)
(14.175, 56.45075823193001)
(14.25, 57.12428182552094)
(14.325000000000001, 57.81962173116839)
(14.4, 58.54351298465863)
(14.475, 59.30812468482684)
(14.55, 60.105390800701684)
(14.625, 60.933720142550584)
(14.700000000000001, 61.80875440566912)
(14.775, 66.05816168749374)
(14.85, 76.73958819008972)
(14.925, 88.14040257900832)
};
\addplot[dashed, black, thick, mark = none] coordinates{
(0.0, 0.845713581991646)
(0.075, 0.868949896108504)
(0.15, 0.8929784712591263)
(0.225, 0.9178795364089575)
(0.3, 0.9438035208682057)
(0.375, 0.9720441167046635)
(0.45, 1.0024408659874415)
(0.525, 1.0338003628555534)
(0.6, 1.0672959559286246)
(0.675, 1.1026568724482801)
(0.75, 1.1398730837938391)
(0.8250000000000001, 1.1793858492752467)
(0.9, 1.2207839954445991)
(0.975, 1.2647093540254533)
(1.05, 1.3546460242887175)
(1.125, 1.5956137220012192)
(1.2, 1.6593155205641381)
(1.2750000000000001, 1.728162001536184)
(1.35, 1.79897409216162)
(1.425, 1.8721228514056265)
(1.5, 1.947207134440981)
(1.575, 2.0248888302326007)
(1.6500000000000001, 2.108377097398265)
(1.725, 2.19510460904375)
(1.8, 2.285191708617223)
(1.875, 2.379390542669725)
(1.95, 2.4779217408562295)
(2.025, 3.367259822808313)
(2.1, 3.542209110580686)
(2.1750000000000003, 3.6518821063432934)
(2.25, 3.745318765224073)
(2.325, 3.8371508447959632)
(2.4, 3.9292737543675895)
(2.475, 4.023592931868259)
(2.5500000000000003, 4.117370563852178)
(2.625, 4.217726971002545)
(2.7, 4.318043263670188)
(2.775, 4.422842349782043)
(2.85, 4.52875461278944)
(2.9250000000000003, 4.637334488897866)
(3.0, 4.7468069122468615)
(3.075, 4.864472718691875)
(3.15, 4.978909309277748)
(3.225, 5.0937470446908435)
(3.3000000000000003, 5.211001677687953)
(3.375, 5.329720489304425)
(3.45, 5.453283124709609)
(3.525, 5.578510511147765)
(3.6, 5.709975699649228)
(3.6750000000000003, 5.84656551331846)
(3.75, 5.989553586981888)
(3.825, 6.142981454773779)
(3.9, 6.307420748072926)
(3.975, 6.503269681343586)
(4.05, 6.802784466589198)
(4.125, 6.9291751730263)
(4.2, 7.057892519461291)
(4.275, 7.189548251755686)
(4.3500000000000005, 7.325375890253194)
(4.425, 7.461023013578452)
(4.5, 7.601824847933518)
(4.575, 7.746136699526779)
(4.65, 7.892614733187042)
(4.7250000000000005, 8.040837746845723)
(4.8, 8.193072208776627)
(4.875, 8.347683453808825)
(4.95, 8.506235946768482)
(5.025, 8.666633705933362)
(5.1000000000000005, 8.835054361642692)
(5.175, 9.001960695629256)
(5.25, 9.175255260989337)
(5.325, 9.353473879103575)
(5.4, 9.536105090317257)
(5.4750000000000005, 9.722747749803164)
(5.55, 9.914474919974115)
(5.625, 10.111928432553665)
(5.7, 10.314656999611191)
(5.775, 10.521908474595648)
(5.8500000000000005, 10.738496595433707)
(5.925, 10.960470085577228)
(6.0, 11.195019466054172)
(6.075, 11.445474238930483)
(6.15, 11.640280195650368)
(6.2250000000000005, 11.838967228573626)
(6.3, 12.042869144250776)
(6.375, 12.248897127512206)
(6.45, 12.460490995251348)
(6.525, 12.674963077125808)
(6.6000000000000005, 12.892684432100774)
(6.675, 13.115530412243501)
(6.75, 13.338817651696175)
(6.825, 13.56853323700509)
(6.9, 13.805118427480187)
(6.9750000000000005, 14.041111929335129)
(7.05, 14.28781599807691)
(7.125, 14.535773644403763)
(7.2, 14.788294313140272)
(7.275, 15.04641095221653)
(7.3500000000000005, 15.309251071633334)
(7.425, 15.57770721863125)
(7.5, 15.853103171140118)
(7.575, 16.13297188847251)
(7.65, 16.415468104423216)
(7.7250000000000005, 16.702527342783572)
(7.8, 16.996325814241263)
(7.875, 17.288349219838498)
(7.95, 17.590792362322833)
(8.025, 17.915719672372983)
(8.1, 18.202427909009522)
(8.175, 18.49286679253923)
(8.25, 18.79324403916337)
(8.325, 19.095165693372316)
(8.4, 19.401550083784112)
(8.475, 19.715636454878577)
(8.55, 20.032039437350253)
(8.625, 20.353376501196767)
(8.700000000000001, 20.682014400898723)
(8.775, 21.011474647496488)
(8.85, 21.3467414654683)
(8.925, 21.68756413929714)
(9.0, 22.040792216907835)
(9.075000000000001, 22.39601599003396)
(9.15, 22.75531138315639)
(9.225, 23.11690333041467)
(9.3, 23.484612736288092)
(9.375, 23.862561363876367)
(9.450000000000001, 24.246396791804127)
(9.525, 24.63283966110884)
(9.6, 25.026733795579204)
(9.675, 25.418371490396442)
(9.75, 25.823788510028773)
(9.825000000000001, 26.224823022423692)
(9.9, 26.63160393446858)
(9.975, 27.04867421133172)
(10.05, 27.48074730473298)
(10.125, 27.89874021469873)
(10.200000000000001, 28.32302106983119)
(10.275, 28.75147383116677)
(10.35, 29.185241761463036)
(10.425, 29.626039754856386)
(10.5, 30.072152917210428)
(10.575000000000001, 30.52800387024529)
(10.65, 30.990022424998703)
(10.725, 31.457667035953907)
(10.8, 31.932512196557756)
(10.875, 32.41598197094688)
(10.950000000000001, 32.901216782575794)
(11.025, 33.39918794246901)
(11.1, 33.89781096270647)
(11.175, 34.40674340500354)
(11.25, 34.915354931438834)
(11.325000000000001, 35.432410556487156)
(11.4, 35.95261516842918)
(11.475, 36.48201602553527)
(11.55, 37.012058714364926)
(11.625, 37.54928189560186)
(11.700000000000001, 38.08561252959822)
(11.775, 38.628020507727)
(11.85, 39.17391844585262)
(11.925, 39.724449606732655)
(12.0, 40.280837482090135)
(12.075000000000001, 40.83970242675572)
(12.15, 41.397263650732825)
(12.225, 41.95032202402436)
(12.3, 42.50980874317214)
(12.375, 43.07148170162828)
(12.450000000000001, 43.635902502150884)
(12.525, 44.19513850578165)
(12.6, 44.75310087458598)
(12.675, 45.31419217304264)
(12.75, 45.87372903529383)
(12.825000000000001, 46.43335615513113)
(12.9, 46.99041594807421)
(12.975, 47.544035924123854)
(13.05, 48.09562009017535)
(13.125, 48.64343349485096)
(13.200000000000001, 49.189792749527875)
(13.275, 49.72999443110694)
(13.35, 50.26681646751665)
(13.425, 50.80309695840961)
(13.5, 51.3338917937903)
(13.575000000000001, 51.85802762503909)
(13.65, 52.382273771115386)
(13.725, 52.90291964236735)
(13.8, 53.42044661258767)
(13.875, 53.93829449866976)
(13.950000000000001, 54.459160999576696)
(14.025, 55.03492417008901)
(14.1, 55.69955094845178)
(14.175, 56.3893295074814)
(14.25, 57.09186447201668)
(14.325000000000001, 57.82198817204419)
(14.4, 58.56745566171296)
(14.475, 59.34157492066608)
(14.55, 60.14148779200962)
(14.625, 60.96938051505191)
(14.700000000000001, 61.848138402186)
(14.775, 66.10095551694982)
(14.85, 76.75490081142573)
(14.925, 88.09786248975952)
};
