# Supplementary material for: CausalSim: A Causal Framework for Unbiased Trace-Driven Simulation
Source: arXiv:2201.01811 source file (2023-05-05)
Supplement: Supplementary file 2 [file new_bola_basic_v1_linear_bba.tex]

\addplot[solid, green!70!black, thick, mark = none] coordinates{
(0.0, 0.42212378418830887)
(0.07980021702477436, 0.431409657207913)
(0.1596004340495487, 0.4440964603819144)
(0.23940065107432307, 0.46033423474653656)
(0.3192008680990974, 0.4837489720105116)
(0.3990010851238718, 0.5294698099930331)
(0.47880130214864614, 0.6182274185323019)
(0.5586015191734205, 0.7613082177975676)
(0.6384017361981948, 1.0121018098449925)
(0.7182019532229692, 1.421888886610488)
(0.7980021702477436, 1.8809394369360017)
(0.8778023872725179, 2.304371912384704)
(0.9576026042972923, 2.655601306957453)
(1.0374028213220665, 2.933819066181267)
(1.117203038346841, 3.1772939899062393)
(1.1970032553716152, 3.3990463058313116)
(1.2768034723963897, 3.611504413123656)
(1.356603689421164, 3.824646040692129)
(1.4364039064459384, 4.037129154823845)
(1.5162041234707127, 4.249545584050572)
(1.5960043404954871, 4.4646960943818135)
(1.6758045575202614, 4.678512906613292)
(1.7556047745450358, 4.889553959674638)
(1.83540499156981, 5.1044960796777925)
(1.9152052085945845, 5.328907456189268)
(1.9950054256193588, 5.569431572868512)
(2.074805642644133, 5.816915926505899)
(2.1546058596689077, 6.042919405123968)
(2.234406076693682, 6.250684562227769)
(2.314206293718456, 6.445687895639457)
(2.3940065107432305, 6.639024106426442)
(2.473806727768005, 6.828675976212828)
(2.5536069447927794, 7.019944954945177)
(2.6334071618175536, 7.212839378236614)
(2.713207378842328, 7.406350636899192)
(2.7930075958671026, 7.601320627858386)
(2.872807812891877, 7.800191685759389)
(2.952608029916651, 8.000013003556472)
(3.0324082469414253, 8.204427244184616)
(3.1122084639662, 8.410008470650055)
(3.1920086809909742, 8.617715278461993)
(3.2718088980157485, 8.829314817602613)
(3.3516091150405227, 9.043631766621504)
(3.4314093320652974, 9.263391871010054)
(3.5112095490900717, 9.487086384792907)
(3.591009766114846, 9.716882567382179)
(3.67080998313962, 9.949096077777272)
(3.750610200164395, 10.186452661469579)
(3.830410417189169, 10.425584730757196)
(3.9102106342139433, 10.671068537244937)
(3.9900108512387176, 10.918727938757918)
(4.069811068263492, 11.16414506034067)
(4.149611285288266, 11.40986226399587)
(4.229411502313041, 11.652578646926601)
(4.309211719337815, 11.895720146126633)
(4.389011936362589, 12.139228412304098)
(4.468812153387364, 12.385679149914168)
(4.548612370412139, 12.631429696021861)
(4.628412587436912, 12.878547282681813)
(4.708212804461687, 13.129190833693016)
(4.788013021486461, 13.387161388639793)
(4.867813238511236, 13.646657360788176)
(4.94761345553601, 13.907253633868862)
(5.027413672560784, 14.171109131680847)
(5.107213889585559, 14.43533973208339)
(5.1870141066103335, 14.705288563088672)
(5.266814323635107, 14.979905337443125)
(5.346614540659882, 15.2543887419876)
(5.426414757684656, 15.534640390813554)
(5.50621497470943, 15.816192395286777)
(5.586015191734205, 16.10107864500941)
(5.665815408758979, 16.388032126786676)
(5.745615625783754, 16.677002826939834)
(5.825415842808528, 16.97287541475927)
(5.905216059833302, 17.269089762716767)
(5.985016276858077, 17.56760473989636)
(6.064816493882851, 17.871546201219367)
(6.144616710907625, 18.179230352834832)
(6.2244169279324, 18.4890400857968)
(6.304217144957174, 18.800175181245404)
(6.3840173619819485, 19.118037116484693)
(6.463817579006723, 19.437232749823742)
(6.543617796031497, 19.760304443265234)
(6.623418013056272, 20.084701499193365)
(6.7032182300810454, 20.413099649420783)
(6.78301844710582, 20.745248825553787)
(6.862818664130595, 21.078956761340894)
(6.942618881155369, 21.41539044261939)
(7.022419098180143, 21.753924698405015)
(7.102219315204918, 22.09726860296291)
(7.182019532229692, 22.443688348763388)
(7.2618197492544665, 22.791933593837914)
(7.34161996627924, 23.13856172996648)
(7.421420183304015, 23.488265707337625)
(7.50122040032879, 23.84012860850776)
(7.5810206173535635, 24.198184870228676)
(7.660820834378338, 24.557374775334388)
(7.740621051403113, 24.92094087732995)
(7.820421268427887, 25.28163952841102)
(7.900221485452661, 25.644938890786626)
(7.980021702477435, 26.014148202866817)
(8.05982191950221, 26.387075198400094)
(8.139622136526985, 26.758851879322325)
(8.219422353551758, 27.138605742003776)
(8.299222570576532, 27.518526316947682)
(8.379022787601308, 27.901531068747303)
(8.458823004626081, 28.288761976400544)
(8.538623221650855, 28.679918957834964)
(8.61842343867563, 29.06908372773287)
(8.698223655700405, 29.463324886022995)
(8.778023872725178, 29.86125872092684)
(8.857824089749954, 30.263710458143635)
(8.937624306774728, 30.66478681919505)
(9.017424523799502, 31.073181848568915)
(9.097224740824277, 31.480284857908636)
(9.177024957849051, 31.888838263931852)
(9.256825174873825, 32.30154280529058)
(9.3366253918986, 32.71262190209022)
(9.416425608923374, 33.129419229492605)
(9.496225825948148, 33.54697509768922)
(9.576026042972922, 33.967056656662265)
(9.655826259997697, 34.38930547504743)
(9.735626477022471, 34.81530531933817)
(9.815426694047245, 35.24278056715178)
(9.89522691107202, 35.671456143255185)
(9.975027128096794, 36.10033177407354)
(10.054827345121568, 36.536234326755036)
(10.134627562146344, 36.96877762734775)
(10.214427779171118, 37.40642232317206)
(10.294227996195891, 37.84816814065314)
(10.374028213220667, 38.28847189706385)
(10.45382843024544, 38.724149388191)
(10.533628647270215, 39.16377795993871)
(10.613428864294988, 39.60763268754004)
(10.693229081319764, 40.04988697742166)
(10.773029298344538, 40.48994066543866)
(10.852829515369312, 40.938663391104136)
(10.932629732394087, 41.38195129701307)
(11.01242994941886, 41.829231961608166)
(11.092230166443635, 42.277996365339256)
(11.17203038346841, 42.724868584891304)
(11.251830600493184, 43.173199536739965)
(11.331630817517958, 43.62668189749896)
(11.411431034542733, 44.075996451696206)
(11.491231251567507, 44.52902868934653)
(11.571031468592281, 44.98394477556278)
(11.650831685617057, 45.437010355665606)
(11.73063190264183, 45.889058990967364)
(11.810432119666604, 46.340065674628676)
(11.890232336691378, 46.79429824056879)
(11.970032553716154, 47.24961443621497)
(12.049832770740927, 47.702296578114115)
(12.129632987765701, 48.15449525445209)
(12.209433204790477, 48.61166195621169)
(12.28923342181525, 49.066669734172294)
(12.369033638840024, 49.5181348765554)
(12.4488338558648, 49.97386785285776)
(12.528634072889574, 50.430867842354886)
(12.608434289914348, 50.89026015281847)
(12.688234506939123, 51.35179471585478)
(12.768034723963897, 51.81536316849324)
(12.84783494098867, 52.273571821893285)
(12.927635158013446, 52.73310583777997)
(13.00743537503822, 53.18828866361617)
(13.087235592062994, 53.64177102437516)
(13.167035809087768, 54.0944865087268)
(13.246836026112543, 54.547418719019646)
(13.326636243137317, 54.997975279572294)
(13.406436460162091, 55.4473815255139)
(13.486236677186866, 55.899205099261316)
(13.56603689421164, 56.35797223874063)
(13.645837111236414, 56.82226588972084)
(13.72563732826119, 57.29984650801995)
(13.805437545285963, 57.7824785078719)
(13.885237762310737, 58.276521962089966)
(13.965037979335513, 58.78093491903369)
(14.044838196360287, 59.293591797356584)
(14.12463841338506, 59.82422025757378)
(14.204438630409836, 60.376754709079606)
(14.28423884743461, 60.96188140789839)
(14.364039064459384, 61.58613547471901)
(14.443839281484157, 62.28681044265607)
(14.523639498508933, 63.12596495141422)
(14.603439715533707, 64.29811053323084)
(14.68323993255848, 66.18813578847148)
(14.763040149583256, 69.66927121234325)
(14.84284036660803, 86.90009217520992)
(14.922640583632804, 93.36509368645658)
(15.00244080065758, 95.3139350278968)
(15.082241017682353, 96.65323465967943)
(15.162041234707127, 97.48947170384433)
(15.241841451731903, 98.07439834794816)
(15.321641668756676, 98.5969245922093)
(15.40144188578145, 99.06285202336173)
(15.481242102806226, 99.42366737302652)
(15.561042319831, 99.68387187229041)
(15.640842536855773, 99.8472665607377)
(15.720642753880547, 99.94095051663297)
(15.800442970905323, 99.98367053389103)
(15.880243187930096, 99.9988996990677)
};
\addplot[solid, blue, thick, mark = none] coordinates{
(0.0, 0.4188027725090919)
(0.075, 0.4188027725090919)
(0.15, 0.4188115447174726)
(0.225, 0.4188203169258532)
(0.3, 0.41882908913423395)
(0.375, 0.41882908913423395)
(0.45, 0.41882908913423395)
(0.525, 0.4188378613426145)
(0.6, 0.4188466335509952)
(0.675, 0.41885540575937585)
(0.75, 0.41886417796775655)
(0.8250000000000001, 0.4188817223845179)
(0.9, 0.4188817223845179)
(0.975, 0.4188817223845179)
(1.05, 0.41889049459289845)
(1.125, 0.4189343556348017)
(1.2, 0.4189343556348017)
(1.2750000000000001, 0.4189606722599437)
(1.35, 0.41897821667670504)
(1.425, 0.4189957610934663)
(1.5, 0.4190220777186083)
(1.575, 0.4190659387605115)
(1.6500000000000001, 0.41912734421917613)
(1.725, 0.41914488863593735)
(1.8, 0.4192326107197439)
(1.875, 0.4193115605951698)
(1.95, 0.41932033280355047)
(2.025, 4.881198859121667)
(2.1, 5.027431572827138)
(2.1750000000000003, 5.179778515773922)
(2.25, 5.335265909320981)
(2.325, 5.496227160897566)
(2.4, 5.663732479926117)
(2.475, 5.839676663416856)
(2.5500000000000003, 6.018199876171507)
(2.625, 6.205951452142603)
(2.7, 6.401466432530577)
(2.775, 6.60180612752791)
(2.85, 6.808944284020246)
(2.9250000000000003, 7.023819528304321)
(3.0, 7.24701082613325)
(3.075, 7.477026902082329)
(3.15, 7.713078257397296)
(3.225, 7.95541928612119)
(3.3000000000000003, 8.207278160938094)
(3.375, 8.467040795505962)
(3.45, 8.733400130776083)
(3.525, 9.01371604957982)
(3.6, 9.29582149889321)
(3.6750000000000003, 9.591085260777579)
(3.75, 9.899375752107217)
(3.825, 10.2222895148074)
(3.9, 10.548291094857573)
(3.975, 10.829326334748526)
(4.05, 11.07170245230594)
(4.125, 11.318692751471582)
(4.2, 11.569349833740334)
(4.275, 11.826200095125827)
(4.3500000000000005, 12.086480289988156)
(4.425, 12.353383502177877)
(4.5, 12.624786857266871)
(4.575, 12.90201495872062)
(4.65, 13.184050230366964)
(4.7250000000000005, 13.471182155082467)
(4.8, 13.766524866842264)
(4.875, 14.060990357763991)
(4.95, 14.36149112805161)
(5.025, 14.665711314692626)
(5.1000000000000005, 14.976545746452649)
(5.175, 15.291187316649879)
(5.25, 15.610565879372661)
(5.325, 15.93466389020423)
(5.4, 16.26228832880483)
(5.4750000000000005, 16.597588449738492)
(5.55, 16.935441283310926)
(5.625, 17.278496036453088)
(5.7, 17.62344558660547)
(5.775, 17.975369042420468)
(5.8500000000000005, 18.321678284871854)
(5.925, 18.656802961637904)
(6.0, 18.9758130916087)
(6.075, 19.294375838952078)
(6.15, 19.616736952524285)
(6.2250000000000005, 19.942966609992354)
(6.3, 20.27168757464053)
(6.375, 20.6044437551438)
(6.45, 20.941831661672065)
(6.525, 21.27927220145061)
(6.6000000000000005, 21.614861805260833)
(6.675, 21.959285022910375)
(6.75, 22.30384859589401)
(6.825, 22.651508758436016)
(6.9, 23.002774298622462)
(6.9750000000000005, 23.356417107280073)
(7.05, 23.713542482664803)
(7.125, 24.072246855558042)
(7.2, 24.433556574340344)
(7.275, 24.79469962116341)
(7.3500000000000005, 25.157562020829083)
(7.425, 25.5261175837338)
(7.5, 25.89628723298056)
(7.575, 26.26503578446965)
(7.65, 26.638565189526194)
(7.7250000000000005, 27.01100684074354)
(7.8, 27.37987820314996)
(7.875, 27.74118792193226)
(7.95, 28.10231342433856)
(8.025, 28.462210817571577)
(8.1, 28.822511732390097)
(8.175, 29.186216264060317)
(8.25, 29.549666401687492)
(8.325, 29.91620435666466)
(8.4, 30.28389147093969)
(8.475, 30.656298033323516)
(8.55, 31.024607974393575)
(8.625, 31.396225038023136)
(8.700000000000001, 31.766657853521313)
(8.775, 32.138836338487245)
(8.85, 32.51440966809648)
(8.925, 32.89260588801153)
(9.0, 33.271854772932265)
(9.075000000000001, 33.652673883153135)
(9.15, 34.03644922759828)
(9.225, 34.41764554277952)
(9.3, 34.80067524951231)
(9.375, 35.18436287187365)
(9.450000000000001, 35.56941018653399)
(9.525, 35.95182583868014)
(9.6, 36.33796967938807)
(9.675, 36.7217976570835)
(9.75, 37.105020352400665)
(9.825000000000001, 37.481427041806064)
(9.9, 37.8593600954697)
(9.975, 38.236670322338306)
(10.05, 38.61107694823292)
(10.125, 38.98563270167)
(10.200000000000001, 39.36175868040722)
(10.275, 39.739875950446844)
(10.35, 40.119502040327944)
(10.425, 40.498707064206776)
(10.5, 40.87638572382737)
(10.575000000000001, 41.25478370453518)
(10.65, 41.63051493389527)
(10.725, 42.00866729276842)
(10.8, 42.38917937569597)
(10.875, 42.76669136335733)
(10.950000000000001, 43.147335029410584)
(11.025, 43.52600494857819)
(11.1, 43.90498189503912)
(11.175, 44.278327083719674)
(11.25, 44.65147928381585)
(11.325000000000001, 45.02517536083163)
(11.4, 45.40063465173193)
(11.475, 45.77387457391191)
(11.55, 46.14314945790384)
(11.625, 46.515599881329564)
(11.700000000000001, 46.883778239273916)
(11.775, 47.252912767931754)
(11.85, 47.62036303258051)
(11.925, 47.98429564166862)
(12.0, 48.34517552224027)
(12.075000000000001, 48.70880110403506)
(12.15, 49.07140033744931)
(12.225, 49.437052299380035)
(12.3, 49.803520076690155)
(12.375, 50.166198259979836)
(12.450000000000001, 50.53033262986071)
(12.525, 50.89112478834854)
(12.6, 51.253259094718615)
(12.675, 51.61791979710233)
(12.75, 51.98498408458233)
(12.825000000000001, 52.34678504703395)
(12.9, 52.71499849381183)
(12.975, 53.08007148998942)
(13.05, 53.44649540625763)
(13.125, 53.81220000143864)
(13.200000000000001, 54.17943973308626)
(13.275, 54.54632857639865)
(13.35, 54.917147369065574)
(13.425, 55.285360815843454)
(13.5, 55.65650418022046)
(13.575000000000001, 56.02861248751934)
(13.65, 56.40597534763824)
(13.725, 56.783618918425304)
(13.8, 57.16114845050343)
(13.875, 57.548546717009785)
(13.950000000000001, 57.94012932691371)
(14.025, 58.337229655889075)
(14.1, 58.74267235503443)
(14.175, 59.15702761789453)
(14.25, 59.573698743767125)
(14.325000000000001, 60.002589555913964)
(14.4, 60.44111225286276)
(14.475, 60.898714503039486)
(14.55, 61.365132822638756)
(14.625, 61.846148096983434)
(14.700000000000001, 62.35343613542816)
(14.775, 62.88162834644398)
(14.85, 63.43895306149195)
(14.925, 64.02605065178385)
};
\addplot[solid, red, thick, mark = none] coordinates{
(0.002438603477429513,0.420515010855469)
(0.2462989512203808,0.47297935985492034)
(0.49015929896333216,0.616076830346433)
(0.7340196467062835,1.0961581325825946)
(0.9778799944492348,2.1043838823251493)
(1.2217403421921862,3.3859010439355166)
(1.4656006899351375,4.222146423713552)
(1.7094610376780888,5.031284389613893)
(1.95332138542104,5.886484953634819)
(2.1971817331639913,6.775069648215454)
(2.441042080906943,7.542229466425734)
(2.684902428649894,8.310664633443913)
(2.9287627763928454,9.085618249924687)
(3.1726231241357965,9.881444241666761)
(3.416483471878748,10.718156415779715)
(3.660343819621699,11.612259286248122)
(3.9042041673646506,12.547948530589784)
(4.148064515107602,13.483262672340885)
(4.391924862850553,14.404689682628199)
(4.635785210593505,15.349931539609415)
(4.879645558336456,16.322280810468328)
(5.123505906079407,17.334749387290756)
(5.367366253822358,18.376384274432393)
(5.61122660156531,19.458988700076137)
(5.855086949308261,20.558214338288188)
(6.098947297051212,21.643544509423325)
(6.3428076447941635,22.73135869326928)
(6.586667992537115,23.831384550341184)
(6.8305283402800665,24.94950702350426)
(7.074388688023018,26.09189446646991)
(7.318249035765969,27.244426350606894)
(7.56210938350892,28.41508819328753)
(7.805969731251872,29.591626643220252)
(8.049830078994823,30.773541563617652)
(8.293690426737774,31.946937487402806)
(8.537550774480726,33.132311687246464)
(8.781411122223677,34.32287897406607)
(9.025271469966627,35.529108877944786)
(9.26913181770958,36.74683359232083)
(9.51299216545253,37.965600258337325)
(9.756852513195483,39.17438919544495)
(10.000712860938433,40.37558438899706)
(10.244573208681384,41.57273681018425)
(10.488433556424337,42.7731317848765)
(10.732293904167287,43.978294730275394)
(10.97615425191024,45.1806569096648)
(11.22001459965319,46.378159426603176)
(11.46387494739614,47.568935103750874)
(11.707735295139093,48.745398533165485)
(11.951595642882044,49.897005164245755)
(12.195455990624994,51.05300466344212)
(12.439316338367947,52.20751208788938)
(12.683176686110897,53.36536209319915)
(12.92703703385385,54.53592390852231)
(13.1708973815968,55.72059791686359)
(13.414757729339751,56.92224323352437)
(13.658618077082703,58.13466649795386)
(13.902478424825654,59.39468611331866)
(14.146338772568607,60.70825370738897)
(14.390199120311557,62.15614970694485)
(14.634059468054508,64.30277847658002)
(14.87791981579746,77.72761683653813)
(15.12178016354041,99.95327888844265)
(15.365640511283363,99.99699917927553)
(15.609500859026314,99.99851626086401)
(15.853361206769264,99.99864129506086)
(16.097221554512217,99.99871631557897)
(16.34108190225517,99.99879967171022)
(16.584942249998118,99.99887469222833)
(16.82880259774107,99.9989413771333)
(17.072662945484023,99.9989747195858)
(17.31652329322697,99.99902473326455)
(17.560383640969924,99.99913309623516)
(17.804243988712877,99.99919978114015)
(18.048104336455825,99.99923312359263)
(18.291964684198778,99.99929980849763)
(18.53582503194173,99.999324815337)
(18.77968537968468,99.99937482901574)
(19.02354572742763,99.9993998358551)
(19.267406075170584,99.9994331783076)
(19.511266422913536,99.99944984953385)
(19.755126770656485,99.99947485637321)
(19.998987118399437,99.99948319198634)
(20.24284746614239,99.99948319198634)
(20.48670781388534,99.99952487005196)
(20.73056816162829,99.99956654811758)
(20.974428509371243,99.99959989057007)
(21.218288857114192,99.99960822618318)
(21.462149204857145,99.9996415686357)
(21.706009552600097,99.99964990424881)
(21.94986990034305,99.99964990424881)
(22.193730248086,99.99965823986193)
(22.43759059582895,99.99967491108819)
(22.681450943571903,99.99969158231443)
(22.925311291314852,99.99970825354067)
(23.169171639057804,99.99973326038005)
(23.413031986800757,99.99975826721942)
(23.656892334543706,99.99977493844567)
(23.900752682286658,99.9997916096719)
(24.14461303002961,99.9997916096719)
(24.38847337777256,99.9997916096719)
(24.63233372551551,99.99980828089816)
(24.876194073258464,99.99981661651128)
(25.120054421001417,99.99981661651128)
(25.363914768744365,99.9998249521244)
(25.607775116487318,99.99983328773753)
(25.85163546423027,99.99983328773753)
(26.09549581197322,99.99984162335065)
(26.33935615971617,99.99984162335065)
(26.583216507459124,99.99985829457691)
(26.827076855202073,99.99985829457691)
(27.070937202945025,99.99986663019003)
(27.314797550687977,99.99986663019003)
(27.55865789843093,99.99986663019003)
(27.80251824617388,99.99986663019003)
(28.04637859391683,99.99986663019003)
(28.290238941659783,99.99987496580314)
(28.534099289402732,99.99988330141628)
(28.777959637145685,99.99989163702939)
(29.021819984888637,99.99989163702939)
(29.265680332631586,99.99989163702939)
(29.50954068037454,99.99989163702939)
(29.75340102811749,99.99989997264251)
(29.99726137586044,99.99989997264251)
(30.241121723603392,99.99989997264251)
(30.484982071346344,99.99990830825564)
(30.728842419089297,99.99990830825564)
(30.972702766832246,99.99990830825564)
(31.216563114575198,99.99990830825564)
(31.46042346231815,99.99990830825564)
(31.7042838100611,99.99990830825564)
(31.94814415780405,99.99990830825564)
(32.192004505547004,99.99990830825564)
(32.43586485328996,99.99990830825564)
(32.67972520103291,99.99990830825564)
(32.923585548775854,99.99991664386877)
(33.16744589651881,99.99991664386877)
(33.41130624426176,99.99991664386877)
(33.65516659200471,99.99991664386877)
(33.899026939747664,99.99991664386877)
(34.142887287490616,99.99991664386877)
(34.38674763523356,99.99991664386877)
(34.630607982976514,99.99991664386877)
(34.874468330719466,99.99992497948189)
(35.11832867846242,99.99992497948189)
(35.36218902620537,99.99992497948189)
(35.60604937394832,99.99992497948189)
(35.849909721691276,99.99992497948189)
(36.09377006943422,99.99992497948189)
(36.337630417177174,99.99992497948189)
(36.581490764920126,99.99992497948189)
(36.82535111266308,99.99992497948189)
(37.06921146040603,99.99992497948189)
(37.31307180814898,99.99992497948189)
(37.55693215589193,99.99992497948189)
(37.80079250363488,99.99992497948189)
(38.04465285137783,99.99992497948189)
(38.288513199120786,99.99992497948189)
(38.53237354686374,99.99992497948189)
(38.77623389460669,99.999933315095)
(39.02009424234964,99.999933315095)
(39.26395459009259,99.999933315095)
(39.50781493783554,99.99994998632125)
(39.75167528557849,99.99994998632125)
(39.995535633321445,99.99994998632125)
(40.2393959810644,99.99994998632125)
(40.48325632880735,99.99994998632125)
(40.7271166765503,99.99994998632125)
(40.97097702429325,99.99994998632125)
(41.2148373720362,99.99994998632125)
(41.45869771977915,99.99994998632125)
(41.702558067522105,99.99994998632125)
(41.94641841526506,99.99994998632125)
(42.19027876300801,99.99994998632125)
(42.434139110750955,99.99994998632125)
(42.67799945849391,99.99994998632125)
(42.92185980623686,99.9999666575475)
(43.16572015397981,99.9999666575475)
(43.409580501722765,99.9999666575475)
(43.65344084946572,99.9999666575475)
(43.89730119720867,99.9999666575475)
(44.141161544951615,99.9999666575475)
(44.38502189269457,99.9999666575475)
(44.62888224043752,99.9999666575475)
(44.87274258818047,99.9999666575475)
(45.116602935923424,99.9999666575475)
(45.36046328366638,99.9999666575475)
(45.60432363140932,99.9999666575475)
(45.848183979152275,99.99997499316063)
(46.09204432689523,99.99997499316063)
(46.33590467463818,99.99997499316063)
(46.57976502238113,99.99998332877375)
(46.823625370124084,99.99998332877375)
(47.06748571786704,99.99998332877375)
(47.31134606560998,99.99998332877375)
(47.555206413352934,99.99998332877375)
(47.79906676109589,99.99998332877375)
(48.04292710883884,99.99998332877375)
(48.28678745658179,99.99998332877375)
(48.530647804324744,99.99999166438688)
};
\addplot[dashed, magenta, thick, mark = none] coordinates{
(0.0, 0.9132228167000467)
(0.075, 0.9406433190096234)
(0.15, 0.9704456021767475)
(0.225, 1.001518835633403)
(0.3, 1.0346836329523585)
(0.375, 1.070040068959561)
(0.45, 1.1073879940031162)
(0.525, 1.1485487699152657)
(0.6, 1.191460855281494)
(0.675, 1.2365745868185642)
(0.75, 1.2849407501989236)
(0.8250000000000001, 1.3361090087058094)
(0.9, 1.3918807092062735)
(0.975, 1.448933367478864)
(1.05, 1.5597362147677818)
(1.125, 1.8411466253317603)
(1.2, 1.9301131455989644)
(1.2750000000000001, 2.025114177870794)
(1.35, 2.1243383677976024)
(1.425, 2.2247634556357787)
(1.5, 2.328551057625787)
(1.575, 2.4406148477216414)
(1.6500000000000001, 2.5584229328268746)
(1.725, 2.68126478167726)
(1.8, 2.8120225492600817)
(1.875, 2.948104297583303)
(1.95, 3.091011149036134)
(2.025, 4.063898576965998)
(2.1, 4.281621368297076)
(2.1750000000000003, 4.439709570846122)
(2.25, 4.583757275314753)
(2.325, 4.728115211743821)
(2.4, 4.873443873984578)
(2.475, 5.022695469402472)
(2.5500000000000003, 5.176040125201613)
(2.625, 5.334608686915207)
(2.7, 5.497020121945178)
(2.775, 5.665466068979776)
(2.85, 5.8389958171725)
(2.9250000000000003, 6.014527061884171)
(3.0, 6.197413806302973)
(3.075, 6.392709829139247)
(3.15, 6.585894273148033)
(3.225, 6.779138762052386)
(3.3000000000000003, 6.975815817486734)
(3.375, 7.176936195193146)
(3.45, 7.380508406135268)
(3.525, 7.588483909419072)
(3.6, 7.805265997386246)
(3.6750000000000003, 8.028773113657081)
(3.75, 8.259815864321753)
(3.825, 8.503648177742498)
(3.9, 8.757077666971595)
(3.975, 9.041570382174752)
(4.05, 9.430371088462843)
(4.125, 9.651416364015375)
(4.2, 9.874753353082099)
(4.275, 10.102503641973103)
(4.3500000000000005, 10.336188368042786)
(4.425, 10.57376600484182)
(4.5, 10.814916312927176)
(4.575, 11.060279771184915)
(4.65, 11.312488347537455)
(4.7250000000000005, 11.564336654516582)
(4.8, 11.821649046992436)
(4.875, 12.086897373165916)
(4.95, 12.352355856473887)
(5.025, 12.620576404978001)
(5.1000000000000005, 12.903628042687517)
(5.175, 13.181305662243659)
(5.25, 13.462355803434228)
(5.325, 13.7460579275124)
(5.4, 14.03535423436103)
(5.4750000000000005, 14.326702075141585)
(5.55, 14.623574046314431)
(5.625, 14.926780753969743)
(5.7, 15.233800312493651)
(5.775, 15.547845123799064)
(5.8500000000000005, 15.86954565928945)
(5.925, 16.19391819263263)
(6.0, 16.524595440010494)
(6.075, 16.871424764296265)
(6.15, 17.17076858367001)
(6.2250000000000005, 17.47143339074626)
(6.3, 17.771537778797207)
(6.375, 18.075214838134475)
(6.45, 18.380553139582464)
(6.525, 18.689324007560455)
(6.6000000000000005, 18.999175683658674)
(6.675, 19.309587778782195)
(6.75, 19.623962837013234)
(6.825, 19.94306142702899)
(6.9, 20.2599583708739)
(6.9750000000000005, 20.58032791117919)
(7.05, 20.910855046318133)
(7.125, 21.23875021353466)
(7.2, 21.56734590453282)
(7.275, 21.899504259334705)
(7.3500000000000005, 22.233594058277372)
(7.425, 22.573268032507908)
(7.5, 22.913732597863422)
(7.575, 23.255348023717335)
(7.65, 23.602877871784735)
(7.7250000000000005, 23.948396215850593)
(7.8, 24.29987901954291)
(7.875, 24.647839189361886)
(7.95, 24.99294722664136)
(8.025, 25.361192563679865)
(8.1, 25.69646324556871)
(8.175, 26.03181398731832)
(8.25, 26.36762507326728)
(8.325, 26.705167453705137)
(8.4, 27.046902969350185)
(8.475, 27.388708537373397)
(8.55, 27.734867360325318)
(8.625, 28.079044701723475)
(8.700000000000001, 28.42402264172922)
(8.775, 28.772463170712744)
(8.85, 29.12335553293197)
(8.925, 29.475739010057822)
(9.0, 29.830674395245328)
(9.075000000000001, 30.189622780953318)
(9.15, 30.545138600131317)
(9.225, 30.905578100745927)
(9.3, 31.26446644155835)
(9.375, 31.62747786519981)
(9.450000000000001, 31.988117515466314)
(9.525, 32.34969786909672)
(9.6, 32.71727270480138)
(9.675, 33.081324906632695)
(9.75, 33.447478679808896)
(9.825000000000001, 33.81425291690597)
(9.9, 34.17380175156965)
(9.975, 34.53548218002601)
(10.05, 34.90890138556599)
(10.125, 35.26690906791007)
(10.200000000000001, 35.62822922699303)
(10.275, 35.98926917656332)
(10.35, 36.3522405702744)
(10.425, 36.71332054977507)
(10.5, 37.07424040955422)
(10.575000000000001, 37.43762211005169)
(10.65, 37.79999305480708)
(10.725, 38.16323465054822)
(10.8, 38.531850264442724)
(10.875, 38.897753850554054)
(10.950000000000001, 39.26676976375236)
(11.025, 39.63466483890004)
(11.1, 40.005061784696416)
(11.175, 40.376049171965875)
(11.25, 40.74973857953592)
(11.325000000000001, 41.11704321321052)
(11.4, 41.49265405743875)
(11.475, 41.86533270926672)
(11.55, 42.235419423102655)
(11.625, 42.60588642127719)
(11.700000000000001, 42.97633340448653)
(11.775, 43.34552945237154)
(11.85, 43.71889862049855)
(11.925, 44.089966067628765)
(12.0, 44.46026293859919)
(12.075000000000001, 44.84107767377668)
(12.15, 45.21267551748443)
(12.225, 45.58376297957983)
(12.3, 45.95780264904069)
(12.375, 46.32883006624053)
(12.450000000000001, 46.70458101522508)
(12.525, 47.07748983915273)
(12.6, 47.45247021197749)
(12.675, 47.83039278468511)
(12.75, 48.208685634248724)
(12.825000000000001, 48.59138177615403)
(12.9, 48.97563908534411)
(12.975, 49.362458310078445)
(13.05, 49.75161928573995)
(13.125, 50.144963389126055)
(13.200000000000001, 50.53743684152641)
(13.275, 50.929149725249566)
(13.35, 51.32481556459765)
(13.425, 51.72268305011657)
(13.5, 52.12825629723344)
(13.575000000000001, 52.53857309110022)
(13.65, 52.95027091756507)
(13.725, 53.37287690005817)
(13.8, 53.794241954709534)
(13.875, 54.22271232200316)
(13.950000000000001, 54.6604796406273)
(14.025, 55.169440190430386)
(14.1, 55.79581853351752)
(14.175, 56.45075823193001)
(14.25, 57.12428182552094)
(14.325000000000001, 57.81962173116839)
(14.4, 58.54351298465863)
(14.475, 59.30812468482684)
(14.55, 60.105390800701684)
(14.625, 60.933720142550584)
(14.700000000000001, 61.80875440566912)
(14.775, 66.05816168749374)
(14.85, 76.73958819008972)
(14.925, 88.14040257900832)
};
\addplot[dashed, black, thick, mark = none] coordinates{
(0.0, 0.5978301732190421)
(0.075, 0.6133760916944118)
(0.15, 0.6302307014301745)
(0.225, 0.6474937562089899)
(0.3, 0.6658404406938631)
(0.375, 0.6855625013441176)
(0.45, 0.7072100886259058)
(0.525, 0.729924634387505)
(0.6, 0.7542562890950675)
(0.675, 0.7787713272913476)
(0.75, 0.8055703234834727)
(0.8250000000000001, 0.8346949557370608)
(0.9, 0.8651199436379183)
(0.975, 0.8980706223152032)
(1.05, 0.9571367769084845)
(1.125, 1.0989005493002337)
(1.2, 1.1451548665226605)
(1.2750000000000001, 1.1934430733472272)
(1.35, 1.2504586671121218)
(1.425, 1.3082328016712572)
(1.5, 1.3678491067306908)
(1.575, 1.431733245709368)
(1.6500000000000001, 1.5001519582272418)
(1.725, 1.5731302511236822)
(1.8, 1.6536022602181697)
(1.875, 1.7413345883432452)
(1.95, 1.8342933458967696)
(2.025, 2.4780944254920385)
(2.1, 2.60748814800848)
(2.1750000000000003, 2.7090742651448503)
(2.25, 2.8046754120585313)
(2.325, 2.9040109136515504)
(2.4, 3.005847099181626)
(2.475, 3.113043083950127)
(2.5500000000000003, 3.2260573266788466)
(2.625, 3.3446564302003265)
(2.7, 3.4692071614920015)
(2.775, 3.6020601634547047)
(2.85, 3.7420984639298847)
(2.9250000000000003, 3.8896138093768644)
(3.0, 4.044789583284362)
(3.075, 4.211743578535397)
(3.15, 4.3851493383440365)
(3.225, 4.567940998529765)
(3.3000000000000003, 4.762994345620194)
(3.375, 4.968975681515561)
(3.45, 5.1898861005151575)
(3.525, 5.4273593827911935)
(3.6, 5.676210776980837)
(3.6750000000000003, 5.947368271889028)
(3.75, 6.237430937361369)
(3.825, 6.549357916056708)
(3.9, 6.891509827937941)
(3.975, 7.275306462984293)
(4.05, 7.7634899811765194)
(4.125, 8.116119758754019)
(4.2, 8.48711289204264)
(4.275, 8.87052608888531)
(4.3500000000000005, 9.27121067611992)
(4.425, 9.682389800277043)
(4.5, 10.10815624740033)
(4.575, 10.5434836427763)
(4.65, 10.981970235526083)
(4.7250000000000005, 11.424399573283294)
(4.8, 11.862452714150654)
(4.875, 12.295629521340754)
(4.95, 12.727806054956032)
(5.025, 13.160140965220654)
(5.1000000000000005, 13.587757918457367)
(5.175, 14.010456859951196)
(5.25, 14.423828250359808)
(5.325, 14.839166845465568)
(5.4, 15.251346243197514)
(5.4750000000000005, 15.66676819443451)
(5.55, 16.075063196450895)
(5.625, 16.484250109071496)
(5.7, 16.894520651398157)
(5.775, 17.309109041322802)
(5.8500000000000005, 17.720679939296733)
(5.925, 18.130767098134672)
(6.0, 18.538695333173624)
(6.075, 18.95191668254601)
(6.15, 19.333304325399663)
(6.2250000000000005, 19.705797869050517)
(6.3, 20.07650759149294)
(6.375, 20.44800086156897)
(6.45, 20.81621823568746)
(6.525, 21.186994643034872)
(6.6000000000000005, 21.553469874010542)
(6.675, 21.92303761745504)
(6.75, 22.287362260244844)
(6.825, 22.653379032498723)
(6.9, 23.022079872178374)
(6.9750000000000005, 23.391764314206604)
(7.05, 23.76241568735716)
(7.125, 24.13397564233818)
(7.2, 24.505969049201624)
(7.275, 24.879329496617324)
(7.3500000000000005, 25.253565183411)
(7.425, 25.62804260298525)
(7.5, 26.006062658137)
(7.575, 26.38009829021571)
(7.65, 26.755175873934856)
(7.7250000000000005, 27.127711095651325)
(7.8, 27.496295236747248)
(7.875, 27.869213896667404)
(7.95, 28.23931511935181)
(8.025, 28.617751955159736)
(8.1, 28.98364369321676)
(8.175, 29.34897694519451)
(8.25, 29.720561907014904)
(8.325, 30.09275536859331)
(8.4, 30.46615749407463)
(8.475, 30.84332731668778)
(8.55, 31.21890503719434)
(8.625, 31.598592214970793)
(8.700000000000001, 31.97865449533781)
(8.775, 32.36687734095275)
(8.85, 32.75448335119655)
(8.925, 33.146215489936495)
(9.0, 33.53790595061083)
(9.075000000000001, 33.9300381987807)
(9.15, 34.32471280895325)
(9.225, 34.71945410403078)
(9.3, 35.11671275427163)
(9.375, 35.51023704983313)
(9.450000000000001, 35.905778563770525)
(9.525, 36.295701874462665)
(9.6, 36.69002638888403)
(9.675, 37.08318391746809)
(9.75, 37.47364070740014)
(9.825000000000001, 37.86537284614009)
(9.9, 38.250669891548675)
(9.975, 38.637117251568306)
(10.05, 39.027840781120304)
(10.125, 39.411112272539874)
(10.200000000000001, 39.790757772250714)
(10.275, 40.16463502768007)
(10.35, 40.53541143502748)
(10.425, 40.90880522489568)
(10.5, 41.273504970276036)
(10.575000000000001, 41.638121359525165)
(10.65, 41.998494921694416)
(10.725, 42.358118278682554)
(10.8, 42.71624122530845)
(10.875, 43.066195271073305)
(10.950000000000001, 43.41125631193465)
(11.025, 43.754591880879424)
(11.1, 44.08891665203766)
(11.175, 44.42049900647827)
(11.25, 44.75122279276715)
(11.325000000000001, 45.072352288350864)
(11.4, 45.39109779858125)
(11.475, 45.70932650079797)
(11.55, 46.02420428653903)
(11.625, 46.337431620881645)
(11.700000000000001, 46.65159254389409)
(11.775, 46.966295281759564)
(11.85, 47.28467402501251)
(11.925, 47.59957681759294)
(12.0, 47.9187391084795)
(12.075000000000001, 48.24137735003857)
(12.15, 48.56677467954152)
(12.225, 48.8958313432057)
(12.3, 49.22941424479595)
(12.375, 49.56739835011542)
(12.450000000000001, 49.914426595673916)
(12.525, 50.266964681507055)
(12.6, 50.62702149037762)
(12.675, 50.99723941164576)
(12.75, 51.37682656206473)
(12.825000000000001, 51.76616637983822)
(12.9, 52.16448365294575)
(12.975, 52.573937305186305)
(13.05, 52.996636246680126)
(13.125, 53.435272880466144)
(13.200000000000001, 53.89191443859895)
(13.275, 54.3584170270569)
(13.35, 54.83736468590826)
(13.425, 55.33235006440928)
(13.5, 55.835370973961375)
(13.575000000000001, 56.34455190161176)
(13.65, 56.86528598905134)
(13.725, 57.39508088795618)
(13.8, 57.92813501159234)
(13.875, 58.46749085874987)
(13.950000000000001, 59.008280431364646)
(14.025, 59.609169774600026)
(14.1, 60.313295686370225)
(14.175, 61.02494865679097)
(14.25, 61.75203918271648)
(14.325000000000001, 62.49846833108855)
(14.4, 63.252357853206185)
(14.475, 64.02990384536838)
(14.55, 64.82927247268795)
(14.625, 65.65083883775546)
(14.700000000000001, 66.52143527921554)
(14.775, 70.33132728467902)
(14.85, 79.65141799615529)
(14.925, 89.58084202696104)
};
