# Supplementary material for: CausalSim: A Causal Framework for Unbiased Trace-Driven Simulation
Source: arXiv:2201.01811 source file (2023-05-05)
Supplement: Supplementary file 3 [file new_bola_basic_v1_puffer_ttp_20190202.tex]

\addplot[solid, green!70!black, thick, mark = none] coordinates{
(0.0, 0.38093833833083757)
(0.07980200171551347, 0.38887472157193564)
(0.15960400343102693, 0.3998970284489124)
(0.23940600514654037, 0.4144322927808321)
(0.31920800686205386, 0.4358081554596475)
(0.3990100085775673, 0.47983292503260166)
(0.47881201029308074, 0.5660292985486087)
(0.5586140120085942, 0.7064911960532406)
(0.6384160137241077, 0.9579577147889465)
(0.7182180154396212, 1.3815672060587236)
(0.7980200171551346, 1.8658396713612186)
(0.877822018870648, 2.30170422751395)
(0.9576240205861615, 2.6587770154284094)
(1.037426022301675, 2.9349148087674073)
(1.1172280240171883, 3.1744968957461386)
(1.197030025732702, 3.388303865985508)
(1.2768320274482154, 3.5973087200708713)
(1.3566340291637289, 3.806096028625769)
(1.4364360308792423, 4.014085670235621)
(1.5162380325947558, 4.222188113231643)
(1.5960400343102692, 4.43134605491252)
(1.6758420360257826, 4.636991039138455)
(1.755644037741296, 4.842128417126634)
(1.8354460394568095, 5.05149584709611)
(1.915248041172323, 5.2639733724270705)
(1.9950500428878366, 5.482614687787921)
(2.07485204460335, 5.697509385679622)
(2.1546540463188633, 5.903823120980696)
(2.2344560480343767, 6.100170048089648)
(2.3142580497498906, 6.289732777544789)
(2.394060051465404, 6.479940086349462)
(2.4738620531809175, 6.671605755932447)
(2.553664054896431, 6.863811260720663)
(2.6334660566119443, 7.055106297177669)
(2.7132680583274578, 7.248125583394669)
(2.793070060042971, 7.443521755963064)
(2.8728720617584846, 7.639780053411456)
(2.952674063473998, 7.83677961711181)
(3.0324760651895115, 8.03678453202935)
(3.112278066905025, 8.241148414798092)
(3.1920800686205384, 8.445778186548516)
(3.271882070336052, 8.650601332103799)
(3.3516840720515653, 8.85953367101234)
(3.4314860737670787, 9.072373772227413)
(3.511288075482592, 9.28545559069856)
(3.5910900771981056, 9.504419195734174)
(3.670892078913619, 9.727910970700243)
(3.7506940806291325, 9.948574653770246)
(3.830496082344646, 10.173275015016685)
(3.9102980840601598, 10.400916269545359)
(3.990100085775673, 10.630644349718137)
(4.069902087491187, 10.864521909453522)
(4.1497040892067, 11.09929382303638)
(4.2295060909222135, 11.336676282984838)
(4.3093080926377265, 11.576258369963568)
(4.38911009435324, 11.822044533181534)
(4.468912096068753, 12.069756377206224)
(4.548714097784267, 12.321255124909406)
(4.628516099499781, 12.576258772825662)
(4.708318101215294, 12.834710920261907)
(4.788120102930808, 13.094935660909366)
(4.867922104646321, 13.357545345150085)
(4.947724106361835, 13.620710979079774)
(5.027526108077348, 13.88820335189319)
(5.107328109792862, 14.1588299917937)
(5.187130111508375, 14.430753847635138)
(5.266932113223889, 14.709679446660855)
(5.346734114939402, 14.989136823649938)
(5.4265361166549155, 15.269448268277147)
(5.5063381183704285, 15.555174179440417)
(5.586140120085942, 15.8430110879734)
(5.665942121801455, 16.133619687709363)
(5.745744123516969, 16.427394783499896)
(5.825546125232482, 16.724320260861266)
(5.905348126947996, 17.023807941137015)
(5.985150128663509, 17.326873036802663)
(6.064952130379023, 17.629688357970362)
(6.144754132094536, 17.93890918642403)
(6.22455613381005, 18.247662694849286)
(6.304358135525564, 18.56374023613359)
(6.384160137241077, 18.87895565253789)
(6.463962138956591, 19.199698336864422)
(6.543764140672104, 19.523470544133744)
(6.6235661423876175, 19.849506836368295)
(6.7033681441031305, 20.180715877882832)
(6.783170145818644, 20.514309862990633)
(6.862972147534157, 20.84961198337469)
(6.942774149249671, 21.189031354353872)
(7.022576150965184, 21.531069328940525)
(7.102378152680698, 21.876491345112214)
(7.182180154396211, 22.221776388172128)
(7.261982156111725, 22.568914596861948)
(7.341784157827238, 22.91849414983811)
(7.421586159542752, 23.271240198868846)
(7.501388161258265, 23.625339864533593)
(7.581190162973779, 23.98327477732805)
(7.660992164689292, 24.344094182711657)
(7.740794166404806, 24.70729047444666)
(7.8205961681203195, 25.073226228417166)
(7.9003981698358325, 25.439000837550292)
(7.980200171551346, 25.808328690347704)
(8.06000217326686, 26.179437193598197)
(8.139804174982373, 26.55531558403522)
(8.219606176697887, 26.931548493114484)
(8.2994081784134, 27.30835346636645)
(8.379210180128913, 27.688832541910752)
(8.459012181844427, 28.071043924456912)
(8.538814183559941, 28.455269617470357)
(8.618616185275453, 28.843048554148087)
(8.698418186990967, 29.230714689439658)
(8.77822018870648, 29.622538361535693)
(8.858022190421995, 30.0157801082007)
(8.937824192137507, 30.41330830754009)
(9.01762619385302, 30.813624312566194)
(9.097428195568535, 31.214496267281273)
(9.177230197284048, 31.614578612293176)
(9.257032198999562, 32.016095146357785)
(9.336834200715074, 32.420729833025746)
(9.416636202430588, 32.824115647203996)
(9.496438204146102, 33.233665251412134)
(9.576240205861616, 33.64325514182961)
(9.656042207577128, 34.0536024129828)
(9.735844209292642, 34.4638127110242)
(9.815646211008156, 34.8742324973542)
(9.89544821272367, 35.28590921341579)
(9.975250214439182, 35.69814187916635)
(10.055052216154696, 36.11449985275391)
(10.13485421787021, 36.53309773958108)
(10.214656219585724, 36.95039841046732)
(10.294458221301236, 37.36778771101413)
(10.37426022301675, 37.78803733242448)
(10.454062224732263, 38.21080081329799)
(10.533864226447777, 38.63068785882423)
(10.61366622816329, 39.052395841012896)
(10.693468229878803, 39.47461948668118)
(10.773270231594317, 39.89809200483918)
(10.853072233309831, 40.32207212923494)
(10.932874235025345, 40.74863057102881)
(11.012676236740857, 41.17004043526832)
(11.092478238456371, 41.59742071573285)
(11.172280240171885, 42.02249662502281)
(11.252082241887399, 42.448007625373705)
(11.33188424360291, 42.872656500844606)
(11.411686245318425, 43.30016569717904)
(11.491488247033939, 43.7247984581662)
(11.571290248749452, 44.15238016967746)
(11.651092250464965, 44.584336963523654)
(11.730894252180478, 45.013860470325376)
(11.810696253895992, 45.442795798470655)
(11.890498255611506, 45.870659513447336)
(11.970300257327018, 46.30105320237092)
(12.050102259042532, 46.732462103770025)
(12.129904260758046, 47.163943520345946)
(12.20970626247356, 47.596367634220556)
(12.289508264189072, 48.025576908589386)
(12.369310265904586, 48.45814605281763)
(12.4491122676201, 48.89364803308626)
(12.528914269335614, 49.330850091389266)
(12.608716271051128, 49.76810855038536)
(12.68851827276664, 50.210547815903304)
(12.768320274482154, 50.65758776652852)
(12.848122276197667, 51.10656951244421)
(12.927924277913181, 51.56010360001595)
(13.007726279628693, 52.01963227553833)
(13.087528281344207, 52.477976536505956)
(13.167330283059721, 52.93960815215618)
(13.247132284775235, 53.40371334106023)
(13.326934286490747, 53.87463495658557)
(13.406736288206261, 54.35066486345593)
(13.486538289921775, 54.833317823142735)
(13.566340291637289, 55.33088473752931)
(13.646142293352801, 55.840150767109854)
(13.725944295068315, 56.36238089885784)
(13.805746296783829, 56.897881307964305)
(13.885548298499343, 57.45149439679257)
(13.965350300214856, 58.020222871367345)
(14.045152301930369, 58.60815981055813)
(14.124954303645882, 59.22869635035144)
(14.204756305361396, 59.87696591665831)
(14.28455830707691, 60.570017633273835)
(14.364360308792422, 61.333771647291016)
(14.444162310507936, 62.198756848152016)
(14.52396431222345, 63.25068617486068)
(14.603766313938964, 64.70249641553453)
(14.683568315654476, 66.93935596048567)
(14.76337031736999, 70.96961251515265)
(14.843172319085504, 88.32556413786102)
(14.922974320801018, 94.6278823272054)
(15.00277632251653, 96.35682945921002)
(15.082578324232044, 97.45995450075516)
(15.162380325947558, 98.17333463860652)
(15.242182327663071, 98.66683264584917)
(15.321984329378584, 99.07736523356535)
(15.401786331094097, 99.40562532455577)
(15.481588332809611, 99.6412674202605)
(15.561390334525125, 99.80179990726114)
(15.641192336240639, 99.9036192727614)
(15.720994337956151, 99.96197787561955)
(15.800796339671665, 99.99083085875291)
(15.880598341387179, 99.99941987858543)
};
\addplot[solid, blue, thick, mark = none] coordinates{
(0.0, 0.3778583782504472)
(0.075, 0.3778583782504472)
(0.15, 0.3778583782504472)
(0.225, 0.3778583782504472)
(0.3, 0.3778583782504472)
(0.375, 0.3778583782504472)
(0.45, 0.3778583782504472)
(0.525, 0.3778583782504472)
(0.6, 0.3778583782504472)
(0.675, 0.3778583782504472)
(0.75, 0.3778583782504472)
(0.8250000000000001, 0.3778583782504472)
(0.9, 0.3778583782504472)
(0.975, 0.3778583782504472)
(1.05, 0.3778583782504472)
(1.125, 0.3778583782504472)
(1.2, 0.3778583782504472)
(1.2750000000000001, 0.3778583782504472)
(1.35, 0.3778583782504472)
(1.425, 0.3778583782504472)
(1.5, 0.3778583782504472)
(1.575, 0.3778583782504472)
(1.6500000000000001, 0.3778583782504472)
(1.725, 0.3778583782504472)
(1.8, 0.3778583782504472)
(1.875, 0.3778583782504472)
(1.95, 0.3778583782504472)
(2.025, 4.844207112942016)
(2.1, 4.987301208385164)
(2.1750000000000003, 5.1370831381295075)
(2.25, 5.29120151075195)
(2.325, 5.450073783425434)
(2.4, 5.611050381031904)
(2.475, 5.780691344860434)
(2.5500000000000003, 5.955622939390927)
(2.625, 6.13711457521049)
(2.7, 6.323300474342103)
(2.775, 6.516242364048043)
(2.85, 6.717678229293209)
(2.9250000000000003, 6.925401510734912)
(3.0, 7.142223654639896)
(3.075, 7.3643619878492705)
(3.15, 7.59432977293482)
(3.225, 7.83374572138346)
(3.3000000000000003, 8.077796296405158)
(3.375, 8.327231217004377)
(3.45, 8.58705996925641)
(3.525, 8.854079208323993)
(3.6, 9.125894945113327)
(3.6750000000000003, 9.405744602598237)
(3.75, 9.695732505711709)
(3.825, 9.998610463981498)
(3.9, 10.31111549583135)
(3.975, 10.615373618632084)
(4.05, 10.85276191795501)
(4.125, 11.09381361695885)
(4.2, 11.335700230308566)
(4.275, 11.585407776000318)
(4.3500000000000005, 11.839477323172597)
(4.425, 12.100004677224243)
(4.5, 12.363854649591135)
(4.575, 12.630797212851444)
(4.65, 12.901863230636312)
(4.7250000000000005, 13.178569180022953)
(4.8, 13.458171771017755)
(4.875, 13.744896692554976)
(4.95, 14.03303585675971)
(5.025, 14.32947304721841)
(5.1000000000000005, 14.627537468698169)
(5.175, 14.92785956672546)
(5.25, 15.232381795084587)
(5.325, 15.542467279238211)
(5.4, 15.857264065772167)
(5.4750000000000005, 16.17669547887918)
(5.55, 16.502542101194855)
(5.625, 16.830211903816846)
(5.7, 17.162686723694726)
(5.775, 17.499003853470487)
(5.8500000000000005, 17.835636206009493)
(5.925, 18.166262286978633)
(6.0, 18.479269971342845)
(6.075, 18.78897207646009)
(6.15, 19.098938287135734)
(6.2250000000000005, 19.414757417766687)
(6.3, 19.734410338761386)
(6.375, 20.055230435933485)
(6.45, 20.375036708542734)
(6.525, 20.70153081545317)
(6.6000000000000005, 21.02582688255507)
(6.675, 21.358318741501233)
(6.75, 21.69361352718)
(6.825, 22.029871020216767)
(6.9, 22.36798577169642)
(6.9750000000000005, 22.707131386807212)
(7.05, 23.051763581905224)
(7.125, 23.39624242538869)
(7.2, 23.74676161857858)
(7.275, 24.09770678847556)
(7.3500000000000005, 24.44972541967438)
(7.425, 24.803447957701536)
(7.5, 25.16068906332919)
(7.575, 25.518909915383137)
(7.65, 25.877326716722337)
(7.7250000000000005, 26.235394217161733)
(7.8, 26.598283773925303)
(7.875, 26.95693060268633)
(7.95, 27.312765985180608)
(8.025, 27.66300403374383)
(8.1, 28.01437518034789)
(8.175, 28.367169089153606)
(8.25, 28.72107905693187)
(8.325, 29.079146557371267)
(8.4, 29.437963776815128)
(8.475, 29.79695138694182)
(8.55, 30.157336200667746)
(8.625, 30.523011645095632)
(8.700000000000001, 30.886472010646692)
(8.775, 31.252334884825693)
(8.85, 31.618990075679875)
(8.925, 31.98601160650214)
(9.0, 32.35975504976217)
(9.075000000000001, 32.72982657380715)
(9.15, 33.10199390325098)
(9.225, 33.47560103396474)
(9.3, 33.85119321613351)
(9.375, 34.22677687876814)
(9.450000000000001, 34.60144043171546)
(9.525, 34.978796157451555)
(9.6, 35.35979824380027)
(9.675, 35.738636368477)
(9.75, 36.1154809221646)
(9.825000000000001, 36.48949699051716)
(9.9, 36.86114462837835)
(9.975, 37.23294561785408)
(10.05, 37.603894653915646)
(10.125, 37.97473293603338)
(10.200000000000001, 38.345000409363614)
(10.275, 38.719902509266916)
(10.35, 39.0907322718505)
(10.425, 39.463265941262414)
(10.5, 39.8367963961689)
(10.575000000000001, 40.211553663991786)
(10.65, 40.58507559936413)
(10.725, 40.959372812343375)
(10.8, 41.333388880695935)
(10.875, 41.70769461320932)
(10.950000000000001, 42.0807735328063)
(11.025, 42.455317812275645)
(11.1, 42.83142116649291)
(11.175, 43.204414890748474)
(11.25, 43.5798537213027)
(11.325000000000001, 43.95789952930426)
(11.4, 44.33065470660386)
(11.475, 44.7032139346182)
(11.55, 45.07449523251129)
(11.625, 45.445129045809615)
(11.700000000000001, 45.81680224227323)
(11.775, 46.186319996599)
(11.85, 46.5526940428265)
(11.925, 46.92170062510378)
(12.0, 47.28860288244807)
(12.075000000000001, 47.65515583889254)
(12.15, 48.020013408042836)
(12.225, 48.38865365035201)
(12.3, 48.75508733331851)
(12.375, 49.12432394301761)
(12.450000000000001, 49.4950940688622)
(12.525, 49.86270344754025)
(12.6, 50.234461839345265)
(12.675, 50.60571757863593)
(12.75, 50.97404259818188)
(12.825000000000001, 51.34506831005072)
(12.9, 51.71403229465729)
(12.975, 52.08828690996582)
(13.05, 52.458571422364344)
(13.125, 52.8330986627654)
(13.200000000000001, 53.21214125626154)
(13.275, 53.59097086140413)
(13.35, 53.97043091207321)
(13.425, 54.35070883801989)
(13.5, 54.73538284358366)
(13.575000000000001, 55.11993757566944)
(13.65, 55.507431547034095)
(13.725, 55.89923640267441)
(13.8, 56.30118802347746)
(13.875, 56.705763660796116)
(13.950000000000001, 57.11352560388375)
(14.025, 57.52751532642893)
(14.1, 57.94894260227977)
(14.175, 58.38061887770303)
(14.25, 58.817440951747834)
(14.325000000000001, 59.2661392563861)
(14.4, 59.72990009738679)
(14.475, 60.20751370090181)
(14.55, 60.695802280696334)
(14.625, 61.20406064851886)
(14.700000000000001, 61.73962412326539)
(14.775, 62.295072190698534)
(14.85, 62.88179546796566)
(14.925, 63.50310805384789)
};
\addplot[solid, red, thick, mark = none] coordinates{
(0.002369915769453915,0.38147817353606966)
(0.23936149271484541,0.42973299509031965)
(0.47635306966023694,0.5577947973583527)
(0.7133446466056284,0.9887605504546501)
(0.9503362235510199,1.9457433389774312)
(1.1873278004964114,3.33378051025707)
(1.4243193774418028,4.151687246876711)
(1.6613109543871944,4.919171763879304)
(1.8983025313325859,5.719690972545352)
(2.1352941082779773,6.600113848827611)
(2.372285685223369,7.3659144022795555)
(2.60927726216876,8.109783143363714)
(2.8462688391141517,8.852330496781333)
(3.0832604160595434,9.605932386043408)
(3.3202519930049346,10.384237778876248)
(3.557243569950326,11.198091722835715)
(3.794235146895718,12.062263142267929)
(4.031226723841109,12.980546998093253)
(4.268218300786501,13.883344835046103)
(4.505209877731892,14.773718405036742)
(4.742201454677284,15.682156311297984)
(4.979193031622675,16.618472274426434)
(5.216184608568066,17.58120793364378)
(5.453176185513458,18.573602300181406)
(5.69016776245885,19.596590014096144)
(5.927159339404241,20.650179132629855)
(6.164150916349633,21.688959040608097)
(6.4011424932950245,22.71606400511796)
(6.638134070240415,23.75249925571228)
(6.875125647185807,24.804742814853846)
(7.1121172241311985,25.880513520253288)
(7.34910880107659,26.966766697324474)
(7.586100378021982,28.072341140397842)
(7.8230919549673725,29.192136615370234)
(8.060083531912763,30.312818386948237)
(8.297075108858156,31.429672968638396)
(8.534066685803548,32.55201453204143)
(8.771058262748937,33.6794402150639)
(9.00804983969433,34.81408518680111)
(9.245041416639722,35.95765758252932)
(9.482032993585115,37.116442050906464)
(9.719024570530504,38.26899827131876)
(9.956016147475896,39.41466554993294)
(10.193007724421289,40.55574825792359)
(10.429999301366678,41.68899126957557)
(10.66699087831207,42.83382865227724)
(10.903982455257463,43.975958801710874)
(11.140974032202855,45.1266537992514)
(11.377965609148244,46.26926738319719)
(11.614957186093637,47.40287297073328)
(11.85194876303903,48.51663357154569)
(12.088940339984418,49.63151412897791)
(12.325931916929811,50.74474295182696)
(12.562923493875203,51.86755183525841)
(12.799915070820592,53.00513770027785)
(13.036906647765985,54.15244865623335)
(13.273898224711377,55.319749629266155)
(13.51088980165677,56.50775771390265)
(13.747881378602159,57.73092760205605)
(13.984872955547551,59.00953131426909)
(14.221864532492944,60.359771963940624)
(14.458856109438333,61.89916442373195)
(14.695847686383726,64.72317129817073)
(14.932839263329118,97.88128379257599)
(15.16983084027451,99.96680416349916)
(15.4068224172199,99.99640647012636)
(15.643813994165292,99.99850135301233)
(15.880805571110685,99.9987994709615)
(16.117797148056077,99.99888810062207)
(16.354788725001466,99.99899284476635)
(16.59178030194686,99.9991137033944)
(16.828771878892248,99.99919427581308)
(17.06576345583764,99.99925873374804)
(17.302755032783033,99.99930707719925)
(17.539746609728425,99.9993473634086)
(17.776738186673818,99.99937959237609)
(18.013729763619207,99.99941182134356)
(18.2507213405646,99.99941182134356)
(18.487712917509988,99.99944405031103)
(18.72470449445538,99.99950045100411)
(18.961696071400773,99.99952462272972)
(19.198687648346166,99.99954073721345)
(19.43567922529156,99.99958908066468)
(19.672670802236947,99.9996051951484)
(19.909662379182336,99.99962936687402)
(20.14665395612773,99.99963742411589)
(20.38364553307312,99.99964548135776)
(20.620637110018514,99.99965353859963)
(20.857628686963906,99.99966159584149)
(21.0946202639093,99.99966965308337)
(21.331611840854688,99.99969382480897)
(21.568603417800077,99.99969382480897)
(21.80559499474547,99.99969382480897)
(22.04258657169086,99.99970188205084)
(22.279578148636254,99.99973411101833)
(22.516569725581647,99.99973411101833)
(22.753561302527036,99.99975022550205)
(22.99055287947243,99.99975828274393)
(23.227544456417817,99.99977439722765)
(23.46453603336321,99.99978245446954)
(23.701527610308602,99.99978245446954)
(23.938519187253995,99.99978245446954)
(24.175510764199387,99.99979051171141)
(24.412502341144776,99.99979856895327)
(24.64949391809017,99.99981468343701)
(24.886485495035558,99.99981468343701)
(25.12347707198095,99.99982274067888)
(25.360468648926343,99.99983079792075)
(25.597460225871735,99.99983885516261)
(25.834451802817128,99.99983885516261)
(26.071443379762517,99.9998469124045)
(26.30843495670791,99.99985496964635)
(26.5454265336533,99.99987108413009)
(26.78241811059869,99.99988719861383)
(27.019409687544083,99.99988719861383)
(27.256401264489476,99.99988719861383)
(27.49339284143487,99.99988719861383)
(27.730384418380257,99.9999194275813)
(27.96737599532565,99.99992748482317)
(28.20436757227104,99.99992748482317)
(28.44135914921643,99.99992748482317)
(28.678350726161824,99.99992748482317)
(28.915342303107217,99.99992748482317)
(29.15233388005261,99.99992748482317)
(29.389325456997998,99.99993554206505)
(29.62631703394339,99.99994359930692)
(29.86330861088878,99.99994359930692)
(30.100300187834172,99.99994359930692)
(30.337291764779565,99.99994359930692)
(30.574283341724957,99.99994359930692)
(30.81127491867035,99.99995971379066)
(31.04826649561574,99.99995971379066)
(31.285258072561128,99.99995971379066)
(31.52224964950652,99.99995971379066)
(31.759241226451913,99.99995971379066)
(31.996232803397305,99.99995971379066)
(32.23322438034269,99.99996777103253)
(32.47021595728809,99.99996777103253)
(32.707207534233476,99.99996777103253)
(32.944199111178875,99.99996777103253)
(33.18119068812426,99.99996777103253)
(33.41818226506965,99.99996777103253)
(33.655173842015046,99.99996777103253)
(33.89216541896043,99.99996777103253)
(34.12915699590583,99.99996777103253)
(34.366148572851216,99.99996777103253)
(34.603140149796616,99.99996777103253)
(34.840131726742,99.99996777103253)
(35.077123303687394,99.99996777103253)
(35.314114880632786,99.99996777103253)
(35.55110645757817,99.99996777103253)
(35.78809803452357,99.99996777103253)
(36.02508961146896,99.99996777103253)
(36.262081188414356,99.99996777103253)
(36.49907276535974,99.99996777103253)
(36.736064342305134,99.99996777103253)
(36.97305591925053,99.99996777103253)
(37.21004749619591,99.99996777103253)
(37.44703907314131,99.99996777103253)
(37.6840306500867,99.99996777103253)
(37.9210222270321,99.99996777103253)
(38.15801380397748,99.99996777103253)
(38.395005380922875,99.99996777103253)
(38.63199695786827,99.99996777103253)
(38.86898853481365,99.99998388551626)
(39.10598011175905,99.99998388551626)
(39.34297168870444,99.99998388551626)
(39.57996326564984,99.99998388551626)
(39.81695484259522,99.99998388551626)
(40.053946419540615,99.99998388551626)
(40.29093799648601,99.99998388551626)
(40.52792957343139,99.99998388551626)
(40.76492115037679,99.99998388551626)
(41.00191272732218,99.99998388551626)
(41.23890430426758,99.99998388551626)
(41.47589588121296,99.99998388551626)
(41.712887458158356,99.99998388551626)
(41.94987903510375,99.99998388551626)
(42.186870612049134,99.99999194275813)
(42.42386218899453,99.99999194275813)
(42.66085376593992,99.99999194275813)
(42.89784534288532,99.99999194275813)
(43.134836919830704,99.99999194275813)
(43.3718284967761,99.99999194275813)
(43.60882007372149,99.99999194275813)
(43.845811650666874,99.99999194275813)
(44.082803227612274,99.99999194275813)
(44.31979480455766,99.99999194275813)
(44.55678638150306,99.99999194275813)
(44.793777958448445,99.99999194275813)
(45.03076953539384,99.99999194275813)
(45.26776111233923,99.99999194275813)
(45.504752689284615,99.99999194275813)
(45.741744266230015,99.99999194275813)
(45.9787358431754,99.99999194275813)
(46.2157274201208,99.99999194275813)
(46.452718997066185,99.99999194275813)
(46.68971057401157,99.99999194275813)
(46.92670215095697,99.99999194275813)
(47.163693727902356,99.99999194275813)
};
\addplot[dashed, magenta, thick, mark = none] coordinates{
(0.0, 0.9132228167000467)
(0.075, 0.9406433190096234)
(0.15, 0.9704456021767475)
(0.225, 1.001518835633403)
(0.3, 1.0346836329523585)
(0.375, 1.070040068959561)
(0.45, 1.1073879940031162)
(0.525, 1.1485487699152657)
(0.6, 1.191460855281494)
(0.675, 1.2365745868185642)
(0.75, 1.2849407501989236)
(0.8250000000000001, 1.3361090087058094)
(0.9, 1.3918807092062735)
(0.975, 1.448933367478864)
(1.05, 1.5597362147677818)
(1.125, 1.8411466253317603)
(1.2, 1.9301131455989644)
(1.2750000000000001, 2.025114177870794)
(1.35, 2.1243383677976024)
(1.425, 2.2247634556357787)
(1.5, 2.328551057625787)
(1.575, 2.4406148477216414)
(1.6500000000000001, 2.5584229328268746)
(1.725, 2.68126478167726)
(1.8, 2.8120225492600817)
(1.875, 2.948104297583303)
(1.95, 3.091011149036134)
(2.025, 4.063898576965998)
(2.1, 4.281621368297076)
(2.1750000000000003, 4.439709570846122)
(2.25, 4.583757275314753)
(2.325, 4.728115211743821)
(2.4, 4.873443873984578)
(2.475, 5.022695469402472)
(2.5500000000000003, 5.176040125201613)
(2.625, 5.334608686915207)
(2.7, 5.497020121945178)
(2.775, 5.665466068979776)
(2.85, 5.8389958171725)
(2.9250000000000003, 6.014527061884171)
(3.0, 6.197413806302973)
(3.075, 6.392709829139247)
(3.15, 6.585894273148033)
(3.225, 6.779138762052386)
(3.3000000000000003, 6.975815817486734)
(3.375, 7.176936195193146)
(3.45, 7.380508406135268)
(3.525, 7.588483909419072)
(3.6, 7.805265997386246)
(3.6750000000000003, 8.028773113657081)
(3.75, 8.259815864321753)
(3.825, 8.503648177742498)
(3.9, 8.757077666971595)
(3.975, 9.041570382174752)
(4.05, 9.430371088462843)
(4.125, 9.651416364015375)
(4.2, 9.874753353082099)
(4.275, 10.102503641973103)
(4.3500000000000005, 10.336188368042786)
(4.425, 10.57376600484182)
(4.5, 10.814916312927176)
(4.575, 11.060279771184915)
(4.65, 11.312488347537455)
(4.7250000000000005, 11.564336654516582)
(4.8, 11.821649046992436)
(4.875, 12.086897373165916)
(4.95, 12.352355856473887)
(5.025, 12.620576404978001)
(5.1000000000000005, 12.903628042687517)
(5.175, 13.181305662243659)
(5.25, 13.462355803434228)
(5.325, 13.7460579275124)
(5.4, 14.03535423436103)
(5.4750000000000005, 14.326702075141585)
(5.55, 14.623574046314431)
(5.625, 14.926780753969743)
(5.7, 15.233800312493651)
(5.775, 15.547845123799064)
(5.8500000000000005, 15.86954565928945)
(5.925, 16.19391819263263)
(6.0, 16.524595440010494)
(6.075, 16.871424764296265)
(6.15, 17.17076858367001)
(6.2250000000000005, 17.47143339074626)
(6.3, 17.771537778797207)
(6.375, 18.075214838134475)
(6.45, 18.380553139582464)
(6.525, 18.689324007560455)
(6.6000000000000005, 18.999175683658674)
(6.675, 19.309587778782195)
(6.75, 19.623962837013234)
(6.825, 19.94306142702899)
(6.9, 20.2599583708739)
(6.9750000000000005, 20.58032791117919)
(7.05, 20.910855046318133)
(7.125, 21.23875021353466)
(7.2, 21.56734590453282)
(7.275, 21.899504259334705)
(7.3500000000000005, 22.233594058277372)
(7.425, 22.573268032507908)
(7.5, 22.913732597863422)
(7.575, 23.255348023717335)
(7.65, 23.602877871784735)
(7.7250000000000005, 23.948396215850593)
(7.8, 24.29987901954291)
(7.875, 24.647839189361886)
(7.95, 24.99294722664136)
(8.025, 25.361192563679865)
(8.1, 25.69646324556871)
(8.175, 26.03181398731832)
(8.25, 26.36762507326728)
(8.325, 26.705167453705137)
(8.4, 27.046902969350185)
(8.475, 27.388708537373397)
(8.55, 27.734867360325318)
(8.625, 28.079044701723475)
(8.700000000000001, 28.42402264172922)
(8.775, 28.772463170712744)
(8.85, 29.12335553293197)
(8.925, 29.475739010057822)
(9.0, 29.830674395245328)
(9.075000000000001, 30.189622780953318)
(9.15, 30.545138600131317)
(9.225, 30.905578100745927)
(9.3, 31.26446644155835)
(9.375, 31.62747786519981)
(9.450000000000001, 31.988117515466314)
(9.525, 32.34969786909672)
(9.6, 32.71727270480138)
(9.675, 33.081324906632695)
(9.75, 33.447478679808896)
(9.825000000000001, 33.81425291690597)
(9.9, 34.17380175156965)
(9.975, 34.53548218002601)
(10.05, 34.90890138556599)
(10.125, 35.26690906791007)
(10.200000000000001, 35.62822922699303)
(10.275, 35.98926917656332)
(10.35, 36.3522405702744)
(10.425, 36.71332054977507)
(10.5, 37.07424040955422)
(10.575000000000001, 37.43762211005169)
(10.65, 37.79999305480708)
(10.725, 38.16323465054822)
(10.8, 38.531850264442724)
(10.875, 38.897753850554054)
(10.950000000000001, 39.26676976375236)
(11.025, 39.63466483890004)
(11.1, 40.005061784696416)
(11.175, 40.376049171965875)
(11.25, 40.74973857953592)
(11.325000000000001, 41.11704321321052)
(11.4, 41.49265405743875)
(11.475, 41.86533270926672)
(11.55, 42.235419423102655)
(11.625, 42.60588642127719)
(11.700000000000001, 42.97633340448653)
(11.775, 43.34552945237154)
(11.85, 43.71889862049855)
(11.925, 44.089966067628765)
(12.0, 44.46026293859919)
(12.075000000000001, 44.84107767377668)
(12.15, 45.21267551748443)
(12.225, 45.58376297957983)
(12.3, 45.95780264904069)
(12.375, 46.32883006624053)
(12.450000000000001, 46.70458101522508)
(12.525, 47.07748983915273)
(12.6, 47.45247021197749)
(12.675, 47.83039278468511)
(12.75, 48.208685634248724)
(12.825000000000001, 48.59138177615403)
(12.9, 48.97563908534411)
(12.975, 49.362458310078445)
(13.05, 49.75161928573995)
(13.125, 50.144963389126055)
(13.200000000000001, 50.53743684152641)
(13.275, 50.929149725249566)
(13.35, 51.32481556459765)
(13.425, 51.72268305011657)
(13.5, 52.12825629723344)
(13.575000000000001, 52.53857309110022)
(13.65, 52.95027091756507)
(13.725, 53.37287690005817)
(13.8, 53.794241954709534)
(13.875, 54.22271232200316)
(13.950000000000001, 54.6604796406273)
(14.025, 55.169440190430386)
(14.1, 55.79581853351752)
(14.175, 56.45075823193001)
(14.25, 57.12428182552094)
(14.325000000000001, 57.81962173116839)
(14.4, 58.54351298465863)
(14.475, 59.30812468482684)
(14.55, 60.105390800701684)
(14.625, 60.933720142550584)
(14.700000000000001, 61.80875440566912)
(14.775, 66.05816168749374)
(14.85, 76.73958819008972)
(14.925, 88.14040257900832)
};
\addplot[dashed, black, thick, mark = none] coordinates{
(0.0, 0.49103249123069936)
(0.075, 0.5009267842459972)
(0.15, 0.5112481110803593)
(0.225, 0.5222301317479904)
(0.3, 0.5338245027976758)
(0.375, 0.545821735940818)
(0.45, 0.5576981104559231)
(0.525, 0.571830512694386)
(0.6, 0.5865510935892958)
(0.675, 0.6014892200146722)
(0.75, 0.6173942154643449)
(0.8250000000000001, 0.6347253427248545)
(0.9, 0.6530394534933985)
(0.975, 0.6725863222679201)
(1.05, 0.7051698083867025)
(1.125, 0.7932193475326107)
(1.2, 0.8201385926173911)
(1.2750000000000001, 0.8478474474053465)
(1.35, 0.8786099968617043)
(1.425, 0.9099446104907707)
(1.5, 0.9433418780383356)
(1.575, 0.979156318146641)
(1.6500000000000001, 1.0165741493869043)
(1.725, 1.0563849814623008)
(1.8, 1.0989352757732032)
(1.875, 1.1427586142994288)
(1.95, 1.1884431756974247)
(2.025, 1.6587524408407088)
(2.1, 1.7172480168106292)
(2.1750000000000003, 1.7643345382938551)
(2.25, 1.8085929678810138)
(2.325, 1.8531495154173308)
(2.4, 1.89926916787626)
(2.475, 1.9470647266439693)
(2.5500000000000003, 1.9962461310131698)
(2.625, 2.0469986975468517)
(2.7, 2.0998461469665086)
(2.775, 2.1557634055383064)
(2.85, 2.2138641766566396)
(2.9250000000000003, 2.2761305418213156)
(3.0, 2.3401856146809394)
(3.075, 2.4116372355764293)
(3.15, 2.484410244138457)
(3.225, 2.5608251260253345)
(3.3000000000000003, 2.641671490940236)
(3.375, 2.726602877482789)
(3.45, 2.820268314211484)
(3.525, 2.921902363148754)
(3.6, 3.0298532897114256)
(3.6750000000000003, 3.1456600270965045)
(3.75, 3.268130103507358)
(3.825, 3.3921874565664303)
(3.9, 3.5224408286228686)
(3.975, 3.6661981380519766)
(4.05, 3.832507667472794)
(4.125, 3.9506510049999215)
(4.2, 4.079260699715056)
(4.275, 4.216604444616332)
(4.3500000000000005, 4.360917703734411)
(4.425, 4.51640635732498)
(4.5, 4.682490283973461)
(4.575, 4.859338685759107)
(4.65, 5.047459168919673)
(4.7250000000000005, 5.250090744686551)
(4.8, 5.464493950824235)
(4.875, 5.69445569101122)
(4.95, 5.93638243537387)
(5.025, 6.193875771027689)
(5.1000000000000005, 6.467016270391368)
(5.175, 6.7540313402536984)
(5.25, 7.058466167037099)
(5.325, 7.379418339652226)
(5.4, 7.715993504251604)
(5.4750000000000005, 8.070705520298407)
(5.55, 8.439985029644607)
(5.625, 8.828690549137292)
(5.7, 9.23634670150618)
(5.775, 9.660939176283993)
(5.8500000000000005, 10.104836802580252)
(5.925, 10.566420074779263)
(6.0, 11.049089148949799)
(6.075, 11.557493053650354)
(6.15, 12.077733046656668)
(6.2250000000000005, 12.618591521606099)
(6.3, 13.183444462841814)
(6.375, 13.768811141876347)
(6.45, 14.378768523095479)
(6.525, 15.00866757794072)
(6.6000000000000005, 15.65759783808086)
(6.675, 16.331368574903546)
(6.75, 17.02990727323195)
(6.825, 17.744753829103484)
(6.9, 18.485568875519238)
(6.9750000000000005, 19.239162707539442)
(7.05, 20.0213275192276)
(7.125, 20.816778722757963)
(7.2, 21.626160897480055)
(7.275, 22.45660470244807)
(7.3500000000000005, 23.298900710205583)
(7.425, 24.157778521729778)
(7.5, 25.024012595080492)
(7.575, 25.902856251956397)
(7.65, 26.798966578157863)
(7.7250000000000005, 27.7032550048565)
(7.8, 28.61444848783699)
(7.875, 29.528792352388304)
(7.95, 30.443385991437573)
(8.025, 31.363756672907)
(8.1, 32.27968781410654)
(8.175, 33.192597489605156)
(8.25, 34.09665225628958)
(8.325, 34.99908751735832)
(8.4, 35.895777964974364)
(8.475, 36.78031003460988)
(8.55, 37.652466180734415)
(8.625, 38.506751364393196)
(8.700000000000001, 39.35401869038396)
(8.775, 40.18371317185815)
(8.85, 40.98835768836119)
(8.925, 41.77932100817044)
(9.0, 42.55234085033713)
(9.075000000000001, 43.30823905353191)
(9.15, 44.037628930977235)
(9.225, 44.74938150597102)
(9.3, 45.43680926776189)
(9.375, 46.10350574622347)
(9.450000000000001, 46.74880219028063)
(9.525, 47.37265831372402)
(9.6, 47.97608127178729)
(9.675, 48.557282356775474)
(9.75, 49.120427162734934)
(9.825000000000001, 49.661019748702685)
(9.9, 50.17802878771948)
(9.975, 50.67495917999838)
(10.05, 51.15388163669977)
(10.125, 51.61213726800683)
(10.200000000000001, 52.053061772053375)
(10.275, 52.474568323195314)
(10.35, 52.87789773668047)
(10.425, 53.2631708711369)
(10.5, 53.63648705865954)
(10.575000000000001, 53.992955553433816)
(10.65, 54.33583148117486)
(10.725, 54.66373705352305)
(10.8, 54.98632484623761)
(10.875, 55.29557790365875)
(10.950000000000001, 55.593711967300486)
(11.025, 55.88108155580505)
(11.1, 56.16324616606217)
(11.175, 56.43509750672679)
(11.25, 56.69876268965237)
(11.325000000000001, 56.9555469880217)
(11.4, 57.2033877479163)
(11.475, 57.44773972208156)
(11.55, 57.68600042139374)
(11.625, 57.921610288131)
(11.700000000000001, 58.15054875860061)
(11.775, 58.37749709032853)
(11.85, 58.598563635491985)
(11.925, 58.81899365854779)
(12.0, 59.03321960536435)
(12.075000000000001, 59.24915368745717)
(12.15, 59.45943158575786)
(12.225, 59.669685312332945)
(12.3, 59.87925417334914)
(12.375, 60.08813816880647)
(12.450000000000001, 60.29920567681033)
(12.525, 60.50694554392224)
(12.6, 60.71619211526368)
(12.675, 60.92540645763764)
(12.75, 61.135329837296084)
(12.825000000000001, 61.3439560010136)
(12.9, 61.55129300603206)
(12.975, 61.76481797280601)
(13.05, 61.982822766059186)
(13.125, 62.197669120499675)
(13.200000000000001, 62.41487624680783)
(13.275, 62.63417825600194)
(13.35, 62.85669510470184)
(13.425, 63.080960374887354)
(13.5, 63.30817459559695)
(13.575000000000001, 63.53980418485086)
(13.65, 63.77652595096605)
(13.725, 64.02043477682851)
(13.8, 64.26715558010329)
(13.875, 64.52191751076347)
(13.950000000000001, 64.78333472320756)
(14.025, 65.10578554281035)
(14.1, 65.52153116601585)
(14.175, 65.95923277331474)
(14.25, 66.41214645326255)
(14.325000000000001, 66.89187463415087)
(14.4, 67.39989984848357)
(14.475, 67.93586757761844)
(14.55, 68.49694167241752)
(14.625, 69.08293681631785)
(14.700000000000001, 69.70173299186743)
(14.775, 73.03841410919738)
(14.85, 81.51443918172264)
(14.925, 90.53297446378048)
};
