# Supplementary material for: CausalSim: A Causal Framework for Unbiased Trace-Driven Simulation
Source: arXiv:2201.01811 source file (2023-05-05)
Supplement: Supplementary file 4 [file new_bola_basic_v1_puffer_ttp_cl.tex]

\addplot[solid, green!70!black, thick, mark = none] coordinates{
(0.0, 0.39277254018318597)
(0.08024055532478766, 0.4005780028112952)
(0.16048111064957532, 0.4122945004371059)
(0.24072166597436298, 0.42732416783803967)
(0.32096222129915064, 0.4484404353521692)
(0.40120277662393833, 0.4918520934582916)
(0.48144333194872596, 0.5761012677399898)
(0.5616838872735136, 0.7140586678499969)
(0.6419244425983013, 0.9512616949080485)
(0.722164997923089, 1.3434778882868903)
(0.8024055532478767, 1.7827925753110891)
(0.8826461085726642, 2.1932353542949308)
(0.9628866638974519, 2.5225843587829058)
(1.0431272192222396, 2.7868823055808725)
(1.1233677745470272, 3.014087697528027)
(1.203608329871815, 3.222850608095361)
(1.2838488851966026, 3.4291556283032056)
(1.3640894405213901, 3.6367892378945577)
(1.444329995846178, 3.8412923587510193)
(1.5245705511709655, 4.046850047430641)
(1.6048111064957533, 4.253437392882481)
(1.685051661820541, 4.459003385245749)
(1.7652922171453285, 4.66531670913724)
(1.8455327724701163, 4.87455292967245)
(1.9257733277949038, 5.0844783559503535)
(2.0060138831196914, 5.299195007692532)
(2.086254438444479, 5.510789474383468)
(2.166494993769267, 5.712419520698094)
(2.2467355490940544, 5.905305788132508)
(2.326976104418842, 6.0992632307573755)
(2.40721665974363, 6.291676188223915)
(2.4874572150684173, 6.481473485341674)
(2.567697770393205, 6.675007440100547)
(2.647938325717993, 6.867470219668968)
(2.7281788810427803, 7.063403939001804)
(2.808419436367568, 7.260134811964744)
(2.888659991692356, 7.458318829565896)
(2.9689005470171437, 7.658055636009024)
(3.049141102341931, 7.861271685900212)
(3.129381657666719, 8.065384533625268)
(3.2096222129915066, 8.273408416348026)
(3.289862768316294, 8.482544992679472)
(3.370103323641082, 8.693250965220187)
(3.4503438789658696, 8.906821708619091)
(3.530584434290657, 9.122634446602664)
(3.6108249896154447, 9.342607330093347)
(3.6910655449402325, 9.564805600801405)
(3.77130610026502, 9.790067930775178)
(3.8515466555898077, 10.01836110528008)
(3.9317872109145955, 10.246554635581218)
(4.012027766239383, 10.476998464150673)
(4.092268321564171, 10.708513467910581)
(4.172508876888958, 10.945716494968632)
(4.252749432213746, 11.18611644023075)
(4.332989987538534, 11.42702291019533)
(4.413230542863321, 11.674265090782512)
(4.493471098188109, 11.922985327058848)
(4.5737116535128965, 12.173117189555162)
(4.653952208837684, 12.428978593767853)
(4.734192764162472, 12.685620544243356)
(4.81443331948726, 12.94654719548067)
(4.894673874812048, 13.211924621152738)
(4.974914430136835, 13.479353056685595)
(5.0551549854616225, 13.749372241516292)
(5.13539554078641, 14.021924049859303)
(5.215636096111198, 14.298469930036484)
(5.295876651435986, 14.57818781736679)
(5.376117206760774, 14.861061104482925)
(5.456357762085561, 15.147114702435834)
(5.536598317410348, 15.434447067670371)
(5.616838872735136, 15.723871961183933)
(5.697079428059924, 16.01336328416667)
(5.777319983384712, 16.31006220455494)
(5.8575605387094996, 16.60839695062165)
(5.937801094034287, 16.909347357037138)
(6.018041649359074, 17.21491461156032)
(6.098282204683862, 17.524359686346617)
(6.17852276000865, 17.837657670345088)
(6.258763315333438, 18.152209510574245)
(6.3390038706582255, 18.468563250154784)
(6.419244425983013, 18.79182565452956)
(6.4994849813078, 19.116549507226196)
(6.579725536632588, 19.44511796545136)
(6.659966091957376, 19.774126518909814)
(6.740206647282164, 20.10846603726959)
(6.820447202606951, 20.44722311532953)
(6.900687757931739, 20.78798138114838)
(6.980928313256527, 21.132982829310805)
(7.061168868581314, 21.48000207259944)
(7.141409423906102, 21.827270426397476)
(7.2216499792308895, 22.17342608658683)
(7.301890534555677, 22.524879496942916)
(7.382131089880465, 22.878309184006973)
(7.462371645205253, 23.234396049838043)
(7.54261220053004, 23.592949109712254)
(7.622852755854828, 23.954151044669832)
(7.703093311179615, 24.317387382120906)
(7.783333866504403, 24.68052407536822)
(7.863574421829191, 25.047098493645358)
(7.943814977153979, 25.417766627960432)
(8.024055532478766, 25.787986363358566)
(8.104296087803554, 26.15745876722848)
(8.184536643128341, 26.53384813957629)
(8.26477719845313, 26.9107523403102)
(8.345017753777917, 27.295395574203045)
(8.425258309102704, 27.676393490974892)
(8.505498864427492, 28.061659501141257)
(8.58573941975228, 28.448760625393593)
(8.665979975077068, 28.838959023646233)
(8.746220530401855, 29.229971182896268)
(8.826461085726642, 29.61958001960998)
(8.90670164105143, 30.01421258493008)
(8.986942196376217, 30.40736709456102)
(9.067182751701006, 30.805030504412244)
(9.147423307025793, 31.206654771363052)
(9.227663862350582, 31.605214979048146)
(9.307904417675369, 32.00856641219752)
(9.388144973000156, 32.41071381121808)
(9.468385528324944, 32.81570107004589)
(9.548626083649731, 33.223669351302945)
(9.62886663897452, 33.62648934869891)
(9.709107194299307, 34.035578627248306)
(9.789347749624095, 34.44810563082753)
(9.869588304948882, 34.85644757784869)
(9.94982886027367, 35.26930672877379)
(10.030069415598458, 35.67735804686732)
(10.110309970923245, 36.09146275033945)
(10.190550526248034, 36.507585248937794)
(10.27079108157282, 36.92524392901081)
(10.35103163689761, 37.339821942450826)
(10.431272192222396, 37.754748710604005)
(10.511512747547183, 38.17048923975459)
(10.591753302871972, 38.58730094409562)
(10.671993858196759, 39.00750055136459)
(10.752234413521547, 39.42954357640319)
(10.832474968846334, 39.84652135441716)
(10.912715524171121, 40.26826544684447)
(10.99295607949591, 40.687767544687105)
(11.073196634820697, 41.10914627503395)
(11.153437190145485, 41.533356561504384)
(11.233677745470272, 41.957575151658475)
(11.313918300795061, 42.38097998081517)
(11.394158856119848, 42.801818971724956)
(11.474399411444635, 43.22372083414156)
(11.554639966769424, 43.64904381422069)
(11.63488052209421, 44.07145220133975)
(11.715121077418999, 44.497439476110635)
(11.795361632743786, 44.92180753257037)
(11.875602188068575, 45.35130726552391)
(11.955842743393362, 45.775492640943405)
(12.036083298718149, 46.204278257103304)
(12.116323854042937, 46.63343753902731)
(12.196564409367724, 47.062837627777085)
(12.276804964692513, 47.4958913373315)
(12.3570455200173, 47.92681100018866)
(12.437286075342088, 48.36242224430633)
(12.517526630666875, 48.79906314519622)
(12.597767185991662, 49.24063643417238)
(12.678007741316451, 49.68490011665015)
(12.758248296641238, 50.12991113065613)
(12.838488851966027, 50.5760514456381)
(12.918729407290813, 51.02757254762329)
(12.9989699626156, 51.47859542858965)
(13.079210517940389, 51.93279031670913)
(13.159451073265176, 52.39410976539769)
(13.239691628589965, 52.85914926436006)
(13.319932183914752, 53.330524473945026)
(13.40017273923954, 53.804739543337256)
(13.480413294564327, 54.289716186735895)
(13.560653849889114, 54.78402617055368)
(13.640894405213903, 55.28784387214719)
(13.72113496053869, 55.808285548401834)
(13.801375515863478, 56.34059318858795)
(13.881616071188265, 56.889142833987435)
(13.961856626513054, 57.45838525903507)
(14.04209718183784, 58.047515006417086)
(14.122337737162628, 58.66341582987678)
(14.202578292487416, 59.31070457752187)
(14.282818847812203, 59.99936227709591)
(14.363059403136992, 60.76134150327231)
(14.443299958461779, 61.627307759759155)
(14.523540513786566, 62.68472374640949)
(14.603781069111355, 64.15407717510011)
(14.684021624436141, 66.45717026404385)
(14.76426217976093, 70.60182109746798)
(14.844502735085717, 88.56003164699912)
(14.924743290410506, 94.7293364493183)
(15.004983845735293, 96.44859754104677)
(15.08522440106008, 97.54445958298237)
(15.165464956384868, 98.23710305070693)
(15.245705511709655, 98.7141745872737)
(15.325946067034444, 99.12014998445551)
(15.40618662235923, 99.44119530529656)
(15.48642717768402, 99.67575776095488)
(15.566667733008806, 99.83043047624615)
(15.646908288333593, 99.92272591998172)
(15.727148843658382, 99.97187542348786)
(15.807389398983169, 99.99397982935598)
(15.887629954307958, 99.99972597843964)
(15.967870509632744, 99.99998339263271)
};
\addplot[solid, blue, thick, mark = none] coordinates{
(0.0, 0.38892505836062075)
(0.075, 0.38892505836062075)
(0.15, 0.38892505836062075)
(0.225, 0.38892505836062075)
(0.3, 0.38892505836062075)
(0.375, 0.38892505836062075)
(0.45, 0.38892505836062075)
(0.525, 0.38892505836062075)
(0.6, 0.38892505836062075)
(0.675, 0.38892505836062075)
(0.75, 0.38892505836062075)
(0.8250000000000001, 0.38892505836062075)
(0.9, 0.38892505836062075)
(0.975, 0.38892505836062075)
(1.05, 0.38892505836062075)
(1.125, 0.38892505836062075)
(1.2, 0.38892505836062075)
(1.2750000000000001, 0.38892505836062075)
(1.35, 0.38892505836062075)
(1.425, 0.38892505836062075)
(1.5, 0.38892505836062075)
(1.575, 0.38892505836062075)
(1.6500000000000001, 0.38892505836062075)
(1.725, 0.38892505836062075)
(1.8, 0.38892505836062075)
(1.875, 0.38892505836062075)
(1.95, 0.38892505836062075)
(2.025, 4.752248835083096)
(2.1, 4.894430566929871)
(2.1750000000000003, 5.042812363225835)
(2.25, 5.194779528244179)
(2.325, 5.3505157028219035)
(2.4, 5.51260060347877)
(2.475, 5.6819524343997765)
(2.5500000000000003, 5.86034639034259)
(2.625, 6.041180145976976)
(2.7, 6.230714979364453)
(2.775, 6.4232055557474546)
(2.85, 6.6232953648615505)
(2.9250000000000003, 6.829270425561405)
(3.0, 7.041646681150973)
(3.075, 7.2655136062556815)
(3.15, 7.495361975765531)
(3.225, 7.73108685205938)
(3.3000000000000003, 7.973868783375082)
(3.375, 8.224354885043022)
(3.45, 8.482824990719578)
(3.525, 8.748570771462038)
(3.6, 9.02103255995764)
(3.6750000000000003, 9.301198518805478)
(3.75, 9.59415812263098)
(3.825, 9.898669609583953)
(3.9, 10.211270038166688)
(3.975, 10.509144220582378)
(4.05, 10.747938522294653)
(4.125, 10.988726638808643)
(4.2, 11.235260090080203)
(4.275, 11.485929832585143)
(4.3500000000000005, 11.738873223548177)
(4.425, 11.996582531471448)
(4.5, 12.259232652390196)
(4.575, 12.527995389740513)
(4.65, 12.79975759409516)
(4.7250000000000005, 13.071694694485048)
(4.8, 13.35193061174698)
(4.875, 13.635577001696053)
(4.95, 13.92617550904584)
(5.025, 14.220884073223722)
(5.1000000000000005, 14.522299900352984)
(5.175, 14.827204903385244)
(5.25, 15.131200447034265)
(5.325, 15.444439246145619)
(5.4, 15.762505175829542)
(5.4750000000000005, 16.08099085599804)
(5.55, 16.406402419161957)
(5.625, 16.73672856091607)
(5.7, 17.06791169324285)
(5.775, 17.405530999666386)
(5.8500000000000005, 17.744400812741876)
(5.925, 18.07613486757965)
(6.0, 18.386461647704294)
(6.075, 18.694750889018408)
(6.15, 19.00854061064076)
(6.2250000000000005, 19.32405305821021)
(6.3, 19.64254748318047)
(6.375, 19.96460978726958)
(6.45, 20.285342881490884)
(6.525, 20.609871219676855)
(6.6000000000000005, 20.93903430279663)
(6.675, 21.268538433185125)
(6.75, 21.598497293265233)
(6.825, 21.935224629909058)
(6.9, 22.271829539328216)
(6.9750000000000005, 22.610288346720896)
(7.05, 22.955506885875526)
(7.125, 23.299789731241635)
(7.2, 23.644457347885268)
(7.275, 23.99561360743623)
(7.3500000000000005, 24.35163197676681)
(7.425, 24.707947669357296)
(7.5, 25.064700602035877)
(7.575, 25.42370969356903)
(7.65, 25.78495745435323)
(7.7250000000000005, 26.146887309674856)
(7.8, 26.507487955128674)
(7.875, 26.863147787587017)
(7.95, 27.212852410045503)
(8.025, 27.5599598263807)
(8.1, 27.908343983773147)
(8.175, 28.25803986142987)
(8.25, 28.609991897941168)
(8.325, 28.961121923086846)
(8.4, 29.314088356602525)
(8.475, 29.66963450663796)
(8.55, 30.027541753149112)
(8.625, 30.387469048867267)
(8.700000000000001, 30.7494426281977)
(8.775, 31.1143632057219)
(8.85, 31.479957132981763)
(8.925, 31.847011442135866)
(9.0, 32.21342738076135)
(9.075000000000001, 32.58139989410045)
(9.15, 32.94982713713117)
(9.225, 33.317581030426226)
(9.3, 33.68989096543923)
(9.375, 34.0626468853421)
(9.450000000000001, 34.43591874854891)
(9.525, 34.80824617316544)
(9.6, 35.180101378486825)
(9.675, 35.55298847041612)
(9.75, 35.92435396683884)
(9.825000000000001, 36.296357833790175)
(9.9, 36.662677579596284)
(9.975, 37.02932962786933)
(10.05, 37.39372551728782)
(10.125, 37.76106840490006)
(10.200000000000001, 38.128122714054165)
(10.275, 38.496462509067264)
(10.35, 38.86258986923461)
(10.425, 39.22977535041514)
(10.5, 39.596444888291714)
(10.575000000000001, 39.96635874762196)
(10.65, 40.334908417877344)
(10.725, 40.701744106987405)
(10.8, 41.07399282838807)
(10.875, 41.44207902415008)
(10.950000000000001, 41.81389925026442)
(11.025, 42.185019892237804)
(11.1, 42.556289195841146)
(11.175, 42.9269813425282)
(11.25, 43.29820692212273)
(11.325000000000001, 43.66927509528555)
(11.4, 44.03919769941756)
(11.475, 44.408822980289656)
(11.55, 44.777932317857804)
(11.625, 45.14545010150528)
(11.700000000000001, 45.5152327888091)
(11.775, 45.881141528932396)
(11.85, 46.245519928747356)
(11.925, 46.60865656671213)
(12.0, 46.97367333705571)
(12.075000000000001, 47.33881253462395)
(12.15, 47.70496612919658)
(12.225, 48.06603024914378)
(12.3, 48.4329184070644)
(12.375, 48.796929525205364)
(12.450000000000001, 49.1593840686327)
(12.525, 49.52635967457095)
(12.6, 49.89185740901143)
(12.675, 50.259051634993725)
(12.75, 50.62614092335488)
(12.825000000000001, 50.99454193198031)
(12.9, 51.362750554966986)
(12.975, 51.73047821385674)
(13.05, 52.09960504102842)
(13.125, 52.474599630182325)
(13.200000000000001, 52.84731182607638)
(13.275, 53.22134448703649)
(13.35, 53.60017804416387)
(13.425, 53.97734134415474)
(13.5, 54.354382216920925)
(13.575000000000001, 54.734877286383075)
(13.65, 55.12071542972174)
(13.725, 55.513147153588896)
(13.8, 55.90715294177318)
(13.875, 56.30637063180755)
(13.950000000000001, 56.71022306677575)
(14.025, 57.11959347165569)
(14.1, 57.5379010639363)
(14.175, 57.95937427445473)
(14.25, 58.393798536382526)
(14.325000000000001, 58.840290624741755)
(14.4, 59.30088807834293)
(14.475, 59.76989803123905)
(14.55, 60.25916094501574)
(14.625, 60.76982238870382)
(14.700000000000001, 61.299503776224014)
(14.775, 61.857072336562936)
(14.85, 62.44300903381747)
(14.925, 63.06427473019007)
};
\addplot[solid, red, thick, mark = none] coordinates{
(0.0024455589681865756,0.39337870908941147)
(0.24700145578684413,0.44266937521755656)
(0.4915573526055017,0.5835164572366935)
(0.7361132494241593,1.0534219148161632)
(0.9806691462428168,2.0569386909143086)
(1.2252250430614744,3.320136565702731)
(1.469780939880132,4.116401701657282)
(1.7143368366987897,4.897595651792665)
(1.958892733517447,5.715035181046875)
(2.203448630336105,6.6129623158907265)
(2.448004527154762,7.371055418120365)
(2.6925604239734198,8.124050058590791)
(2.9371163207920774,8.88528195323897)
(3.181672217610735,9.662622994162179)
(3.4262281144293922,10.475146742697408)
(3.67078401124805,11.334362104379297)
(3.9153399080667075,12.249195539128285)
(4.159895804885365,13.211368274348393)
(4.404451701704023,14.12575331018045)
(4.6490075985226795,15.0468975445011)
(4.893563495341338,15.996141444282946)
(5.138119392159995,16.971907309633067)
(5.382675288978653,17.986982813367735)
(5.62723118579731,19.02976770943219)
(5.871787082615969,20.106423331092447)
(6.116342979434625,21.184457364238092)
(6.360898876253284,22.242471216111007)
(6.605454773071941,23.31114699778657)
(6.850010669890599,24.39074212345784)
(7.094566566709256,25.491586375581587)
(7.3391224635279135,26.609743808109176)
(7.583678360346571,27.750586904360162)
(7.828234257165228,28.906409845910204)
(8.072790153983886,30.05340597174356)
(8.317346050802545,31.18939971674474)
(8.561901947621202,32.33424518851355)
(8.806457844439858,33.48586646613824)
(9.051013741258515,34.65368823055809)
(9.295569638077174,35.8306357433059)
(9.540125534895832,37.005000810439526)
(9.784681431714489,38.18424013987389)
(10.029237328533146,39.35114019540893)
(10.273793225351804,40.503375945623496)
(10.518349122170463,41.66111703809597)
(10.76290501898912,42.82002894996267)
(11.007460915807776,43.98191358057496)
(11.252016812626435,45.14464518691924)
(11.496572709445093,46.31136256141404)
(11.74112860626375,47.46481064944106)
(11.985684503082407,48.609714246995395)
(12.230240399901064,49.74821570445795)
(12.474796296719722,50.89338501988898)
(12.71935219353838,52.049988507701826)
(12.963908090357037,53.22035119931764)
(13.208463987175694,54.40725482875811)
(13.453019883994353,55.61774091975585)
(13.697575780813011,56.85925787654216)
(13.942131677631668,58.15547950119441)
(14.186687574450325,59.522838783649846)
(14.431243471268981,61.057052285306604)
(14.675799368087642,63.64997714826261)
(14.920355264906298,96.0724074571065)
(15.164911161724955,99.96566426811997)
(15.409467058543612,99.9966204007557)
(15.65402295536227,99.99866310693285)
(15.898578852180929,99.99888730639131)
(16.143134748999586,99.99897034322778)
(16.387690645818243,99.99902016532967)
(16.6322465426369,99.99910320216613)
(16.87680243945556,99.9991862390026)
(17.121358336274216,99.99925266847177)
(17.365914233092873,99.99927757952271)
(17.610470129911533,99.9993107942573)
(17.855026026730187,99.99937722372648)
(18.099581923548847,99.99943534951201)
(18.344137820367504,99.99951838634847)
(18.58869371718616,99.99952669003213)
(18.83324961400482,99.99954329739941)
(19.077805510823477,99.9995931195013)
(19.322361407642134,99.9996097268686)
(19.56691730446079,99.9996263342359)
(19.811473201279448,99.99965124528683)
(20.056029098098108,99.99965124528683)
(20.300584994916765,99.99967615633777)
(20.54514089173542,99.99968446002143)
(20.78969678855408,99.99969276370506)
(21.034252685372735,99.999717674756)
(21.278808582191395,99.99974258580696)
(21.523364479010052,99.99975919317424)
(21.76792037582871,99.99979240790883)
(22.01247627264737,99.99981731895977)
(22.257032169466026,99.99983392632707)
(22.501588066284683,99.99983392632707)
(22.74614396310334,99.99983392632707)
(22.990699859921996,99.99983392632707)
(23.235255756740656,99.9998422300107)
(23.479811653559313,99.99985053369436)
(23.72436755037797,99.99985053369436)
(23.968923447196627,99.999858837378)
(24.213479344015283,99.99986714106164)
(24.458035240833944,99.99988374842894)
(24.7025911376526,99.99988374842894)
(24.947147034471257,99.99988374842894)
(25.191702931289917,99.99988374842894)
(25.436258828108574,99.99988374842894)
(25.68081472492723,99.9998920521126)
(25.925370621745888,99.99990035579623)
(26.169926518564544,99.99990865947989)
(26.414482415383205,99.99990865947989)
(26.65903831220186,99.99991696316353)
(26.90359420902052,99.99991696316353)
(27.148150105839175,99.99991696316353)
(27.39270600265783,99.99991696316353)
(27.637261899476492,99.99991696316353)
(27.88181779629515,99.99991696316353)
(28.126373693113806,99.99991696316353)
(28.370929589932466,99.99991696316353)
(28.615485486751123,99.99991696316353)
(28.86004138356978,99.99991696316353)
(29.104597280388436,99.99991696316353)
(29.349153177207093,99.99991696316353)
(29.593709074025753,99.99991696316353)
(29.83826497084441,99.99993357053083)
(30.082820867663067,99.99993357053083)
(30.327376764481723,99.99993357053083)
(30.57193266130038,99.99993357053083)
(30.81648855811904,99.99993357053083)
(31.061044454937697,99.99993357053083)
(31.305600351756354,99.99993357053083)
(31.550156248575014,99.99993357053083)
(31.79471214539367,99.99993357053083)
(32.03926804221233,99.99994187421447)
(32.28382393903098,99.99994187421447)
(32.52837983584965,99.99994187421447)
(32.7729357326683,99.99994187421447)
(33.017491629486955,99.99994187421447)
(33.262047526305615,99.99994187421447)
(33.506603423124275,99.99994187421447)
(33.75115931994293,99.99994187421447)
(33.99571521676158,99.99994187421447)
(34.24027111358025,99.99994187421447)
(34.4848270103989,99.99995017789813)
(34.729382907217555,99.99995017789813)
(34.97393880403622,99.99995017789813)
(35.218494700854876,99.99995017789813)
(35.46305059767353,99.99995017789813)
(35.7076064944922,99.99995017789813)
(35.95216239131085,99.99995017789813)
(36.1967182881295,99.99995017789813)
(36.44127418494816,99.99995017789813)
(36.685830081766824,99.99995017789813)
(36.93038597858548,99.99995017789813)
(37.17494187540413,99.99995017789813)
(37.4194977722228,99.99995017789813)
(37.66405366904145,99.99995017789813)
(37.908609565860104,99.99995017789813)
(38.15316546267877,99.99995017789813)
(38.397721359497424,99.99995017789813)
(38.64227725631608,99.99995017789813)
(38.886833153134745,99.99995017789813)
(39.1313890499534,99.99995017789813)
(39.37594494677205,99.99995017789813)
(39.62050084359071,99.99995017789813)
(39.86505674040937,99.99995017789813)
(40.109612637228025,99.99995017789813)
(40.35416853404668,99.99995017789813)
(40.598724430865346,99.99995017789813)
(40.843280327684,99.99995017789813)
(41.08783622450265,99.99995017789813)
(41.33239212132132,99.99995017789813)
(41.57694801813997,99.99995017789813)
(41.821503914958626,99.99995017789813)
(42.06605981177729,99.99995017789813)
(42.31061570859595,99.99995848158176)
(42.5551716054146,99.99995848158176)
(42.79972750223326,99.99995848158176)
(43.04428339905192,99.99996678526541)
(43.288839295870574,99.99996678526541)
(43.53339519268923,99.99996678526541)
(43.777951089507894,99.99996678526541)
(44.02250698632655,99.99996678526541)
(44.2670628831452,99.99996678526541)
(44.51161877996387,99.99996678526541)
(44.75617467678252,99.99996678526541)
(45.000730573601174,99.99996678526541)
(45.24528647041984,99.99996678526541)
(45.489842367238495,99.99996678526541)
(45.73439826405715,99.99996678526541)
(45.97895416087581,99.99996678526541)
(46.22351005769447,99.99996678526541)
(46.46806595451312,99.99996678526541)
(46.712621851331775,99.99996678526541)
(46.95717774815044,99.99996678526541)
(47.201733644969096,99.99996678526541)
(47.44628954178775,99.99996678526541)
(47.69084543860642,99.99996678526541)
(47.93540133542507,99.99996678526541)
(48.17995723224372,99.99996678526541)
(48.42451312906239,99.99996678526541)
(48.66906902588104,99.99998339263271)
};
\addplot[dashed, magenta, thick, mark = none] coordinates{
(0.0, 0.9132228167000467)
(0.075, 0.9406433190096234)
(0.15, 0.9704456021767475)
(0.225, 1.001518835633403)
(0.3, 1.0346836329523585)
(0.375, 1.070040068959561)
(0.45, 1.1073879940031162)
(0.525, 1.1485487699152657)
(0.6, 1.191460855281494)
(0.675, 1.2365745868185642)
(0.75, 1.2849407501989236)
(0.8250000000000001, 1.3361090087058094)
(0.9, 1.3918807092062735)
(0.975, 1.448933367478864)
(1.05, 1.5597362147677818)
(1.125, 1.8411466253317603)
(1.2, 1.9301131455989644)
(1.2750000000000001, 2.025114177870794)
(1.35, 2.1243383677976024)
(1.425, 2.2247634556357787)
(1.5, 2.328551057625787)
(1.575, 2.4406148477216414)
(1.6500000000000001, 2.5584229328268746)
(1.725, 2.68126478167726)
(1.8, 2.8120225492600817)
(1.875, 2.948104297583303)
(1.95, 3.091011149036134)
(2.025, 4.063898576965998)
(2.1, 4.281621368297076)
(2.1750000000000003, 4.439709570846122)
(2.25, 4.583757275314753)
(2.325, 4.728115211743821)
(2.4, 4.873443873984578)
(2.475, 5.022695469402472)
(2.5500000000000003, 5.176040125201613)
(2.625, 5.334608686915207)
(2.7, 5.497020121945178)
(2.775, 5.665466068979776)
(2.85, 5.8389958171725)
(2.9250000000000003, 6.014527061884171)
(3.0, 6.197413806302973)
(3.075, 6.392709829139247)
(3.15, 6.585894273148033)
(3.225, 6.779138762052386)
(3.3000000000000003, 6.975815817486734)
(3.375, 7.176936195193146)
(3.45, 7.380508406135268)
(3.525, 7.588483909419072)
(3.6, 7.805265997386246)
(3.6750000000000003, 8.028773113657081)
(3.75, 8.259815864321753)
(3.825, 8.503648177742498)
(3.9, 8.757077666971595)
(3.975, 9.041570382174752)
(4.05, 9.430371088462843)
(4.125, 9.651416364015375)
(4.2, 9.874753353082099)
(4.275, 10.102503641973103)
(4.3500000000000005, 10.336188368042786)
(4.425, 10.57376600484182)
(4.5, 10.814916312927176)
(4.575, 11.060279771184915)
(4.65, 11.312488347537455)
(4.7250000000000005, 11.564336654516582)
(4.8, 11.821649046992436)
(4.875, 12.086897373165916)
(4.95, 12.352355856473887)
(5.025, 12.620576404978001)
(5.1000000000000005, 12.903628042687517)
(5.175, 13.181305662243659)
(5.25, 13.462355803434228)
(5.325, 13.7460579275124)
(5.4, 14.03535423436103)
(5.4750000000000005, 14.326702075141585)
(5.55, 14.623574046314431)
(5.625, 14.926780753969743)
(5.7, 15.233800312493651)
(5.775, 15.547845123799064)
(5.8500000000000005, 15.86954565928945)
(5.925, 16.19391819263263)
(6.0, 16.524595440010494)
(6.075, 16.871424764296265)
(6.15, 17.17076858367001)
(6.2250000000000005, 17.47143339074626)
(6.3, 17.771537778797207)
(6.375, 18.075214838134475)
(6.45, 18.380553139582464)
(6.525, 18.689324007560455)
(6.6000000000000005, 18.999175683658674)
(6.675, 19.309587778782195)
(6.75, 19.623962837013234)
(6.825, 19.94306142702899)
(6.9, 20.2599583708739)
(6.9750000000000005, 20.58032791117919)
(7.05, 20.910855046318133)
(7.125, 21.23875021353466)
(7.2, 21.56734590453282)
(7.275, 21.899504259334705)
(7.3500000000000005, 22.233594058277372)
(7.425, 22.573268032507908)
(7.5, 22.913732597863422)
(7.575, 23.255348023717335)
(7.65, 23.602877871784735)
(7.7250000000000005, 23.948396215850593)
(7.8, 24.29987901954291)
(7.875, 24.647839189361886)
(7.95, 24.99294722664136)
(8.025, 25.361192563679865)
(8.1, 25.69646324556871)
(8.175, 26.03181398731832)
(8.25, 26.36762507326728)
(8.325, 26.705167453705137)
(8.4, 27.046902969350185)
(8.475, 27.388708537373397)
(8.55, 27.734867360325318)
(8.625, 28.079044701723475)
(8.700000000000001, 28.42402264172922)
(8.775, 28.772463170712744)
(8.85, 29.12335553293197)
(8.925, 29.475739010057822)
(9.0, 29.830674395245328)
(9.075000000000001, 30.189622780953318)
(9.15, 30.545138600131317)
(9.225, 30.905578100745927)
(9.3, 31.26446644155835)
(9.375, 31.62747786519981)
(9.450000000000001, 31.988117515466314)
(9.525, 32.34969786909672)
(9.6, 32.71727270480138)
(9.675, 33.081324906632695)
(9.75, 33.447478679808896)
(9.825000000000001, 33.81425291690597)
(9.9, 34.17380175156965)
(9.975, 34.53548218002601)
(10.05, 34.90890138556599)
(10.125, 35.26690906791007)
(10.200000000000001, 35.62822922699303)
(10.275, 35.98926917656332)
(10.35, 36.3522405702744)
(10.425, 36.71332054977507)
(10.5, 37.07424040955422)
(10.575000000000001, 37.43762211005169)
(10.65, 37.79999305480708)
(10.725, 38.16323465054822)
(10.8, 38.531850264442724)
(10.875, 38.897753850554054)
(10.950000000000001, 39.26676976375236)
(11.025, 39.63466483890004)
(11.1, 40.005061784696416)
(11.175, 40.376049171965875)
(11.25, 40.74973857953592)
(11.325000000000001, 41.11704321321052)
(11.4, 41.49265405743875)
(11.475, 41.86533270926672)
(11.55, 42.235419423102655)
(11.625, 42.60588642127719)
(11.700000000000001, 42.97633340448653)
(11.775, 43.34552945237154)
(11.85, 43.71889862049855)
(11.925, 44.089966067628765)
(12.0, 44.46026293859919)
(12.075000000000001, 44.84107767377668)
(12.15, 45.21267551748443)
(12.225, 45.58376297957983)
(12.3, 45.95780264904069)
(12.375, 46.32883006624053)
(12.450000000000001, 46.70458101522508)
(12.525, 47.07748983915273)
(12.6, 47.45247021197749)
(12.675, 47.83039278468511)
(12.75, 48.208685634248724)
(12.825000000000001, 48.59138177615403)
(12.9, 48.97563908534411)
(12.975, 49.362458310078445)
(13.05, 49.75161928573995)
(13.125, 50.144963389126055)
(13.200000000000001, 50.53743684152641)
(13.275, 50.929149725249566)
(13.35, 51.32481556459765)
(13.425, 51.72268305011657)
(13.5, 52.12825629723344)
(13.575000000000001, 52.53857309110022)
(13.65, 52.95027091756507)
(13.725, 53.37287690005817)
(13.8, 53.794241954709534)
(13.875, 54.22271232200316)
(13.950000000000001, 54.6604796406273)
(14.025, 55.169440190430386)
(14.1, 55.79581853351752)
(14.175, 56.45075823193001)
(14.25, 57.12428182552094)
(14.325000000000001, 57.81962173116839)
(14.4, 58.54351298465863)
(14.475, 59.30812468482684)
(14.55, 60.105390800701684)
(14.625, 60.933720142550584)
(14.700000000000001, 61.80875440566912)
(14.775, 66.05816168749374)
(14.85, 76.73958819008972)
(14.925, 88.14040257900832)
};
\addplot[dashed, black, thick, mark = none] coordinates{
(0.0, 0.4969173404829157)
(0.075, 0.5062340735347652)
(0.15, 0.5163977823186011)
(0.225, 0.5269434605501954)
(0.3, 0.53835272188107)
(0.375, 0.550268507914407)
(0.45, 0.562831981272204)
(0.525, 0.5761012677399898)
(0.6, 0.5904915515001102)
(0.675, 0.6063432835820896)
(0.75, 0.6221950156640689)
(0.8250000000000001, 0.6391677450383829)
(0.9, 0.6574524564289111)
(0.975, 0.6764180698784872)
(1.05, 0.7090598502945483)
(1.125, 0.7954098565389183)
(1.2, 0.8221975399838976)
(1.2750000000000001, 0.8511690922280178)
(1.35, 0.8842177531427782)
(1.425, 0.9161703278161446)
(1.5, 0.9497006023824264)
(1.575, 0.9857551967773736)
(1.6500000000000001, 1.02340409843253)
(1.725, 1.0635690162327052)
(1.8, 1.1058513733628457)
(1.875, 1.1509735903002347)
(1.95, 1.1987446823209924)
(2.025, 1.7221922920558328)
(2.1, 1.7916692131296517)
(2.1750000000000003, 1.843243392260701)
(2.25, 1.8896692875306573)
(2.325, 1.9366432259213102)
(2.4, 1.9850370942155877)
(2.475, 2.0365116291428738)
(2.5500000000000003, 2.0894891308102537)
(2.625, 2.143712185024672)
(2.7, 2.2025603910304272)
(2.775, 2.2620978027788774)
(2.85, 2.3243173043452843)
(2.9250000000000003, 2.3913861571614956)
(3.0, 2.462689888637638)
(3.075, 2.5398061986666276)
(3.15, 2.6193803990551072)
(3.225, 2.7038454691116254)
(3.3000000000000003, 2.7930602462141843)
(3.375, 2.890636832749197)
(3.45, 2.9943913599175214)
(3.525, 3.1081933442986243)
(3.6, 3.229892131827953)
(3.6750000000000003, 3.3595624556583292)
(3.75, 3.497171101055166)
(3.825, 3.6439885316164413)
(3.9, 3.796552111261389)
(3.975, 3.9640457141035075)
(4.05, 4.160718461280919)
(4.125, 4.3076438397296055)
(4.2, 4.464525334870954)
(4.275, 4.632600195568357)
(4.3500000000000005, 4.812590842299097)
(4.425, 5.005867382864917)
(4.5, 5.2136587624455615)
(4.575, 5.438995825572157)
(4.65, 5.677577264115598)
(4.7250000000000005, 5.928796909169658)
(4.8, 6.202577662692413)
(4.875, 6.492376221970085)
(4.95, 6.800127345292409)
(5.025, 7.128961521394276)
(5.1000000000000005, 7.478231062951222)
(5.175, 7.847404534209848)
(5.25, 8.235319419459582)
(5.325, 8.641660178721844)
(5.4, 9.071799295316191)
(5.4750000000000005, 9.520206515933772)
(5.55, 9.991232970805578)
(5.625, 10.479414836091928)
(5.7, 10.992316767595174)
(5.775, 11.52684979499866)
(5.8500000000000005, 12.083105258822497)
(5.925, 12.66119941063775)
(6.0, 13.257935332240347)
(6.075, 13.880611961555939)
(6.15, 14.515802242127442)
(6.2250000000000005, 15.172058968111198)
(6.3, 15.844051174605875)
(6.375, 16.53359736833015)
(6.45, 17.238314392077356)
(6.525, 17.967560497317578)
(6.6000000000000005, 18.71260020885425)
(6.675, 19.468443012815573)
(6.75, 20.24003790465511)
(6.825, 21.023714656200926)
(6.9, 21.815313121945906)
(6.9750000000000005, 22.6223979576924)
(7.05, 23.43845077177757)
(7.125, 24.258979271348437)
(7.2, 25.086009555214844)
(7.275, 25.916651941467666)
(7.3500000000000005, 26.750399905404436)
(7.425, 27.58905534637654)
(7.5, 28.4297036714239)
(7.575, 29.272876316299936)
(7.65, 30.108550734842787)
(7.7250000000000005, 30.937416132795164)
(7.8, 31.767742979069403)
(7.875, 32.594872907139575)
(7.95, 33.41305146423836)
(8.025, 34.22857284257013)
(8.1, 35.029454826632374)
(8.175, 35.81735815315447)
(8.25, 36.594126239906046)
(8.325, 37.364309505525604)
(8.4, 38.123291101905465)
(8.475, 38.86482665894314)
(8.55, 39.598083443384816)
(8.625, 40.31560474731559)
(8.700000000000001, 41.01306435155538)
(8.775, 41.69369238904286)
(8.85, 42.367876768020324)
(8.925, 43.02274677883504)
(9.0, 43.66313516536952)
(9.075000000000001, 44.28660064463157)
(9.15, 44.893168127672126)
(9.225, 45.47962408891983)
(9.3, 46.04844302610147)
(9.375, 46.60949801907323)
(9.450000000000001, 47.1497439808258)
(9.525, 47.67525090410508)
(9.6, 48.182755441237816)
(9.675, 48.677671593961826)
(9.75, 49.15570635783163)
(9.825000000000001, 49.61625356394102)
(9.9, 50.06293361836004)
(9.975, 50.49758993885831)
(10.05, 50.9185866997574)
(10.125, 51.322594123914875)
(10.200000000000001, 51.71207010169023)
(10.275, 52.08970502658508)
(10.35, 52.45745856794007)
(10.425, 52.810713877647544)
(10.5, 53.1511898182224)
(10.575000000000001, 53.48158508684989)
(10.65, 53.80176682459166)
(10.725, 54.11220003773194)
(10.8, 54.412245342629916)
(10.875, 54.70402017861555)
(10.950000000000001, 54.98860402456296)
(11.025, 55.26488418686344)
(11.1, 55.53651428632163)
(11.175, 55.799417214266924)
(11.25, 56.05691444415805)
(11.325000000000001, 56.305900398311096)
(11.4, 56.552320514217236)
(11.475, 56.793368146803815)
(11.55, 57.027374255657804)
(11.625, 57.25936256938559)
(11.700000000000001, 57.491035343134776)
(11.775, 57.718307164551106)
(11.85, 57.93951729690519)
(11.925, 58.15959812828327)
(12.0, 58.37749509086223)
(12.075000000000001, 58.59598991866376)
(12.15, 58.80997584624501)
(12.225, 59.02287399126851)
(12.3, 59.232583521771595)
(12.375, 59.44123848445152)
(12.450000000000001, 59.65192784962494)
(12.525, 59.85984378446029)
(12.6, 60.06953670759607)
(12.675, 60.27927945283375)
(12.75, 60.49015980273105)
(12.825000000000001, 60.70515877971723)
(12.9, 60.916769853775456)
(12.975, 61.13025756033789)
(13.05, 61.34844515184448)
(13.125, 61.564581733490286)
(13.200000000000001, 61.78546802218213)
(13.275, 62.0060055561608)
(13.35, 62.22949920151778)
(13.425, 62.45551716670342)
(13.5, 62.687380925176505)
(13.575000000000001, 62.92040719936015)
(13.65, 63.160151153614166)
(13.725, 63.40534232434055)
(13.8, 63.65456908531936)
(13.875, 63.91151827208979)
(13.950000000000001, 64.17222902755229)
(14.025, 64.49729333127846)
(14.1, 64.92511572013531)
(14.175, 65.37155496772856)
(14.25, 65.84285544416072)
(14.325000000000001, 66.34035404249892)
(14.4, 66.85715040163257)
(14.475, 67.40418877660832)
(14.55, 67.96977758085131)
(14.625, 68.57305680516768)
(14.700000000000001, 69.21068006504774)
(14.775, 72.6176897690646)
(14.85, 81.23674732089951)
(14.925, 90.38879341497959)
};
