# Supplementary material for: CausalSim: A Causal Framework for Unbiased Trace-Driven Simulation
Source: arXiv:2201.01811 source file (2023-05-05)
Supplement: Supplementary file 5 [file new_bola_basic_v2_bola_basic_v1.tex]

\addplot[solid, green!70!black, thick, mark = none] coordinates{
(0.0, 0.5049875792129775)
(0.07952424440737206, 0.5135840067618558)
(0.15904848881474412, 0.5289655075099652)
(0.2385727332221162, 0.5541243187531317)
(0.31809697762948824, 0.5904614880546184)
(0.39762122203686034, 0.6405589459238673)
(0.4771454664442324, 0.7108014662563199)
(0.5566697108516044, 0.8059626182496653)
(0.6361939552589765, 0.9248314965099406)
(0.7157181996663486, 1.0610833720372723)
(0.7952424440737207, 1.2252661314865125)
(0.8747666884810927, 1.4168293633149505)
(0.9542909328884648, 1.6118651916037623)
(1.0338151772958368, 1.783683660272786)
(1.1133394217032089, 1.9503883053358997)
(1.192863666110581, 2.1105680717472453)
(1.272387910517953, 2.2552762700671294)
(1.351912154925325, 2.3968621338174554)
(1.4314363993326973, 2.539899082544018)
(1.5109606437400693, 2.671447441251824)
(1.5904848881474414, 2.8056177603994503)
(1.6700091325548134, 2.94423140181914)
(1.7495333769621855, 3.093723176819308)
(1.8290576213695575, 3.268603935162321)
(1.9085818657769296, 3.463879943033406)
(1.9881061101843016, 3.672225723173217)
(2.0676303545916737, 3.825970678276147)
(2.147154598999046, 3.9542866201058535)
(2.2266788434064178, 4.076718162169855)
(2.30620308781379, 4.1985092253477925)
(2.385727332221162, 4.322722099313657)
(2.465251576628534, 4.446434599149784)
(2.544775821035906, 4.574590421257974)
(2.624300065443278, 4.701605390350365)
(2.70382430985065, 4.833433958570824)
(2.7833485542580223, 4.9673841131013665)
(2.8628727986653946, 5.101154132945203)
(2.9423970430727664, 5.236435282660846)
(3.0219212874801387, 5.376680143743477)
(3.1014455318875105, 5.520907982898813)
(3.1809697762948828, 5.666646951925955)
(3.2604940207022546, 5.81812020847988)
(3.340018265109627, 5.972595709812226)
(3.4195425095169987, 6.131774727964099)
(3.499066753924371, 6.296397816647508)
(3.5785909983317428, 6.4665650506884)
(3.658115242739115, 6.644117806884207)
(3.737639487146487, 6.826263997590999)
(3.817163731553859, 7.009821243343647)
(3.8966879759612314, 7.196140554292445)
(3.9762122203686032, 7.380568451030836)
(4.0557364647759755, 7.560783197596843)
(4.135260709183347, 7.738566125892329)
(4.214784953590719, 7.911275260512285)
(4.294309197998092, 8.076618887942514)
(4.373833442405464, 8.247276488630549)
(4.4533576868128355, 8.420185772902398)
(4.532881931220207, 8.592714772835649)
(4.61240617562758, 8.769226750841604)
(4.691930420034952, 8.950942619796821)
(4.771454664442324, 9.135250426744076)
(4.850978908849696, 9.323070860082083)
(4.930503153257068, 9.516075169404163)
(5.01002739766444, 9.711010922867027)
(5.089551642071812, 9.91057013328866)
(5.169075886479185, 10.110569672944461)
(5.248600130886556, 10.315482886554276)
(5.328124375293928, 10.527921727075334)
(5.4076486197013, 10.745754600714955)
(5.487172864108673, 10.96530876136087)
(5.566697108516045, 11.190236940160156)
(5.646221352923416, 11.419268186823288)
(5.725745597330789, 11.65318308499265)
(5.805269841738161, 11.886407466862973)
(5.884794086145533, 12.123574796875623)
(5.964318330552905, 12.36208312955597)
(6.043842574960277, 12.605615218498873)
(6.123366819367649, 12.849427516954426)
(6.202891063775021, 13.092229059667915)
(6.282415308182393, 13.333059128310238)
(6.3619395525897655, 13.57739181586072)
(6.441463796997137, 13.825147062458601)
(6.520988041404509, 14.072912316539076)
(6.600512285811881, 14.322348820212873)
(6.680036530219254, 14.57744955903529)
(6.7595607746266255, 14.835622595014291)
(6.839085019033997, 15.095046566317635)
(6.91860926344137, 15.357773006877244)
(6.998133507848742, 15.626844191401911)
(7.077657752256114, 15.899648166934416)
(7.1571819966634855, 16.17213190302389)
(7.236706241070858, 16.448758736907585)
(7.31623048547823, 16.731540172587042)
(7.395754729885602, 17.017864257105035)
(7.475278974292974, 17.30883181354699)
(7.554803218700346, 17.60605404661065)
(7.634327463107718, 17.903716608908482)
(7.71385170751509, 18.204591573119224)
(7.793375951922463, 18.506717472654305)
(7.872900196329835, 18.811014995912444)
(7.9524244407372064, 19.118354793879384)
(8.03194868514458, 19.431078617482292)
(8.111472929551951, 19.744442919971263)
(8.190997173959323, 20.058757933306733)
(8.270521418366695, 20.375584824773483)
(8.350045662774066, 20.694863549475944)
(8.429569907181438, 21.016804264548604)
(8.50909415158881, 21.34099666320508)
(8.588618395996184, 21.670783244632013)
(8.668142640403556, 22.00248125523454)
(8.747666884810927, 22.33624080725158)
(8.8271911292183, 22.671061152423665)
(8.906715373625671, 23.015458658438913)
(8.986239618033043, 23.36242808748101)
(9.065763862440415, 23.7099779505136)
(9.145288106847788, 24.064793245909964)
(9.22481235125516, 24.421459925586362)
(9.304336595662532, 24.78460144650155)
(9.383860840069904, 25.14989457617461)
(9.463385084477276, 25.518029830904567)
(9.542909328884647, 25.897503563414364)
(9.62243357329202, 26.277067363267513)
(9.701957817699393, 26.655110025766266)
(9.781482062106765, 27.041949265465785)
(9.861006306514136, 27.435163271578162)
(9.940530550921508, 27.83188990408128)
(10.02005479532888, 28.23295978403052)
(10.099579039736252, 28.639994123606222)
(10.179103284143624, 29.050410992298943)
(10.258627528550996, 29.462419050724225)
(10.33815177295837, 29.88236304284714)
(10.417676017365741, 30.305629519191502)
(10.497200261773113, 30.737442385671766)
(10.576724506180485, 31.171046591536495)
(10.656248750587856, 31.606952518398007)
(10.735772994995228, 32.05006383272773)
(10.8152972394026, 32.49895947199721)
(10.894821483809974, 32.95538073817794)
(10.974345728217346, 33.416225311665535)
(11.053869972624717, 33.88258400806283)
(11.13339421703209, 34.35788939389982)
(11.212918461439461, 34.83505617149943)
(11.292442705846833, 35.32901550489301)
(11.371966950254205, 35.82226430702236)
(11.451491194661578, 36.323098780958524)
(11.53101543906895, 36.82845663702751)
(11.610539683476322, 37.345873509623146)
(11.690063927883694, 37.87019554520915)
(11.769588172291066, 38.40292386617474)
(11.849112416698437, 38.94222710320507)
(11.92863666110581, 39.484882846904625)
(12.008160905513181, 40.036345175287565)
(12.087685149920555, 40.59402215036182)
(12.167209394327926, 41.155712125956576)
(12.246733638735298, 41.72894072898306)
(12.32625788314267, 42.30602221280852)
(12.405782127550042, 42.88769713114496)
(12.485306371957414, 43.47072305963169)
(12.564830616364786, 44.06307596189671)
(12.64435486077216, 44.66529624200014)
(12.723879105179531, 45.269207786662086)
(12.803403349586903, 45.87884361136822)
(12.882927593994275, 46.49145165840499)
(12.962451838401646, 47.112526035716904)
(13.041976082809018, 47.73509152793544)
(13.12150032721639, 48.363171143063674)
(13.201024571623762, 48.99211140169505)
(13.280548816031136, 49.61829960261287)
(13.360073060438507, 50.25309423856217)
(13.43959730484588, 50.881744280198305)
(13.519121549253251, 51.52104228331523)
(13.598645793660623, 52.15790846816164)
(13.678170038067995, 52.79919796031493)
(13.757694282475367, 53.442939285703915)
(13.83721852688274, 54.09043341706594)
(13.916742771290112, 54.73909842389154)
(13.996267015697484, 55.39065559318702)
(14.075791260104856, 56.04985847918489)
(14.155315504512227, 56.71184344534408)
(14.2348397489196, 57.38660796677676)
(14.314363993326971, 58.081417475846685)
(14.393888237734345, 58.82427290885395)
(14.473412482141716, 59.63309766712571)
(14.552936726549088, 60.56304298724156)
(14.63246097095646, 61.68168939916375)
(14.711985215363832, 63.088151010510565)
(14.791509459771204, 65.15837891991842)
(14.871033704178576, 76.83991320310196)
(14.950557948585947, 99.21404233945721)
(15.030082192993321, 99.97569182477739)
(15.109606437400693, 99.99663748584817)
(15.189130681808065, 99.99877908712345)
(15.268654926215437, 99.99960970817881)
(15.348179170622808, 99.99989992517405)
(15.42770341503018, 99.99995997006963)
(15.507227659437552, 99.99996997755221)
(15.586751903844926, 99.99997998503481)
(15.666276148252297, 99.9999899925174)
(15.74580039265967, 99.9999899925174)
(15.825324637067041, 99.9999899925174)
};
\addplot[solid, blue, thick, mark = none] coordinates{
(0.0, 0.4986352084424983)
(0.075, 0.4986453026813024)
(0.15, 0.4986453026813024)
(0.225, 0.4986453026813024)
(0.3, 0.4986453026813024)
(0.375, 0.4986453026813024)
(0.45, 0.4986553969201064)
(0.525, 0.49866549115891046)
(0.6, 0.49866549115891046)
(0.675, 0.49866549115891046)
(0.75, 0.49869577387532266)
(0.8250000000000001, 0.49869577387532266)
(0.9, 0.4987159623529307)
(0.975, 0.4987159623529307)
(1.05, 0.49873615083053885)
(1.125, 0.49873615083053885)
(1.2, 0.49873615083053885)
(1.2750000000000001, 0.498766433546951)
(1.35, 0.4987967162633632)
(1.425, 0.4988068105021672)
(1.5, 0.4988370932185794)
(1.575, 0.4988471874573834)
(1.6500000000000001, 0.4988673759349914)
(1.725, 0.4989380356066198)
(1.8, 0.4989885068006401)
(1.875, 0.4990692607110725)
(1.95, 0.4990894491886806)
(2.025, 3.2895509184192706)
(2.1, 3.373312912015283)
(2.1750000000000003, 3.4593360151034034)
(2.25, 3.549063703832611)
(2.325, 3.640487224680898)
(2.4, 3.7351106192300696)
(2.475, 3.8307333434208424)
(2.5500000000000003, 3.929485281640871)
(2.625, 4.030922287382777)
(2.7, 4.136780569720857)
(2.775, 4.244243836028781)
(2.85, 4.354483018007819)
(2.9250000000000003, 4.468931497568147)
(3.0, 4.5886794525006005)
(3.075, 4.710890401701243)
(3.15, 4.839713077318538)
(3.225, 4.974319751770555)
(3.3000000000000003, 5.109633022938855)
(3.375, 5.25280970613551)
(3.45, 5.4002663465850835)
(3.525, 5.555939697421154)
(3.6, 5.7192341985542825)
(3.6750000000000003, 5.893369912162962)
(3.75, 6.080779549798968)
(3.825, 6.288549267102744)
(3.9, 6.5105619553590355)
(3.975, 6.680478277147622)
(4.05, 6.809422083630566)
(4.125, 6.940626999605618)
(4.2, 7.073881046057892)
(4.275, 7.2083363069278485)
(4.3500000000000005, 7.347152278961154)
(4.425, 7.49020783129216)
(4.5, 7.635938356906241)
(4.575, 7.789693802369542)
(4.65, 7.945478189832457)
(4.7250000000000005, 8.100939561653641)
(4.8, 8.260539571384488)
(4.875, 8.425691412457564)
(4.95, 8.596263859768412)
(5.025, 8.770227971317421)
(5.1000000000000005, 8.94911807140281)
(5.175, 9.129451647637175)
(5.25, 9.3181533478401)
(5.325, 9.511690188430165)
(5.4, 9.712464598242734)
(5.4750000000000005, 9.917720850084303)
(5.55, 10.132909832909055)
(5.625, 10.352469621135963)
(5.7, 10.580538852674685)
(5.775, 10.814230575227263)
(5.8500000000000005, 11.039049461871082)
(5.925, 11.244154300130589)
(6.0, 11.444080793883618)
(6.075, 11.641978345637034)
(6.15, 11.84655828347873)
(6.2250000000000005, 12.053560838633398)
(6.3, 12.266640125548104)
(6.375, 12.483171642133797)
(6.45, 12.704649335733473)
(6.525, 12.93076028494421)
(6.6000000000000005, 13.16046478316919)
(6.675, 13.392834160438438)
(6.75, 13.628998971498007)
(6.825, 13.870554106078941)
(6.9, 14.118337386001976)
(6.9750000000000005, 14.371258633476272)
(7.05, 14.628692005695976)
(7.125, 14.892686633138316)
(7.2, 15.158094454013222)
(7.275, 15.430325980319667)
(7.3500000000000005, 15.708492919042893)
(7.425, 15.992050181287482)
(7.5, 16.279958060456618)
(7.575, 16.573024095654624)
(7.65, 16.871117061777046)
(7.7250000000000005, 17.165616478885223)
(7.8, 17.459873634262106)
(7.875, 17.74807424635656)
(7.95, 18.034367047317048)
(8.025, 18.32214370138173)
(8.1, 18.61447285714704)
(8.175, 18.910062452046056)
(8.25, 19.211637930555877)
(8.325, 19.521177763482093)
(8.4, 19.83454331291504)
(8.475, 20.150472799004223)
(8.55, 20.47127780243576)
(8.625, 20.79550475282187)
(8.700000000000001, 21.12534409998303)
(8.775, 21.461643759978784)
(8.85, 21.807502664121976)
(8.925, 22.151807055489343)
(9.0, 22.50343986422845)
(9.075000000000001, 22.862310242190063)
(9.15, 23.222654379017065)
(9.225, 23.5965348900803)
(9.3, 23.970163045173436)
(9.375, 24.353734025488556)
(9.450000000000001, 24.737537173296175)
(9.525, 25.128971565639656)
(9.6, 25.525382417713534)
(9.675, 25.919077919549117)
(9.75, 26.31540801771256)
(9.825000000000001, 26.711384817517864)
(9.9, 27.109905365501792)
(9.975, 27.5163801736633)
(10.05, 27.930254058868186)
(10.125, 28.343794834192536)
(10.200000000000001, 28.767530790708978)
(10.275, 29.197757342776427)
(10.35, 29.63293007185786)
(10.425, 30.0728672816548)
(10.5, 30.518043401391047)
(10.575000000000001, 30.972324524528545)
(10.65, 31.43667969799249)
(10.725, 31.900701761575895)
(10.8, 32.37320298575471)
(10.875, 32.85383007217078)
(10.950000000000001, 33.34183604715261)
(11.025, 33.833597078969554)
(11.1, 34.336855448784306)
(11.175, 34.83913467743507)
(11.25, 35.34624904647296)
(11.325000000000001, 35.86442670124011)
(11.4, 36.38718714042429)
(11.475, 36.91369254220477)
(11.55, 37.439885022582324)
(11.625, 37.96675381695975)
(11.700000000000001, 38.493451009277514)
(11.775, 39.02072357320711)
(11.85, 39.55962470023896)
(11.925, 40.10109985816585)
(12.0, 40.646400732599474)
(12.075000000000001, 41.19380120870434)
(12.15, 41.74844934827052)
(12.225, 42.30662037717931)
(12.3, 42.859946171462155)
(12.375, 43.4147861015656)
(12.450000000000001, 43.97209912017605)
(12.525, 44.52855412848815)
(12.6, 45.09012691587391)
(12.675, 45.648065777290206)
(12.75, 46.20429871234862)
(12.825000000000001, 46.75839166878057)
(12.9, 47.307578825153755)
(12.975, 47.86087433672019)
(13.05, 48.412060152376576)
(13.125, 48.956210283586536)
(13.200000000000001, 49.49598960939434)
(13.275, 50.035799217918566)
(13.35, 50.570854439966084)
(13.425, 51.10003481502964)
(13.5, 51.62745879254128)
(13.575000000000001, 52.15058262432242)
(13.65, 52.670405640014614)
(13.725, 53.18885583922947)
(13.8, 53.70594331620576)
(13.875, 54.2256149183159)
(13.950000000000001, 54.74150118087453)
(14.025, 55.25899242740299)
(14.1, 55.78138947399023)
(14.175, 56.308005912397554)
(14.25, 56.84262708217649)
(14.325000000000001, 57.380670198909996)
(14.4, 57.92928198367135)
(14.475, 58.4878365936547)
(14.55, 59.06122973468)
(14.625, 59.652883353701824)
(14.700000000000001, 60.26179812107858)
(14.775, 60.89483811919701)
(14.85, 61.55825168187683)
(14.925, 62.257287813296145)
};
\addplot[solid, red, thick, mark = none] coordinates{
(0.001328141468250317,0.5929333362555183)
(0.134142288293282,0.6270488444209735)
(0.2669564351183137,0.676746002986433)
(0.39977058194334536,0.7579867466905005)
(0.5325847287683771,0.8960499765674794)
(0.6653988755934088,1.0745834660575713)
(0.7982130224184405,1.2779755423129873)
(0.9310271692434722,1.4822382695541456)
(1.0638413160685039,1.6928657557255562)
(1.1966554628935355,1.9067156512924714)
(1.3294696097185672,2.1239380684938127)
(1.462283756543599,2.3446631046033115)
(1.5950979033686306,2.5828511978406254)
(1.7279120501936625,2.850551357249816)
(1.860726197018694,3.159352247675587)
(1.9935403438437258,3.50942399632205)
(2.1263544906687573,3.77031906756682)
(2.259168637493789,3.9919747995576293)
(2.391982784318821,4.207485937235271)
(2.5247969311438525,4.418823954670907)
(2.657611077968884,4.631593042117591)
(2.790425224793916,4.849095668831585)
(2.9232393716189478,5.071662081738515)
(3.056053518443979,5.30454620920062)
(3.1888676652690107,5.545416307773323)
(3.3216818120940426,5.797244599787261)
(3.4544959589190745,6.063053344986046)
(3.587310105744106,6.341251353637115)
(3.7201242525691374,6.638613691457103)
(3.8529383993941693,6.93981890259347)
(3.985752546219201,7.207318912350765)
(4.118566693044233,7.465562000707929)
(4.251380839869265,7.723434812209089)
(4.384194986694296,7.98746222550601)
(4.517009133519328,8.261757315945133)
(4.64982328034436,8.546350105974238)
(4.782637427169391,8.840850303772129)
(4.915451573994423,9.148650445938427)
(5.048265720819455,9.471331714723098)
(5.1810798676444865,9.80515131163571)
(5.313894014469518,10.155983628959373)
(5.446708161294549,10.512159941988624)
(5.579522308119581,10.885168840742223)
(5.712336454944613,11.257657350400894)
(5.845150601769644,11.626102837091294)
(5.977964748594676,11.989794769549192)
(6.110778895419708,12.361232493535416)
(6.24359304224474,12.742357460673345)
(6.376407189069772,13.13790321023029)
(6.509221335894804,13.545678103518)
(6.642035482719835,13.961188780851444)
(6.774849629544867,14.38809798086029)
(6.9076637763698985,14.831589579528615)
(7.0404779231949295,15.284027867636633)
(7.173292070019961,15.746483645821982)
(7.306106216844993,16.22190912145011)
(7.438920363670025,16.70601108448787)
(7.571734510495057,17.198589385283377)
(7.704548657320088,17.69452019274812)
(7.83736280414512,18.19507445717163)
(7.970176950970152,18.70535599467722)
(8.102991097795183,19.22412387742315)
(8.235805244620217,19.758793650012112)
(8.368619391445247,20.300658802586693)
(8.501433538270279,20.85935654088562)
(8.63424768509531,21.43528716421268)
(8.76706183192034,22.023526991131266)
(8.899875978745374,22.627268408589103)
(9.032690125570404,23.24486018195805)
(9.165504272395438,23.87602210172546)
(9.298318419220468,24.524066644630192)
(9.431132566045502,25.189294035150084)
(9.563946712870532,25.861706798172996)
(9.696760859695562,26.548059984450372)
(9.829575006520596,27.24482095262628)
(9.962389153345626,27.962697709077077)
(10.09520330017066,28.702480844927752)
(10.22801744699569,29.45560395507721)
(10.360831593820723,30.221446575604578)
(10.493645740645754,31.00922559797961)
(10.626459887470787,31.804850486708915)
(10.759274034295817,32.62913680558954)
(10.892088181120847,33.47211710195713)
(11.024902327945881,34.32897777668363)
(11.157716474770911,35.19794750534975)
(11.290530621595945,36.0826389891722)
(11.423344768420975,36.980360215333)
(11.556158915246009,37.89310267286851)
(11.688973062071039,38.82420886096534)
(11.82178720889607,39.75824724146244)
(11.954601355721103,40.70859781858896)
(12.087415502546133,41.67396962709017)
(12.220229649371166,42.643534570798586)
(12.353043796196197,43.63189356681991)
(12.48585794302123,44.62485600483482)
(12.61867208984626,45.625063860248304)
(12.751486236671294,46.62429098236752)
(12.884300383496324,47.62904223487902)
(13.017114530321356,48.636505515173695)
(13.149928677146388,49.637884246050774)
(13.282742823971418,50.632698068345704)
(13.415556970796452,51.62466976558373)
(13.548371117621482,52.604692528603636)
(13.681185264446516,53.574037307694965)
(13.813999411271546,54.54217118139233)
(13.94681355809658,55.513387359728874)
(14.07962770492161,56.510072581269014)
(14.212441851746641,57.53960236068508)
(14.345255998571673,58.63543171229127)
(14.478070145396703,59.860067372374324)
(14.610884292221737,61.37141740879656)
(14.743698439046767,63.60265570567113)
(14.8765125858718,83.91694469955185)
(15.009326732696831,99.91022287364262)
(15.142140879521865,99.99554667024533)
(15.274955026346895,99.99942957349211)
(15.407769173171925,99.99966975307437)
(15.540583319996959,99.99971979048735)
(15.673397466821989,99.9998098578307)
(15.806211613647022,99.99982987279589)
(15.939025760472052,99.99984988776109)
(16.071839907297083,99.99987991020886)
(16.204654054122116,99.99988991769145)
(16.33746820094715,99.99990993265665)
(16.47028234777218,99.99991994013924)
(16.60309649459721,99.99992994762184)
(16.735910641422244,99.99992994762184)
(16.868724788247278,99.99993995510444)
(17.001538935072308,99.99993995510444)
(17.134353081897338,99.99993995510444)
(17.26716722872237,99.99993995510444)
(17.3999813755474,99.99993995510444)
(17.53279552237243,99.99994996258704)
(17.665609669197465,99.99995997006963)
(17.7984238160225,99.99995997006963)
(17.93123796284753,99.99995997006963)
(18.06405210967256,99.99995997006963)
(18.196866256497593,99.99995997006963)
(18.329680403322623,99.99996997755221)
(18.462494550147653,99.99996997755221)
(18.595308696972687,99.99996997755221)
(18.72812284379772,99.99996997755221)
(18.86093699062275,99.99996997755221)
(18.99375113744778,99.99996997755221)
(19.126565284272814,99.99996997755221)
(19.259379431097845,99.99996997755221)
(19.392193577922875,99.99996997755221)
(19.52500772474791,99.99996997755221)
(19.657821871572942,99.99996997755221)
(19.790636018397972,99.99996997755221)
(19.923450165223002,99.99996997755221)
(20.056264312048036,99.99997998503481)
(20.18907845887307,99.99997998503481)
(20.3218926056981,99.99997998503481)
(20.45470675252313,99.99997998503481)
(20.587520899348164,99.99997998503481)
(20.720335046173194,99.99997998503481)
(20.853149192998224,99.99997998503481)
(20.985963339823257,99.99997998503481)
(21.11877748664829,99.99997998503481)
(21.25159163347332,99.99997998503481)
(21.38440578029835,99.99997998503481)
(21.517219927123385,99.99997998503481)
(21.650034073948415,99.99997998503481)
(21.782848220773445,99.99997998503481)
(21.91566236759848,99.99997998503481)
(22.048476514423513,99.99997998503481)
(22.181290661248543,99.99997998503481)
(22.314104808073573,99.99997998503481)
(22.446918954898607,99.99997998503481)
(22.57973310172364,99.9999899925174)
(22.71254724854867,99.9999899925174)
(22.8453613953737,99.9999899925174)
(22.978175542198734,99.9999899925174)
(23.110989689023764,99.9999899925174)
(23.243803835848794,99.9999899925174)
(23.376617982673828,99.9999899925174)
(23.50943212949886,99.9999899925174)
(23.642246276323892,99.9999899925174)
(23.775060423148922,99.9999899925174)
(23.907874569973956,99.9999899925174)
(24.040688716798986,99.9999899925174)
(24.173502863624016,99.9999899925174)
(24.30631701044905,99.9999899925174)
(24.439131157274083,99.9999899925174)
(24.571945304099113,99.9999899925174)
(24.704759450924143,99.9999899925174)
(24.837573597749177,99.9999899925174)
(24.970387744574207,99.9999899925174)
(25.103201891399237,99.9999899925174)
(25.23601603822427,99.9999899925174)
(25.368830185049305,99.9999899925174)
(25.501644331874335,99.9999899925174)
(25.634458478699365,99.9999899925174)
(25.7672726255244,99.9999899925174)
(25.900086772349432,99.9999899925174)
(26.032900919174462,99.9999899925174)
(26.165715065999493,99.9999899925174)
(26.298529212824526,99.9999899925174)
(26.431343359649556,99.9999899925174)
};
\addplot[dashed, magenta, thick, mark = none] coordinates{
(0.0, 0.845713581991646)
(0.075, 0.868949896108504)
(0.15, 0.8929784712591263)
(0.225, 0.9178795364089575)
(0.3, 0.9438035208682057)
(0.375, 0.9720441167046635)
(0.45, 1.0024408659874415)
(0.525, 1.0338003628555534)
(0.6, 1.0672959559286246)
(0.675, 1.1026568724482801)
(0.75, 1.1398730837938391)
(0.8250000000000001, 1.1793858492752467)
(0.9, 1.2207839954445991)
(0.975, 1.2647093540254533)
(1.05, 1.3546460242887175)
(1.125, 1.5956137220012192)
(1.2, 1.6593155205641381)
(1.2750000000000001, 1.728162001536184)
(1.35, 1.79897409216162)
(1.425, 1.8721228514056265)
(1.5, 1.947207134440981)
(1.575, 2.0248888302326007)
(1.6500000000000001, 2.108377097398265)
(1.725, 2.19510460904375)
(1.8, 2.285191708617223)
(1.875, 2.379390542669725)
(1.95, 2.4779217408562295)
(2.025, 3.367259822808313)
(2.1, 3.542209110580686)
(2.1750000000000003, 3.6518821063432934)
(2.25, 3.745318765224073)
(2.325, 3.8371508447959632)
(2.4, 3.9292737543675895)
(2.475, 4.023592931868259)
(2.5500000000000003, 4.117370563852178)
(2.625, 4.217726971002545)
(2.7, 4.318043263670188)
(2.775, 4.422842349782043)
(2.85, 4.52875461278944)
(2.9250000000000003, 4.637334488897866)
(3.0, 4.7468069122468615)
(3.075, 4.864472718691875)
(3.15, 4.978909309277748)
(3.225, 5.0937470446908435)
(3.3000000000000003, 5.211001677687953)
(3.375, 5.329720489304425)
(3.45, 5.453283124709609)
(3.525, 5.578510511147765)
(3.6, 5.709975699649228)
(3.6750000000000003, 5.84656551331846)
(3.75, 5.989553586981888)
(3.825, 6.142981454773779)
(3.9, 6.307420748072926)
(3.975, 6.503269681343586)
(4.05, 6.802784466589198)
(4.125, 6.9291751730263)
(4.2, 7.057892519461291)
(4.275, 7.189548251755686)
(4.3500000000000005, 7.325375890253194)
(4.425, 7.461023013578452)
(4.5, 7.601824847933518)
(4.575, 7.746136699526779)
(4.65, 7.892614733187042)
(4.7250000000000005, 8.040837746845723)
(4.8, 8.193072208776627)
(4.875, 8.347683453808825)
(4.95, 8.506235946768482)
(5.025, 8.666633705933362)
(5.1000000000000005, 8.835054361642692)
(5.175, 9.001960695629256)
(5.25, 9.175255260989337)
(5.325, 9.353473879103575)
(5.4, 9.536105090317257)
(5.4750000000000005, 9.722747749803164)
(5.55, 9.914474919974115)
(5.625, 10.111928432553665)
(5.7, 10.314656999611191)
(5.775, 10.521908474595648)
(5.8500000000000005, 10.738496595433707)
(5.925, 10.960470085577228)
(6.0, 11.195019466054172)
(6.075, 11.445474238930483)
(6.15, 11.640280195650368)
(6.2250000000000005, 11.838967228573626)
(6.3, 12.042869144250776)
(6.375, 12.248897127512206)
(6.45, 12.460490995251348)
(6.525, 12.674963077125808)
(6.6000000000000005, 12.892684432100774)
(6.675, 13.115530412243501)
(6.75, 13.338817651696175)
(6.825, 13.56853323700509)
(6.9, 13.805118427480187)
(6.9750000000000005, 14.041111929335129)
(7.05, 14.28781599807691)
(7.125, 14.535773644403763)
(7.2, 14.788294313140272)
(7.275, 15.04641095221653)
(7.3500000000000005, 15.309251071633334)
(7.425, 15.57770721863125)
(7.5, 15.853103171140118)
(7.575, 16.13297188847251)
(7.65, 16.415468104423216)
(7.7250000000000005, 16.702527342783572)
(7.8, 16.996325814241263)
(7.875, 17.288349219838498)
(7.95, 17.590792362322833)
(8.025, 17.915719672372983)
(8.1, 18.202427909009522)
(8.175, 18.49286679253923)
(8.25, 18.79324403916337)
(8.325, 19.095165693372316)
(8.4, 19.401550083784112)
(8.475, 19.715636454878577)
(8.55, 20.032039437350253)
(8.625, 20.353376501196767)
(8.700000000000001, 20.682014400898723)
(8.775, 21.011474647496488)
(8.85, 21.3467414654683)
(8.925, 21.68756413929714)
(9.0, 22.040792216907835)
(9.075000000000001, 22.39601599003396)
(9.15, 22.75531138315639)
(9.225, 23.11690333041467)
(9.3, 23.484612736288092)
(9.375, 23.862561363876367)
(9.450000000000001, 24.246396791804127)
(9.525, 24.63283966110884)
(9.6, 25.026733795579204)
(9.675, 25.418371490396442)
(9.75, 25.823788510028773)
(9.825000000000001, 26.224823022423692)
(9.9, 26.63160393446858)
(9.975, 27.04867421133172)
(10.05, 27.48074730473298)
(10.125, 27.89874021469873)
(10.200000000000001, 28.32302106983119)
(10.275, 28.75147383116677)
(10.35, 29.185241761463036)
(10.425, 29.626039754856386)
(10.5, 30.072152917210428)
(10.575000000000001, 30.52800387024529)
(10.65, 30.990022424998703)
(10.725, 31.457667035953907)
(10.8, 31.932512196557756)
(10.875, 32.41598197094688)
(10.950000000000001, 32.901216782575794)
(11.025, 33.39918794246901)
(11.1, 33.89781096270647)
(11.175, 34.40674340500354)
(11.25, 34.915354931438834)
(11.325000000000001, 35.432410556487156)
(11.4, 35.95261516842918)
(11.475, 36.48201602553527)
(11.55, 37.012058714364926)
(11.625, 37.54928189560186)
(11.700000000000001, 38.08561252959822)
(11.775, 38.628020507727)
(11.85, 39.17391844585262)
(11.925, 39.724449606732655)
(12.0, 40.280837482090135)
(12.075000000000001, 40.83970242675572)
(12.15, 41.397263650732825)
(12.225, 41.95032202402436)
(12.3, 42.50980874317214)
(12.375, 43.07148170162828)
(12.450000000000001, 43.635902502150884)
(12.525, 44.19513850578165)
(12.6, 44.75310087458598)
(12.675, 45.31419217304264)
(12.75, 45.87372903529383)
(12.825000000000001, 46.43335615513113)
(12.9, 46.99041594807421)
(12.975, 47.544035924123854)
(13.05, 48.09562009017535)
(13.125, 48.64343349485096)
(13.200000000000001, 49.189792749527875)
(13.275, 49.72999443110694)
(13.35, 50.26681646751665)
(13.425, 50.80309695840961)
(13.5, 51.3338917937903)
(13.575000000000001, 51.85802762503909)
(13.65, 52.382273771115386)
(13.725, 52.90291964236735)
(13.8, 53.42044661258767)
(13.875, 53.93829449866976)
(13.950000000000001, 54.459160999576696)
(14.025, 55.03492417008901)
(14.1, 55.69955094845178)
(14.175, 56.3893295074814)
(14.25, 57.09186447201668)
(14.325000000000001, 57.82198817204419)
(14.4, 58.56745566171296)
(14.475, 59.34157492066608)
(14.55, 60.14148779200962)
(14.625, 60.96938051505191)
(14.700000000000001, 61.848138402186)
(14.775, 66.10095551694982)
(14.85, 76.75490081142573)
(14.925, 88.09786248975952)
};
\addplot[dashed, black, thick, mark = none] coordinates{
(0.0, 0.9132228167000467)
(0.075, 0.9406433190096234)
(0.15, 0.9704456021767475)
(0.225, 1.001518835633403)
(0.3, 1.0346836329523585)
(0.375, 1.070040068959561)
(0.45, 1.1073879940031162)
(0.525, 1.1485487699152657)
(0.6, 1.191460855281494)
(0.675, 1.2365745868185642)
(0.75, 1.2849407501989236)
(0.8250000000000001, 1.3361090087058094)
(0.9, 1.3918807092062735)
(0.975, 1.448933367478864)
(1.05, 1.5597362147677818)
(1.125, 1.8411466253317603)
(1.2, 1.9301131455989644)
(1.2750000000000001, 2.025114177870794)
(1.35, 2.1243383677976024)
(1.425, 2.2247634556357787)
(1.5, 2.328551057625787)
(1.575, 2.4406148477216414)
(1.6500000000000001, 2.5584229328268746)
(1.725, 2.68126478167726)
(1.8, 2.8120225492600817)
(1.875, 2.948104297583303)
(1.95, 3.091011149036134)
(2.025, 4.063898576965998)
(2.1, 4.281621368297076)
(2.1750000000000003, 4.439709570846122)
(2.25, 4.583757275314753)
(2.325, 4.728115211743821)
(2.4, 4.873443873984578)
(2.475, 5.022695469402472)
(2.5500000000000003, 5.176040125201613)
(2.625, 5.334608686915207)
(2.7, 5.497020121945178)
(2.775, 5.665466068979776)
(2.85, 5.8389958171725)
(2.9250000000000003, 6.014527061884171)
(3.0, 6.197413806302973)
(3.075, 6.392709829139247)
(3.15, 6.585894273148033)
(3.225, 6.779138762052386)
(3.3000000000000003, 6.975815817486734)
(3.375, 7.176936195193146)
(3.45, 7.380508406135268)
(3.525, 7.588483909419072)
(3.6, 7.805265997386246)
(3.6750000000000003, 8.028773113657081)
(3.75, 8.259815864321753)
(3.825, 8.503648177742498)
(3.9, 8.757077666971595)
(3.975, 9.041570382174752)
(4.05, 9.430371088462843)
(4.125, 9.651416364015375)
(4.2, 9.874753353082099)
(4.275, 10.102503641973103)
(4.3500000000000005, 10.336188368042786)
(4.425, 10.57376600484182)
(4.5, 10.814916312927176)
(4.575, 11.060279771184915)
(4.65, 11.312488347537455)
(4.7250000000000005, 11.564336654516582)
(4.8, 11.821649046992436)
(4.875, 12.086897373165916)
(4.95, 12.352355856473887)
(5.025, 12.620576404978001)
(5.1000000000000005, 12.903628042687517)
(5.175, 13.181305662243659)
(5.25, 13.462355803434228)
(5.325, 13.7460579275124)
(5.4, 14.03535423436103)
(5.4750000000000005, 14.326702075141585)
(5.55, 14.623574046314431)
(5.625, 14.926780753969743)
(5.7, 15.233800312493651)
(5.775, 15.547845123799064)
(5.8500000000000005, 15.86954565928945)
(5.925, 16.19391819263263)
(6.0, 16.524595440010494)
(6.075, 16.871424764296265)
(6.15, 17.17076858367001)
(6.2250000000000005, 17.47143339074626)
(6.3, 17.771537778797207)
(6.375, 18.075214838134475)
(6.45, 18.380553139582464)
(6.525, 18.689324007560455)
(6.6000000000000005, 18.999175683658674)
(6.675, 19.309587778782195)
(6.75, 19.623962837013234)
(6.825, 19.94306142702899)
(6.9, 20.2599583708739)
(6.9750000000000005, 20.58032791117919)
(7.05, 20.910855046318133)
(7.125, 21.23875021353466)
(7.2, 21.56734590453282)
(7.275, 21.899504259334705)
(7.3500000000000005, 22.233594058277372)
(7.425, 22.573268032507908)
(7.5, 22.913732597863422)
(7.575, 23.255348023717335)
(7.65, 23.602877871784735)
(7.7250000000000005, 23.948396215850593)
(7.8, 24.29987901954291)
(7.875, 24.647839189361886)
(7.95, 24.99294722664136)
(8.025, 25.361192563679865)
(8.1, 25.69646324556871)
(8.175, 26.03181398731832)
(8.25, 26.36762507326728)
(8.325, 26.705167453705137)
(8.4, 27.046902969350185)
(8.475, 27.388708537373397)
(8.55, 27.734867360325318)
(8.625, 28.079044701723475)
(8.700000000000001, 28.42402264172922)
(8.775, 28.772463170712744)
(8.85, 29.12335553293197)
(8.925, 29.475739010057822)
(9.0, 29.830674395245328)
(9.075000000000001, 30.189622780953318)
(9.15, 30.545138600131317)
(9.225, 30.905578100745927)
(9.3, 31.26446644155835)
(9.375, 31.62747786519981)
(9.450000000000001, 31.988117515466314)
(9.525, 32.34969786909672)
(9.6, 32.71727270480138)
(9.675, 33.081324906632695)
(9.75, 33.447478679808896)
(9.825000000000001, 33.81425291690597)
(9.9, 34.17380175156965)
(9.975, 34.53548218002601)
(10.05, 34.90890138556599)
(10.125, 35.26690906791007)
(10.200000000000001, 35.62822922699303)
(10.275, 35.98926917656332)
(10.35, 36.3522405702744)
(10.425, 36.71332054977507)
(10.5, 37.07424040955422)
(10.575000000000001, 37.43762211005169)
(10.65, 37.79999305480708)
(10.725, 38.16323465054822)
(10.8, 38.531850264442724)
(10.875, 38.897753850554054)
(10.950000000000001, 39.26676976375236)
(11.025, 39.63466483890004)
(11.1, 40.005061784696416)
(11.175, 40.376049171965875)
(11.25, 40.74973857953592)
(11.325000000000001, 41.11704321321052)
(11.4, 41.49265405743875)
(11.475, 41.86533270926672)
(11.55, 42.235419423102655)
(11.625, 42.60588642127719)
(11.700000000000001, 42.97633340448653)
(11.775, 43.34552945237154)
(11.85, 43.71889862049855)
(11.925, 44.089966067628765)
(12.0, 44.46026293859919)
(12.075000000000001, 44.84107767377668)
(12.15, 45.21267551748443)
(12.225, 45.58376297957983)
(12.3, 45.95780264904069)
(12.375, 46.32883006624053)
(12.450000000000001, 46.70458101522508)
(12.525, 47.07748983915273)
(12.6, 47.45247021197749)
(12.675, 47.83039278468511)
(12.75, 48.208685634248724)
(12.825000000000001, 48.59138177615403)
(12.9, 48.97563908534411)
(12.975, 49.362458310078445)
(13.05, 49.75161928573995)
(13.125, 50.144963389126055)
(13.200000000000001, 50.53743684152641)
(13.275, 50.929149725249566)
(13.35, 51.32481556459765)
(13.425, 51.72268305011657)
(13.5, 52.12825629723344)
(13.575000000000001, 52.53857309110022)
(13.65, 52.95027091756507)
(13.725, 53.37287690005817)
(13.8, 53.794241954709534)
(13.875, 54.22271232200316)
(13.950000000000001, 54.6604796406273)
(14.025, 55.169440190430386)
(14.1, 55.79581853351752)
(14.175, 56.45075823193001)
(14.25, 57.12428182552094)
(14.325000000000001, 57.81962173116839)
(14.4, 58.54351298465863)
(14.475, 59.30812468482684)
(14.55, 60.105390800701684)
(14.625, 60.933720142550584)
(14.700000000000001, 61.80875440566912)
(14.775, 66.05816168749374)
(14.85, 76.73958819008972)
(14.925, 88.14040257900832)
};
