# Supplementary material for: CausalSim: A Causal Framework for Unbiased Trace-Driven Simulation
Source: arXiv:2201.01811 source file (2023-05-05)
Supplement: Supplementary file 6 [file new_bola_basic_v2_linear_bba.tex]

\addplot[solid, green!70!black, thick, mark = none] coordinates{
(0.0, 0.4098454260573601)
(0.07846738601242167, 0.4179893200790416)
(0.15693477202484335, 0.4311345819748368)
(0.23540215803726505, 0.4522486900167196)
(0.3138695440496867, 0.48435747176852867)
(0.3923369300621084, 0.5337043014597826)
(0.4708043160745301, 0.612550865995183)
(0.5492717020869518, 0.7368015152144111)
(0.6277390880993734, 0.9188262989927745)
(0.7062064741117952, 1.1498144742587098)
(0.7846738601242168, 1.4468207054629443)
(0.8631412461366385, 1.8314842442741424)
(0.9416086321490602, 2.238962356204422)
(1.0200760181614819, 2.5476717882340822)
(1.0985434041739035, 2.804875466773496)
(1.1770107901863252, 3.0226433596255244)
(1.2554781761987468, 3.2074105601215264)
(1.3339455622111687, 3.383758791362771)
(1.4124129482235903, 3.5564643596690364)
(1.490880334236012, 3.7195589660438797)
(1.5693477202484336, 3.8736010965665777)
(1.6478151062608553, 4.032211143080966)
(1.726282492273277, 4.195714194498862)
(1.8047498782856985, 4.3730877061543)
(1.8832172642981204, 4.561639275008381)
(1.961684650310542, 4.770504733044487)
(2.0401520363229637, 4.94133478839796)
(2.1186194223353856, 5.086666203206577)
(2.197086808347807, 5.2236453336654245)
(2.275554194360229, 5.3568400957661915)
(2.3540215803726503, 5.489217967780855)
(2.432488966385072, 5.621070696168736)
(2.5109563523974936, 5.753356876439039)
(2.5894237384099155, 5.88639326189046)
(2.6678911244223373, 6.015003436773291)
(2.7463585104347588, 6.146406042052501)
(2.8248258964471806, 6.278625537417818)
(2.903293282459602, 6.415479633679812)
(2.981760668472024, 6.549724683034143)
(3.0602280544844453, 6.686120320574345)
(3.138695440496867, 6.822424266370186)
(3.217162826509289, 6.960653738797561)
(3.2956302125217105, 7.099575067114189)
(3.3740975985341324, 7.240897052010392)
(3.452564984546554, 7.382677495628388)
(3.5310323705589757, 7.530726320315273)
(3.609499756571397, 7.681300835778586)
(3.687967142583819, 7.8327755974592375)
(3.766434528596241, 7.987426227739953)
(3.8449019146086623, 8.142260241509385)
(3.923369300621084, 8.299278185917181)
(4.001836686633506, 8.454687356992137)
(4.080304072645927, 8.609104590105394)
(4.158771458658349, 8.760220920421736)
(4.237238844670771, 8.90751120431438)
(4.315706230683192, 9.054943193630125)
(4.394173616695614, 9.204384065708638)
(4.472641002708036, 9.354066670567732)
(4.551108388720458, 9.5039159876893)
(4.629575774732879, 9.659416850508615)
(4.708043160745301, 9.81835198593482)
(4.7865105467577225, 9.976286847786204)
(4.864977932770144, 10.136914112676482)
(4.943445318782566, 10.298399945718488)
(5.021912704794987, 10.463970229191018)
(5.100380090807409, 10.629915615254106)
(5.178847476819831, 10.799453650573431)
(5.257314862832253, 10.973559601884448)
(5.335782248844675, 11.151424914714173)
(5.414249634857096, 11.3299987546594)
(5.4927170208695175, 11.51130667570914)
(5.571184406881939, 11.695515390125866)
(5.649651792894361, 11.883300082572584)
(5.728119178906782, 12.074018910838781)
(5.806586564919204, 12.27053932583895)
(5.885053950931626, 12.46604279603805)
(5.963521336944048, 12.668939955077713)
(6.04198872295647, 12.875029653943686)
(6.120456108968891, 13.082969858923082)
(6.198923494981313, 13.294419357027481)
(6.277390880993734, 13.510070004146135)
(6.355858267006156, 13.727712862801308)
(6.434325653018578, 13.949423500660766)
(6.512793039030999, 14.169567043252995)
(6.591260425043421, 14.394403536033773)
(6.669727811055843, 14.62109053492797)
(6.748195197068265, 14.849686389227454)
(6.826662583080687, 15.0820249338194)
(6.905129969093108, 15.316614093954698)
(6.9835973551055295, 15.555821183760424)
(7.062064741117951, 15.799821251112178)
(7.140532127130373, 16.046463707824092)
(7.218999513142794, 16.29559017724681)
(7.297466899155216, 16.548842775165674)
(7.375934285167638, 16.80565467988828)
(7.45440167118006, 17.06944349279528)
(7.532869057192482, 17.335732989639332)
(7.611336443204903, 17.602997753218837)
(7.6898038292173245, 17.878481431338137)
(7.768271215229746, 18.156657512496334)
(7.846738601242168, 18.44074354335911)
(7.92520598725459, 18.730514462372124)
(8.003673373267011, 19.021327333025585)
(8.082140759279433, 19.31529106543973)
(8.160608145291855, 19.617648760269265)
(8.239075531304277, 19.92460771354299)
(8.317542917316699, 20.23431741914747)
(8.39601030332912, 20.54752808226383)
(8.474477689341542, 20.868365831388218)
(8.552945075353962, 21.19002880621183)
(8.631412461366384, 21.51778511422874)
(8.709879847378806, 21.849025708531283)
(8.788347233391228, 22.187935066907468)
(8.86681461940365, 22.528144780930916)
(8.945282005416072, 22.875848211152416)
(9.023749391428494, 23.224460223204378)
(9.102216777440916, 23.58342506675576)
(9.180684163453337, 23.942873375868302)
(9.259151549465757, 24.305547567259644)
(9.33761893547818, 24.675873851498384)
(9.416086321490601, 25.04617512889775)
(9.494553707503023, 25.42784618259761)
(9.573021093515445, 25.811442762928994)
(9.651488479527867, 26.19809851327671)
(9.729955865540289, 26.592631418026162)
(9.80842325155271, 26.995374901702284)
(9.886890637565132, 27.40031898724301)
(9.965358023577554, 27.812306665873116)
(10.043825409589974, 28.23285501918108)
(10.122292795602396, 28.655620645579898)
(10.200760181614818, 29.085404858228724)
(10.27922756762724, 29.522632773396857)
(10.357694953639662, 29.968754787767786)
(10.436162339652084, 30.42057836151521)
(10.514629725664506, 30.876086276263226)
(10.593097111676927, 31.340404934082805)
(10.67156449768935, 31.813767732141407)
(10.75003188370177, 32.29299880183897)
(10.828499269714191, 32.780198717682616)
(10.906966655726613, 33.27320022026024)
(10.985434041739035, 33.77341202818971)
(11.063901427751457, 34.280925833215385)
(11.142368813763879, 34.79750044970633)
(11.2208361997763, 35.324352877178576)
(11.299303585788723, 35.8530057970855)
(11.377770971801144, 36.39617935505361)
(11.456238357813564, 36.94949735419304)
(11.534705743825986, 37.508650282518936)
(11.613173129838408, 38.076472248493296)
(11.69164051585083, 38.654138573566534)
(11.770107901863252, 39.23916524502785)
(11.848575287875674, 39.832810940458884)
(11.927042673888096, 40.43085783961914)
(12.005510059900518, 41.04159987756651)
(12.08397744591294, 41.65756834494234)
(12.162444831925361, 42.28609858129532)
(12.240912217937781, 42.91673772776854)
(12.319379603950203, 43.554937275344805)
(12.397846989962625, 44.199521902573686)
(12.476314375975047, 44.85369248489462)
(12.554781761987469, 45.50834653277672)
(12.63324914799989, 46.167835236270456)
(12.711716534012313, 46.83066652062672)
(12.790183920024734, 47.49949944643193)
(12.868651306037156, 48.167115372721106)
(12.947118692049576, 48.8350563879221)
(13.025586078061998, 49.502372232138825)
(13.10405346407442, 50.17187200699391)
(13.182520850086842, 50.847123354904234)
(13.260988236099264, 51.516548109241214)
(13.339455622111686, 52.18181339262955)
(13.417923008124108, 52.84905421632816)
(13.49639039413653, 53.51046011084032)
(13.574857780148951, 54.16446398089878)
(13.653325166161373, 54.820043281837584)
(13.731792552173793, 55.469295852415634)
(13.810259938186215, 56.118740142095525)
(13.888727324198637, 56.76116584552542)
(13.967194710211059, 57.40201611807496)
(14.04566209622348, 58.03590615366636)
(14.124129482235903, 58.67037968217641)
(14.202596868248325, 59.30778734650593)
(14.281064254260746, 59.951796816429294)
(14.359531640273168, 60.62278033042037)
(14.437999026285588, 61.33517517040911)
(14.51646641229801, 62.121106789373556)
(14.594933798310432, 63.037957548056056)
(14.673401184322854, 64.13701647400563)
(14.751868570335276, 65.5587886620324)
(14.830335956347698, 67.97299061293263)
(14.90880334236012, 95.83027624722028)
(14.987270728372541, 99.88113415685856)
(15.065738114384963, 99.99416507081354)
(15.144205500397385, 99.9981911719522)
(15.222672886409805, 99.99935815778949)
(15.301140272422227, 99.9997499316063)
(15.379607658434649, 99.99988330141628)
(15.458075044447071, 99.99994165070814)
(15.536542430459493, 99.99997499316063)
(15.615009816471915, 99.99998332877375)
};
\addplot[solid, blue, thick, mark = none] coordinates{
(0.0, 0.4149718813619992)
(0.075, 0.4149718813619992)
(0.15, 0.4149893593816416)
(0.225, 0.4149980983914629)
(0.3, 0.41500683740128413)
(0.375, 0.41500683740128413)
(0.45, 0.41500683740128413)
(0.525, 0.41501557641110537)
(0.6, 0.41502431542092666)
(0.675, 0.4150330544307479)
(0.75, 0.4150417934405692)
(0.8250000000000001, 0.4150592714602116)
(0.9, 0.4150592714602116)
(0.975, 0.4150592714602116)
(1.05, 0.41506801047003283)
(1.125, 0.4151029665093179)
(1.2, 0.4151029665093179)
(1.2750000000000001, 0.4151291835387816)
(1.35, 0.4151379225486028)
(1.425, 0.41515540056824535)
(1.5, 0.41518161759770916)
(1.575, 0.4152165736369941)
(1.6500000000000001, 0.4152602686861004)
(1.725, 0.4152777467057428)
(1.8, 0.4153651368039553)
(1.875, 0.4154437878923466)
(1.95, 0.41547000492181035)
(2.025, 4.371672185060069)
(2.1, 4.484685060068458)
(2.1750000000000003, 4.5967541220161525)
(2.25, 4.711645884136111)
(2.325, 4.83158879393275)
(2.4, 4.954634052215933)
(2.475, 5.080659312848161)
(2.5500000000000003, 5.207217653079487)
(2.625, 5.3403739457258546)
(2.7, 5.475636339739144)
(2.775, 5.614219557484508)
(2.85, 5.756656678561042)
(2.9250000000000003, 5.902938963958925)
(3.0, 6.051274916664803)
(3.075, 6.205579613078592)
(3.15, 6.363441086489631)
(3.225, 6.526301273518423)
(3.3000000000000003, 6.6954797646479784)
(3.375, 6.867821777332826)
(3.45, 7.046053882637196)
(3.525, 7.2302285146200145)
(3.6, 7.4222420384124925)
(3.6750000000000003, 7.6217711106512445)
(3.75, 7.828710863218416)
(3.825, 8.05147696257187)
(3.9, 8.28107696760554)
(3.975, 8.473256532584623)
(4.05, 8.628426390970716)
(4.125, 8.785955782008546)
(4.2, 8.945224236000806)
(4.275, 9.108617502628693)
(4.3500000000000005, 9.275279158929731)
(4.425, 9.445025685697667)
(4.5, 9.61580341562451)
(4.575, 9.791571120159286)
(4.65, 9.970712082485067)
(4.7250000000000005, 10.154904192487528)
(4.8, 10.343509502449718)
(4.875, 10.53728830622609)
(4.95, 10.730166991990872)
(5.025, 10.927694830980558)
(5.1000000000000005, 11.132379919013848)
(5.175, 11.339442017718516)
(5.25, 11.552848637553414)
(5.325, 11.771874440703371)
(5.4, 11.991975142061344)
(5.4750000000000005, 12.220561421955749)
(5.55, 12.454181371507191)
(5.625, 12.694102147139757)
(5.7, 12.938313776594553)
(5.775, 13.191211981811673)
(5.8500000000000005, 13.44079810230654)
(5.925, 13.677974828855232)
(6.0, 13.900819579297078)
(6.075, 14.12576169209602)
(6.15, 14.354540230206492)
(6.2250000000000005, 14.587854314414193)
(6.3, 14.82262781326204)
(6.375, 15.064156566701717)
(6.45, 15.309032360902927)
(6.525, 15.558094140808521)
(6.6000000000000005, 15.810039793955122)
(6.675, 16.066931726660552)
(6.75, 16.325859848654332)
(6.825, 16.59057319514978)
(6.9, 16.863116694445065)
(6.9750000000000005, 17.139129580639388)
(7.05, 17.41682909572921)
(7.125, 17.700034187006423)
(7.2, 17.986848489339806)
(7.275, 18.281527900512316)
(7.3500000000000005, 18.58196631915703)
(7.425, 18.88645089934898)
(7.5, 19.196292492561355)
(7.575, 19.507427459227277)
(7.65, 19.82411169712969)
(7.7250000000000005, 20.143269074811517)
(7.8, 20.462714839817444)
(7.875, 20.78136535492964)
(7.95, 21.09340917861697)
(8.025, 21.408013532181926)
(8.1, 21.72418216850489)
(8.175, 22.048748993266067)
(8.25, 22.376846377995033)
(8.325, 22.70907731436945)
(8.4, 23.04532819526164)
(8.475, 23.38319579297076)
(8.55, 23.72790603536992)
(8.625, 24.080053175126963)
(8.700000000000001, 24.434533630506277)
(8.775, 24.794318664847086)
(8.85, 25.161863939909168)
(8.925, 25.532642648605115)
(9.0, 25.907013090337593)
(9.075000000000001, 26.288348522897603)
(9.15, 26.67497105639947)
(9.225, 27.066094179959283)
(9.3, 27.46760798619656)
(9.375, 27.870004432425784)
(9.450000000000001, 28.276595603369202)
(9.525, 28.689216691089285)
(9.6, 29.1072384868789)
(9.675, 29.531631020828208)
(9.75, 29.952300736593664)
(9.825000000000001, 30.37476194937247)
(9.9, 30.80319190585919)
(9.975, 31.23222485402358)
(10.05, 31.661651057629925)
(10.125, 32.10242923499408)
(10.200000000000001, 32.54694770856171)
(10.275, 32.997207711581915)
(10.35, 33.45639024362961)
(10.425, 33.91706714635674)
(10.5, 34.388414380075616)
(10.575000000000001, 34.86615856898364)
(10.65, 35.344767919863976)
(10.725, 35.83492150271818)
(10.8, 36.329811628895506)
(10.875, 36.82587278238887)
(10.950000000000001, 37.33161675876418)
(11.025, 37.841651588961724)
(11.1, 38.358834929193044)
(11.175, 38.880457686413564)
(11.25, 39.40583821785722)
(11.325000000000001, 39.93418127363028)
(11.4, 40.467776474305914)
(11.475, 41.00652769077608)
(11.55, 41.54648489060158)
(11.625, 42.08481663460032)
(11.700000000000001, 42.628811256963246)
(11.775, 43.1711367284503)
(11.85, 43.716153814962304)
(11.925, 44.259606618716305)
(12.0, 44.80583842759346)
(12.075000000000001, 45.35135363766527)
(12.15, 45.90018093245934)
(12.225, 46.4515949741605)
(12.3, 47.003760570706284)
(12.375, 47.55156540135126)
(12.450000000000001, 48.097377737757)
(12.525, 48.64390667296807)
(12.6, 49.18913349571579)
(12.675, 49.73099579968232)
(12.75, 50.26863716190518)
(12.825000000000001, 50.803298521779006)
(12.9, 51.33504979138236)
(12.975, 51.86070123213047)
(13.05, 52.382516247567054)
(13.125, 52.89953354661178)
(13.200000000000001, 53.41078309917447)
(13.275, 53.919043910378306)
(13.35, 54.421563192129575)
(13.425, 54.918332205418466)
(13.5, 55.406799159377165)
(13.575000000000001, 55.89045965793418)
(13.65, 56.37212766225195)
(13.725, 56.84556351931811)
(13.8, 57.31539016532808)
(13.875, 57.78068126524083)
(13.950000000000001, 58.244644035660755)
(14.025, 58.70595888610484)
(14.1, 59.1744659416318)
(14.175, 59.63918026689635)
(14.25, 60.10523166066355)
(14.325000000000001, 60.58057262187073)
(14.4, 61.05782742622877)
(14.475, 61.546853676816035)
(14.55, 62.045781225530774)
(14.625, 62.55637535235687)
(14.700000000000001, 63.08246374359605)
(14.775, 63.63095895601691)
(14.85, 64.21061747746035)
(14.925, 64.82271520336026)
};
\addplot[solid, red, thick, mark = none] coordinates{

(0.0031690185597714644,0.5579192575836157)
(0.3200708745369179,0.7789213683275709)
(0.6369727305140643,1.5498822261221779)
(0.9538745864912108,2.6731394369693446)
(1.2707764424683572,3.6700954377688966)
(1.5876782984455038,4.577060159286899)
(1.9045801544226502,5.583593779565378)
(2.2214820103997965,6.486857488856536)
(2.538383866376943,7.238604758401424)
(2.8552857223540897,7.966803920872359)
(3.1721875783312363,8.706172804928816)
(3.489089434308382,9.482326749699375)
(3.8059912902855286,10.310820009272536)
(4.122893146262675,11.091066740086747)
(4.439795002239822,11.868237629658378)
(4.7566968582169675,12.684152449028144)
(5.073598714194114,13.554415465963274)
(5.390500570171261,14.487012197836108)
(5.707402426148407,15.46738032851985)
(6.024304282125554,16.451566170014164)
(6.3412061381027005,17.474729338474074)
(6.658107994079847,18.55012345876597)
(6.975009850056994,19.67498944294598)
(7.29191170603414,20.862664272011727)
(7.608813562011286,22.103878744169865)
(7.925715417988433,23.390797383084276)
(8.242617273965578,24.732089226403424)
(8.559519129942725,26.138915660099705)
(8.876420985919871,27.623938480507753)
(9.193322841897018,29.195885074567897)
(9.510224697874165,30.84613641831041)
(9.827126553851311,32.575909511251325)
(10.144028409828458,34.39476530164333)
(10.460930265805604,36.29075885588042)
(10.777832121782751,38.274126306878266)
(11.094733977759898,40.339924636054626)
(11.411635833737044,42.47746758738515)
(11.72853768971419,44.67781938360142)
(12.045439545691337,46.926367694897884)
(12.362341401668484,49.202840310158166)
(12.67924325764563,51.47952965135965)
(12.996145113622775,53.72597738814899)
(13.313046969599922,55.92306995963396)
(13.629948825577069,58.038156769209714)
(13.946850681554213,60.0777062526601)
(14.26375253753136,62.176338561930024)
(14.580654393508507,64.79759714281856)
(14.897556249485653,93.59944944942443)
(15.2144581054628,99.99627398093378)
(15.531359961439946,99.99745763799733)
(15.848261817417093,99.99774938445665)
(16.16516367339424,99.99789942549288)
(16.482065529371386,99.99799111723723)
(16.798967385348533,99.99817450072595)
(17.11586924132568,99.99829119930968)
(17.432771097302826,99.99841623350653)
(17.749672953279973,99.99857461015587)
(18.06657480925712,99.99874132241835)
(18.383476665234266,99.99880800732333)
(18.700378521211412,99.99888302784144)
(19.017280377188555,99.99894971274644)
(19.334182233165706,99.99901639765142)
(19.65108408914285,99.99907474694328)
(19.96798594512,99.9991164250089)
(20.284887801097142,99.99922478797951)
(20.601789657074292,99.99931647972387)
(20.918691513051435,99.99933315095012)
(21.235593369028585,99.99937482901574)
(21.55249522500573,99.9993998358551)
(21.86939708098288,99.99944151392073)
(22.18629893696002,99.99948319198634)
(22.50320079293717,99.99950819882571)
(22.820102648914315,99.99953320566507)
(23.13700450489146,99.99954987689132)
(23.453906360868608,99.9995748837307)
(23.770808216845754,99.99959989057007)
(24.0877100728229,99.99960822618318)
(24.404611928800048,99.99963323302256)
(24.721513784777194,99.99964990424881)
(25.03841564075434,99.99966657547506)
(25.355317496731487,99.99968324670131)
(25.672219352708634,99.99968324670131)
(25.98912120868578,99.99970825354067)
(26.306023064662924,99.99973326038005)
(26.622924920640074,99.99973326038005)
(26.939826776617217,99.99976660283254)
(27.256728632594367,99.99978327405879)
(27.57363048857151,99.99978327405879)
(27.89053234454866,99.99980828089816)
(28.207434200525803,99.99980828089816)
(28.524336056502953,99.99981661651128)
(28.841237912480096,99.9998249521244)
(29.158139768457247,99.99984162335065)
(29.47504162443439,99.99984995896376)
(29.79194348041154,99.99984995896376)
(30.108845336388683,99.99984995896376)
(30.42574719236583,99.99984995896376)
(30.742649048342976,99.99984995896376)
(31.059550904320123,99.99986663019003)
(31.37645276029727,99.99986663019003)
(31.693354616274416,99.99986663019003)
(32.01025647225156,99.99986663019003)
(32.327158328228705,99.99986663019003)
(32.644060184205856,99.99986663019003)
(32.960962040183006,99.99986663019003)
(33.27786389616015,99.99986663019003)
(33.59476575213729,99.99986663019003)
(33.91166760811444,99.99986663019003)
(34.22856946409159,99.99986663019003)
(34.54547132006873,99.99986663019003)
(34.86237317604588,99.99986663019003)
(35.17927503202303,99.99987496580314)
(35.49617688800018,99.99989163702939)
(35.813078743977314,99.99989163702939)
(36.129980599954465,99.99989163702939)
(36.446882455931615,99.99989997264251)
(36.763784311908765,99.99991664386877)
(37.0806861678859,99.99991664386877)
(37.39758802386305,99.99991664386877)
(37.7144898798402,99.99991664386877)
(38.031391735817344,99.99991664386877)
(38.34829359179449,99.99992497948189)
(38.66519544777164,99.99992497948189)
(38.98209730374879,99.99992497948189)
(39.29899915972593,99.99992497948189)
(39.61590101570307,99.99992497948189)
(39.932802871680224,99.99992497948189)
(40.249704727657374,99.999933315095)
(40.56660658363452,99.99994998632125)
(40.88350843961166,99.99994998632125)
(41.20041029558881,99.99994998632125)
(41.51731215156596,99.99994998632125)
(41.834214007543096,99.99994998632125)
(42.151115863520246,99.99994998632125)
(42.4680177194974,99.99994998632125)
(42.78491957547455,99.99994998632125)
(43.10182143145168,99.99994998632125)
(43.41872328742883,99.99994998632125)
(43.73562514340598,99.99994998632125)
(44.05252699938313,99.99994998632125)
(44.36942885536027,99.99994998632125)
(44.68633071133742,99.99994998632125)
(45.00323256731457,99.99994998632125)
(45.32013442329171,99.99994998632125)
(45.637036279268855,99.99994998632125)
(45.953938135246005,99.99994998632125)
(46.270839991223156,99.99995832193437)
(46.5877418472003,99.9999666575475)
(46.90464370317744,99.9999666575475)
(47.22154555915459,99.9999666575475)
(47.53844741513174,99.9999666575475)
(47.855349271108885,99.9999666575475)
(48.17225112708603,99.9999666575475)
(48.48915298306318,99.9999666575475)
(48.80605483904033,99.9999666575475)
(49.122956695017464,99.9999666575475)
(49.439858550994614,99.9999666575475)
(49.756760406971765,99.9999666575475)
(50.073662262948915,99.9999666575475)
(50.39056411892605,99.9999666575475)
(50.7074659749032,99.99997499316063)
(51.02436783088035,99.99997499316063)
(51.3412696868575,99.99998332877375)
(51.65817154283464,99.99998332877375)
(51.97507339881179,99.99998332877375)
(52.29197525478894,99.99998332877375)
(52.60887711076608,99.99998332877375)
(52.92577896674322,99.99998332877375)
(53.242680822720374,99.99998332877375)
(53.559582678697524,99.99998332877375)
(53.87648453467467,99.99998332877375)
(54.19338639065181,99.99998332877375)
(54.51028824662896,99.99998332877375)
(54.82719010260611,99.99998332877375)
(55.14409195858325,99.99998332877375)
(55.460993814560396,99.99998332877375)
(55.777895670537546,99.99998332877375)
(56.0947975265147,99.99998332877375)
(56.41169938249183,99.99998332877375)
(56.72860123846898,99.99998332877375)
(57.04550309444613,99.99998332877375)
(57.36240495042328,99.99998332877375)
(57.67930680640042,99.99998332877375)
(57.99620866237757,99.99998332877375)
(58.31311051835472,99.99998332877375)
(58.63001237433187,99.99998332877375)
(58.946914230309005,99.99998332877375)
(59.263816086286155,99.99998332877375)
(59.580717942263306,99.99998332877375)
(59.89761979824045,99.99998332877375)
(60.21452165421759,99.99998332877375)
(60.53142351019474,99.99998332877375)
(60.84832536617189,99.99998332877375)
(61.165227222149035,99.99998332877375)
(61.48212907812618,99.99998332877375)
(61.79903093410333,99.99998332877375)
(62.11593279008048,99.99998332877375)
(62.43283464605762,99.99999166438688)
(62.749736502034764,99.99999166438688)
(63.066638358011915,99.99999166438688)
};
\addplot[dashed, magenta, thick, mark = none] coordinates{
(0.0, 0.845713581991646)
(0.075, 0.868949896108504)
(0.15, 0.8929784712591263)
(0.225, 0.9178795364089575)
(0.3, 0.9438035208682057)
(0.375, 0.9720441167046635)
(0.45, 1.0024408659874415)
(0.525, 1.0338003628555534)
(0.6, 1.0672959559286246)
(0.675, 1.1026568724482801)
(0.75, 1.1398730837938391)
(0.8250000000000001, 1.1793858492752467)
(0.9, 1.2207839954445991)
(0.975, 1.2647093540254533)
(1.05, 1.3546460242887175)
(1.125, 1.5956137220012192)
(1.2, 1.6593155205641381)
(1.2750000000000001, 1.728162001536184)
(1.35, 1.79897409216162)
(1.425, 1.8721228514056265)
(1.5, 1.947207134440981)
(1.575, 2.0248888302326007)
(1.6500000000000001, 2.108377097398265)
(1.725, 2.19510460904375)
(1.8, 2.285191708617223)
(1.875, 2.379390542669725)
(1.95, 2.4779217408562295)
(2.025, 3.367259822808313)
(2.1, 3.542209110580686)
(2.1750000000000003, 3.6518821063432934)
(2.25, 3.745318765224073)
(2.325, 3.8371508447959632)
(2.4, 3.9292737543675895)
(2.475, 4.023592931868259)
(2.5500000000000003, 4.117370563852178)
(2.625, 4.217726971002545)
(2.7, 4.318043263670188)
(2.775, 4.422842349782043)
(2.85, 4.52875461278944)
(2.9250000000000003, 4.637334488897866)
(3.0, 4.7468069122468615)
(3.075, 4.864472718691875)
(3.15, 4.978909309277748)
(3.225, 5.0937470446908435)
(3.3000000000000003, 5.211001677687953)
(3.375, 5.329720489304425)
(3.45, 5.453283124709609)
(3.525, 5.578510511147765)
(3.6, 5.709975699649228)
(3.6750000000000003, 5.84656551331846)
(3.75, 5.989553586981888)
(3.825, 6.142981454773779)
(3.9, 6.307420748072926)
(3.975, 6.503269681343586)
(4.05, 6.802784466589198)
(4.125, 6.9291751730263)
(4.2, 7.057892519461291)
(4.275, 7.189548251755686)
(4.3500000000000005, 7.325375890253194)
(4.425, 7.461023013578452)
(4.5, 7.601824847933518)
(4.575, 7.746136699526779)
(4.65, 7.892614733187042)
(4.7250000000000005, 8.040837746845723)
(4.8, 8.193072208776627)
(4.875, 8.347683453808825)
(4.95, 8.506235946768482)
(5.025, 8.666633705933362)
(5.1000000000000005, 8.835054361642692)
(5.175, 9.001960695629256)
(5.25, 9.175255260989337)
(5.325, 9.353473879103575)
(5.4, 9.536105090317257)
(5.4750000000000005, 9.722747749803164)
(5.55, 9.914474919974115)
(5.625, 10.111928432553665)
(5.7, 10.314656999611191)
(5.775, 10.521908474595648)
(5.8500000000000005, 10.738496595433707)
(5.925, 10.960470085577228)
(6.0, 11.195019466054172)
(6.075, 11.445474238930483)
(6.15, 11.640280195650368)
(6.2250000000000005, 11.838967228573626)
(6.3, 12.042869144250776)
(6.375, 12.248897127512206)
(6.45, 12.460490995251348)
(6.525, 12.674963077125808)
(6.6000000000000005, 12.892684432100774)
(6.675, 13.115530412243501)
(6.75, 13.338817651696175)
(6.825, 13.56853323700509)
(6.9, 13.805118427480187)
(6.9750000000000005, 14.041111929335129)
(7.05, 14.28781599807691)
(7.125, 14.535773644403763)
(7.2, 14.788294313140272)
(7.275, 15.04641095221653)
(7.3500000000000005, 15.309251071633334)
(7.425, 15.57770721863125)
(7.5, 15.853103171140118)
(7.575, 16.13297188847251)
(7.65, 16.415468104423216)
(7.7250000000000005, 16.702527342783572)
(7.8, 16.996325814241263)
(7.875, 17.288349219838498)
(7.95, 17.590792362322833)
(8.025, 17.915719672372983)
(8.1, 18.202427909009522)
(8.175, 18.49286679253923)
(8.25, 18.79324403916337)
(8.325, 19.095165693372316)
(8.4, 19.401550083784112)
(8.475, 19.715636454878577)
(8.55, 20.032039437350253)
(8.625, 20.353376501196767)
(8.700000000000001, 20.682014400898723)
(8.775, 21.011474647496488)
(8.85, 21.3467414654683)
(8.925, 21.68756413929714)
(9.0, 22.040792216907835)
(9.075000000000001, 22.39601599003396)
(9.15, 22.75531138315639)
(9.225, 23.11690333041467)
(9.3, 23.484612736288092)
(9.375, 23.862561363876367)
(9.450000000000001, 24.246396791804127)
(9.525, 24.63283966110884)
(9.6, 25.026733795579204)
(9.675, 25.418371490396442)
(9.75, 25.823788510028773)
(9.825000000000001, 26.224823022423692)
(9.9, 26.63160393446858)
(9.975, 27.04867421133172)
(10.05, 27.48074730473298)
(10.125, 27.89874021469873)
(10.200000000000001, 28.32302106983119)
(10.275, 28.75147383116677)
(10.35, 29.185241761463036)
(10.425, 29.626039754856386)
(10.5, 30.072152917210428)
(10.575000000000001, 30.52800387024529)
(10.65, 30.990022424998703)
(10.725, 31.457667035953907)
(10.8, 31.932512196557756)
(10.875, 32.41598197094688)
(10.950000000000001, 32.901216782575794)
(11.025, 33.39918794246901)
(11.1, 33.89781096270647)
(11.175, 34.40674340500354)
(11.25, 34.915354931438834)
(11.325000000000001, 35.432410556487156)
(11.4, 35.95261516842918)
(11.475, 36.48201602553527)
(11.55, 37.012058714364926)
(11.625, 37.54928189560186)
(11.700000000000001, 38.08561252959822)
(11.775, 38.628020507727)
(11.85, 39.17391844585262)
(11.925, 39.724449606732655)
(12.0, 40.280837482090135)
(12.075000000000001, 40.83970242675572)
(12.15, 41.397263650732825)
(12.225, 41.95032202402436)
(12.3, 42.50980874317214)
(12.375, 43.07148170162828)
(12.450000000000001, 43.635902502150884)
(12.525, 44.19513850578165)
(12.6, 44.75310087458598)
(12.675, 45.31419217304264)
(12.75, 45.87372903529383)
(12.825000000000001, 46.43335615513113)
(12.9, 46.99041594807421)
(12.975, 47.544035924123854)
(13.05, 48.09562009017535)
(13.125, 48.64343349485096)
(13.200000000000001, 49.189792749527875)
(13.275, 49.72999443110694)
(13.35, 50.26681646751665)
(13.425, 50.80309695840961)
(13.5, 51.3338917937903)
(13.575000000000001, 51.85802762503909)
(13.65, 52.382273771115386)
(13.725, 52.90291964236735)
(13.8, 53.42044661258767)
(13.875, 53.93829449866976)
(13.950000000000001, 54.459160999576696)
(14.025, 55.03492417008901)
(14.1, 55.69955094845178)
(14.175, 56.3893295074814)
(14.25, 57.09186447201668)
(14.325000000000001, 57.82198817204419)
(14.4, 58.56745566171296)
(14.475, 59.34157492066608)
(14.55, 60.14148779200962)
(14.625, 60.96938051505191)
(14.700000000000001, 61.848138402186)
(14.775, 66.10095551694982)
(14.85, 76.75490081142573)
(14.925, 88.09786248975952)
};
\addplot[dashed, black, thick, mark = none] coordinates{
(0.0, 0.5978301732190421)
(0.075, 0.6133760916944118)
(0.15, 0.6302307014301745)
(0.225, 0.6474937562089899)
(0.3, 0.6658404406938631)
(0.375, 0.6855625013441176)
(0.45, 0.7072100886259058)
(0.525, 0.729924634387505)
(0.6, 0.7542562890950675)
(0.675, 0.7787713272913476)
(0.75, 0.8055703234834727)
(0.8250000000000001, 0.8346949557370608)
(0.9, 0.8651199436379183)
(0.975, 0.8980706223152032)
(1.05, 0.9571367769084845)
(1.125, 1.0989005493002337)
(1.2, 1.1451548665226605)
(1.2750000000000001, 1.1934430733472272)
(1.35, 1.2504586671121218)
(1.425, 1.3082328016712572)
(1.5, 1.3678491067306908)
(1.575, 1.431733245709368)
(1.6500000000000001, 1.5001519582272418)
(1.725, 1.5731302511236822)
(1.8, 1.6536022602181697)
(1.875, 1.7413345883432452)
(1.95, 1.8342933458967696)
(2.025, 2.4780944254920385)
(2.1, 2.60748814800848)
(2.1750000000000003, 2.7090742651448503)
(2.25, 2.8046754120585313)
(2.325, 2.9040109136515504)
(2.4, 3.005847099181626)
(2.475, 3.113043083950127)
(2.5500000000000003, 3.2260573266788466)
(2.625, 3.3446564302003265)
(2.7, 3.4692071614920015)
(2.775, 3.6020601634547047)
(2.85, 3.7420984639298847)
(2.9250000000000003, 3.8896138093768644)
(3.0, 4.044789583284362)
(3.075, 4.211743578535397)
(3.15, 4.3851493383440365)
(3.225, 4.567940998529765)
(3.3000000000000003, 4.762994345620194)
(3.375, 4.968975681515561)
(3.45, 5.1898861005151575)
(3.525, 5.4273593827911935)
(3.6, 5.676210776980837)
(3.6750000000000003, 5.947368271889028)
(3.75, 6.237430937361369)
(3.825, 6.549357916056708)
(3.9, 6.891509827937941)
(3.975, 7.275306462984293)
(4.05, 7.7634899811765194)
(4.125, 8.116119758754019)
(4.2, 8.48711289204264)
(4.275, 8.87052608888531)
(4.3500000000000005, 9.27121067611992)
(4.425, 9.682389800277043)
(4.5, 10.10815624740033)
(4.575, 10.5434836427763)
(4.65, 10.981970235526083)
(4.7250000000000005, 11.424399573283294)
(4.8, 11.862452714150654)
(4.875, 12.295629521340754)
(4.95, 12.727806054956032)
(5.025, 13.160140965220654)
(5.1000000000000005, 13.587757918457367)
(5.175, 14.010456859951196)
(5.25, 14.423828250359808)
(5.325, 14.839166845465568)
(5.4, 15.251346243197514)
(5.4750000000000005, 15.66676819443451)
(5.55, 16.075063196450895)
(5.625, 16.484250109071496)
(5.7, 16.894520651398157)
(5.775, 17.309109041322802)
(5.8500000000000005, 17.720679939296733)
(5.925, 18.130767098134672)
(6.0, 18.538695333173624)
(6.075, 18.95191668254601)
(6.15, 19.333304325399663)
(6.2250000000000005, 19.705797869050517)
(6.3, 20.07650759149294)
(6.375, 20.44800086156897)
(6.45, 20.81621823568746)
(6.525, 21.186994643034872)
(6.6000000000000005, 21.553469874010542)
(6.675, 21.92303761745504)
(6.75, 22.287362260244844)
(6.825, 22.653379032498723)
(6.9, 23.022079872178374)
(6.9750000000000005, 23.391764314206604)
(7.05, 23.76241568735716)
(7.125, 24.13397564233818)
(7.2, 24.505969049201624)
(7.275, 24.879329496617324)
(7.3500000000000005, 25.253565183411)
(7.425, 25.62804260298525)
(7.5, 26.006062658137)
(7.575, 26.38009829021571)
(7.65, 26.755175873934856)
(7.7250000000000005, 27.127711095651325)
(7.8, 27.496295236747248)
(7.875, 27.869213896667404)
(7.95, 28.23931511935181)
(8.025, 28.617751955159736)
(8.1, 28.98364369321676)
(8.175, 29.34897694519451)
(8.25, 29.720561907014904)
(8.325, 30.09275536859331)
(8.4, 30.46615749407463)
(8.475, 30.84332731668778)
(8.55, 31.21890503719434)
(8.625, 31.598592214970793)
(8.700000000000001, 31.97865449533781)
(8.775, 32.36687734095275)
(8.85, 32.75448335119655)
(8.925, 33.146215489936495)
(9.0, 33.53790595061083)
(9.075000000000001, 33.9300381987807)
(9.15, 34.32471280895325)
(9.225, 34.71945410403078)
(9.3, 35.11671275427163)
(9.375, 35.51023704983313)
(9.450000000000001, 35.905778563770525)
(9.525, 36.295701874462665)
(9.6, 36.69002638888403)
(9.675, 37.08318391746809)
(9.75, 37.47364070740014)
(9.825000000000001, 37.86537284614009)
(9.9, 38.250669891548675)
(9.975, 38.637117251568306)
(10.05, 39.027840781120304)
(10.125, 39.411112272539874)
(10.200000000000001, 39.790757772250714)
(10.275, 40.16463502768007)
(10.35, 40.53541143502748)
(10.425, 40.90880522489568)
(10.5, 41.273504970276036)
(10.575000000000001, 41.638121359525165)
(10.65, 41.998494921694416)
(10.725, 42.358118278682554)
(10.8, 42.71624122530845)
(10.875, 43.066195271073305)
(10.950000000000001, 43.41125631193465)
(11.025, 43.754591880879424)
(11.1, 44.08891665203766)
(11.175, 44.42049900647827)
(11.25, 44.75122279276715)
(11.325000000000001, 45.072352288350864)
(11.4, 45.39109779858125)
(11.475, 45.70932650079797)
(11.55, 46.02420428653903)
(11.625, 46.337431620881645)
(11.700000000000001, 46.65159254389409)
(11.775, 46.966295281759564)
(11.85, 47.28467402501251)
(11.925, 47.59957681759294)
(12.0, 47.9187391084795)
(12.075000000000001, 48.24137735003857)
(12.15, 48.56677467954152)
(12.225, 48.8958313432057)
(12.3, 49.22941424479595)
(12.375, 49.56739835011542)
(12.450000000000001, 49.914426595673916)
(12.525, 50.266964681507055)
(12.6, 50.62702149037762)
(12.675, 50.99723941164576)
(12.75, 51.37682656206473)
(12.825000000000001, 51.76616637983822)
(12.9, 52.16448365294575)
(12.975, 52.573937305186305)
(13.05, 52.996636246680126)
(13.125, 53.435272880466144)
(13.200000000000001, 53.89191443859895)
(13.275, 54.3584170270569)
(13.35, 54.83736468590826)
(13.425, 55.33235006440928)
(13.5, 55.835370973961375)
(13.575000000000001, 56.34455190161176)
(13.65, 56.86528598905134)
(13.725, 57.39508088795618)
(13.8, 57.92813501159234)
(13.875, 58.46749085874987)
(13.950000000000001, 59.008280431364646)
(14.025, 59.609169774600026)
(14.1, 60.313295686370225)
(14.175, 61.02494865679097)
(14.25, 61.75203918271648)
(14.325000000000001, 62.49846833108855)
(14.4, 63.252357853206185)
(14.475, 64.02990384536838)
(14.55, 64.82927247268795)
(14.625, 65.65083883775546)
(14.700000000000001, 66.52143527921554)
(14.775, 70.33132728467902)
(14.85, 79.65141799615529)
(14.925, 89.58084202696104)
};
