# Supplementary material for: CausalSim: A Causal Framework for Unbiased Trace-Driven Simulation
Source: arXiv:2201.01811 source file (2023-05-05)
Supplement: Supplementary file 7 [file new_bola_basic_v2_puffer_ttp_20190202.tex]

\addplot[solid, green!70!black, thick, mark = none] coordinates{
(0.0, 0.3706170114964756)
(0.07722353301491655, 0.3777234988250527)
(0.1544470660298331, 0.3896643312751109)
(0.23167059904474965, 0.408461876555803)
(0.3088941320596662, 0.4380480686992671)
(0.3861176650745828, 0.48189557895110025)
(0.4633411980894993, 0.5526381625621062)
(0.5405647311044158, 0.6661324715307431)
(0.6177882641193324, 0.8371474302031352)
(0.695011797134249, 1.0560546345456663)
(0.7722353301491656, 1.3418369464020186)
(0.849458863164082, 1.7195604452270714)
(0.9266823961789986, 2.1536926943779386)
(1.0039059291939152, 2.481598266726129)
(1.0811294622088317, 2.738245591983689)
(1.1583529952237483, 2.948418746140078)
(1.2355765282386648, 3.1229224905418054)
(1.3128000612535813, 3.284268758971235)
(1.390023594268498, 3.440675938134886)
(1.4672471272834144, 3.5909193272686477)
(1.5444706602983311, 3.7325978682955188)
(1.6216941933132476, 3.873639887214728)
(1.698917726328164, 4.0212324437735445)
(1.7761412593430808, 4.175971773870284)
(1.8533647923579972, 4.338832803771112)
(1.9305883253729137, 4.51127389425434)
(2.0078118583878304, 4.669985444592563)
(2.085035391402747, 4.808884237174583)
(2.1622589244176633, 4.946961191085951)
(2.23948245743258, 5.083869844926294)
(2.3167059904474967, 5.213108004507221)
(2.393929523462413, 5.339469728740866)
(2.4711530564773296, 5.464397263921806)
(2.5483765894922463, 5.588599647334523)
(2.6256001225071626, 5.710658804410051)
(2.7028236555220793, 5.833016079434737)
(2.780047188536996, 5.955808445520354)
(2.857270721551912, 6.07761782809794)
(2.934494254566829, 6.199958988638886)
(3.0117177875817456, 6.323831025134968)
(3.0889413205966623, 6.448694102380956)
(3.1661648536115785, 6.5735732941106795)
(3.243388386626495, 6.699532156250869)
(3.320611919641412, 6.824371061771248)
(3.397835452656328, 6.951828570899096)
(3.475058985671245, 7.081131188414975)
(3.5522825186861615, 7.210498263865809)
(3.6295060517010778, 7.342475885682241)
(3.7067295847159945, 7.475654036537175)
(3.783953117730911, 7.611652222046306)
(3.8611766507458274, 7.748101613100109)
(3.938400183760744, 7.885791819401758)
(4.015623716775661, 8.023554540880228)
(4.0928472497905775, 8.165031650860373)
(4.170070782805494, 8.308837303740695)
(4.24729431582041, 8.454101317399331)
(4.324517848835327, 8.599486189686004)
(4.401741381850243, 8.746248850332302)
(4.47896491486516, 8.895614000102327)
(4.556188447880077, 9.046904830679077)
(4.633411980894993, 9.19852600817246)
(4.710635513909909, 9.351750576797803)
(4.787859046924826, 9.5054827516609)
(4.865082579939743, 9.661108378363243)
(4.942306112954659, 9.818135965150818)
(5.019529645969576, 9.977250377582497)
(5.096753178984493, 10.137525032843332)
(5.173976711999409, 10.301159557963596)
(5.251200245014325, 10.466179928685353)
(5.328423778029242, 10.633867246465792)
(5.4056473110441585, 10.804970834798745)
(5.482870844059075, 10.97746026873319)
(5.560094377073992, 11.153269286317716)
(5.637317910088909, 11.332019197184477)
(5.714541443103824, 11.514161206878146)
(5.791764976118741, 11.698140267717976)
(5.868988509133658, 11.885640343254618)
(5.9462120421485745, 12.079787643333297)
(6.023435575163491, 12.277302870513275)
(6.100659108178408, 12.475140387368016)
(6.1778826411933245, 12.677844478311718)
(6.25510617420824, 12.884432159836342)
(6.332329707223157, 13.093654559452172)
(6.409553240238074, 13.30634157307173)
(6.48677677325299, 13.523524527654269)
(6.564000306267907, 13.743124654797544)
(6.641223839282824, 13.968477652635384)
(6.71844737229774, 14.196529826499383)
(6.795670905312656, 14.427901584013464)
(6.872894438327573, 14.665404902589959)
(6.95011797134249, 14.906791811747377)
(7.027341504357406, 15.150966526591517)
(7.104565037372323, 15.401224459046853)
(7.18178857038724, 15.654955062747785)
(7.2590121034021555, 15.91267400117394)
(7.336235636417072, 16.1751950557541)
(7.413459169431989, 16.439263100773132)
(7.490682702446906, 16.711243357307655)
(7.567906235461822, 16.986639884394695)
(7.645129768476739, 17.268232430479095)
(7.722353301491655, 17.55183122978891)
(7.7995768345065715, 17.840804209425443)
(7.876800367521488, 18.135151369388687)
(7.954023900536405, 18.43145643912613)
(8.031247433551322, 18.734698794112894)
(8.108470966566237, 19.04299303975161)
(8.185694499581155, 19.356677580200778)
(8.26291803259607, 19.674342398133298)
(8.340141565610988, 19.996994648782813)
(8.417365098625904, 20.3250049652753)
(8.49458863164082, 20.65706807442797)
(8.571812164655737, 20.99070234574511)
(8.649035697670653, 21.333392956923163)
(8.72625923068557, 21.682239300889236)
(8.803482763700487, 22.033841221574555)
(8.880706296715404, 22.393597071031436)
(8.95792982973032, 22.756575817235973)
(9.035153362745236, 23.125138232055818)
(9.112376895760153, 23.50174983150293)
(9.18960042877507, 23.878675663382936)
(9.266823961789987, 24.26227289153059)
(9.344047494804903, 24.653580900147006)
(9.421271027819818, 25.05259968923218)
(9.498494560834736, 25.4543740550366)
(9.575718093849652, 25.86096665147877)
(9.65294162686457, 26.275326429082774)
(9.730165159879485, 26.69542296289761)
(9.807388692894403, 27.119096912102343)
(9.884612225909319, 27.549434200332847)
(9.961835758924234, 27.989134003615284)
(10.039059291939152, 28.434731707945932)
(10.116282824954068, 28.888362482420106)
(10.193506357968985, 29.345465928139873)
(10.270729890983901, 29.8124233806656)
(10.347953423998819, 30.286753209501583)
(10.425176957013734, 30.767706091153997)
(10.50240049002865, 31.256184436712175)
(10.579624023043568, 31.750302851578756)
(10.656847556058484, 32.25159221170886)
(10.734071089073401, 32.75902924738512)
(10.811294622088317, 33.27526479118248)
(10.888518155103235, 33.793941679266176)
(10.96574168811815, 34.321916624466866)
(11.042965221133066, 34.857400919089585)
(11.120188754147984, 35.40447958476199)
(11.1974122871629, 35.951864425625416)
(11.274635820177817, 36.503310116390885)
(11.351859353192733, 37.06554445401913)
(11.429082886207649, 37.63457104654306)
(11.506306419222566, 38.20932633803594)
(11.583529952237482, 38.7912928610017)
(11.6607534852524, 39.377239661450815)
(11.737977018267316, 39.97032517819598)
(11.815200551282233, 40.56209736451647)
(11.892424084297149, 41.1620315368504)
(11.969647617312065, 41.77181165874841)
(12.046871150326982, 42.38247807725203)
(12.124094683341898, 42.9956100117676)
(12.201318216356816, 43.61585649085362)
(12.278541749371731, 44.23572427957179)
(12.355765282386649, 44.857775580836496)
(12.432988815401565, 45.4839521899382)
(12.51021234841648, 46.110910351501204)
(12.587435881431398, 46.73364651832478)
(12.664659414446314, 47.35886431564406)
(12.741882947461232, 47.98264792391063)
(12.819106480476147, 48.60989614618092)
(12.896330013491063, 49.22918381348452)
(12.97355354650598, 49.844217257081205)
(13.050777079520897, 50.45348977274146)
(13.128000612535814, 51.061360328316496)
(13.20522414555073, 51.66134284410163)
(13.282447678565648, 52.26189742405949)
(13.359671211580563, 52.85748068578408)
(13.43689474459548, 53.45566643663241)
(13.514118277610397, 54.04591580423964)
(13.591341810625313, 54.62936485970932)
(13.66856534364023, 55.212177393071336)
(13.745788876655146, 55.79652080238849)
(13.823012409670064, 56.381009242059285)
(13.90023594268498, 56.965707170018675)
(13.977459475699895, 57.5485197033807)
(14.054683008714813, 58.13658555844139)
(14.131906541729728, 58.730194795908055)
(14.209130074744646, 59.33795255009691)
(14.286353607759562, 59.95972990513806)
(14.36357714077448, 60.610199098475206)
(14.440800673789395, 61.30744058086268)
(14.518024206804311, 62.08158037964918)
(14.595247739819229, 62.99011497281285)
(14.672471272834144, 64.08683450707204)
(14.749694805849062, 65.53988556299373)
(14.826918338863978, 67.9650106214591)
(14.904141871878894, 94.25819995576575)
(14.981365404893811, 99.8416751972715)
(15.058588937908727, 99.99394095411441)
(15.135812470923645, 99.99850941025421)
(15.21303600393856, 99.99954879445532)
(15.290259536953478, 99.99988719861383)
(15.367483069968394, 99.99994359930692)
};
\addplot[solid, blue, thick, mark = none] coordinates{
(0.0, 0.37561724741744035)
(0.075, 0.37561724741744035)
(0.15, 0.37561724741744035)
(0.225, 0.37561724741744035)
(0.3, 0.37561724741744035)
(0.375, 0.37561724741744035)
(0.45, 0.37561724741744035)
(0.525, 0.37561724741744035)
(0.6, 0.37561724741744035)
(0.675, 0.37561724741744035)
(0.75, 0.37561724741744035)
(0.8250000000000001, 0.37561724741744035)
(0.9, 0.37561724741744035)
(0.975, 0.37561724741744035)
(1.05, 0.37561724741744035)
(1.125, 0.37561724741744035)
(1.2, 0.37561724741744035)
(1.2750000000000001, 0.37561724741744035)
(1.35, 0.37561724741744035)
(1.425, 0.37561724741744035)
(1.5, 0.37561724741744035)
(1.575, 0.37561724741744035)
(1.6500000000000001, 0.37561724741744035)
(1.725, 0.37561724741744035)
(1.8, 0.37561724741744035)
(1.875, 0.37561724741744035)
(1.95, 0.37561724741744035)
(2.025, 4.341887776408051)
(2.1, 4.450447919916324)
(2.1750000000000003, 4.562166794232972)
(2.25, 4.676356611198108)
(2.325, 4.794571262580368)
(2.4, 4.913176509707748)
(2.475, 5.036112274878868)
(2.5500000000000003, 5.160984036351897)
(2.625, 5.288335231685263)
(2.7, 5.419431051444686)
(2.775, 5.55574896649215)
(2.85, 5.695522804762755)
(2.9250000000000003, 5.838964846552763)
(3.0, 5.985022181592717)
(3.075, 6.1377196442997395)
(3.15, 6.294025872043211)
(3.225, 6.454484302381565)
(3.3000000000000003, 6.617082518106236)
(3.375, 6.786541633006088)
(3.45, 6.959303829315773)
(3.525, 7.136625806389161)
(3.6, 7.3201718417489445)
(3.6750000000000003, 7.509194708752283)
(3.75, 7.7050275276596984)
(3.825, 7.91127057229579)
(3.9, 8.132135483738395)
(3.975, 8.344110096373557)
(4.05, 8.496425454547307)
(4.125, 8.650931545378478)
(4.2, 8.808375595509915)
(4.275, 8.96778111557881)
(4.3500000000000005, 9.12963210466064)
(4.425, 9.295193753321126)
(4.5, 9.463430133714509)
(4.575, 9.634545034925203)
(4.65, 9.811204697474254)
(4.7250000000000005, 9.9904541796377)
(4.8, 10.172072709907427)
(4.875, 10.357648144899473)
(4.95, 10.548590025781017)
(5.025, 10.74129807872746)
(5.1000000000000005, 10.938574403649454)
(5.175, 11.141582296570519)
(5.25, 11.34777439393551)
(5.325, 11.558093220259828)
(5.4, 11.771664180722876)
(5.4750000000000005, 11.989642080136322)
(5.55, 12.212884530897057)
(5.625, 12.442427460850842)
(5.7, 12.676504697932781)
(5.775, 12.915914416056815)
(5.8500000000000005, 13.158856478310643)
(5.925, 13.40087299847277)
(6.0, 13.620523666620757)
(6.075, 13.840836649293081)
(6.15, 14.063399803105781)
(6.2250000000000005, 14.287610252017469)
(6.3, 14.51454637993316)
(6.375, 14.744369519878012)
(6.45, 14.980246893872248)
(6.525, 15.221949239195908)
(6.6000000000000005, 15.464483723280917)
(6.675, 15.711408163892616)
(6.75, 15.96254424558215)
(6.825, 16.217450425333293)
(6.9, 16.477417367347318)
(6.9750000000000005, 16.741281775600704)
(7.05, 17.01041073520139)
(7.125, 17.28312298620297)
(7.2, 17.558093899556777)
(7.275, 17.839195467866624)
(7.3500000000000005, 18.123812397882563)
(7.425, 18.414194860744974)
(7.5, 18.710563627961967)
(7.575, 19.01122045716345)
(7.65, 19.315188858986616)
(7.7250000000000005, 19.62454068912298)
(7.8, 19.935760585866447)
(7.875, 20.247175780482472)
(7.95, 20.556001155484108)
(8.025, 20.860733766373816)
(8.1, 21.169100615935523)
(8.175, 21.479853496027218)
(8.25, 21.795021806281152)
(8.325, 22.112075165565894)
(8.4, 22.434146831054264)
(8.475, 22.763393570556282)
(8.55, 23.09988331376675)
(8.625, 23.439744068081858)
(8.700000000000001, 23.78762901759566)
(8.775, 24.135004494398434)
(8.85, 24.488858765843116)
(8.925, 24.848011553482493)
(9.0, 25.209575845287404)
(9.075000000000001, 25.577814229606783)
(9.15, 25.95364375732049)
(9.225, 26.333566049146118)
(9.3, 26.716969737830436)
(9.375, 27.1056125042265)
(9.450000000000001, 27.501506765542867)
(9.525, 27.901578703089662)
(9.6, 28.306575543509734)
(9.675, 28.71710016284446)
(9.75, 29.132108142036238)
(9.825000000000001, 29.551480604119156)
(9.9, 29.97148990709086)
(9.975, 30.391753946418078)
(10.05, 30.816076785009816)
(10.125, 31.244076318332816)
(10.200000000000001, 31.68364088219615)
(10.275, 32.12318846363579)
(10.35, 32.573969918353605)
(10.425, 33.02766385873612)
(10.5, 33.48944992401214)
(10.575000000000001, 33.953027634988615)
(10.65, 34.421088705822136)
(10.725, 34.90074028083155)
(10.8, 35.384611988130644)
(10.875, 35.87331519497266)
(10.950000000000001, 36.367682040118936)
(11.025, 36.8697673968373)
(11.1, 37.37691351581853)
(11.175, 37.89141302426228)
(11.25, 38.40613330421414)
(11.325000000000001, 38.92844472756032)
(11.4, 39.45264969114915)
(11.475, 39.98162671579795)
(11.55, 40.51468801334683)
(11.625, 41.049974008400525)
(11.700000000000001, 41.5910425187244)
(11.775, 42.13240822146303)
(11.85, 42.675327815970306)
(11.925, 43.21924088226408)
(12.0, 43.75861964142971)
(12.075000000000001, 44.30162414805549)
(12.15, 44.85174429021196)
(12.225, 45.39867173671265)
(12.3, 45.94450381688464)
(12.375, 46.49015758160777)
(12.450000000000001, 47.03773885142095)
(12.525, 47.58361338765218)
(12.6, 48.128613329062816)
(12.675, 48.6715838708412)
(12.75, 49.21489406109359)
(12.825000000000001, 49.754323767530316)
(12.9, 50.28814078293389)
(12.975, 50.82357112858904)
(13.05, 51.35405109773538)
(13.125, 51.87790792163835)
(13.200000000000001, 52.39987120529865)
(13.275, 52.913385733167736)
(13.35, 53.42278202328936)
(13.425, 53.93066687770158)
(13.5, 54.435987386134975)
(13.575000000000001, 54.93580558928925)
(13.65, 55.43362835765867)
(13.725, 55.924386437768504)
(13.8, 56.413650064592645)
(13.875, 56.900434257556455)
(13.950000000000001, 57.38269263460396)
(14.025, 57.86832202275611)
(14.1, 58.352890009426936)
(14.175, 58.83986950026331)
(14.25, 59.33202863032847)
(14.325000000000001, 59.82902775114839)
(14.4, 60.336088958011125)
(14.475, 60.851097939165896)
(14.55, 61.37057329775403)
(14.625, 61.91240601714444)
(14.700000000000001, 62.47377701500278)
(14.775, 63.057997863950746)
(14.85, 63.670401045030424)
(14.925, 64.31369525482211)
};
\addplot[solid, red, thick, mark = none] coordinates{

(0.0027847693242870394,0.5271933927393777)
(0.281261701752991,0.7153138758999436)
(0.5597386341816949,1.312516643240236)
(0.8382155666103989,2.3167793270511017)
(1.1166924990391027,3.2724246134236066)
(1.3951694314678067,4.091338505276889)
(1.6736463638965107,4.890939188369855)
(1.9521232963252146,5.774053183436405)
(2.2306002287539184,6.554856321248679)
(2.5090771611826224,7.212206399142065)
(2.7875540936113263,7.846972028076266)
(3.0660310260400303,8.48558901862391)
(3.3445079584687343,9.132690284859759)
(3.6229848908974382,9.805365236788239)
(3.901461823326142,10.515079329589133)
(4.179938755754846,11.220418340055087)
(4.45841568818355,11.90658917211437)
(4.736892620612254,12.610961313556027)
(5.015369553040958,13.34482296023872)
(5.293846485469662,14.11987322735643)
(5.572323417898366,14.936047656974209)
(5.85080035032707,15.797544072105868)
(6.1292772827557735,16.679965144371675)
(6.407754215184478,17.58211840197499)
(6.6862311476131815,18.507935778947957)
(6.964708080041886,19.46847181113503)
(7.243185012470589,20.470575154124965)
(7.521661944899293,21.520748002106163)
(7.800138877327997,22.612673477453217)
(8.078615809756702,23.748776809968742)
(8.357092742185404,24.927913871307318)
(8.63556967461411,26.151478564312303)
(8.914046607042813,27.427318642564234)
(9.192523539471516,28.759438555272077)
(9.471000471900222,30.165000227617085)
(9.749477404328925,31.63820244545348)
(10.027954336757627,33.18938265009936)
(10.306431269186334,34.798671683105454)
(10.584908201615036,36.464917358884456)
(10.863385134043739,38.199270900183265)
(11.141862066472445,39.99060525598059)
(11.420338998901148,41.833360929386735)
(11.698815931329854,43.741879810928765)
(11.977292863758557,45.69812979330354)
(12.25576979618726,47.67559449351976)
(12.534246728615965,49.66609581108024)
(12.812723661044668,51.63914514275216)
(13.09120059347337,53.60337985181927)
(13.369677525902077,55.53260584496497)
(13.64815445833078,57.40605960989252)
(13.926631390759484,59.24878305433119)
(14.205108323188188,61.1415903142284)
(14.483585255616891,63.33593179383613)
(14.762062188045597,67.05285026945431)
(15.0405391204743,99.94568613256017)
(15.319016052903002,99.99711550741085)
(15.597492985331709,99.99745391156935)
(15.875969917760411,99.99759894192299)
(16.154446850189117,99.99780037296972)
(16.43292378261782,99.99796151780711)
(16.711400715046523,99.99810654816075)
(16.989877647475225,99.99825963575627)
(17.26835457990393,99.99836437990056)
(17.546831512332634,99.99845300956113)
(17.82530844476134,99.99858192543103)
(18.103785377190043,99.99866249784972)
(18.382262309618746,99.99877529923589)
(18.66073924204745,99.99887198613831)
(18.939216174476154,99.99896061579888)
(19.21769310690486,99.99907341718504)
(19.496170039333563,99.99917010408748)
(19.774646971762266,99.99925067650616)
(20.05312390419097,99.99929096271552)
(20.331600836619675,99.99936347789233)
(20.61007776904838,99.99938764961794)
(20.888554701477084,99.99944405031103)
(21.167031633905786,99.99948433652037)
(21.44550856633449,99.9995326799716)
(21.72398549876319,99.99957296618093)
(22.002462431191898,99.9996051951484)
(22.280939363620604,99.99965353859963)
(22.559416296049307,99.99965353859963)
(22.83789322847801,99.99967771032523)
(23.116370160906712,99.99970188205084)
(23.394847093335418,99.99971799653457)
(23.673324025764124,99.99971799653457)
(23.951800958192827,99.99973411101833)
(24.23027789062153,99.99974216826018)
(24.508754823050232,99.99975828274393)
(24.78723175547894,99.99975828274393)
(25.06570868790764,99.9997663399858)
(25.344185620336347,99.99977439722765)
(25.62266255276505,99.99977439722765)
(25.901139485193752,99.99977439722765)
(26.179616417622455,99.99979051171141)
(26.45809335005116,99.99979856895327)
(26.736570282479867,99.99979856895327)
(27.01504721490857,99.99980662619514)
(27.293524147337273,99.99983079792075)
(27.572001079765975,99.9998469124045)
(27.85047801219468,99.99985496964635)
(28.128954944623384,99.99985496964635)
(28.40743187705209,99.99985496964635)
(28.685908809480793,99.99985496964635)
(28.964385741909496,99.99987108413009)
(29.2428626743382,99.99987914137196)
(29.521339606766904,99.99989525585569)
(29.79981653919561,99.99989525585569)
(30.078293471624313,99.99990331309758)
(30.356770404053016,99.99991137033945)
(30.63524733648172,99.99991137033945)
(30.913724268910425,99.99991137033945)
(31.192201201339127,99.99991137033945)
(31.470678133767834,99.9999194275813)
(31.749155066196536,99.9999194275813)
(32.02763199862524,99.9999194275813)
(32.30610893105394,99.9999194275813)
(32.584585863482644,99.9999194275813)
(32.863062795911354,99.9999194275813)
(33.14153972834006,99.9999194275813)
(33.42001666076876,99.99992748482317)
(33.69849359319746,99.99992748482317)
(33.97697052562617,99.99992748482317)
(34.255447458054874,99.99992748482317)
(34.53392439048358,99.99992748482317)
(34.81240132291228,99.99994359930692)
(35.09087825534098,99.99994359930692)
(35.369355187769685,99.99994359930692)
(35.64783212019839,99.99994359930692)
(35.9263090526271,99.99994359930692)
(36.2047859850558,99.99994359930692)
(36.4832629174845,99.99994359930692)
(36.761739849913205,99.99994359930692)
(37.040216782341915,99.99994359930692)
(37.31869371477062,99.99994359930692)
(37.59717064719932,99.99994359930692)
(37.87564757962802,99.99995165654877)
(38.154124512056725,99.99995165654877)
(38.43260144448543,99.99995165654877)
(38.71107837691413,99.99995165654877)
(38.98955530934284,99.99995165654877)
(39.26803224177154,99.99995165654877)
(39.546509174200246,99.99995165654877)
(39.82498610662895,99.99995165654877)
(40.10346303905766,99.99995165654877)
(40.38193997148636,99.99995165654877)
(40.66041690391506,99.99995165654877)
(40.938893836343766,99.99995165654877)
(41.21737076877247,99.99995971379066)
(41.49584770120117,99.99995971379066)
(41.774324633629874,99.99995971379066)
(42.052801566058584,99.99996777103253)
(42.331278498487286,99.99996777103253)
(42.60975543091599,99.99996777103253)
(42.88823236334469,99.99996777103253)
(43.1667092957734,99.99996777103253)
(43.445186228202104,99.99996777103253)
(43.72366316063081,99.99996777103253)
(44.00214009305951,99.99996777103253)
(44.28061702548821,99.99997582827439)
(44.559093957916915,99.99997582827439)
(44.83757089034562,99.99997582827439)
(45.11604782277433,99.99997582827439)
(45.39452475520303,99.99997582827439)
(45.67300168763173,99.99997582827439)
(45.951478620060435,99.99997582827439)
(46.229955552489145,99.99997582827439)
(46.50843248491785,99.99997582827439)
(46.78690941734655,99.99997582827439)
(47.06538634977525,99.99997582827439)
(47.343863282203955,99.99997582827439)
(47.62234021463266,99.99997582827439)
(47.90081714706136,99.99997582827439)
(48.17929407949007,99.99997582827439)
(48.45777101191877,99.99997582827439)
(48.736247944347475,99.99997582827439)
(49.01472487677618,99.99997582827439)
(49.29320180920489,99.99997582827439)
(49.57167874163359,99.99997582827439)
(49.85015567406229,99.99997582827439)
(50.128632606490996,99.99997582827439)
(50.4071095389197,99.99997582827439)
(50.6855864713484,99.99997582827439)
(50.964063403777104,99.99998388551626)
(51.24254033620581,99.99998388551626)
(51.521017268634516,99.99998388551626)
(51.79949420106322,99.99998388551626)
(52.07797113349192,99.99998388551626)
(52.35644806592063,99.99998388551626)
(52.634924998349334,99.99998388551626)
(52.913401930778036,99.99998388551626)
(53.19187886320674,99.99998388551626)
(53.47035579563544,99.99998388551626)
(53.748832728064144,99.99998388551626)
(54.02730966049285,99.99998388551626)
(54.30578659292156,99.99998388551626)
(54.58426352535026,99.99998388551626)
(54.86274045777896,99.99998388551626)
(55.141217390207665,99.99998388551626)
(55.419694322636374,99.99999194275813)
};
\addplot[dashed, magenta, thick, mark = none] coordinates{
(0.0, 0.845713581991646)
(0.075, 0.868949896108504)
(0.15, 0.8929784712591263)
(0.225, 0.9178795364089575)
(0.3, 0.9438035208682057)
(0.375, 0.9720441167046635)
(0.45, 1.0024408659874415)
(0.525, 1.0338003628555534)
(0.6, 1.0672959559286246)
(0.675, 1.1026568724482801)
(0.75, 1.1398730837938391)
(0.8250000000000001, 1.1793858492752467)
(0.9, 1.2207839954445991)
(0.975, 1.2647093540254533)
(1.05, 1.3546460242887175)
(1.125, 1.5956137220012192)
(1.2, 1.6593155205641381)
(1.2750000000000001, 1.728162001536184)
(1.35, 1.79897409216162)
(1.425, 1.8721228514056265)
(1.5, 1.947207134440981)
(1.575, 2.0248888302326007)
(1.6500000000000001, 2.108377097398265)
(1.725, 2.19510460904375)
(1.8, 2.285191708617223)
(1.875, 2.379390542669725)
(1.95, 2.4779217408562295)
(2.025, 3.367259822808313)
(2.1, 3.542209110580686)
(2.1750000000000003, 3.6518821063432934)
(2.25, 3.745318765224073)
(2.325, 3.8371508447959632)
(2.4, 3.9292737543675895)
(2.475, 4.023592931868259)
(2.5500000000000003, 4.117370563852178)
(2.625, 4.217726971002545)
(2.7, 4.318043263670188)
(2.775, 4.422842349782043)
(2.85, 4.52875461278944)
(2.9250000000000003, 4.637334488897866)
(3.0, 4.7468069122468615)
(3.075, 4.864472718691875)
(3.15, 4.978909309277748)
(3.225, 5.0937470446908435)
(3.3000000000000003, 5.211001677687953)
(3.375, 5.329720489304425)
(3.45, 5.453283124709609)
(3.525, 5.578510511147765)
(3.6, 5.709975699649228)
(3.6750000000000003, 5.84656551331846)
(3.75, 5.989553586981888)
(3.825, 6.142981454773779)
(3.9, 6.307420748072926)
(3.975, 6.503269681343586)
(4.05, 6.802784466589198)
(4.125, 6.9291751730263)
(4.2, 7.057892519461291)
(4.275, 7.189548251755686)
(4.3500000000000005, 7.325375890253194)
(4.425, 7.461023013578452)
(4.5, 7.601824847933518)
(4.575, 7.746136699526779)
(4.65, 7.892614733187042)
(4.7250000000000005, 8.040837746845723)
(4.8, 8.193072208776627)
(4.875, 8.347683453808825)
(4.95, 8.506235946768482)
(5.025, 8.666633705933362)
(5.1000000000000005, 8.835054361642692)
(5.175, 9.001960695629256)
(5.25, 9.175255260989337)
(5.325, 9.353473879103575)
(5.4, 9.536105090317257)
(5.4750000000000005, 9.722747749803164)
(5.55, 9.914474919974115)
(5.625, 10.111928432553665)
(5.7, 10.314656999611191)
(5.775, 10.521908474595648)
(5.8500000000000005, 10.738496595433707)
(5.925, 10.960470085577228)
(6.0, 11.195019466054172)
(6.075, 11.445474238930483)
(6.15, 11.640280195650368)
(6.2250000000000005, 11.838967228573626)
(6.3, 12.042869144250776)
(6.375, 12.248897127512206)
(6.45, 12.460490995251348)
(6.525, 12.674963077125808)
(6.6000000000000005, 12.892684432100774)
(6.675, 13.115530412243501)
(6.75, 13.338817651696175)
(6.825, 13.56853323700509)
(6.9, 13.805118427480187)
(6.9750000000000005, 14.041111929335129)
(7.05, 14.28781599807691)
(7.125, 14.535773644403763)
(7.2, 14.788294313140272)
(7.275, 15.04641095221653)
(7.3500000000000005, 15.309251071633334)
(7.425, 15.57770721863125)
(7.5, 15.853103171140118)
(7.575, 16.13297188847251)
(7.65, 16.415468104423216)
(7.7250000000000005, 16.702527342783572)
(7.8, 16.996325814241263)
(7.875, 17.288349219838498)
(7.95, 17.590792362322833)
(8.025, 17.915719672372983)
(8.1, 18.202427909009522)
(8.175, 18.49286679253923)
(8.25, 18.79324403916337)
(8.325, 19.095165693372316)
(8.4, 19.401550083784112)
(8.475, 19.715636454878577)
(8.55, 20.032039437350253)
(8.625, 20.353376501196767)
(8.700000000000001, 20.682014400898723)
(8.775, 21.011474647496488)
(8.85, 21.3467414654683)
(8.925, 21.68756413929714)
(9.0, 22.040792216907835)
(9.075000000000001, 22.39601599003396)
(9.15, 22.75531138315639)
(9.225, 23.11690333041467)
(9.3, 23.484612736288092)
(9.375, 23.862561363876367)
(9.450000000000001, 24.246396791804127)
(9.525, 24.63283966110884)
(9.6, 25.026733795579204)
(9.675, 25.418371490396442)
(9.75, 25.823788510028773)
(9.825000000000001, 26.224823022423692)
(9.9, 26.63160393446858)
(9.975, 27.04867421133172)
(10.05, 27.48074730473298)
(10.125, 27.89874021469873)
(10.200000000000001, 28.32302106983119)
(10.275, 28.75147383116677)
(10.35, 29.185241761463036)
(10.425, 29.626039754856386)
(10.5, 30.072152917210428)
(10.575000000000001, 30.52800387024529)
(10.65, 30.990022424998703)
(10.725, 31.457667035953907)
(10.8, 31.932512196557756)
(10.875, 32.41598197094688)
(10.950000000000001, 32.901216782575794)
(11.025, 33.39918794246901)
(11.1, 33.89781096270647)
(11.175, 34.40674340500354)
(11.25, 34.915354931438834)
(11.325000000000001, 35.432410556487156)
(11.4, 35.95261516842918)
(11.475, 36.48201602553527)
(11.55, 37.012058714364926)
(11.625, 37.54928189560186)
(11.700000000000001, 38.08561252959822)
(11.775, 38.628020507727)
(11.85, 39.17391844585262)
(11.925, 39.724449606732655)
(12.0, 40.280837482090135)
(12.075000000000001, 40.83970242675572)
(12.15, 41.397263650732825)
(12.225, 41.95032202402436)
(12.3, 42.50980874317214)
(12.375, 43.07148170162828)
(12.450000000000001, 43.635902502150884)
(12.525, 44.19513850578165)
(12.6, 44.75310087458598)
(12.675, 45.31419217304264)
(12.75, 45.87372903529383)
(12.825000000000001, 46.43335615513113)
(12.9, 46.99041594807421)
(12.975, 47.544035924123854)
(13.05, 48.09562009017535)
(13.125, 48.64343349485096)
(13.200000000000001, 49.189792749527875)
(13.275, 49.72999443110694)
(13.35, 50.26681646751665)
(13.425, 50.80309695840961)
(13.5, 51.3338917937903)
(13.575000000000001, 51.85802762503909)
(13.65, 52.382273771115386)
(13.725, 52.90291964236735)
(13.8, 53.42044661258767)
(13.875, 53.93829449866976)
(13.950000000000001, 54.459160999576696)
(14.025, 55.03492417008901)
(14.1, 55.69955094845178)
(14.175, 56.3893295074814)
(14.25, 57.09186447201668)
(14.325000000000001, 57.82198817204419)
(14.4, 58.56745566171296)
(14.475, 59.34157492066608)
(14.55, 60.14148779200962)
(14.625, 60.96938051505191)
(14.700000000000001, 61.848138402186)
(14.775, 66.10095551694982)
(14.85, 76.75490081142573)
(14.925, 88.09786248975952)
};
\addplot[dashed, black, thick, mark = none] coordinates{
(0.0, 0.49103249123069936)
(0.075, 0.5009267842459972)
(0.15, 0.5112481110803593)
(0.225, 0.5222301317479904)
(0.3, 0.5338245027976758)
(0.375, 0.545821735940818)
(0.45, 0.5576981104559231)
(0.525, 0.571830512694386)
(0.6, 0.5865510935892958)
(0.675, 0.6014892200146722)
(0.75, 0.6173942154643449)
(0.8250000000000001, 0.6347253427248545)
(0.9, 0.6530394534933985)
(0.975, 0.6725863222679201)
(1.05, 0.7051698083867025)
(1.125, 0.7932193475326107)
(1.2, 0.8201385926173911)
(1.2750000000000001, 0.8478474474053465)
(1.35, 0.8786099968617043)
(1.425, 0.9099446104907707)
(1.5, 0.9433418780383356)
(1.575, 0.979156318146641)
(1.6500000000000001, 1.0165741493869043)
(1.725, 1.0563849814623008)
(1.8, 1.0989352757732032)
(1.875, 1.1427586142994288)
(1.95, 1.1884431756974247)
(2.025, 1.6587524408407088)
(2.1, 1.7172480168106292)
(2.1750000000000003, 1.7643345382938551)
(2.25, 1.8085929678810138)
(2.325, 1.8531495154173308)
(2.4, 1.89926916787626)
(2.475, 1.9470647266439693)
(2.5500000000000003, 1.9962461310131698)
(2.625, 2.0469986975468517)
(2.7, 2.0998461469665086)
(2.775, 2.1557634055383064)
(2.85, 2.2138641766566396)
(2.9250000000000003, 2.2761305418213156)
(3.0, 2.3401856146809394)
(3.075, 2.4116372355764293)
(3.15, 2.484410244138457)
(3.225, 2.5608251260253345)
(3.3000000000000003, 2.641671490940236)
(3.375, 2.726602877482789)
(3.45, 2.820268314211484)
(3.525, 2.921902363148754)
(3.6, 3.0298532897114256)
(3.6750000000000003, 3.1456600270965045)
(3.75, 3.268130103507358)
(3.825, 3.3921874565664303)
(3.9, 3.5224408286228686)
(3.975, 3.6661981380519766)
(4.05, 3.832507667472794)
(4.125, 3.9506510049999215)
(4.2, 4.079260699715056)
(4.275, 4.216604444616332)
(4.3500000000000005, 4.360917703734411)
(4.425, 4.51640635732498)
(4.5, 4.682490283973461)
(4.575, 4.859338685759107)
(4.65, 5.047459168919673)
(4.7250000000000005, 5.250090744686551)
(4.8, 5.464493950824235)
(4.875, 5.69445569101122)
(4.95, 5.93638243537387)
(5.025, 6.193875771027689)
(5.1000000000000005, 6.467016270391368)
(5.175, 6.7540313402536984)
(5.25, 7.058466167037099)
(5.325, 7.379418339652226)
(5.4, 7.715993504251604)
(5.4750000000000005, 8.070705520298407)
(5.55, 8.439985029644607)
(5.625, 8.828690549137292)
(5.7, 9.23634670150618)
(5.775, 9.660939176283993)
(5.8500000000000005, 10.104836802580252)
(5.925, 10.566420074779263)
(6.0, 11.049089148949799)
(6.075, 11.557493053650354)
(6.15, 12.077733046656668)
(6.2250000000000005, 12.618591521606099)
(6.3, 13.183444462841814)
(6.375, 13.768811141876347)
(6.45, 14.378768523095479)
(6.525, 15.00866757794072)
(6.6000000000000005, 15.65759783808086)
(6.675, 16.331368574903546)
(6.75, 17.02990727323195)
(6.825, 17.744753829103484)
(6.9, 18.485568875519238)
(6.9750000000000005, 19.239162707539442)
(7.05, 20.0213275192276)
(7.125, 20.816778722757963)
(7.2, 21.626160897480055)
(7.275, 22.45660470244807)
(7.3500000000000005, 23.298900710205583)
(7.425, 24.157778521729778)
(7.5, 25.024012595080492)
(7.575, 25.902856251956397)
(7.65, 26.798966578157863)
(7.7250000000000005, 27.7032550048565)
(7.8, 28.61444848783699)
(7.875, 29.528792352388304)
(7.95, 30.443385991437573)
(8.025, 31.363756672907)
(8.1, 32.27968781410654)
(8.175, 33.192597489605156)
(8.25, 34.09665225628958)
(8.325, 34.99908751735832)
(8.4, 35.895777964974364)
(8.475, 36.78031003460988)
(8.55, 37.652466180734415)
(8.625, 38.506751364393196)
(8.700000000000001, 39.35401869038396)
(8.775, 40.18371317185815)
(8.85, 40.98835768836119)
(8.925, 41.77932100817044)
(9.0, 42.55234085033713)
(9.075000000000001, 43.30823905353191)
(9.15, 44.037628930977235)
(9.225, 44.74938150597102)
(9.3, 45.43680926776189)
(9.375, 46.10350574622347)
(9.450000000000001, 46.74880219028063)
(9.525, 47.37265831372402)
(9.6, 47.97608127178729)
(9.675, 48.557282356775474)
(9.75, 49.120427162734934)
(9.825000000000001, 49.661019748702685)
(9.9, 50.17802878771948)
(9.975, 50.67495917999838)
(10.05, 51.15388163669977)
(10.125, 51.61213726800683)
(10.200000000000001, 52.053061772053375)
(10.275, 52.474568323195314)
(10.35, 52.87789773668047)
(10.425, 53.2631708711369)
(10.5, 53.63648705865954)
(10.575000000000001, 53.992955553433816)
(10.65, 54.33583148117486)
(10.725, 54.66373705352305)
(10.8, 54.98632484623761)
(10.875, 55.29557790365875)
(10.950000000000001, 55.593711967300486)
(11.025, 55.88108155580505)
(11.1, 56.16324616606217)
(11.175, 56.43509750672679)
(11.25, 56.69876268965237)
(11.325000000000001, 56.9555469880217)
(11.4, 57.2033877479163)
(11.475, 57.44773972208156)
(11.55, 57.68600042139374)
(11.625, 57.921610288131)
(11.700000000000001, 58.15054875860061)
(11.775, 58.37749709032853)
(11.85, 58.598563635491985)
(11.925, 58.81899365854779)
(12.0, 59.03321960536435)
(12.075000000000001, 59.24915368745717)
(12.15, 59.45943158575786)
(12.225, 59.669685312332945)
(12.3, 59.87925417334914)
(12.375, 60.08813816880647)
(12.450000000000001, 60.29920567681033)
(12.525, 60.50694554392224)
(12.6, 60.71619211526368)
(12.675, 60.92540645763764)
(12.75, 61.135329837296084)
(12.825000000000001, 61.3439560010136)
(12.9, 61.55129300603206)
(12.975, 61.76481797280601)
(13.05, 61.982822766059186)
(13.125, 62.197669120499675)
(13.200000000000001, 62.41487624680783)
(13.275, 62.63417825600194)
(13.35, 62.85669510470184)
(13.425, 63.080960374887354)
(13.5, 63.30817459559695)
(13.575000000000001, 63.53980418485086)
(13.65, 63.77652595096605)
(13.725, 64.02043477682851)
(13.8, 64.26715558010329)
(13.875, 64.52191751076347)
(13.950000000000001, 64.78333472320756)
(14.025, 65.10578554281035)
(14.1, 65.52153116601585)
(14.175, 65.95923277331474)
(14.25, 66.41214645326255)
(14.325000000000001, 66.89187463415087)
(14.4, 67.39989984848357)
(14.475, 67.93586757761844)
(14.55, 68.49694167241752)
(14.625, 69.08293681631785)
(14.700000000000001, 69.70173299186743)
(14.775, 73.03841410919738)
(14.85, 81.51443918172264)
(14.925, 90.53297446378048)
};
