# Supplementary material for: CausalSim: A Causal Framework for Unbiased Trace-Driven Simulation
Source: arXiv:2201.01811 source file (2023-05-05)
Supplement: Supplementary file 8 [file new_bola_basic_v2_puffer_ttp_cl.tex]

\addplot[solid, green!70!black, thick, mark = none] coordinates{
(0.0, 0.381180597812079)
(0.07826325007796112, 0.3884463210031381)
(0.15652650015592223, 0.401258904870343)
(0.23478975023388335, 0.4198591562394543)
(0.31305300031184446, 0.44734434911077514)
(0.39131625038980555, 0.4914203019086515)
(0.4695795004677667, 0.5611463334918784)
(0.5478427505457278, 0.671909169658207)
(0.6261060006236889, 0.8365546090094303)
(0.70436925070165, 1.0468038789495642)
(0.7826325007796111, 1.3236071733197994)
(0.8608957508575723, 1.6937438718814684)
(0.9391590009355334, 2.08925662766814)
(1.0174222510134945, 2.380848782613548)
(1.0956855010914557, 2.6171051897358497)
(1.1739487511694167, 2.8156628731011137)
(1.2522120012473779, 2.984252562184626)
(1.330475251325339, 3.1447378560287396)
(1.4087385014033, 3.300498353877754)
(1.4870017514812612, 3.4471497107660913)
(1.5652650015592222, 3.588021703836169)
(1.6435282516371834, 3.7316671272443194)
(1.7217915017151446, 3.8777040115427845)
(1.8000547517931056, 4.037965105928432)
(1.8783180018710668, 4.2035654688990505)
(1.9565812519490278, 4.373641517355363)
(2.034844502026989, 4.522377098839079)
(2.11310775210495, 4.664594288659958)
(2.1913710021829114, 4.80710210740848)
(2.269634252260872, 4.945607550639184)
(2.3478975023388333, 5.076606463853069)
(2.4261607524167945, 5.205404900900517)
(2.5044240024947557, 5.330773916601787)
(2.582687252572717, 5.453170213557457)
(2.660950502650678, 5.573897470100096)
(2.739213752728639, 5.695330539752723)
(2.8174770028066, 5.816298603121122)
(2.8957402528845613, 5.93818837537433)
(2.9740035029625225, 6.062569252721615)
(3.0522667530404837, 6.187116203741839)
(3.1305300031184444, 6.313888541979439)
(3.2087932531964056, 6.440038103943518)
(3.287056503274367, 6.565357297542906)
(3.365319753352328, 6.693067952032609)
(3.4435830034302892, 6.8233029263509755)
(3.52184625350825, 6.952217614969482)
(3.600109503586211, 7.085026731218397)
(3.6783727536641724, 7.218251031649656)
(3.7566360037421336, 7.350561926879755)
(3.8348992538200948, 7.48598670347745)
(3.9131625038980555, 7.624110177260396)
(3.9914257539760167, 7.761810163177348)
(4.069689004053978, 7.9017604473626175)
(4.147952254131939, 8.045837662320409)
(4.2262155042099, 8.191899457669814)
(4.304478754287861, 8.338326615099684)
(4.382742004365823, 8.487676669173272)
(4.4610052544437835, 8.636711183268277)
(4.539268504521744, 8.78713241253232)
(4.617531754599706, 8.940102872675965)
(4.695795004677667, 9.093480213318312)
(4.774058254755628, 9.248784008566744)
(4.852321504833589, 9.406138813675968)
(4.930584754911551, 9.565187570249163)
(5.008848004989511, 9.7250749988707)
(5.087111255067472, 9.887362192066195)
(5.165374505145434, 10.0503053762698)
(5.243637755223395, 10.215349392436075)
(5.321901005301356, 10.382494240565023)
(5.400164255379317, 10.55417289996519)
(5.478427505457278, 10.731348597939624)
(5.556690755535239, 10.907801875436773)
(5.6349540056132, 11.085716601255783)
(5.713217255691162, 11.268347819386245)
(5.7914805057691225, 11.452191375329159)
(5.869743755847083, 11.64038606150306)
(5.948007005925045, 11.832167939012434)
(6.026270256003006, 12.028350768854676)
(6.104533506080967, 12.228992676815318)
(6.182796756158928, 12.43392758922142)
(6.261060006236889, 12.64127056988513)
(6.3393232563148505, 12.850564916205867)
(6.417586506392811, 13.063645742269603)
(6.495849756470773, 13.282406287947834)
(6.574113006548734, 13.503782493974848)
(6.652376256626694, 13.728089900329223)
(6.730639506704656, 13.956781651649178)
(6.808902756782617, 14.192589659854546)
(6.8871660068605784, 14.429884027432713)
(6.965429256938539, 14.672667129901498)
(7.0436925070165, 14.920914056209961)
(7.121955757094462, 15.172831210690363)
(7.200219007172422, 15.428875295943284)
(7.278482257250384, 15.688871934612145)
(7.356745507328345, 15.954133108713156)
(7.4350087574063055, 16.222034854213888)
(7.513272007484267, 16.496645976101334)
(7.591535257562228, 16.778697198536427)
(7.6697985076401896, 17.059610816311892)
(7.74806175771815, 17.346378531058434)
(7.826325007796111, 17.640146251119337)
(7.904588257874073, 17.935798907368092)
(7.9828515079520335, 18.236940298507463)
(8.061114758029994, 18.54338774349722)
(8.139378008107956, 18.85500838339901)
(8.217641258185918, 19.17522333587537)
(8.295904508263877, 19.497671979252747)
(8.374167758341839, 19.827801530003534)
(8.4524310084198, 20.16079585161251)
(8.530694258497762, 20.49836550291094)
(8.608957508575722, 20.842561493759614)
(8.687220758653684, 21.190286550158234)
(8.765484008731645, 21.542927387275835)
(8.843747258809605, 21.904677365354107)
(8.922010508887567, 22.271069102591014)
(9.000273758965529, 22.644020749908993)
(9.078537009043488, 23.022220325291826)
(9.15680025912145, 23.403201634696376)
(9.235063509199412, 23.79166456306681)
(9.313326759277373, 24.182568774429434)
(9.391590009355333, 24.580348435851718)
(9.469853259433295, 24.983965586877787)
(9.548116509511257, 25.39643446467148)
(9.626379759589216, 25.811552217548538)
(9.704643009667178, 26.234267840962538)
(9.78290625974514, 26.663269352897256)
(9.861169509823101, 27.100499815326074)
(9.939432759901061, 27.542405251648116)
(10.017696009979023, 27.98818020454962)
(10.095959260056985, 28.440465245430318)
(10.174222510134944, 28.902357648290504)
(10.252485760212906, 29.36591078788008)
(10.330749010290868, 29.843704744924125)
(10.409012260368828, 30.32887237304664)
(10.48727551044679, 30.814754117962796)
(10.56553876052475, 31.308283555517765)
(10.643802010602712, 31.80752592742182)
(10.722065260680672, 32.3094088707256)
(10.800328510758634, 32.82531673570902)
(10.878591760836596, 33.34917952962621)
(10.956855010914555, 33.879917773603054)
(11.035118260992517, 34.41736539396661)
(11.113381511070479, 34.9629589279878)
(11.191644761148439, 35.511168122357766)
(11.2699080112264, 36.06205940654569)
(11.348171261304362, 36.62558059356059)
(11.426434511382324, 37.19258102402355)
(11.504697761460283, 37.76777719024603)
(11.582961011538245, 38.348935401327)
(11.661224261616207, 38.930550315008546)
(11.739487511694167, 39.522353848524865)
(11.817750761772128, 40.116258214003864)
(11.89601401185009, 40.71648998642182)
(11.97427726192805, 41.31914643446467)
(12.052540512006011, 41.92568070277064)
(12.130803762083973, 42.53668235287865)
(12.209067012161935, 43.153646047845164)
(12.287330262239895, 43.76933927921369)
(12.365593512317856, 44.395686136701215)
(12.443856762395818, 45.023120776746495)
(12.522120012473778, 45.651294444636356)
(12.60038326255174, 46.278114612091755)
(12.678646512629701, 46.90447807694658)
(12.75690976270766, 47.52610013843901)
(12.835173012785623, 48.14612789267124)
(12.913436262863584, 48.76318292815785)
(12.991699512941546, 49.376974615971235)
(13.069962763019506, 49.99132265058896)
(13.148226013097467, 50.60137768076123)
(13.226489263175429, 51.20840186640236)
(13.304752513253389, 51.814172195812816)
(13.38301576333135, 52.412211795747986)
(13.461279013409312, 53.00935459784928)
(13.539542263487274, 53.602328950759826)
(13.617805513565234, 54.19422382479626)
(13.696068763643195, 54.784308495797674)
(13.774332013721157, 55.372616178498646)
(13.852595263799117, 55.96126431222913)
(13.930858513877078, 56.555949223970934)
(14.00912176395504, 57.15011100364299)
(14.087385014033, 57.74743648678452)
(14.165648264110962, 58.35780705693537)
(14.243911514188923, 58.97394868722083)
(14.322174764266885, 59.61593138101552)
(14.400438014344845, 60.297763452631806)
(14.478701264422806, 61.03499770154036)
(14.556964514500768, 61.881682804599045)
(14.635227764578728, 62.888653913094316)
(14.71349101465669, 64.15006649589866)
(14.791754264734651, 65.98219955943976)
(14.870017514812611, 77.15237292706841)
(14.948280764890573, 99.24327700557211)
(15.026544014968534, 99.97630959055532)
(15.104807265046496, 99.99691933336699)
(15.183070515124456, 99.99902016532967)
(15.261333765202417, 99.99963463791953)
(15.339597015280379, 99.99983392632707)
(15.417860265358339, 99.99995017789813)
(15.4961235154363, 99.99996678526541)
(15.574386765514262, 99.99999169631634)
};
\addplot[solid, blue, thick, mark = none] coordinates{
(0.0, 0.38650541846808634)
(0.075, 0.38650541846808634)
(0.15, 0.38650541846808634)
(0.225, 0.38650541846808634)
(0.3, 0.38650541846808634)
(0.375, 0.38650541846808634)
(0.45, 0.38650541846808634)
(0.525, 0.38650541846808634)
(0.6, 0.38650541846808634)
(0.675, 0.38650541846808634)
(0.75, 0.38650541846808634)
(0.8250000000000001, 0.38650541846808634)
(0.9, 0.38650541846808634)
(0.975, 0.38650541846808634)
(1.05, 0.38650541846808634)
(1.125, 0.38650541846808634)
(1.2, 0.38650541846808634)
(1.2750000000000001, 0.38650541846808634)
(1.35, 0.38650541846808634)
(1.425, 0.38650541846808634)
(1.5, 0.38650541846808634)
(1.575, 0.38650541846808634)
(1.6500000000000001, 0.38650541846808634)
(1.725, 0.38650541846808634)
(1.8, 0.38650541846808634)
(1.875, 0.38650541846808634)
(1.95, 0.38650541846808634)
(2.025, 4.264417546498682)
(2.1, 4.372720657127206)
(2.1750000000000003, 4.482270334466924)
(2.25, 4.595394084195383)
(2.325, 4.711377091834831)
(2.4, 4.831701289839139)
(2.475, 4.952374177832592)
(2.5500000000000003, 5.078007180921636)
(2.625, 5.205732323945552)
(2.7, 5.337476119094369)
(2.775, 5.470544936201936)
(2.85, 5.607824184928433)
(2.9250000000000003, 5.749296430774402)
(3.0, 5.89478732874527)
(3.075, 6.047426371493617)
(3.15, 6.2005274284775815)
(3.225, 6.358327083065278)
(3.3000000000000003, 6.518951126565052)
(3.375, 6.685773134621882)
(3.45, 6.855654897333463)
(3.525, 7.033539095295928)
(3.6, 7.217385892072777)
(3.6750000000000003, 7.405643617212314)
(3.75, 7.603263668560402)
(3.825, 7.810141439120296)
(3.9, 8.030339167265542)
(3.975, 8.235177101388937)
(4.05, 8.383875947259941)
(4.125, 8.537404149480608)
(4.2, 8.691176434693677)
(4.275, 8.848583813043586)
(4.3500000000000005, 9.009417070536847)
(4.425, 9.173528013928072)
(4.5, 9.340132090741687)
(4.575, 9.511582958404423)
(4.65, 9.684428586023738)
(4.7250000000000005, 9.85940993982657)
(4.8, 10.040528237438357)
(4.875, 10.223756109484473)
(4.95, 10.412789669849857)
(5.025, 10.605807013341227)
(5.1000000000000005, 10.803244002445014)
(5.175, 11.004603753926686)
(5.25, 11.208692004573418)
(5.325, 11.415447733637112)
(5.4, 11.630659194937579)
(5.4750000000000005, 11.84903501788954)
(5.55, 12.074053385134718)
(5.625, 12.30446772996192)
(5.7, 12.54037394211816)
(5.775, 12.777892845474195)
(5.8500000000000005, 13.020136498183152)
(5.925, 13.255755041098347)
(6.0, 13.47428777454542)
(6.075, 13.692428231754707)
(6.15, 13.913340774377703)
(6.2250000000000005, 14.137888410137533)
(6.3, 14.361015134191598)
(6.375, 14.593940046940645)
(6.45, 14.828416630141392)
(6.525, 15.068934267404078)
(6.6000000000000005, 15.311221506361674)
(6.675, 15.557954542680875)
(6.75, 15.813064855989293)
(6.825, 16.068968439023013)
(6.9, 16.327147224235908)
(6.9750000000000005, 16.590617380034082)
(7.05, 16.857260614733477)
(7.125, 17.128977288774937)
(7.2, 17.404512118197538)
(7.275, 17.685303449206504)
(7.3500000000000005, 17.971115916059162)
(7.425, 18.26010146181304)
(7.5, 18.55688022882432)
(7.575, 18.858296572691227)
(7.65, 19.15968676480895)
(7.7250000000000005, 19.469088109427286)
(7.8, 19.776318858863192)
(7.875, 20.087019073691096)
(7.95, 20.393613463896813)
(8.025, 20.698054693419557)
(8.1, 21.00607871258077)
(8.175, 21.316168719927667)
(8.25, 21.634156555528705)
(8.325, 21.95345197858904)
(8.4, 22.27669631577644)
(8.475, 22.60544995479234)
(8.55, 22.936470078737685)
(8.625, 23.273313325501757)
(8.700000000000001, 23.618420525008567)
(8.775, 23.96697975540792)
(8.85, 24.322434330342617)
(8.925, 24.67788018802759)
(9.0, 25.03791131906982)
(9.075000000000001, 25.405726954119718)
(9.15, 25.77989746422179)
(9.225, 26.156430349000324)
(9.3, 26.540756455036252)
(9.375, 26.932640416586906)
(9.450000000000001, 27.325535579106074)
(9.525, 27.725186610164943)
(9.6, 28.129579825076178)
(9.675, 28.53730302938376)
(9.75, 28.948521850832513)
(9.825000000000001, 29.36350652416404)
(9.9, 29.78111508966389)
(9.975, 30.1962479562408)
(10.05, 30.616340937913307)
(10.125, 31.04216115265752)
(10.200000000000001, 31.472950199747064)
(10.275, 31.910120273637954)
(10.35, 32.35446464405551)
(10.425, 32.80331583258278)
(10.5, 33.25515703776696)
(10.575000000000001, 33.714599684714514)
(10.65, 34.1876935447371)
(10.725, 34.65899165131559)
(10.8, 35.13689743318839)
(10.875, 35.619083384677936)
(10.950000000000001, 36.10638636175819)
(11.025, 36.6042982317582)
(11.1, 37.10136452853452)
(11.175, 37.607819303268585)
(11.25, 38.11858039936859)
(11.325000000000001, 38.63349962358916)
(11.4, 39.15549725458937)
(11.475, 39.6746356276786)
(11.55, 40.20283994048559)
(11.625, 40.73120988103744)
(11.700000000000001, 41.26338054247096)
(11.775, 41.79671931536813)
(11.85, 42.32745163059643)
(11.925, 42.86504442136116)
(12.0, 43.398051938768646)
(12.075000000000001, 43.93276803712293)
(12.15, 44.475059425491395)
(12.225, 45.01383776221923)
(12.3, 45.55483899762786)
(12.375, 46.09824619396159)
(12.450000000000001, 46.640241195839295)
(12.525, 47.1820880044716)
(12.6, 47.72334204012236)
(12.675, 48.26646156721505)
(12.75, 48.80253755652701)
(12.825000000000001, 49.336687033648936)
(12.9, 49.86789879761231)
(12.975, 50.39628617266361)
(13.05, 50.92088154408295)
(13.125, 51.44190284311356)
(13.200000000000001, 51.95701384682816)
(13.275, 52.47474874271107)
(13.35, 52.981587076433186)
(13.425, 53.48565332474161)
(13.5, 53.983922601980495)
(13.575000000000001, 54.482130858471265)
(13.65, 54.9769481048176)
(13.725, 55.467302119302886)
(13.8, 55.9564793050748)
(13.875, 56.443895606401526)
(13.950000000000001, 56.92812139432758)
(14.025, 57.41099600854569)
(14.1, 57.895561769211156)
(14.175, 58.38045006811659)
(14.25, 58.87063845485703)
(14.325000000000001, 59.367024806154525)
(14.4, 59.873313953143736)
(14.475, 60.38404889749456)
(14.55, 60.90856581366635)
(14.625, 61.450595684542954)
(14.700000000000001, 62.0078284389463)
(14.775, 62.59442089043568)
(14.85, 63.20787990558869)
(14.925, 63.854647531954825)
};
\addplot[solid, red, thick, mark = none] coordinates{
(0.00343610844773101,0.5368580588246236)
(0.347046953220832,0.7842247946665107)
(0.690657797993933,1.705618139496571)
(1.034268642767034,2.8938752693714975)
(1.377879487540135,3.88827460082532)
(1.721490332313236,4.853752202136903)
(2.065101177086337,5.932475441025246)
(2.4087120218594382,6.779310010389569)
(2.752322866632539,7.549842030722301)
(3.09593371140564,8.315449966652407)
(3.439544556178741,9.100480218632669)
(3.783155400951842,9.94148560207685)
(4.1267662457249426,10.810316629421877)
(4.470377090498044,11.64813339834564)
(4.813987935271145,12.513867151690365)
(5.157598780044246,13.426400466069154)
(5.501209624817347,14.406608802170384)
(5.844820469590449,15.445723470062894)
(6.18843131436355,16.525127611010284)
(6.532042159136649,17.63949026011123)
(6.8756530039097505,18.796965634707004)
(7.219263848682852,20.011362760702454)
(7.562874693455953,21.300086159021518)
(7.906485538229054,22.6608855313959)
(8.250096383002155,24.080167747695562)
(8.593707227775255,25.56854491562129)
(8.937318072548358,27.14068964417719)
(9.280928917321457,28.79868615795865)
(9.62453976209456,30.56319402187921)
(9.96815060686766,32.43264383972961)
(10.311761451640761,34.39213880304725)
(10.655372296413862,36.43437167022286)
(10.998983141186963,38.575974719601206)
(11.342593985960065,40.80587083719732)
(11.686204830733164,43.11401256579839)
(12.029815675506267,45.493541062712076)
(12.373426520279367,47.911515614911025)
(12.717037365052468,50.34274284621046)
(13.060648209825569,52.758849069588855)
(13.40425905459867,55.12751634829236)
(13.747869899371771,57.42660706171829)
(14.09148074414487,59.72175352541193)
(14.435091588917974,62.26757159103893)
(14.778702433691073,66.81482652608419)
(15.122313278464176,99.98854922025089)
(15.465924123237276,99.99769157594616)
(15.809534968010377,99.99810676012851)
(16.153145812783478,99.99833926327062)
(16.49675665755658,99.99847212220897)
(16.84036750232968,99.99860498114732)
(17.18397834710278,99.99873784008567)
(17.527589191875883,99.99885409165672)
(17.871200036648986,99.99894543217684)
(18.214810881422082,99.99902846901331)
(18.558421726195185,99.99910320216613)
(18.902032570968288,99.99916963163531)
(19.245643415741387,99.99919454268625)
(19.589254260514487,99.99926097215543)
(19.93286510528759,99.99929418689001)
(20.276475950060693,99.99936061635918)
(20.62008679483379,99.99938552741013)
(20.96369763960689,99.99946026056294)
(21.307308484379995,99.99948517161388)
(21.650919329153094,99.99952669003213)
(21.994530173926194,99.9995931195013)
(22.338141018699297,99.99961803055224)
(22.6817518634724,99.99963463791953)
(23.025362708245495,99.99964294160318)
(23.3689735530186,99.99968446002143)
(23.7125843977917,99.99970937107236)
(24.0561952425648,99.99970937107236)
(24.3998060873379,99.999717674756)
(24.743416932111003,99.9997342821233)
(25.087027776884106,99.99975919317424)
(25.430638621657202,99.99978410422517)
(25.774249466430305,99.99979240790883)
(26.11786031120341,99.99980071159248)
(26.46147115597651,99.99980901527611)
(26.805082000749607,99.99982562264341)
(27.14869284552271,99.99983392632707)
(27.492303690295813,99.99983392632707)
(27.835914535068913,99.999858837378)
(28.179525379842012,99.99986714106164)
(28.523136224615115,99.9998754447453)
(28.866747069388218,99.99990035579623)
(29.210357914161314,99.99990865947989)
(29.553968758934417,99.99990865947989)
(29.89757960370752,99.99991696316353)
(30.24119044848062,99.99991696316353)
(30.58480129325372,99.99991696316353)
(30.92841213802682,99.99992526684719)
(31.272022982799925,99.99992526684719)
(31.61563382757302,99.99994187421447)
(31.959244672346124,99.99994187421447)
(32.30285551711923,99.99994187421447)
(32.64646636189232,99.99994187421447)
(32.990077206665426,99.99995017789813)
(33.33368805143853,99.99995017789813)
(33.67729889621163,99.99995017789813)
(34.020909740984735,99.99995017789813)
(34.36452058575783,99.99995017789813)
(34.70813143053093,99.99995017789813)
(35.051742275304036,99.99995017789813)
(35.39535312007713,99.99995017789813)
(35.738963964850235,99.99995017789813)
(36.08257480962334,99.99995017789813)
(36.426185654396434,99.99995017789813)
(36.76979649916954,99.99995017789813)
(37.11340734394264,99.99995017789813)
(37.457018188715736,99.99995017789813)
(37.800629033488846,99.99995017789813)
(38.14423987826194,99.99995017789813)
(38.487850723035045,99.99995017789813)
(38.83146156780815,99.99995017789813)
(39.175072412581244,99.99995848158176)
(39.51868325735435,99.99995848158176)
(39.86229410212745,99.99995848158176)
(40.205904946900546,99.99996678526541)
(40.54951579167365,99.99996678526541)
(40.89312663644675,99.99996678526541)
(41.23673748121985,99.99996678526541)
(41.58034832599295,99.99996678526541)
(41.923959170766054,99.99996678526541)
(42.26757001553915,99.99996678526541)
(42.61118086031226,99.99996678526541)
(42.954791705085356,99.99996678526541)
(43.29840254985846,99.99996678526541)
(43.64201339463156,99.99996678526541)
(43.98562423940466,99.99996678526541)
(44.32923508417776,99.99997508894906)
(44.67284592895086,99.99997508894906)
(45.01645677372396,99.99997508894906)
(45.36006761849706,99.99997508894906)
(45.703678463270165,99.99997508894906)
(46.04728930804326,99.99997508894906)
(46.39090015281637,99.99997508894906)
(46.73451099758947,99.99997508894906)
(47.07812184236257,99.99998339263271)
(47.42173268713567,99.99998339263271)
(47.76534353190877,99.99998339263271)
(48.10895437668187,99.99998339263271)
(48.452565221454975,99.99998339263271)
(48.79617606622807,99.99998339263271)
(49.139786911001174,99.99998339263271)
(49.48339775577428,99.99998339263271)
(49.82700860054737,99.99998339263271)
(50.170619445320476,99.99998339263271)
(50.51423029009358,99.99998339263271)
(50.857841134866675,99.99998339263271)
(51.201451979639785,99.99998339263271)
(51.54506282441288,99.99998339263271)
(51.888673669185984,99.99998339263271)
(52.23228451395909,99.99998339263271)
(52.57589535873218,99.99998339263271)
(52.919506203505286,99.99998339263271)
(53.26311704827839,99.99998339263271)
(53.606727893051485,99.99998339263271)
(53.95033873782459,99.99998339263271)
(54.29394958259769,99.99998339263271)
(54.637560427370786,99.99998339263271)
(54.98117127214389,99.99998339263271)
(55.32478211691699,99.99998339263271)
(55.668392961690095,99.99998339263271)
(56.0120038064632,99.99998339263271)
(56.355614651236294,99.99998339263271)
(56.6992254960094,99.99998339263271)
(57.0428363407825,99.99998339263271)
(57.386447185555596,99.99998339263271)
(57.7300580303287,99.99998339263271)
(58.0736688751018,99.99998339263271)
(58.4172797198749,99.99998339263271)
(58.760890564648,99.99998339263271)
(59.104501409421104,99.99998339263271)
(59.4481122541942,99.99998339263271)
(59.79172309896731,99.99998339263271)
(60.135333943740406,99.99998339263271)
(60.47894478851351,99.99998339263271)
(60.82255563328661,99.99998339263271)
(61.16616647805971,99.99998339263271)
(61.50977732283281,99.99998339263271)
(61.853388167605914,99.99998339263271)
(62.19699901237901,99.99998339263271)
(62.54060985715211,99.99998339263271)
(62.884220701925216,99.99998339263271)
(63.22783154669831,99.99998339263271)
(63.571442391471415,99.99998339263271)
(63.91505323624452,99.99998339263271)
(64.25866408101761,99.99998339263271)
(64.60227492579072,99.99998339263271)
(64.94588577056382,99.99998339263271)
(65.28949661533693,99.99998339263271)
(65.63310746011003,99.99998339263271)
(65.97671830488312,99.99999169631634)
(66.32032914965623,99.99999169631634)
(66.66393999442933,99.99999169631634)
(67.00755083920242,99.99999169631634)
(67.35116168397553,99.99999169631634)
(67.69477252874863,99.99999169631634)
(68.03838337352173,99.99999169631634)
(68.38199421829484,99.99999169631634)
};
\addplot[dashed, magenta, thick, mark = none] coordinates{
(0.0, 0.845713581991646)
(0.075, 0.868949896108504)
(0.15, 0.8929784712591263)
(0.225, 0.9178795364089575)
(0.3, 0.9438035208682057)
(0.375, 0.9720441167046635)
(0.45, 1.0024408659874415)
(0.525, 1.0338003628555534)
(0.6, 1.0672959559286246)
(0.675, 1.1026568724482801)
(0.75, 1.1398730837938391)
(0.8250000000000001, 1.1793858492752467)
(0.9, 1.2207839954445991)
(0.975, 1.2647093540254533)
(1.05, 1.3546460242887175)
(1.125, 1.5956137220012192)
(1.2, 1.6593155205641381)
(1.2750000000000001, 1.728162001536184)
(1.35, 1.79897409216162)
(1.425, 1.8721228514056265)
(1.5, 1.947207134440981)
(1.575, 2.0248888302326007)
(1.6500000000000001, 2.108377097398265)
(1.725, 2.19510460904375)
(1.8, 2.285191708617223)
(1.875, 2.379390542669725)
(1.95, 2.4779217408562295)
(2.025, 3.367259822808313)
(2.1, 3.542209110580686)
(2.1750000000000003, 3.6518821063432934)
(2.25, 3.745318765224073)
(2.325, 3.8371508447959632)
(2.4, 3.9292737543675895)
(2.475, 4.023592931868259)
(2.5500000000000003, 4.117370563852178)
(2.625, 4.217726971002545)
(2.7, 4.318043263670188)
(2.775, 4.422842349782043)
(2.85, 4.52875461278944)
(2.9250000000000003, 4.637334488897866)
(3.0, 4.7468069122468615)
(3.075, 4.864472718691875)
(3.15, 4.978909309277748)
(3.225, 5.0937470446908435)
(3.3000000000000003, 5.211001677687953)
(3.375, 5.329720489304425)
(3.45, 5.453283124709609)
(3.525, 5.578510511147765)
(3.6, 5.709975699649228)
(3.6750000000000003, 5.84656551331846)
(3.75, 5.989553586981888)
(3.825, 6.142981454773779)
(3.9, 6.307420748072926)
(3.975, 6.503269681343586)
(4.05, 6.802784466589198)
(4.125, 6.9291751730263)
(4.2, 7.057892519461291)
(4.275, 7.189548251755686)
(4.3500000000000005, 7.325375890253194)
(4.425, 7.461023013578452)
(4.5, 7.601824847933518)
(4.575, 7.746136699526779)
(4.65, 7.892614733187042)
(4.7250000000000005, 8.040837746845723)
(4.8, 8.193072208776627)
(4.875, 8.347683453808825)
(4.95, 8.506235946768482)
(5.025, 8.666633705933362)
(5.1000000000000005, 8.835054361642692)
(5.175, 9.001960695629256)
(5.25, 9.175255260989337)
(5.325, 9.353473879103575)
(5.4, 9.536105090317257)
(5.4750000000000005, 9.722747749803164)
(5.55, 9.914474919974115)
(5.625, 10.111928432553665)
(5.7, 10.314656999611191)
(5.775, 10.521908474595648)
(5.8500000000000005, 10.738496595433707)
(5.925, 10.960470085577228)
(6.0, 11.195019466054172)
(6.075, 11.445474238930483)
(6.15, 11.640280195650368)
(6.2250000000000005, 11.838967228573626)
(6.3, 12.042869144250776)
(6.375, 12.248897127512206)
(6.45, 12.460490995251348)
(6.525, 12.674963077125808)
(6.6000000000000005, 12.892684432100774)
(6.675, 13.115530412243501)
(6.75, 13.338817651696175)
(6.825, 13.56853323700509)
(6.9, 13.805118427480187)
(6.9750000000000005, 14.041111929335129)
(7.05, 14.28781599807691)
(7.125, 14.535773644403763)
(7.2, 14.788294313140272)
(7.275, 15.04641095221653)
(7.3500000000000005, 15.309251071633334)
(7.425, 15.57770721863125)
(7.5, 15.853103171140118)
(7.575, 16.13297188847251)
(7.65, 16.415468104423216)
(7.7250000000000005, 16.702527342783572)
(7.8, 16.996325814241263)
(7.875, 17.288349219838498)
(7.95, 17.590792362322833)
(8.025, 17.915719672372983)
(8.1, 18.202427909009522)
(8.175, 18.49286679253923)
(8.25, 18.79324403916337)
(8.325, 19.095165693372316)
(8.4, 19.401550083784112)
(8.475, 19.715636454878577)
(8.55, 20.032039437350253)
(8.625, 20.353376501196767)
(8.700000000000001, 20.682014400898723)
(8.775, 21.011474647496488)
(8.85, 21.3467414654683)
(8.925, 21.68756413929714)
(9.0, 22.040792216907835)
(9.075000000000001, 22.39601599003396)
(9.15, 22.75531138315639)
(9.225, 23.11690333041467)
(9.3, 23.484612736288092)
(9.375, 23.862561363876367)
(9.450000000000001, 24.246396791804127)
(9.525, 24.63283966110884)
(9.6, 25.026733795579204)
(9.675, 25.418371490396442)
(9.75, 25.823788510028773)
(9.825000000000001, 26.224823022423692)
(9.9, 26.63160393446858)
(9.975, 27.04867421133172)
(10.05, 27.48074730473298)
(10.125, 27.89874021469873)
(10.200000000000001, 28.32302106983119)
(10.275, 28.75147383116677)
(10.35, 29.185241761463036)
(10.425, 29.626039754856386)
(10.5, 30.072152917210428)
(10.575000000000001, 30.52800387024529)
(10.65, 30.990022424998703)
(10.725, 31.457667035953907)
(10.8, 31.932512196557756)
(10.875, 32.41598197094688)
(10.950000000000001, 32.901216782575794)
(11.025, 33.39918794246901)
(11.1, 33.89781096270647)
(11.175, 34.40674340500354)
(11.25, 34.915354931438834)
(11.325000000000001, 35.432410556487156)
(11.4, 35.95261516842918)
(11.475, 36.48201602553527)
(11.55, 37.012058714364926)
(11.625, 37.54928189560186)
(11.700000000000001, 38.08561252959822)
(11.775, 38.628020507727)
(11.85, 39.17391844585262)
(11.925, 39.724449606732655)
(12.0, 40.280837482090135)
(12.075000000000001, 40.83970242675572)
(12.15, 41.397263650732825)
(12.225, 41.95032202402436)
(12.3, 42.50980874317214)
(12.375, 43.07148170162828)
(12.450000000000001, 43.635902502150884)
(12.525, 44.19513850578165)
(12.6, 44.75310087458598)
(12.675, 45.31419217304264)
(12.75, 45.87372903529383)
(12.825000000000001, 46.43335615513113)
(12.9, 46.99041594807421)
(12.975, 47.544035924123854)
(13.05, 48.09562009017535)
(13.125, 48.64343349485096)
(13.200000000000001, 49.189792749527875)
(13.275, 49.72999443110694)
(13.35, 50.26681646751665)
(13.425, 50.80309695840961)
(13.5, 51.3338917937903)
(13.575000000000001, 51.85802762503909)
(13.65, 52.382273771115386)
(13.725, 52.90291964236735)
(13.8, 53.42044661258767)
(13.875, 53.93829449866976)
(13.950000000000001, 54.459160999576696)
(14.025, 55.03492417008901)
(14.1, 55.69955094845178)
(14.175, 56.3893295074814)
(14.25, 57.09186447201668)
(14.325000000000001, 57.82198817204419)
(14.4, 58.56745566171296)
(14.475, 59.34157492066608)
(14.55, 60.14148779200962)
(14.625, 60.96938051505191)
(14.700000000000001, 61.848138402186)
(14.775, 66.10095551694982)
(14.85, 76.75490081142573)
(14.925, 88.09786248975952)
};
\addplot[dashed, black, thick, mark = none] coordinates{
(0.0, 0.4969173404829157)
(0.075, 0.5062340735347652)
(0.15, 0.5163977823186011)
(0.225, 0.5269434605501954)
(0.3, 0.53835272188107)
(0.375, 0.550268507914407)
(0.45, 0.562831981272204)
(0.525, 0.5761012677399898)
(0.6, 0.5904915515001102)
(0.675, 0.6063432835820896)
(0.75, 0.6221950156640689)
(0.8250000000000001, 0.6391677450383829)
(0.9, 0.6574524564289111)
(0.975, 0.6764180698784872)
(1.05, 0.7090598502945483)
(1.125, 0.7954098565389183)
(1.2, 0.8221975399838976)
(1.2750000000000001, 0.8511690922280178)
(1.35, 0.8842177531427782)
(1.425, 0.9161703278161446)
(1.5, 0.9497006023824264)
(1.575, 0.9857551967773736)
(1.6500000000000001, 1.02340409843253)
(1.725, 1.0635690162327052)
(1.8, 1.1058513733628457)
(1.875, 1.1509735903002347)
(1.95, 1.1987446823209924)
(2.025, 1.7221922920558328)
(2.1, 1.7916692131296517)
(2.1750000000000003, 1.843243392260701)
(2.25, 1.8896692875306573)
(2.325, 1.9366432259213102)
(2.4, 1.9850370942155877)
(2.475, 2.0365116291428738)
(2.5500000000000003, 2.0894891308102537)
(2.625, 2.143712185024672)
(2.7, 2.2025603910304272)
(2.775, 2.2620978027788774)
(2.85, 2.3243173043452843)
(2.9250000000000003, 2.3913861571614956)
(3.0, 2.462689888637638)
(3.075, 2.5398061986666276)
(3.15, 2.6193803990551072)
(3.225, 2.7038454691116254)
(3.3000000000000003, 2.7930602462141843)
(3.375, 2.890636832749197)
(3.45, 2.9943913599175214)
(3.525, 3.1081933442986243)
(3.6, 3.229892131827953)
(3.6750000000000003, 3.3595624556583292)
(3.75, 3.497171101055166)
(3.825, 3.6439885316164413)
(3.9, 3.796552111261389)
(3.975, 3.9640457141035075)
(4.05, 4.160718461280919)
(4.125, 4.3076438397296055)
(4.2, 4.464525334870954)
(4.275, 4.632600195568357)
(4.3500000000000005, 4.812590842299097)
(4.425, 5.005867382864917)
(4.5, 5.2136587624455615)
(4.575, 5.438995825572157)
(4.65, 5.677577264115598)
(4.7250000000000005, 5.928796909169658)
(4.8, 6.202577662692413)
(4.875, 6.492376221970085)
(4.95, 6.800127345292409)
(5.025, 7.128961521394276)
(5.1000000000000005, 7.478231062951222)
(5.175, 7.847404534209848)
(5.25, 8.235319419459582)
(5.325, 8.641660178721844)
(5.4, 9.071799295316191)
(5.4750000000000005, 9.520206515933772)
(5.55, 9.991232970805578)
(5.625, 10.479414836091928)
(5.7, 10.992316767595174)
(5.775, 11.52684979499866)
(5.8500000000000005, 12.083105258822497)
(5.925, 12.66119941063775)
(6.0, 13.257935332240347)
(6.075, 13.880611961555939)
(6.15, 14.515802242127442)
(6.2250000000000005, 15.172058968111198)
(6.3, 15.844051174605875)
(6.375, 16.53359736833015)
(6.45, 17.238314392077356)
(6.525, 17.967560497317578)
(6.6000000000000005, 18.71260020885425)
(6.675, 19.468443012815573)
(6.75, 20.24003790465511)
(6.825, 21.023714656200926)
(6.9, 21.815313121945906)
(6.9750000000000005, 22.6223979576924)
(7.05, 23.43845077177757)
(7.125, 24.258979271348437)
(7.2, 25.086009555214844)
(7.275, 25.916651941467666)
(7.3500000000000005, 26.750399905404436)
(7.425, 27.58905534637654)
(7.5, 28.4297036714239)
(7.575, 29.272876316299936)
(7.65, 30.108550734842787)
(7.7250000000000005, 30.937416132795164)
(7.8, 31.767742979069403)
(7.875, 32.594872907139575)
(7.95, 33.41305146423836)
(8.025, 34.22857284257013)
(8.1, 35.029454826632374)
(8.175, 35.81735815315447)
(8.25, 36.594126239906046)
(8.325, 37.364309505525604)
(8.4, 38.123291101905465)
(8.475, 38.86482665894314)
(8.55, 39.598083443384816)
(8.625, 40.31560474731559)
(8.700000000000001, 41.01306435155538)
(8.775, 41.69369238904286)
(8.85, 42.367876768020324)
(8.925, 43.02274677883504)
(9.0, 43.66313516536952)
(9.075000000000001, 44.28660064463157)
(9.15, 44.893168127672126)
(9.225, 45.47962408891983)
(9.3, 46.04844302610147)
(9.375, 46.60949801907323)
(9.450000000000001, 47.1497439808258)
(9.525, 47.67525090410508)
(9.6, 48.182755441237816)
(9.675, 48.677671593961826)
(9.75, 49.15570635783163)
(9.825000000000001, 49.61625356394102)
(9.9, 50.06293361836004)
(9.975, 50.49758993885831)
(10.05, 50.9185866997574)
(10.125, 51.322594123914875)
(10.200000000000001, 51.71207010169023)
(10.275, 52.08970502658508)
(10.35, 52.45745856794007)
(10.425, 52.810713877647544)
(10.5, 53.1511898182224)
(10.575000000000001, 53.48158508684989)
(10.65, 53.80176682459166)
(10.725, 54.11220003773194)
(10.8, 54.412245342629916)
(10.875, 54.70402017861555)
(10.950000000000001, 54.98860402456296)
(11.025, 55.26488418686344)
(11.1, 55.53651428632163)
(11.175, 55.799417214266924)
(11.25, 56.05691444415805)
(11.325000000000001, 56.305900398311096)
(11.4, 56.552320514217236)
(11.475, 56.793368146803815)
(11.55, 57.027374255657804)
(11.625, 57.25936256938559)
(11.700000000000001, 57.491035343134776)
(11.775, 57.718307164551106)
(11.85, 57.93951729690519)
(11.925, 58.15959812828327)
(12.0, 58.37749509086223)
(12.075000000000001, 58.59598991866376)
(12.15, 58.80997584624501)
(12.225, 59.02287399126851)
(12.3, 59.232583521771595)
(12.375, 59.44123848445152)
(12.450000000000001, 59.65192784962494)
(12.525, 59.85984378446029)
(12.6, 60.06953670759607)
(12.675, 60.27927945283375)
(12.75, 60.49015980273105)
(12.825000000000001, 60.70515877971723)
(12.9, 60.916769853775456)
(12.975, 61.13025756033789)
(13.05, 61.34844515184448)
(13.125, 61.564581733490286)
(13.200000000000001, 61.78546802218213)
(13.275, 62.0060055561608)
(13.35, 62.22949920151778)
(13.425, 62.45551716670342)
(13.5, 62.687380925176505)
(13.575000000000001, 62.92040719936015)
(13.65, 63.160151153614166)
(13.725, 63.40534232434055)
(13.8, 63.65456908531936)
(13.875, 63.91151827208979)
(13.950000000000001, 64.17222902755229)
(14.025, 64.49729333127846)
(14.1, 64.92511572013531)
(14.175, 65.37155496772856)
(14.25, 65.84285544416072)
(14.325000000000001, 66.34035404249892)
(14.4, 66.85715040163257)
(14.475, 67.40418877660832)
(14.55, 67.96977758085131)
(14.625, 68.57305680516768)
(14.700000000000001, 69.21068006504774)
(14.775, 72.6176897690646)
(14.85, 81.23674732089951)
(14.925, 90.38879341497959)
};
