# Supplementary material for: CausalSim: A Causal Framework for Unbiased Trace-Driven Simulation
Source: arXiv:2201.01811 source file (2023-05-05)
Supplement: Supplementary file 9 [file new_linear_bba_bola_basic_v1.tex]

\addplot[solid, green!70!black, thick, mark = none] coordinates{
(0.0, 0.515735615519724)
(0.08112770646241939, 0.5298561734608966)
(0.16225541292483878, 0.549981220958911)
(0.24338311938725818, 0.5748998526198038)
(0.32451082584967755, 0.6036513501144806)
(0.40563853231209696, 0.6377968807277201)
(0.48676623877451636, 0.6758553370355015)
(0.5678939452369357, 0.7198482305219612)
(0.6490216516993551, 0.7708363543421417)
(0.7301493581617745, 0.8272285187634794)
(0.8112770646241939, 0.8896551951894432)
(0.8924047710866133, 0.9574558897687802)
(0.9735324775490327, 1.031931575238806)
(1.054660184011452, 1.1102701489904)
(1.1357878904738714, 1.1906302342261308)
(1.2169155969362908, 1.2768346892971876)
(1.2980433033987102, 1.3651407157131388)
(1.3791710098611296, 1.4562788597034002)
(1.460298716323549, 1.5525108123343825)
(1.5414264227859684, 1.6500537451852748)
(1.6225541292483878, 1.7512093792528673)
(1.7036818357108072, 1.8558676322286174)
(1.7848095421732266, 1.9628276062011567)
(1.865937248635646, 2.0770930424678533)
(1.9470649550980654, 2.209532067126591)
(2.028192661560485, 2.348826217362722)
(2.109320368022904, 2.4810750998521596)
(2.1904480744853236, 2.6115226354745444)
(2.271575780947743, 2.7255979295719412)
(2.3527034874101624, 2.8311468484986224)
(2.4338311938725816, 2.9408989101150933)
(2.5149589003350012, 3.056585408910242)
(2.5960866067974204, 3.1756844592701965)
(2.67721431325984, 3.3023791889195553)
(2.7583420197222592, 3.4389513038899184)
(2.839469726184679, 3.581928207720913)
(2.920597432647098, 3.731750229646707)
(3.0017251391095177, 3.891709831440968)
(3.082852845571937, 4.06434891368276)
(3.1639805520343565, 4.2459547003294364)
(3.2451082584967756, 4.444753342073868)
(3.326235964959195, 4.6589034621186265)
(3.4073636714216144, 4.887914693816567)
(3.4884913778840336, 5.136600636295759)
(3.5696190843464533, 5.409324551967506)
(3.6507467908088724, 5.696449235093079)
(3.731874497271292, 6.000016212121803)
(3.8130022037337112, 6.317253410374938)
(3.894129910196131, 6.649571884898338)
(3.97525761665855, 6.989836300601961)
(4.05638532312097, 7.333943589621961)
(4.137513029583389, 7.690930508741387)
(4.218640736045808, 8.063118793922214)
(4.299768442508228, 8.452079619931823)
(4.380896148970647, 8.856722171167382)
(4.462023855433067, 9.274964891249187)
(4.543151561895486, 9.709729965094901)
(4.624279268357905, 10.162638604884872)
(4.705406974820325, 10.630408356328026)
(4.7865346812827445, 11.116061479167975)
(4.867662387745163, 11.619477883613579)
(4.948790094207583, 12.133131942753597)
(5.0299178006700025, 12.665970346027725)
(5.111045507132421, 13.208526014901341)
(5.192173213594841, 13.756655851580227)
(5.2733009200572605, 14.315463672187695)
(5.35442862651968, 14.870959016056307)
(5.435556332982099, 15.43715235881869)
(5.5166840394445185, 16.002084758774135)
(5.597811745906938, 16.568117981815004)
(5.678939452369358, 17.133040374287855)
(5.7600671588317764, 17.683151692520497)
(5.841194865294196, 18.227458670848193)
(5.922322571756616, 18.761237777486226)
(6.003450278219035, 19.287991631342756)
(6.084577984681454, 19.810122028240514)
(6.165705691143874, 20.327068549154205)
(6.246833397606293, 20.838811179118625)
(6.327961104068713, 21.34427911749615)
(6.409088810531132, 21.84675481857785)
(6.490216516993551, 22.348650085669057)
(6.571344223455971, 22.84205900751992)
(6.65247192991839, 23.335287794684085)
(6.733599636380809, 23.828176327440026)
(6.814727342843229, 24.322275765589932)
(6.8958550493056485, 24.811411492372848)
(6.976982755768067, 25.30076738377285)
(7.058110462230487, 25.789823050695006)
(7.1392381686929065, 26.27636683948588)
(7.220365875155326, 26.75895767265184)
(7.301493581617745, 27.241648580643744)
(7.3826212880801645, 27.718855388173736)
(7.463748994542584, 28.195421716817666)
(7.544876701005004, 28.667644798015473)
(7.6260044074674225, 29.13744606842536)
(7.707132113929842, 29.599281382689835)
(7.788259820392262, 30.056213030482894)
(7.869387526854681, 30.51268433407659)
(7.9505152333171, 30.9634213501435)
(8.03164293977952, 31.40648262706025)
(8.11277064624194, 31.84359945931573)
(8.193898352704359, 32.27518215369632)
(8.275026059166779, 32.70628448891236)
(8.356153765629196, 33.13379413787689)
(8.437281472091616, 33.55833156451079)
(8.518409178554036, 33.97764508523023)
(8.599536885016455, 34.39498713187851)
(8.680664591478875, 34.809537090882856)
(8.761792297941295, 35.21916336845059)
(8.842920004403714, 35.62299531359597)
(8.924047710866134, 36.022804250738275)
(9.005175417328552, 36.418970464216095)
(9.086303123790971, 36.814296049155956)
(9.167430830253391, 37.20619907504841)
(9.24855853671581, 37.59047639920369)
(9.32968624317823, 37.9786566415709)
(9.41081394964065, 38.36152291068032)
(9.49194165610307, 38.74198738396699)
(9.573069362565489, 39.1256242292362)
(9.654197069027907, 39.50369691418273)
(9.735324775490326, 39.88125921751694)
(9.816452481952746, 40.256369687615425)
(9.897580188415166, 40.626646543620666)
(9.978707894877585, 40.997123549277795)
(10.059835601340005, 41.36356753944925)
(10.140963307802425, 41.728670526953)
(10.222091014264842, 42.09552482391084)
(10.303218720727262, 42.45900659923424)
(10.384346427189682, 42.82098725216844)
(10.465474133652101, 43.181857074534626)
(10.546601840114521, 43.540635333038516)
(10.62772954657694, 43.89929350175126)
(10.70885725303936, 44.25101648502585)
(10.78998495950178, 44.59995738813911)
(10.871112665964198, 44.94832786474447)
(10.952240372426617, 45.29124426333569)
(11.033368078889037, 45.63392048234465)
(11.114495785351457, 45.97571604288527)
(11.195623491813876, 46.313848864796206)
(11.276751198276296, 46.652251888737204)
(11.357878904738715, 46.98887358077635)
(11.439006611201135, 47.320221329488064)
(11.520134317663553, 47.65202942239913)
(11.601262024125973, 47.98032488891945)
(11.682389730588392, 48.30965112614702)
(11.763517437050812, 48.63207220038423)
(11.844645143513231, 48.96098813082542)
(11.925772849975651, 49.28886328307676)
(12.00690055643807, 49.61608794895944)
(12.088028262900488, 49.94579447052561)
(12.169155969362908, 50.276561785246834)
(12.250283675825328, 50.6072290251421)
(12.331411382287747, 50.94404085935054)
(12.412539088750167, 51.28094276090233)
(12.493666795212587, 51.62335878536381)
(12.574794501675006, 51.97113882049609)
(12.655922208137426, 52.32497338259817)
(12.737049914599844, 52.68792476134405)
(12.818177621062263, 53.06020311386824)
(12.899305327524683, 53.442859225843165)
(12.980433033987103, 53.831549849822714)
(13.061560740449522, 54.232909946767194)
(13.142688446911942, 54.64891099074778)
(13.223816153374361, 55.08240511430397)
(13.30494385983678, 55.522093869586286)
(13.386071566299199, 55.984159355950446)
(13.467199272761619, 56.464878789871186)
(13.548326979224038, 56.97056689286579)
(13.629454685686458, 57.499632475201714)
(13.710582392148877, 58.049453576439106)
(13.791710098611297, 58.621421236658655)
(13.872837805073717, 59.22226048416401)
(13.953965511536135, 59.86428052254671)
(14.035093217998554, 60.542797849952414)
(14.116220924460974, 61.26368685866422)
(14.197348630923393, 62.04305959565968)
(14.278476337385813, 62.896167464413146)
(14.359604043848233, 63.8276339218834)
(14.440731750310652, 64.8747968856314)
(14.521859456773072, 66.11386333561605)
(14.60298716323549, 67.69813789770612)
(14.68411486969791, 69.91051208988961)
(14.765242576160329, 73.92722538642143)
(14.846370282622749, 84.71792359146934)
(14.927497989085168, 94.46408079320908)
(15.008625695547588, 99.50543021016814)
(15.089753402010007, 99.87879937829514)
(15.170881108472425, 99.94587953412767)
(15.252008814934845, 99.98143611978676)
(15.333136521397265, 99.99496623625484)
(15.414264227859684, 99.99902927418832)
(15.495391934322104, 99.99974981293514)
(15.576519640784523, 99.99986990272627)
(15.657647347246943, 99.99991994013924)
(15.738775053709363, 99.99995997006963)
(15.81990276017178, 99.99995997006963)
(15.9010304666342, 99.99996997755221)
(15.98215817309662, 99.99997998503481)
(16.06328587955904, 99.99997998503481)
(16.144413586021457, 99.99997998503481)
};
\addplot[solid, blue, thick, mark = none] coordinates{
(0.0, 0.49727243146563277)
(0.075, 0.49727243146563277)
(0.15, 0.49727243146563277)
(0.225, 0.49727243146563277)
(0.3, 0.49727243146563277)
(0.375, 0.49727243146563277)
(0.45, 0.4972824650087708)
(0.525, 0.49729249855190893)
(0.6, 0.49729249855190893)
(0.675, 0.49729249855190893)
(0.75, 0.4973225991813231)
(0.8250000000000001, 0.49733263272446115)
(0.9, 0.49734266626759915)
(0.975, 0.49734266626759915)
(1.05, 0.4973627333538754)
(1.125, 0.49737276689701343)
(1.2, 0.49737276689701343)
(1.2750000000000001, 0.4974028675264276)
(1.35, 0.49743296815584176)
(1.425, 0.4974530352421179)
(1.5, 0.4974630687852559)
(1.575, 0.49747310232839403)
(1.6500000000000001, 0.49748313587153214)
(1.725, 0.4975333035872225)
(1.8, 0.4975935048460508)
(1.875, 0.4976838067342934)
(1.95, 0.4977038738205696)
(2.025, 1.6343237075868335)
(2.1, 1.672300668364409)
(2.1750000000000003, 1.712194035881355)
(2.25, 1.7554085061770004)
(2.325, 1.8009407249375387)
(2.4, 1.8495833420708774)
(2.475, 1.9013463911201538)
(2.5500000000000003, 1.9564405764912678)
(2.625, 2.015217072194052)
(2.7, 2.0777461130304724)
(2.775, 2.145974206369313)
(2.85, 2.219369574424258)
(2.9250000000000003, 2.2975810431854735)
(3.0, 2.381933040347185)
(3.075, 2.471301809077928)
(3.15, 2.568948250897576)
(3.225, 2.6751834056434065)
(3.3000000000000003, 2.7901878770919057)
(3.375, 2.9137609943803127)
(3.45, 3.0476485940146505)
(3.525, 3.1943590617794353)
(3.6, 3.3578857478436164)
(3.6750000000000003, 3.5400647906014595)
(3.75, 3.7469564501083577)
(3.825, 3.9969722780226578)
(3.9, 4.284664060420392)
(3.975, 4.528860433314614)
(4.05, 4.731046361089759)
(4.125, 4.941740733445983)
(4.2, 5.171308200444908)
(4.275, 5.411731961119218)
(4.3500000000000005, 5.666734459973136)
(4.425, 5.9352220408046135)
(4.5, 6.213432124936877)
(4.575, 6.503070414703395)
(4.65, 6.802100100847142)
(4.7250000000000005, 7.106066290214817)
(4.8, 7.420216525867628)
(4.875, 7.7358517259048725)
(4.95, 8.052590615687304)
(5.025, 8.369730847195259)
(5.1000000000000005, 8.690111913136809)
(5.175, 9.010412710733252)
(5.25, 9.335820581786972)
(5.325, 9.665201735923365)
(5.4, 9.999419057852306)
(5.4750000000000005, 10.341934119956427)
(5.55, 10.686074616048913)
(5.625, 11.035211816624155)
(5.7, 11.38009479490886)
(5.775, 11.718726875818549)
(5.8500000000000005, 12.044746793003691)
(5.925, 12.364435544468714)
(6.0, 12.677702828325375)
(6.075, 12.993428330250861)
(6.15, 13.311882955909901)
(6.2250000000000005, 13.628702114037438)
(6.3, 13.948922643288778)
(6.375, 14.272434174689405)
(6.45, 14.596547718678313)
(6.525, 14.922296730198727)
(6.6000000000000005, 15.251557481817462)
(6.675, 15.582544002855947)
(6.75, 15.916159312196603)
(6.825, 16.25370777044738)
(6.9, 16.593413440472844)
(6.9750000000000005, 16.936931856890773)
(7.05, 17.27995862969493)
(7.125, 17.629256366960387)
(7.2, 17.978875177606255)
(7.275, 18.328764893916855)
(7.3500000000000005, 18.680751620743308)
(7.425, 19.032828649458004)
(7.5, 19.388698357478887)
(7.575, 19.73710310940505)
(7.65, 20.086561383360714)
(7.7250000000000005, 20.436360797783067)
(7.8, 20.78706323108785)
(7.875, 21.13828740863581)
(7.95, 21.48951158618377)
(8.025, 21.843003344480934)
(8.1, 22.19984630618621)
(8.175, 22.55721101213467)
(8.25, 22.91921121501291)
(8.325, 23.281873631738264)
(8.4, 23.651720065350474)
(8.475, 24.02375381136678)
(8.55, 24.39515544416539)
(8.625, 24.769326334870104)
(8.700000000000001, 25.150099296959667)
(8.775, 25.52981873701973)
(8.85, 25.914775686597864)
(8.925, 26.303886523035157)
(9.0, 26.69693050838257)
(9.075000000000001, 27.088840703355388)
(9.15, 27.48148334697728)
(9.225, 27.87676481244448)
(9.3, 28.269678361731103)
(9.375, 28.663474862813874)
(9.450000000000001, 29.05723122972409)
(9.525, 29.449201625955734)
(9.6, 29.841723867059965)
(9.675, 30.235279563107426)
(9.75, 30.63469484834751)
(9.825000000000001, 31.02838098045576)
(9.9, 31.42185640815811)
(9.975, 31.813967273993686)
(10.05, 32.20472361150563)
(10.125, 32.595269244611664)
(10.200000000000001, 32.9856041733118)
(10.275, 33.375347122966794)
(10.35, 33.76825063871027)
(10.425, 34.15347849395313)
(10.5, 34.54150570773152)
(10.575000000000001, 34.92570010803116)
(10.65, 35.30705501562273)
(10.725, 35.68499851854735)
(10.8, 36.05780484738529)
(10.875, 36.42440041302077)
(10.950000000000001, 36.78227682966927)
(11.025, 37.13880875153727)
(11.1, 37.4927419857325)
(11.175, 37.8380965405447)
(11.25, 38.18035073052722)
(11.325000000000001, 38.52065841314097)
(11.4, 38.85760485880347)
(11.475, 39.18874188298902)
(11.55, 39.51911635789608)
(11.625, 39.84907945753448)
(11.700000000000001, 40.18106933288678)
(11.775, 40.51313947658417)
(11.85, 40.84603237081888)
(11.925, 41.17950721055561)
(12.0, 41.51936338372814)
(12.075000000000001, 41.85802556526724)
(12.15, 42.2004703925694)
(12.225, 42.55254742128409)
(12.3, 42.90757431168139)
(12.375, 43.27610635114251)
(12.450000000000001, 43.648691942031405)
(12.525, 44.024187260430345)
(12.6, 44.411732864138095)
(12.675, 44.81070667348011)
(12.75, 45.21912204691504)
(12.825000000000001, 45.63636693831147)
(12.9, 46.06825076914633)
(12.975, 46.51510464634319)
(13.05, 46.97574461181175)
(13.125, 47.45405364674644)
(13.200000000000001, 47.94935950375701)
(13.275, 48.460397956408066)
(13.35, 48.9882726944448)
(13.425, 49.53260244322796)
(13.5, 50.09217314403783)
(13.575000000000001, 50.66010178628172)
(13.65, 51.2438733931406)
(13.725, 51.82959150736828)
(13.8, 52.42573447291641)
(13.875, 53.02810826875327)
(13.950000000000001, 53.627993745891885)
(14.025, 54.23580572210959)
(14.1, 54.836423647897284)
(14.175, 55.436770668020266)
(14.25, 56.03997724793758)
(14.325000000000001, 56.64076574395863)
(14.4, 57.24504591299172)
(14.475, 57.85250671519958)
(14.55, 58.47057297250438)
(14.625, 59.099174450104144)
(14.700000000000001, 59.74330785248163)
(14.775, 60.409535116849135)
(14.85, 61.10333455776005)
(14.925, 61.83422800765238)
};
\addplot[solid, red, thick, mark = none] coordinates{
(0.0008446301757070708,0.5086303028774615)
(0.08530764774641415,0.5129735503235769)
(0.16977066531712123,0.5184076133725186)
(0.2542336828878283,0.5252227090195339)
(0.3386967004585354,0.5334588671950017)
(0.42315971802924246,0.5444971204969956)
(0.5076227355999496,0.5603689878922471)
(0.5920857531706567,0.5825855992525611)
(0.6765487707413638,0.6055928017378593)
(0.7610117883120708,0.6296207674478207)
(0.8454748058827779,0.6547795786909872)
(0.929937823453485,0.6800684872078853)
(1.014400841024192,0.7073989221741096)
(1.098863858594899,0.7371011305152863)
(1.1833268761656062,0.7702258979038628)
(1.2677898937363135,0.807073448817681)
(1.3522529113070205,0.8479740301823673)
(1.4367159288777276,0.8977612560911794)
(1.5211789464484347,0.9560648496881118)
(1.6056419640191417,1.017150523446381)
(1.6901049815898488,1.086572430206065)
(1.7745679991605559,1.168823929652201)
(1.859031016731263,1.2729217636026458)
(1.94349403430197,1.394252482581226)
(2.027957051872677,1.5481175274752932)
(2.112420069443384,1.724989774854659)
(2.196883087014091,1.8335609535249506)
(2.2813461045847983,1.9017319249602926)
(2.3658091221555053,1.967891392394093)
(2.4502721397262124,2.0378236807661088)
(2.5347351572969194,2.1121292390320243)
(2.6191981748676265,2.189026735289976)
(2.7036611924383336,2.2712281973231385)
(2.7881242100090406,2.3595842611520634)
(2.8725872275797477,2.4516931309540144)
(2.9570502451504552,2.549886550173565)
(3.0415132627211623,2.6538342718850885)
(3.1259762802918694,2.7664584810062487)
(3.2104392978625764,2.888009364601913)
(3.2949023154332835,3.0185970049806237)
(3.3793653330039906,3.1615038564334554)
(3.4638283505746976,3.317740674702475)
(3.5482913681454047,3.4860064870503673)
(3.6327543857161118,3.671525199391585)
(3.717217403286819,3.8773791163653066)
(3.801680420857526,4.107090871844878)
(3.886143438428233,4.358358744833512)
(3.97060645599894,4.63163307204797)
(4.055069473569647,4.9272541078964744)
(4.139532491140354,5.230841099890388)
(4.223995508711061,5.524930990901898)
(4.308458526281768,5.81661908609067)
(4.392921543852475,6.122027439916826)
(4.477384561423182,6.440475543563923)
(4.5618475789938895,6.776096487343588)
(4.6463105965645966,7.125547772069177)
(4.730773614135304,7.488939480049233)
(4.815236631706011,7.861488034603473)
(4.899699649276718,8.241312029004085)
(4.984162666847425,8.622627138311316)
(5.068625684418132,9.00995674465798)
(5.153088701988839,9.402340129714988)
(5.237551719559546,9.792671980840074)
(5.322014737130253,10.18378441560755)
(5.40647775470096,10.58002068146353)
(5.490940772271667,10.978168376495105)
(5.575403789842374,11.378918017001311)
(5.659866807413081,11.780818518005914)
(5.744329824983788,12.183699752304799)
(5.8287928425544955,12.587351562763477)
(5.9132558601252025,12.989252063768078)
(5.99771887769591,13.3831265637317)
(6.082181895266617,13.772637801284022)
(6.166644912837324,14.158866584545265)
(6.251107930408031,14.542803654292314)
(6.335570947978738,14.92719106075613)
(6.420033965549445,15.310327531895599)
(6.504496983120152,15.694885065563522)
(6.588960000690859,16.08071354952098)
(6.673423018261566,16.472136216248888)
(6.757886035832273,16.863488830598637)
(6.84234905340298,17.262697318785257)
(6.926812070973687,17.66118526822505)
(7.011275088544394,18.06265544747808)
(7.095738106115102,18.469219435371826)
(7.180201123685809,18.87870560818324)
(7.2646641412565165,19.290553546887008)
(7.349127158827224,19.70509349840876)
(7.433590176397931,20.11886287377072)
(7.518053193968638,20.536885429235436)
(7.602516211539345,20.952155926986606)
(7.686979229110052,21.365545018009964)
(7.771442246680759,21.7827869898323)
(7.855905264251466,22.199218355564458)
(7.940368281822173,22.610856137133734)
(8.02483129939288,23.026016552576362)
(8.109294316963588,23.438364865409866)
(8.193757334534293,23.84874170417221)
(8.278220352105002,24.264992935217663)
(8.362683369675707,24.682214892074803)
(8.447146387246416,25.10345985693503)
(8.531609404817122,25.523433871505723)
(8.61607242238783,25.94860176954309)
(8.700535439958536,26.373359360794062)
(8.784998457529245,26.804331598736375)
(8.86946147509995,27.236254547525185)
(8.953924492670659,27.67282096823795)
(9.038387510241364,28.110147957627916)
(9.122850527812073,28.551818194464)
(9.207313545382778,28.99183719667195)
(9.291776562953487,29.432596752591913)
(9.376239580524192,29.872705822143214)
(9.460702598094901,30.313825647436587)
(9.545165615665606,30.75135278647845)
(9.629628633236315,31.191872162816136)
(9.71409165080702,31.630730297043097)
(9.79855466837773,32.067506874890356)
(9.883017685948435,32.50367299629933)
(9.967480703519144,32.936616708312805)
(10.051943721089849,33.36738879660322)
(10.136406738660558,33.79948187259614)
(10.220869756231263,34.2326457492267)
(10.305332773801972,34.6605857199428)
(10.389795791372677,35.086524194139955)
(10.474258808943386,35.510711358883036)
(10.558721826514091,35.93235662304705)
(10.6431848440848,36.35093959753708)
(10.727647861655505,36.76334795526615)
(10.812110879226214,37.17337453213768)
(10.89657389679692,37.5767461330837)
(10.981036914367628,37.97581451651399)
(11.065499931938334,38.36594621798719)
(11.149962949509042,38.753425936572775)
(11.234425967079748,39.13220915278354)
(11.318888984650457,39.5037569590783)
(11.403352002221162,39.86945038805515)
(11.48781501979187,40.230390262799496)
(11.572278037362576,40.5874172118493)
(11.656741054933285,40.94219247731529)
(11.74120407250399,41.298618977409404)
(11.825667090074699,41.650982439570065)
(11.910130107645404,42.00335590921332)
(11.994593125216113,42.36253446702099)
(12.079056142786818,42.725275688632394)
(12.163519160357527,43.09336090594938)
(12.247982177928233,43.46779086723143)
(12.332445195498941,43.84302142712106)
(12.416908213069647,44.23768651820967)
(12.501371230640355,44.63843615871587)
(12.58583424821106,45.04619103703839)
(12.67029726578177,45.466275133917634)
(12.754760283352475,45.903702198133544)
(12.839223300923184,46.354999633225766)
(12.923686318493889,46.82758298379699)
(13.008149336064598,47.312165305999294)
(13.092612353635303,47.814651014563594)
(13.177075371206012,48.3370716284566)
(13.261538388776717,48.88225926525263)
(13.346001406347426,49.44015640494398)
(13.430464423918131,50.026765012199625)
(13.51492744148884,50.62537259108636)
(13.599390459059547,51.243274596415745)
(13.683853476630254,51.87815929970839)
(13.768316494200961,52.52290137335686)
(13.852779511771669,53.1760497323849)
(13.937242529342376,53.831489804927145)
(14.021705546913083,54.49033242155159)
(14.106168564483792,55.152737701979774)
(14.190631582054497,55.81786501767372)
(14.275094599625206,56.4929798009972)
(14.359557617195911,57.17932297979199)
(14.44402063476662,57.881487988569056)
(14.528483652337325,58.63407069465839)
(14.612946669908034,59.55765125584399)
(14.69740968747874,60.78183657921028)
(14.781872705049448,62.75888481817855)
(14.866335722620153,67.02982820254705)
(14.950798740190862,92.24783370526143)
(15.035261757761567,98.85462360206728)
(15.119724775332276,99.75017320450502)
(15.204187792902982,99.94536915251534)
(15.28865081047369,99.98847138005087)
(15.373113828044396,99.99895922181014)
(15.457576845615105,99.99977983538292)
(15.54203986318581,99.99983988027849)
(15.626502880756519,99.99986990272627)
(15.710965898327224,99.99990993265665)
(15.795428915897933,99.99992994762184)
(15.879891933468638,99.99994996258704)
(15.964354951039347,99.99995997006963)
(16.048817968610052,99.99995997006963)
(16.133280986180758,99.99995997006963)
(16.217744003751466,99.99997998503481)
(16.302207021322175,99.99997998503481)
(16.38667003889288,99.99997998503481)
(16.471133056463586,99.99997998503481)
(16.555596074034295,99.99997998503481)
(16.640059091605004,99.9999899925174)
(16.72452210917571,99.9999899925174)
(16.808985126746414,99.9999899925174)
};
\addplot[dashed, magenta, thick, mark = none] coordinates{
(0.0, 0.5978301732190421)
(0.075, 0.6133760916944118)
(0.15, 0.6302307014301745)
(0.225, 0.6474937562089899)
(0.3, 0.6658404406938631)
(0.375, 0.6855625013441176)
(0.45, 0.7072100886259058)
(0.525, 0.729924634387505)
(0.6, 0.7542562890950675)
(0.675, 0.7787713272913476)
(0.75, 0.8055703234834727)
(0.8250000000000001, 0.8346949557370608)
(0.9, 0.8651199436379183)
(0.975, 0.8980706223152032)
(1.05, 0.9571367769084845)
(1.125, 1.0989005493002337)
(1.2, 1.1451548665226605)
(1.2750000000000001, 1.1934430733472272)
(1.35, 1.2504586671121218)
(1.425, 1.3082328016712572)
(1.5, 1.3678491067306908)
(1.575, 1.431733245709368)
(1.6500000000000001, 1.5001519582272418)
(1.725, 1.5731302511236822)
(1.8, 1.6536022602181697)
(1.875, 1.7413345883432452)
(1.95, 1.8342933458967696)
(2.025, 2.4780944254920385)
(2.1, 2.60748814800848)
(2.1750000000000003, 2.7090742651448503)
(2.25, 2.8046754120585313)
(2.325, 2.9040109136515504)
(2.4, 3.005847099181626)
(2.475, 3.113043083950127)
(2.5500000000000003, 3.2260573266788466)
(2.625, 3.3446564302003265)
(2.7, 3.4692071614920015)
(2.775, 3.6020601634547047)
(2.85, 3.7420984639298847)
(2.9250000000000003, 3.8896138093768644)
(3.0, 4.044789583284362)
(3.075, 4.211743578535397)
(3.15, 4.3851493383440365)
(3.225, 4.567940998529765)
(3.3000000000000003, 4.762994345620194)
(3.375, 4.968975681515561)
(3.45, 5.1898861005151575)
(3.525, 5.4273593827911935)
(3.6, 5.676210776980837)
(3.6750000000000003, 5.947368271889028)
(3.75, 6.237430937361369)
(3.825, 6.549357916056708)
(3.9, 6.891509827937941)
(3.975, 7.275306462984293)
(4.05, 7.7634899811765194)
(4.125, 8.116119758754019)
(4.2, 8.48711289204264)
(4.275, 8.87052608888531)
(4.3500000000000005, 9.27121067611992)
(4.425, 9.682389800277043)
(4.5, 10.10815624740033)
(4.575, 10.5434836427763)
(4.65, 10.981970235526083)
(4.7250000000000005, 11.424399573283294)
(4.8, 11.862452714150654)
(4.875, 12.295629521340754)
(4.95, 12.727806054956032)
(5.025, 13.160140965220654)
(5.1000000000000005, 13.587757918457367)
(5.175, 14.010456859951196)
(5.25, 14.423828250359808)
(5.325, 14.839166845465568)
(5.4, 15.251346243197514)
(5.4750000000000005, 15.66676819443451)
(5.55, 16.075063196450895)
(5.625, 16.484250109071496)
(5.7, 16.894520651398157)
(5.775, 17.309109041322802)
(5.8500000000000005, 17.720679939296733)
(5.925, 18.130767098134672)
(6.0, 18.538695333173624)
(6.075, 18.95191668254601)
(6.15, 19.333304325399663)
(6.2250000000000005, 19.705797869050517)
(6.3, 20.07650759149294)
(6.375, 20.44800086156897)
(6.45, 20.81621823568746)
(6.525, 21.186994643034872)
(6.6000000000000005, 21.553469874010542)
(6.675, 21.92303761745504)
(6.75, 22.287362260244844)
(6.825, 22.653379032498723)
(6.9, 23.022079872178374)
(6.9750000000000005, 23.391764314206604)
(7.05, 23.76241568735716)
(7.125, 24.13397564233818)
(7.2, 24.505969049201624)
(7.275, 24.879329496617324)
(7.3500000000000005, 25.253565183411)
(7.425, 25.62804260298525)
(7.5, 26.006062658137)
(7.575, 26.38009829021571)
(7.65, 26.755175873934856)
(7.7250000000000005, 27.127711095651325)
(7.8, 27.496295236747248)
(7.875, 27.869213896667404)
(7.95, 28.23931511935181)
(8.025, 28.617751955159736)
(8.1, 28.98364369321676)
(8.175, 29.34897694519451)
(8.25, 29.720561907014904)
(8.325, 30.09275536859331)
(8.4, 30.46615749407463)
(8.475, 30.84332731668778)
(8.55, 31.21890503719434)
(8.625, 31.598592214970793)
(8.700000000000001, 31.97865449533781)
(8.775, 32.36687734095275)
(8.85, 32.75448335119655)
(8.925, 33.146215489936495)
(9.0, 33.53790595061083)
(9.075000000000001, 33.9300381987807)
(9.15, 34.32471280895325)
(9.225, 34.71945410403078)
(9.3, 35.11671275427163)
(9.375, 35.51023704983313)
(9.450000000000001, 35.905778563770525)
(9.525, 36.295701874462665)
(9.6, 36.69002638888403)
(9.675, 37.08318391746809)
(9.75, 37.47364070740014)
(9.825000000000001, 37.86537284614009)
(9.9, 38.250669891548675)
(9.975, 38.637117251568306)
(10.05, 39.027840781120304)
(10.125, 39.411112272539874)
(10.200000000000001, 39.790757772250714)
(10.275, 40.16463502768007)
(10.35, 40.53541143502748)
(10.425, 40.90880522489568)
(10.5, 41.273504970276036)
(10.575000000000001, 41.638121359525165)
(10.65, 41.998494921694416)
(10.725, 42.358118278682554)
(10.8, 42.71624122530845)
(10.875, 43.066195271073305)
(10.950000000000001, 43.41125631193465)
(11.025, 43.754591880879424)
(11.1, 44.08891665203766)
(11.175, 44.42049900647827)
(11.25, 44.75122279276715)
(11.325000000000001, 45.072352288350864)
(11.4, 45.39109779858125)
(11.475, 45.70932650079797)
(11.55, 46.02420428653903)
(11.625, 46.337431620881645)
(11.700000000000001, 46.65159254389409)
(11.775, 46.966295281759564)
(11.85, 47.28467402501251)
(11.925, 47.59957681759294)
(12.0, 47.9187391084795)
(12.075000000000001, 48.24137735003857)
(12.15, 48.56677467954152)
(12.225, 48.8958313432057)
(12.3, 49.22941424479595)
(12.375, 49.56739835011542)
(12.450000000000001, 49.914426595673916)
(12.525, 50.266964681507055)
(12.6, 50.62702149037762)
(12.675, 50.99723941164576)
(12.75, 51.37682656206473)
(12.825000000000001, 51.76616637983822)
(12.9, 52.16448365294575)
(12.975, 52.573937305186305)
(13.05, 52.996636246680126)
(13.125, 53.435272880466144)
(13.200000000000001, 53.89191443859895)
(13.275, 54.3584170270569)
(13.35, 54.83736468590826)
(13.425, 55.33235006440928)
(13.5, 55.835370973961375)
(13.575000000000001, 56.34455190161176)
(13.65, 56.86528598905134)
(13.725, 57.39508088795618)
(13.8, 57.92813501159234)
(13.875, 58.46749085874987)
(13.950000000000001, 59.008280431364646)
(14.025, 59.609169774600026)
(14.1, 60.313295686370225)
(14.175, 61.02494865679097)
(14.25, 61.75203918271648)
(14.325000000000001, 62.49846833108855)
(14.4, 63.252357853206185)
(14.475, 64.02990384536838)
(14.55, 64.82927247268795)
(14.625, 65.65083883775546)
(14.700000000000001, 66.52143527921554)
(14.775, 70.33132728467902)
(14.85, 79.65141799615529)
(14.925, 89.58084202696104)
};
\addplot[dashed, black, thick, mark = none] coordinates{
(0.0, 0.9132228167000467)
(0.075, 0.9406433190096234)
(0.15, 0.9704456021767475)
(0.225, 1.001518835633403)
(0.3, 1.0346836329523585)
(0.375, 1.070040068959561)
(0.45, 1.1073879940031162)
(0.525, 1.1485487699152657)
(0.6, 1.191460855281494)
(0.675, 1.2365745868185642)
(0.75, 1.2849407501989236)
(0.8250000000000001, 1.3361090087058094)
(0.9, 1.3918807092062735)
(0.975, 1.448933367478864)
(1.05, 1.5597362147677818)
(1.125, 1.8411466253317603)
(1.2, 1.9301131455989644)
(1.2750000000000001, 2.025114177870794)
(1.35, 2.1243383677976024)
(1.425, 2.2247634556357787)
(1.5, 2.328551057625787)
(1.575, 2.4406148477216414)
(1.6500000000000001, 2.5584229328268746)
(1.725, 2.68126478167726)
(1.8, 2.8120225492600817)
(1.875, 2.948104297583303)
(1.95, 3.091011149036134)
(2.025, 4.063898576965998)
(2.1, 4.281621368297076)
(2.1750000000000003, 4.439709570846122)
(2.25, 4.583757275314753)
(2.325, 4.728115211743821)
(2.4, 4.873443873984578)
(2.475, 5.022695469402472)
(2.5500000000000003, 5.176040125201613)
(2.625, 5.334608686915207)
(2.7, 5.497020121945178)
(2.775, 5.665466068979776)
(2.85, 5.8389958171725)
(2.9250000000000003, 6.014527061884171)
(3.0, 6.197413806302973)
(3.075, 6.392709829139247)
(3.15, 6.585894273148033)
(3.225, 6.779138762052386)
(3.3000000000000003, 6.975815817486734)
(3.375, 7.176936195193146)
(3.45, 7.380508406135268)
(3.525, 7.588483909419072)
(3.6, 7.805265997386246)
(3.6750000000000003, 8.028773113657081)
(3.75, 8.259815864321753)
(3.825, 8.503648177742498)
(3.9, 8.757077666971595)
(3.975, 9.041570382174752)
(4.05, 9.430371088462843)
(4.125, 9.651416364015375)
(4.2, 9.874753353082099)
(4.275, 10.102503641973103)
(4.3500000000000005, 10.336188368042786)
(4.425, 10.57376600484182)
(4.5, 10.814916312927176)
(4.575, 11.060279771184915)
(4.65, 11.312488347537455)
(4.7250000000000005, 11.564336654516582)
(4.8, 11.821649046992436)
(4.875, 12.086897373165916)
(4.95, 12.352355856473887)
(5.025, 12.620576404978001)
(5.1000000000000005, 12.903628042687517)
(5.175, 13.181305662243659)
(5.25, 13.462355803434228)
(5.325, 13.7460579275124)
(5.4, 14.03535423436103)
(5.4750000000000005, 14.326702075141585)
(5.55, 14.623574046314431)
(5.625, 14.926780753969743)
(5.7, 15.233800312493651)
(5.775, 15.547845123799064)
(5.8500000000000005, 15.86954565928945)
(5.925, 16.19391819263263)
(6.0, 16.524595440010494)
(6.075, 16.871424764296265)
(6.15, 17.17076858367001)
(6.2250000000000005, 17.47143339074626)
(6.3, 17.771537778797207)
(6.375, 18.075214838134475)
(6.45, 18.380553139582464)
(6.525, 18.689324007560455)
(6.6000000000000005, 18.999175683658674)
(6.675, 19.309587778782195)
(6.75, 19.623962837013234)
(6.825, 19.94306142702899)
(6.9, 20.2599583708739)
(6.9750000000000005, 20.58032791117919)
(7.05, 20.910855046318133)
(7.125, 21.23875021353466)
(7.2, 21.56734590453282)
(7.275, 21.899504259334705)
(7.3500000000000005, 22.233594058277372)
(7.425, 22.573268032507908)
(7.5, 22.913732597863422)
(7.575, 23.255348023717335)
(7.65, 23.602877871784735)
(7.7250000000000005, 23.948396215850593)
(7.8, 24.29987901954291)
(7.875, 24.647839189361886)
(7.95, 24.99294722664136)
(8.025, 25.361192563679865)
(8.1, 25.69646324556871)
(8.175, 26.03181398731832)
(8.25, 26.36762507326728)
(8.325, 26.705167453705137)
(8.4, 27.046902969350185)
(8.475, 27.388708537373397)
(8.55, 27.734867360325318)
(8.625, 28.079044701723475)
(8.700000000000001, 28.42402264172922)
(8.775, 28.772463170712744)
(8.85, 29.12335553293197)
(8.925, 29.475739010057822)
(9.0, 29.830674395245328)
(9.075000000000001, 30.189622780953318)
(9.15, 30.545138600131317)
(9.225, 30.905578100745927)
(9.3, 31.26446644155835)
(9.375, 31.62747786519981)
(9.450000000000001, 31.988117515466314)
(9.525, 32.34969786909672)
(9.6, 32.71727270480138)
(9.675, 33.081324906632695)
(9.75, 33.447478679808896)
(9.825000000000001, 33.81425291690597)
(9.9, 34.17380175156965)
(9.975, 34.53548218002601)
(10.05, 34.90890138556599)
(10.125, 35.26690906791007)
(10.200000000000001, 35.62822922699303)
(10.275, 35.98926917656332)
(10.35, 36.3522405702744)
(10.425, 36.71332054977507)
(10.5, 37.07424040955422)
(10.575000000000001, 37.43762211005169)
(10.65, 37.79999305480708)
(10.725, 38.16323465054822)
(10.8, 38.531850264442724)
(10.875, 38.897753850554054)
(10.950000000000001, 39.26676976375236)
(11.025, 39.63466483890004)
(11.1, 40.005061784696416)
(11.175, 40.376049171965875)
(11.25, 40.74973857953592)
(11.325000000000001, 41.11704321321052)
(11.4, 41.49265405743875)
(11.475, 41.86533270926672)
(11.55, 42.235419423102655)
(11.625, 42.60588642127719)
(11.700000000000001, 42.97633340448653)
(11.775, 43.34552945237154)
(11.85, 43.71889862049855)
(11.925, 44.089966067628765)
(12.0, 44.46026293859919)
(12.075000000000001, 44.84107767377668)
(12.15, 45.21267551748443)
(12.225, 45.58376297957983)
(12.3, 45.95780264904069)
(12.375, 46.32883006624053)
(12.450000000000001, 46.70458101522508)
(12.525, 47.07748983915273)
(12.6, 47.45247021197749)
(12.675, 47.83039278468511)
(12.75, 48.208685634248724)
(12.825000000000001, 48.59138177615403)
(12.9, 48.97563908534411)
(12.975, 49.362458310078445)
(13.05, 49.75161928573995)
(13.125, 50.144963389126055)
(13.200000000000001, 50.53743684152641)
(13.275, 50.929149725249566)
(13.35, 51.32481556459765)
(13.425, 51.72268305011657)
(13.5, 52.12825629723344)
(13.575000000000001, 52.53857309110022)
(13.65, 52.95027091756507)
(13.725, 53.37287690005817)
(13.8, 53.794241954709534)
(13.875, 54.22271232200316)
(13.950000000000001, 54.6604796406273)
(14.025, 55.169440190430386)
(14.1, 55.79581853351752)
(14.175, 56.45075823193001)
(14.25, 57.12428182552094)
(14.325000000000001, 57.81962173116839)
(14.4, 58.54351298465863)
(14.475, 59.30812468482684)
(14.55, 60.105390800701684)
(14.625, 60.933720142550584)
(14.700000000000001, 61.80875440566912)
(14.775, 66.05816168749374)
(14.85, 76.73958819008972)
(14.925, 88.14040257900832)
};
