# Supplementary material for: CausalSim: A Causal Framework for Unbiased Trace-Driven Simulation
Source: arXiv:2201.01811 source file (2023-05-05)
Supplement: Supplementary file 10 [file new_linear_bba_puffer_ttp_20190202.tex]

\addplot[solid, green!70!black, thick, mark = none] coordinates{
(0.0, 0.3673941147488215)
(0.08432496574713919, 0.3735176185693642)
(0.16864993149427837, 0.3830654501842892)
(0.25297489724141753, 0.39635184202649304)
(0.33729986298855674, 0.4139327437849458)
(0.4216248287356959, 0.4352683202544155)
(0.5059497944828351, 0.4618572184225613)
(0.5902747602299743, 0.4963905570736742)
(0.6745997259771135, 0.5381995851326162)
(0.7589246917242526, 0.585785655611728)
(0.8432496574713918, 0.6396805464743726)
(0.927574623218531, 0.7013909619500781)
(1.0118995889656701, 0.7715937103558521)
(1.0962245547128093, 0.8461634838546972)
(1.1805495204599485, 0.9255031445400704)
(1.2648744862070878, 1.006188364617589)
(1.349199451954227, 1.0934160650928455)
(1.433524417701366, 1.1857923431224793)
(1.5178493834485052, 1.2800943019588364)
(1.6021743491956444, 1.3776433292684547)
(1.6864993149427836, 1.4750876124337744)
(1.7708242806899228, 1.5766572034360913)
(1.855149246437062, 1.6843664127426894)
(1.9394742121842012, 1.8034363330847674)
(2.0237991779313402, 1.9250523418574923)
(2.1081241436784794, 2.041390857205934)
(2.1924491094256187, 2.1569236483674614)
(2.276774075172758, 2.272005233984318)
(2.361099040919897, 2.3982219278643195)
(2.4454240066670363, 2.532592550515885)
(2.5297489724141755, 2.6761887151076102)
(2.6140739381613147, 2.8331760156858383)
(2.698398903908454, 3.000089838246841)
(2.782723869655593, 3.1778164793962227)
(2.867048835402732, 3.37085993733883)
(2.951373801149871, 3.579486101056345)
(3.0356987668970103, 3.805113045117734)
(3.1200237326441496, 4.053147178817189)
(3.2043486983912888, 4.31760197144594)
(3.288673664138428, 4.604520354405841)
(3.372998629885567, 4.911050064075216)
(3.4573235956327064, 5.234153520269402)
(3.5416485613798456, 5.57763374115063)
(3.625973527126985, 5.937349304398166)
(3.710298492874124, 6.311793505782481)
(3.7946234586212633, 6.702046015714039)
(3.8789484243684025, 7.107486426568917)
(3.9632733901155413, 7.530169335023743)
(4.0475983558626805, 7.961900526097608)
(4.13192332160982, 8.405234145463028)
(4.216248287356959, 8.863602578156254)
(4.3005732531040985, 9.332453482521224)
(4.384898218851237, 9.808531732842809)
(4.469223184598377, 10.29070125801746)
(4.553548150345516, 10.78294233552853)
(4.6378731160926545, 11.280331990593975)
(4.722198081839794, 11.786246207556967)
(4.806523047586933, 12.299871204988722)
(4.890848013334073, 12.821061952535596)
(4.975172979081211, 13.344831017480589)
(5.059497944828351, 13.872910706825573)
(5.14382291057549, 14.405542737826615)
(5.2281478763226295, 14.939737873750273)
(5.312472842069768, 15.474400329702338)
(5.396797807816908, 16.011512187182618)
(5.481122773564047, 16.540800462807972)
(5.565447739311186, 17.07124092402061)
(5.649772705058325, 17.589128202401138)
(5.734097670805464, 18.094156122758527)
(5.8184226365526035, 18.591086515037432)
(5.902747602299742, 19.077099344583658)
(5.987072568046882, 19.554208921864493)
(6.071397533794021, 20.020642653668723)
(6.15572249954116, 20.480477504382133)
(6.240047465288299, 20.938652563270498)
(6.324372431035439, 21.389092669964498)
(6.4086973967825775, 21.837921328284665)
(6.493022362529717, 22.281665866985414)
(6.577347328276856, 22.72482222702971)
(6.661672294023996, 23.165005464824297)
(6.745997259771134, 23.60256204176955)
(6.830322225518273, 24.03774978960527)
(6.914647191265413, 24.46831268060811)
(6.998972157012552, 24.903484313960096)
(7.083297122759691, 25.335376649871343)
(7.16762208850683, 25.76701115404278)
(7.25194705425397, 26.198041365074033)
(7.3362720200011085, 26.631142287265654)
(7.420596985748248, 27.05812776287859)
(7.504921951495387, 27.486676343414153)
(7.5892469172425265, 27.911333276126914)
(7.673571882989665, 28.33694902062211)
(7.757896848736805, 28.762605051326645)
(7.842221814483944, 29.187866277179598)
(7.9265467802310825, 29.612176748491986)
(8.010871745978221, 30.035721781826812)
(8.095196711725361, 30.458662522021452)
(8.1795216774725, 30.87328818860714)
(8.26384664321964, 31.292707914104966)
(8.348171608966778, 31.710145558102987)
(8.432496574713918, 32.125149915056525)
(8.516821540461057, 32.54315962322726)
(8.601146506208197, 32.95960622647537)
(8.685471471955335, 33.376109230416574)
(8.769796437702475, 33.795327524867666)
(8.854121403449614, 34.210646114254104)
(8.938446369196754, 34.627833983754186)
(9.022771334943892, 35.04513465464043)
(9.107096300691031, 35.46324104971358)
(9.191421266438171, 35.883289240077204)
(9.275746232185309, 36.300863857187)
(9.360071197932449, 36.718970252260156)
(9.444396163679588, 37.13860752328845)
(9.528721129426728, 37.562595704926075)
(9.613046095173866, 37.982345777340534)
(9.697371060921006, 38.401588243517246)
(9.781696026668145, 38.81897754406405)
(9.866020992415285, 39.23955751239103)
(9.950345958162423, 39.659654046205866)
(10.034670923909562, 40.07965389311827)
(10.118995889656702, 40.50101541390656)
(10.20332085540384, 40.919065408286635)
(10.28764582115098, 41.33424702456129)
(10.37197078689812, 41.7509836885167)
(10.456295752645259, 42.165093691622765)
(10.540620718392397, 42.57727801392211)
(10.624945684139536, 42.987464140237904)
(10.709270649886676, 43.396046875421746)
(10.793595615633816, 43.80639414657493)
(10.877920581380954, 44.2093287552085)
(10.962245547128093, 44.61065191546825)
(11.046570512875233, 45.009074468655115)
(11.130895478622373, 45.403774576098435)
(11.21522044436951, 45.79422045983485)
(11.29954541011665, 46.18030737572006)
(11.38387037586379, 46.56766733582061)
(11.468195341610928, 46.95232811989498)
(11.552520307358067, 47.33442670105498)
(11.636845273105207, 47.7153408676602)
(11.721170238852347, 48.09105005601798)
(11.805495204599485, 48.469627622481156)
(11.889820170346624, 48.84455525837762)
(11.974145136093764, 49.219192833566794)
(12.058470101840904, 49.595280712292414)
(12.142795067588041, 49.97404359531858)
(12.227120033335181, 50.349188776745514)
(12.31144499908232, 50.72770188527373)
(12.395769964829459, 51.10791507183635)
(12.480094930576598, 51.48923210053504)
(12.564419896323738, 51.872080005188856)
(12.648744862070878, 52.263073781372384)
(12.733069827818015, 52.658934131644855)
(12.817394793565155, 53.06269057894909)
(12.901719759312295, 53.46825990567387)
(12.986044725059434, 53.88038782728013)
(13.070369690806572, 54.30535899242579)
(13.154694656553712, 54.73681623727611)
(13.239019622300852, 55.181390671889375)
(13.323344588047991, 55.640298939787826)
(13.40766955379513, 56.11311400715241)
(13.491994519542269, 56.60810260414085)
(13.576319485289408, 57.121308624995415)
(13.660644451036546, 57.657155495502245)
(13.744969416783686, 58.210857213991076)
(13.829294382530826, 58.79000370230264)
(13.913619348277965, 59.402378256082514)
(13.997944314025103, 60.04254223706903)
(14.082269279772243, 60.721187605222546)
(14.166594245519383, 61.4566768147628)
(14.250919211266522, 62.256591730288655)
(14.33524417701366, 63.13888388668456)
(14.4195691427608, 64.13399354373209)
(14.50389410850794, 65.29695972063931)
(14.588219074255077, 66.79161031633134)
(14.672544040002217, 68.99190609768036)
(14.756869005749357, 73.11428109863715)
(14.841193971496496, 84.02926551391707)
(14.925518937243634, 94.56124087970578)
(15.009843902990774, 99.50485025817417)
(15.094168868737913, 99.86066611635704)
(15.178493834485053, 99.93106223856768)
(15.262818800232191, 99.9677307463141)
(15.34714376597933, 99.98436089353201)
(15.43146873172647, 99.99163658293983)
(15.51579369747361, 99.99462581967329)
(15.600118663220748, 99.99618086735403)
(15.684443628967887, 99.9973088812157)
(15.768768594715027, 99.99805820470954)
(15.853093560462165, 99.99860609715664)
(15.937418526209305, 99.99906535994319)
(16.021743491956443, 99.99933930616673)
(16.106068457703582, 99.99956490893906)
(16.190393423450722, 99.99972605377646)
(16.27471838919786, 99.99985496964635)
(16.359043354945, 99.99987914137196)
(16.44336832069214, 99.99991137033945)
(16.52769328643928, 99.99992748482317)
(16.61201825218642, 99.99996777103253)
(16.696343217933556, 99.99997582827439)
(16.780668183680696, 99.99999194275813)
};
\addplot[solid, blue, thick, mark = none] coordinates{
(0.0, 0.3601917781131121)
(0.075, 0.3601917781131121)
(0.15, 0.3601917781131121)
(0.225, 0.3601917781131121)
(0.3, 0.3601917781131121)
(0.375, 0.3601917781131121)
(0.45, 0.3601917781131121)
(0.525, 0.3601917781131121)
(0.6, 0.3601917781131121)
(0.675, 0.3601917781131121)
(0.75, 0.3601917781131121)
(0.8250000000000001, 0.3601917781131121)
(0.9, 0.3601917781131121)
(0.975, 0.3601917781131121)
(1.05, 0.3601917781131121)
(1.125, 0.3601917781131121)
(1.2, 0.3601917781131121)
(1.2750000000000001, 0.3601917781131121)
(1.35, 0.3601917781131121)
(1.425, 0.3601917781131121)
(1.5, 0.3601917781131121)
(1.575, 0.3601917781131121)
(1.6500000000000001, 0.3601917781131121)
(1.725, 0.3601917781131121)
(1.8, 0.3601917781131121)
(1.875, 0.3601917781131121)
(1.95, 0.3601917781131121)
(2.025, 2.1562070983187)
(2.1, 2.2409447568168597)
(2.1750000000000003, 2.3313472606947254)
(2.25, 2.4264664169488284)
(2.325, 2.5261806623735947)
(2.4, 2.6310978129968894)
(2.475, 2.7422714166003472)
(2.5500000000000003, 2.858680342257153)
(2.625, 2.9817428273656605)
(2.7, 3.111969437389276)
(2.775, 3.2499923009969804)
(2.85, 3.3965407974222117)
(2.9250000000000003, 3.5492728089042616)
(3.0, 3.712280963364092)
(3.075, 3.8835067905206633)
(3.15, 4.065251887066161)
(3.225, 4.259274867374542)
(3.3000000000000003, 4.463557782233294)
(3.375, 4.681390942406595)
(3.45, 4.912150323439169)
(3.525, 5.15941798778857)
(3.6, 5.421767593842743)
(3.6750000000000003, 5.701095527608625)
(3.75, 6.003277344022251)
(3.825, 6.335298875297222)
(3.9, 6.710013404369468)
(3.975, 7.102557203592435)
(4.05, 7.439676285287773)
(4.125, 7.787987286109539)
(4.2, 8.159379087562787)
(4.275, 8.543364837113408)
(4.3500000000000005, 8.948308083304832)
(4.425, 9.366550344185956)
(4.5, 9.800449945944894)
(4.575, 10.241813528526022)
(4.65, 10.693655859427551)
(4.7250000000000005, 11.144930895369738)
(4.8, 11.600079745462857)
(4.875, 12.049887918724462)
(4.95, 12.496883929830476)
(5.025, 12.93387123701097)
(5.1000000000000005, 13.362049263894269)
(5.175, 13.782901081588362)
(5.25, 14.198363597168711)
(5.325, 14.610487176702655)
(5.4, 15.019417696036877)
(5.4750000000000005, 15.431427816578951)
(5.55, 15.842303347202344)
(5.625, 16.253827214922126)
(5.7, 16.665270040504858)
(5.775, 17.07651026074497)
(5.8500000000000005, 17.478203717240742)
(5.925, 17.867019578159468)
(6.0, 18.23903540406799)
(6.075, 18.612299278887065)
(6.15, 18.98343984971546)
(6.2250000000000005, 19.354920797519462)
(6.3, 19.724270337119084)
(6.375, 20.092801351134508)
(6.45, 20.457871865897957)
(6.525, 20.8260949197926)
(6.6000000000000005, 21.190273971048505)
(6.675, 21.55373985149839)
(6.75, 21.91627374737221)
(6.825, 22.28116596943415)
(6.9, 22.649064854780594)
(6.9750000000000005, 23.016688196861075)
(7.05, 23.385559587852107)
(7.125, 23.753442264771145)
(7.2, 24.124753024087344)
(7.275, 24.497627896648584)
(7.3500000000000005, 24.871645463342208)
(7.425, 25.24512815193132)
(7.5, 25.61570142780037)
(7.575, 25.988738384635706)
(7.65, 26.361459277136557)
(7.7250000000000005, 26.72978768580936)
(7.8, 27.091397701320822)
(7.875, 27.450933038123843)
(7.95, 27.812437698857146)
(8.025, 28.17080602888666)
(8.1, 28.53098970278607)
(8.175, 28.89248625930566)
(8.25, 29.25318049866848)
(8.325, 29.614968806881446)
(8.4, 29.979147858137363)
(8.475, 30.3457014440088)
(8.55, 30.713827247338983)
(8.625, 31.086086199658652)
(8.700000000000001, 31.463223888628654)
(8.775, 31.838538129515058)
(8.85, 32.21299332374875)
(8.925, 32.59146010376635)
(9.0, 32.972050187774634)
(9.075000000000001, 33.35382348698383)
(9.15, 33.73588043367268)
(9.225, 34.123893977434626)
(9.3, 34.50933038123842)
(9.375, 34.893186463369766)
(9.450000000000001, 35.27675079380773)
(9.525, 35.65621439211103)
(9.6, 36.03559694827729)
(9.675, 36.413423495412204)
(9.75, 36.790237015834016)
(9.825000000000001, 37.163233451600824)
(9.9, 37.53701599609701)
(9.975, 37.9089750925096)
(10.05, 38.281866173498244)
(10.125, 38.64803886132556)
(10.200000000000001, 39.01483557360814)
(10.275, 39.379881775730475)
(10.35, 39.73883360914674)
(10.425, 40.098166340607136)
(10.5, 40.45358473684807)
(10.575000000000001, 40.80975682496357)
(10.65, 41.15898360193399)
(10.725, 41.507675500799884)
(10.8, 41.847396035094484)
(10.875, 42.188794141626)
(10.950000000000001, 42.5240330457418)
(11.025, 42.85199436595063)
(11.1, 43.17827000970885)
(11.175, 43.496627836677405)
(11.25, 43.81460476560183)
(11.325000000000001, 44.12538515275632)
(11.4, 44.434325883399815)
(11.475, 44.74290192442659)
(11.55, 45.046907188923804)
(11.625, 45.34854602301921)
(11.700000000000001, 45.64753477923311)
(11.775, 45.951102416190274)
(11.85, 46.25462953207891)
(11.925, 46.558116126899016)
(12.0, 46.861481158513556)
(12.075000000000001, 47.173679783066405)
(12.15, 47.488747299270784)
(12.225, 47.80577603519174)
(12.3, 48.13061723312419)
(12.375, 48.46226597056874)
(12.450000000000001, 48.798550318252474)
(12.525, 49.141520642242725)
(12.6, 49.49238447038153)
(12.675, 49.851465971217074)
(12.75, 50.21827078771336)
(12.825000000000001, 50.59475203537327)
(12.9, 50.983640834215336)
(12.975, 51.38607177415826)
(13.05, 51.80308219455624)
(13.125, 52.230903636036516)
(13.200000000000001, 52.676821786719785)
(13.275, 53.1397749946107)
(13.35, 53.609592471509636)
(13.425, 54.093746302452494)
(13.5, 54.59454618834517)
(13.575000000000001, 55.105541175078564)
(13.65, 55.63055645152141)
(13.725, 56.15865943338579)
(13.8, 56.69415345814903)
(13.875, 57.2298581924686)
(13.950000000000001, 57.76870736170564)
(14.025, 58.306770422213326)
(14.1, 58.84886938114603)
(14.175, 59.387062109073)
(14.25, 59.92156741976423)
(14.325000000000001, 60.45912801902221)
(14.4, 61.00050570293518)
(14.475, 61.54230480596081)
(14.55, 62.09709496355536)
(14.625, 62.65845763846455)
(14.700000000000001, 63.23785218886708)
(14.775, 63.83903086570831)
(14.85, 64.46701828148528)
(14.925, 65.1192372962398)
};
\addplot[solid, red, thick, mark = none] coordinates{
(0.0007848920106977707,0.374403915174969)
(0.07927409308047484,0.38011649966018585)
(0.15776329415025192,0.3877305932265185)
(0.236252495220029,0.39696419240854725)
(0.3147416962898061,0.4085666207001018)
(0.39323089735958316,0.42345640367426346)
(0.4717200984293602,0.44956992457213024)
(0.5502092994991372,0.49659198812040256)
(0.6286985005689143,0.5609774078966611)
(0.7071877016386914,0.618473885874809)
(0.7856769027084685,0.6738915954507201)
(0.8641661037782455,0.7284794091141104)
(0.9426553048480226,0.7838407179969374)
(1.0211445059177997,0.8430614457350802)
(1.0996337069875768,0.9057226157513438)
(1.1781229080573539,0.9737337943687131)
(1.256612109127131,1.0469418939916744)
(1.335101310196908,1.125290513927144)
(1.4135905112666851,1.211486887443151)
(1.4920797123364622,1.30549072833035)
(1.5705689134062393,1.4096789229401359)
(1.6490581144760164,1.5170174991207535)
(1.7275473155457934,1.6357812442718045)
(1.8060365166155705,1.7664133066960919)
(1.8845257176853476,1.9114517175823922)
(1.9630149187551247,2.066440822177075)
(2.0415041198249018,2.2395023202842275)
(2.119993320894679,2.4224017107135936)
(2.198482521964456,2.585254683372552)
(2.276971723034233,2.717192018979639)
(2.35546092410401,2.847163387570657)
(2.433950125173787,2.981139205370635)
(2.5124393262435643,3.1183620916438746)
(2.5909285273133413,3.261644023802704)
(2.6694177283831184,3.4080441085648885)
(2.7479069294528955,3.561308963399576)
(2.8263961305226726,3.720761779989759)
(2.9048853315924497,3.8873774846016036)
(2.9833745326622267,4.061784542100902)
(3.061863733732004,4.245948919503722)
(3.140352934801781,4.438863461576424)
(3.218842135871558,4.639214837894336)
(3.297331336941335,4.850886639038384)
(3.375820538011112,5.075611172010431)
(3.4543097390808892,5.313670440275896)
(3.5327989401506663,5.56367054099142)
(3.6112881412204434,5.832742133211186)
(3.6897773422902205,6.120079492748281)
(3.7682665433599976,6.429340607411292)
(3.8467557444297746,6.757222008033875)
(3.9252449454995513,7.107284995522188)
(4.003734146569329,7.478377384288942)
(4.082223347639106,7.8697981942915245)
(4.160712548708883,8.282723782842828)
(4.23920174977866,8.70964480052082)
(4.317690950848437,9.145082322854488)
(4.396180151918214,9.578424962302181)
(4.474669352987991,10.0275275668459)
(4.553158554057768,10.48372054423446)
(4.6316477551275455,10.951846296831208)
(4.7101369561973225,11.428287123036904)
(4.7886261572671,11.903607992622788)
(4.867115358336877,12.387058619254633)
(4.945604559406654,12.86299989646444)
(5.024093760476431,13.333381676784548)
(5.102582961546208,13.798598765066538)
(5.181072162615985,14.254566139682762)
(5.259561363685762,14.701340201326301)
(5.338050564755539,15.13967027349099)
(5.416539765825316,15.570168706558876)
(5.495028966895093,15.997798761521354)
(5.57351816796487,16.42524349992084)
(5.6520073690346475,16.84878853325566)
(5.730496570104424,17.26883672361928)
(5.808985771174201,17.68980343955598)
(5.887474972243978,18.112816694927442)
(5.965964173313755,18.52522661999912)
(6.044453374383532,18.93391409932726)
(6.122942575453309,19.34214231586886)
(6.201431776523086,19.74578596178692)
(6.279920977592863,20.142419807278834)
(6.35841017866264,20.530964181934134)
(6.436899379732417,20.916051999827577)
(6.5153885808021945,21.298513156871678)
(6.593877781871972,21.67766278750757)
(6.672366982941749,22.058730041708312)
(6.750856184011526,22.435373870122902)
(6.829345385081303,22.810792997773383)
(6.90783458615108,23.1850277108691)
(6.986323787220857,23.563186300755085)
(7.064812988290634,23.938718229791732)
(7.143302189360411,24.319165076368556)
(7.221791390430188,24.698290535278836)
(7.300280591499965,25.07700507485379)
(7.378769792569742,25.457790325589112)
(7.4572589936395195,25.84031594056817)
(7.535748194709297,26.22442883219545)
(7.614237395779074,26.605512200879932)
(7.692726596848851,26.98733683581637)
(7.771215797918628,27.37100657914085)
(7.849704998988405,27.751703200215612)
(7.928194200058182,28.131827757117666)
(8.006683401127958,28.51059869738571)
(8.085172602197737,28.886324000227216)
(8.163661803267512,29.258745833902378)
(8.242151004337291,29.627622481155118)
(8.320640205407067,30.00172827838093)
(8.399129406476845,30.370169834572742)
(8.47761860754662,30.73981191980305)
(8.5561078086164,31.109663493321953)
(8.634597009686175,31.484768388539543)
(8.713086210755954,31.861017412102544)
(8.791575411825729,32.23955469235638)
(8.870064612895508,32.621218182455436)
(8.948553813965283,33.00757098732233)
(9.027043015035062,33.39422191013839)
(9.105532216104837,33.780469970860985)
(9.184021417174616,34.16803941925012)
(9.262510618244391,34.5549965172572)
(9.34099981931417,34.94538600030054)
(9.419489020383946,35.334341294291164)
(9.497978221453723,35.72427957178982)
(9.5764674225235,36.108835611719904)
(9.654956623593277,36.49465663862343)
(9.733445824663054,36.87889038887875)
(9.811935025732831,37.26476781647537)
(9.890424226802608,37.64314395189182)
(9.968913427872385,38.01849056436548)
(10.047402628942162,38.39490073276586)
(10.12589183001194,38.767362852650365)
(10.204381031081716,39.138584157287035)
(10.282870232151494,39.505672096844826)
(10.36135943322127,39.87154339288038)
(10.439848634291048,40.23642364816603)
(10.518337835360825,40.60001474475262)
(10.596827036430602,40.95882789691082)
(10.675316237500379,41.315513937215556)
(10.753805438570156,41.66660019442124)
(10.832294639639933,42.014729443860965)
(10.91078384070971,42.35928933515266)
(10.989273041779487,42.697137543967365)
(11.067762242849264,43.02885419171965)
(11.146251443919041,43.356743649584104)
(11.224740644988819,43.67993573543885)
(11.303229846058596,43.999453719001274)
(11.381719047128373,44.31532177199698)
(11.46020824819815,44.62791858479381)
(11.538697449267927,44.93746976016411)
(11.617186650337704,45.24691619139011)
(11.695675851407481,45.5508836981451)
(11.774165052477258,45.8562853939528)
(11.852654253547035,46.16298430570143)
(11.931143454616812,46.467620563531554)
(12.00963265568659,46.7760114960727)
(12.088121856756366,47.08811681711552)
(12.166611057826143,47.40723999582635)
(12.24510025889592,47.72974721612222)
(12.323589459965698,48.057290212586295)
(12.402078661035475,48.38955475278569)
(12.480567862105252,48.72840205959217)
(12.559057063175029,49.07941580162103)
(12.637546264244806,49.43872044553325)
(12.716035465314583,49.809450258415886)
(12.79452466638436,50.19254793756765)
(12.873013867454137,50.58856943267751)
(12.951503068523914,50.994009843532396)
(13.029992269593691,51.413937175267975)
(13.108481470663468,51.84976950245323)
(13.186970671733246,52.30167602716741)
(13.265459872803023,52.768270903809025)
(13.3439490738728,53.249360758573204)
(13.422438274942577,53.73977284217998)
(13.500927476012354,54.24911138693736)
(13.579416677082131,54.770664710368344)
(13.657905878151908,55.30091179777612)
(13.736395079221685,55.84467893704031)
(13.814884280291462,56.400427194963896)
(13.89337348136124,56.957714386084504)
(13.971862682431016,57.518933511237236)
(14.050351883500793,58.08157876820081)
(14.12884108457057,58.64322492717261)
(14.207330285640348,59.21529715712307)
(14.285819486710125,59.79629681106453)
(14.364308687779902,60.38252561497905)
(14.442797888849679,60.98625474823335)
(14.521287089919456,61.63107581502023)
(14.599776290989233,62.417849369057535)
(14.67826549205901,63.41442544412524)
(14.756754693128787,64.91140458271745)
(14.835243894198564,67.59990476340111)
(14.913733095268341,80.97803636152683)
(14.992222296338118,97.19270384519783)
(15.070711497407896,99.34144133582625)
(15.149200698477673,99.81719729647305)
(15.22768989954745,99.95003704316949)
(15.306179100617227,99.98542444945873)
(15.384668301687004,99.99494005210619)
(15.463157502756781,99.99800180401645)
(15.541646703826558,99.99931513444112)
(15.620135904896335,99.99983079792075)
};
\addplot[dashed, magenta, thick, mark = none] coordinates{
(0.0, 0.5978301732190421)
(0.075, 0.6133760916944118)
(0.15, 0.6302307014301745)
(0.225, 0.6474937562089899)
(0.3, 0.6658404406938631)
(0.375, 0.6855625013441176)
(0.45, 0.7072100886259058)
(0.525, 0.729924634387505)
(0.6, 0.7542562890950675)
(0.675, 0.7787713272913476)
(0.75, 0.8055703234834727)
(0.8250000000000001, 0.8346949557370608)
(0.9, 0.8651199436379183)
(0.975, 0.8980706223152032)
(1.05, 0.9571367769084845)
(1.125, 1.0989005493002337)
(1.2, 1.1451548665226605)
(1.2750000000000001, 1.1934430733472272)
(1.35, 1.2504586671121218)
(1.425, 1.3082328016712572)
(1.5, 1.3678491067306908)
(1.575, 1.431733245709368)
(1.6500000000000001, 1.5001519582272418)
(1.725, 1.5731302511236822)
(1.8, 1.6536022602181697)
(1.875, 1.7413345883432452)
(1.95, 1.8342933458967696)
(2.025, 2.4780944254920385)
(2.1, 2.60748814800848)
(2.1750000000000003, 2.7090742651448503)
(2.25, 2.8046754120585313)
(2.325, 2.9040109136515504)
(2.4, 3.005847099181626)
(2.475, 3.113043083950127)
(2.5500000000000003, 3.2260573266788466)
(2.625, 3.3446564302003265)
(2.7, 3.4692071614920015)
(2.775, 3.6020601634547047)
(2.85, 3.7420984639298847)
(2.9250000000000003, 3.8896138093768644)
(3.0, 4.044789583284362)
(3.075, 4.211743578535397)
(3.15, 4.3851493383440365)
(3.225, 4.567940998529765)
(3.3000000000000003, 4.762994345620194)
(3.375, 4.968975681515561)
(3.45, 5.1898861005151575)
(3.525, 5.4273593827911935)
(3.6, 5.676210776980837)
(3.6750000000000003, 5.947368271889028)
(3.75, 6.237430937361369)
(3.825, 6.549357916056708)
(3.9, 6.891509827937941)
(3.975, 7.275306462984293)
(4.05, 7.7634899811765194)
(4.125, 8.116119758754019)
(4.2, 8.48711289204264)
(4.275, 8.87052608888531)
(4.3500000000000005, 9.27121067611992)
(4.425, 9.682389800277043)
(4.5, 10.10815624740033)
(4.575, 10.5434836427763)
(4.65, 10.981970235526083)
(4.7250000000000005, 11.424399573283294)
(4.8, 11.862452714150654)
(4.875, 12.295629521340754)
(4.95, 12.727806054956032)
(5.025, 13.160140965220654)
(5.1000000000000005, 13.587757918457367)
(5.175, 14.010456859951196)
(5.25, 14.423828250359808)
(5.325, 14.839166845465568)
(5.4, 15.251346243197514)
(5.4750000000000005, 15.66676819443451)
(5.55, 16.075063196450895)
(5.625, 16.484250109071496)
(5.7, 16.894520651398157)
(5.775, 17.309109041322802)
(5.8500000000000005, 17.720679939296733)
(5.925, 18.130767098134672)
(6.0, 18.538695333173624)
(6.075, 18.95191668254601)
(6.15, 19.333304325399663)
(6.2250000000000005, 19.705797869050517)
(6.3, 20.07650759149294)
(6.375, 20.44800086156897)
(6.45, 20.81621823568746)
(6.525, 21.186994643034872)
(6.6000000000000005, 21.553469874010542)
(6.675, 21.92303761745504)
(6.75, 22.287362260244844)
(6.825, 22.653379032498723)
(6.9, 23.022079872178374)
(6.9750000000000005, 23.391764314206604)
(7.05, 23.76241568735716)
(7.125, 24.13397564233818)
(7.2, 24.505969049201624)
(7.275, 24.879329496617324)
(7.3500000000000005, 25.253565183411)
(7.425, 25.62804260298525)
(7.5, 26.006062658137)
(7.575, 26.38009829021571)
(7.65, 26.755175873934856)
(7.7250000000000005, 27.127711095651325)
(7.8, 27.496295236747248)
(7.875, 27.869213896667404)
(7.95, 28.23931511935181)
(8.025, 28.617751955159736)
(8.1, 28.98364369321676)
(8.175, 29.34897694519451)
(8.25, 29.720561907014904)
(8.325, 30.09275536859331)
(8.4, 30.46615749407463)
(8.475, 30.84332731668778)
(8.55, 31.21890503719434)
(8.625, 31.598592214970793)
(8.700000000000001, 31.97865449533781)
(8.775, 32.36687734095275)
(8.85, 32.75448335119655)
(8.925, 33.146215489936495)
(9.0, 33.53790595061083)
(9.075000000000001, 33.9300381987807)
(9.15, 34.32471280895325)
(9.225, 34.71945410403078)
(9.3, 35.11671275427163)
(9.375, 35.51023704983313)
(9.450000000000001, 35.905778563770525)
(9.525, 36.295701874462665)
(9.6, 36.69002638888403)
(9.675, 37.08318391746809)
(9.75, 37.47364070740014)
(9.825000000000001, 37.86537284614009)
(9.9, 38.250669891548675)
(9.975, 38.637117251568306)
(10.05, 39.027840781120304)
(10.125, 39.411112272539874)
(10.200000000000001, 39.790757772250714)
(10.275, 40.16463502768007)
(10.35, 40.53541143502748)
(10.425, 40.90880522489568)
(10.5, 41.273504970276036)
(10.575000000000001, 41.638121359525165)
(10.65, 41.998494921694416)
(10.725, 42.358118278682554)
(10.8, 42.71624122530845)
(10.875, 43.066195271073305)
(10.950000000000001, 43.41125631193465)
(11.025, 43.754591880879424)
(11.1, 44.08891665203766)
(11.175, 44.42049900647827)
(11.25, 44.75122279276715)
(11.325000000000001, 45.072352288350864)
(11.4, 45.39109779858125)
(11.475, 45.70932650079797)
(11.55, 46.02420428653903)
(11.625, 46.337431620881645)
(11.700000000000001, 46.65159254389409)
(11.775, 46.966295281759564)
(11.85, 47.28467402501251)
(11.925, 47.59957681759294)
(12.0, 47.9187391084795)
(12.075000000000001, 48.24137735003857)
(12.15, 48.56677467954152)
(12.225, 48.8958313432057)
(12.3, 49.22941424479595)
(12.375, 49.56739835011542)
(12.450000000000001, 49.914426595673916)
(12.525, 50.266964681507055)
(12.6, 50.62702149037762)
(12.675, 50.99723941164576)
(12.75, 51.37682656206473)
(12.825000000000001, 51.76616637983822)
(12.9, 52.16448365294575)
(12.975, 52.573937305186305)
(13.05, 52.996636246680126)
(13.125, 53.435272880466144)
(13.200000000000001, 53.89191443859895)
(13.275, 54.3584170270569)
(13.35, 54.83736468590826)
(13.425, 55.33235006440928)
(13.5, 55.835370973961375)
(13.575000000000001, 56.34455190161176)
(13.65, 56.86528598905134)
(13.725, 57.39508088795618)
(13.8, 57.92813501159234)
(13.875, 58.46749085874987)
(13.950000000000001, 59.008280431364646)
(14.025, 59.609169774600026)
(14.1, 60.313295686370225)
(14.175, 61.02494865679097)
(14.25, 61.75203918271648)
(14.325000000000001, 62.49846833108855)
(14.4, 63.252357853206185)
(14.475, 64.02990384536838)
(14.55, 64.82927247268795)
(14.625, 65.65083883775546)
(14.700000000000001, 66.52143527921554)
(14.775, 70.33132728467902)
(14.85, 79.65141799615529)
(14.925, 89.58084202696104)
};
\addplot[dashed, black, thick, mark = none] coordinates{
(0.0, 0.49103249123069936)
(0.075, 0.5009267842459972)
(0.15, 0.5112481110803593)
(0.225, 0.5222301317479904)
(0.3, 0.5338245027976758)
(0.375, 0.545821735940818)
(0.45, 0.5576981104559231)
(0.525, 0.571830512694386)
(0.6, 0.5865510935892958)
(0.675, 0.6014892200146722)
(0.75, 0.6173942154643449)
(0.8250000000000001, 0.6347253427248545)
(0.9, 0.6530394534933985)
(0.975, 0.6725863222679201)
(1.05, 0.7051698083867025)
(1.125, 0.7932193475326107)
(1.2, 0.8201385926173911)
(1.2750000000000001, 0.8478474474053465)
(1.35, 0.8786099968617043)
(1.425, 0.9099446104907707)
(1.5, 0.9433418780383356)
(1.575, 0.979156318146641)
(1.6500000000000001, 1.0165741493869043)
(1.725, 1.0563849814623008)
(1.8, 1.0989352757732032)
(1.875, 1.1427586142994288)
(1.95, 1.1884431756974247)
(2.025, 1.6587524408407088)
(2.1, 1.7172480168106292)
(2.1750000000000003, 1.7643345382938551)
(2.25, 1.8085929678810138)
(2.325, 1.8531495154173308)
(2.4, 1.89926916787626)
(2.475, 1.9470647266439693)
(2.5500000000000003, 1.9962461310131698)
(2.625, 2.0469986975468517)
(2.7, 2.0998461469665086)
(2.775, 2.1557634055383064)
(2.85, 2.2138641766566396)
(2.9250000000000003, 2.2761305418213156)
(3.0, 2.3401856146809394)
(3.075, 2.4116372355764293)
(3.15, 2.484410244138457)
(3.225, 2.5608251260253345)
(3.3000000000000003, 2.641671490940236)
(3.375, 2.726602877482789)
(3.45, 2.820268314211484)
(3.525, 2.921902363148754)
(3.6, 3.0298532897114256)
(3.6750000000000003, 3.1456600270965045)
(3.75, 3.268130103507358)
(3.825, 3.3921874565664303)
(3.9, 3.5224408286228686)
(3.975, 3.6661981380519766)
(4.05, 3.832507667472794)
(4.125, 3.9506510049999215)
(4.2, 4.079260699715056)
(4.275, 4.216604444616332)
(4.3500000000000005, 4.360917703734411)
(4.425, 4.51640635732498)
(4.5, 4.682490283973461)
(4.575, 4.859338685759107)
(4.65, 5.047459168919673)
(4.7250000000000005, 5.250090744686551)
(4.8, 5.464493950824235)
(4.875, 5.69445569101122)
(4.95, 5.93638243537387)
(5.025, 6.193875771027689)
(5.1000000000000005, 6.467016270391368)
(5.175, 6.7540313402536984)
(5.25, 7.058466167037099)
(5.325, 7.379418339652226)
(5.4, 7.715993504251604)
(5.4750000000000005, 8.070705520298407)
(5.55, 8.439985029644607)
(5.625, 8.828690549137292)
(5.7, 9.23634670150618)
(5.775, 9.660939176283993)
(5.8500000000000005, 10.104836802580252)
(5.925, 10.566420074779263)
(6.0, 11.049089148949799)
(6.075, 11.557493053650354)
(6.15, 12.077733046656668)
(6.2250000000000005, 12.618591521606099)
(6.3, 13.183444462841814)
(6.375, 13.768811141876347)
(6.45, 14.378768523095479)
(6.525, 15.00866757794072)
(6.6000000000000005, 15.65759783808086)
(6.675, 16.331368574903546)
(6.75, 17.02990727323195)
(6.825, 17.744753829103484)
(6.9, 18.485568875519238)
(6.9750000000000005, 19.239162707539442)
(7.05, 20.0213275192276)
(7.125, 20.816778722757963)
(7.2, 21.626160897480055)
(7.275, 22.45660470244807)
(7.3500000000000005, 23.298900710205583)
(7.425, 24.157778521729778)
(7.5, 25.024012595080492)
(7.575, 25.902856251956397)
(7.65, 26.798966578157863)
(7.7250000000000005, 27.7032550048565)
(7.8, 28.61444848783699)
(7.875, 29.528792352388304)
(7.95, 30.443385991437573)
(8.025, 31.363756672907)
(8.1, 32.27968781410654)
(8.175, 33.192597489605156)
(8.25, 34.09665225628958)
(8.325, 34.99908751735832)
(8.4, 35.895777964974364)
(8.475, 36.78031003460988)
(8.55, 37.652466180734415)
(8.625, 38.506751364393196)
(8.700000000000001, 39.35401869038396)
(8.775, 40.18371317185815)
(8.85, 40.98835768836119)
(8.925, 41.77932100817044)
(9.0, 42.55234085033713)
(9.075000000000001, 43.30823905353191)
(9.15, 44.037628930977235)
(9.225, 44.74938150597102)
(9.3, 45.43680926776189)
(9.375, 46.10350574622347)
(9.450000000000001, 46.74880219028063)
(9.525, 47.37265831372402)
(9.6, 47.97608127178729)
(9.675, 48.557282356775474)
(9.75, 49.120427162734934)
(9.825000000000001, 49.661019748702685)
(9.9, 50.17802878771948)
(9.975, 50.67495917999838)
(10.05, 51.15388163669977)
(10.125, 51.61213726800683)
(10.200000000000001, 52.053061772053375)
(10.275, 52.474568323195314)
(10.35, 52.87789773668047)
(10.425, 53.2631708711369)
(10.5, 53.63648705865954)
(10.575000000000001, 53.992955553433816)
(10.65, 54.33583148117486)
(10.725, 54.66373705352305)
(10.8, 54.98632484623761)
(10.875, 55.29557790365875)
(10.950000000000001, 55.593711967300486)
(11.025, 55.88108155580505)
(11.1, 56.16324616606217)
(11.175, 56.43509750672679)
(11.25, 56.69876268965237)
(11.325000000000001, 56.9555469880217)
(11.4, 57.2033877479163)
(11.475, 57.44773972208156)
(11.55, 57.68600042139374)
(11.625, 57.921610288131)
(11.700000000000001, 58.15054875860061)
(11.775, 58.37749709032853)
(11.85, 58.598563635491985)
(11.925, 58.81899365854779)
(12.0, 59.03321960536435)
(12.075000000000001, 59.24915368745717)
(12.15, 59.45943158575786)
(12.225, 59.669685312332945)
(12.3, 59.87925417334914)
(12.375, 60.08813816880647)
(12.450000000000001, 60.29920567681033)
(12.525, 60.50694554392224)
(12.6, 60.71619211526368)
(12.675, 60.92540645763764)
(12.75, 61.135329837296084)
(12.825000000000001, 61.3439560010136)
(12.9, 61.55129300603206)
(12.975, 61.76481797280601)
(13.05, 61.982822766059186)
(13.125, 62.197669120499675)
(13.200000000000001, 62.41487624680783)
(13.275, 62.63417825600194)
(13.35, 62.85669510470184)
(13.425, 63.080960374887354)
(13.5, 63.30817459559695)
(13.575000000000001, 63.53980418485086)
(13.65, 63.77652595096605)
(13.725, 64.02043477682851)
(13.8, 64.26715558010329)
(13.875, 64.52191751076347)
(13.950000000000001, 64.78333472320756)
(14.025, 65.10578554281035)
(14.1, 65.52153116601585)
(14.175, 65.95923277331474)
(14.25, 66.41214645326255)
(14.325000000000001, 66.89187463415087)
(14.4, 67.39989984848357)
(14.475, 67.93586757761844)
(14.55, 68.49694167241752)
(14.625, 69.08293681631785)
(14.700000000000001, 69.70173299186743)
(14.775, 73.03841410919738)
(14.85, 81.51443918172264)
(14.925, 90.53297446378048)
};
