# Supplementary material for: CausalSim: A Causal Framework for Unbiased Trace-Driven Simulation
Source: arXiv:2201.01811 source file (2023-05-05)
Supplement: Supplementary file 11 [file new_linear_bba_puffer_ttp_cl.tex]

\addplot[solid, green!70!black, thick, mark = none] coordinates{
(0.0, 0.37866458166706085)
(0.0851435971603314, 0.3848342186167259)
(0.1702871943206628, 0.39439175849433616)
(0.2554307914809942, 0.4070714834231903)
(0.3405743886413256, 0.4241853754195021)
(0.425717985801657, 0.4459576339417387)
(0.5108615829619884, 0.47497070460409363)
(0.5960051801223197, 0.5102032343179952)
(0.6811487772826512, 0.5531249750889491)
(0.7662923744429826, 0.601992153351101)
(0.851435971603314, 0.6602092793996902)
(0.9365795687636453, 0.7250195302639375)
(1.0217231659239767, 0.7961654917507885)
(1.106866763084308, 0.8707076598492317)
(1.1920103602446395, 0.9499829276264219)
(1.2771539574049708, 1.0318489447014527)
(1.3622975545653024, 1.1165465179000849)
(1.4474411517256338, 1.207953467485432)
(1.5325847488859652, 1.2999914970279456)
(1.6177283460462966, 1.3935075822596117)
(1.702871943206628, 1.4904115704192231)
(1.7880155403669593, 1.5884199485038755)
(1.8731591375272907, 1.691908757795498)
(1.958302734687622, 1.8077202336191571)
(2.0434463318479534, 1.920675242268274)
(2.128589929008285, 2.025368085688701)
(2.213733526168616, 2.128566266052681)
(2.2988771233289476, 2.237867653897151)
(2.384020720489279, 2.3554312069703114)
(2.4691643176496103, 2.4856495739213846)
(2.5543079148099417, 2.62182998573095)
(2.6394515119702735, 2.7696023399116223)
(2.724595109130605, 2.929489768533158)
(2.8097387062909362, 3.101650041584848)
(2.8948823034512676, 3.2866395058710363)
(2.980025900611599, 3.4825400104692843)
(3.0651694977719304, 3.6982448005654476)
(3.1503130949322617, 3.9331975293551826)
(3.235456692092593, 4.1859699632512175)
(3.3206002892529245, 4.460165900956318)
(3.405743886413256, 4.753443703682052)
(3.4908874835735872, 5.0631794073959915)
(3.5760310807339186, 5.391581791948217)
(3.66117467789425, 5.731650852024372)
(3.7463182750545814, 6.089489795104945)
(3.8314618722149127, 6.462997789227266)
(3.916605469375244, 6.849384796685968)
(4.0017490665355755, 7.249663866885972)
(4.086892663695907, 7.663378297226703)
(4.172036260856238, 8.08844386311278)
(4.25717985801657, 8.5259400434183)
(4.342323455176901, 8.973392340416487)
(4.427467052337232, 9.429214750530772)
(4.512610649497564, 9.89277619380399)
(4.597754246657895, 10.361012610970429)
(4.6828978438182265, 10.840276320019981)
(4.768041440978558, 11.32382472983135)
(4.853185038138889, 11.814414663375308)
(4.938328635299221, 12.313889538421478)
(5.023472232459552, 12.816503205886182)
(5.108615829619883, 13.327619845405339)
(5.193759426780216, 13.843751909847239)
(5.278903023940547, 14.363653846664842)
(5.364046621100878, 14.88715958218521)
(5.44919021826121, 15.405799359088482)
(5.534333815421541, 15.921300343573213)
(5.6194774125818725, 16.431835725237086)
(5.704621009742204, 16.938759004514548)
(5.789764606902535, 17.434015608268076)
(5.874908204062867, 17.921201031516798)
(5.960051801223198, 18.3953413677562)
(6.045195398383529, 18.86348644440252)
(6.130338995543861, 19.326707436646213)
(6.215482592704192, 19.785386313935042)
(6.3006261898645235, 20.243309556011997)
(6.385769787024855, 20.694199578040013)
(6.470913384185186, 21.143976906459336)
(6.556056981345518, 21.593438694900076)
(6.641200578505849, 22.037021475318795)
(6.72634417566618, 22.48102774360351)
(6.811487772826512, 22.925573751325267)
(6.896631369986843, 23.37049342481114)
(6.9817749671471745, 23.815031128849256)
(7.066918564307506, 24.256687454661886)
(7.152062161467837, 24.699464777766853)
(7.237205758628169, 25.143221935542158)
(7.3223493557885, 25.58622345810559)
(7.407492952948831, 26.02981454220796)
(7.492636550109163, 26.470407996513785)
(7.577780147269494, 26.910362067178795)
(7.6629237444298255, 27.350532033618624)
(7.748067341590157, 27.787895354985796)
(7.833210938750488, 28.226030918932132)
(7.91835453591082, 28.66575248645503)
(8.003498133071151, 29.104427789838418)
(8.088641730231483, 29.542015310664056)
(8.173785327391814, 29.9759409070014)
(8.258928924552146, 30.41136116639519)
(8.344072521712476, 30.844489609102432)
(8.429216118872809, 31.27805814704296)
(8.51435971603314, 31.715595845766714)
(8.599503313193471, 32.14885714741231)
(8.684646910353802, 32.58504964938526)
(8.769790507514134, 33.02128366977645)
(8.854934104674465, 33.45805742960469)
(8.940077701834797, 33.89415028737388)
(9.025221298995127, 34.32979474622614)
(9.11036489615546, 34.76906791483211)
(9.19550849331579, 35.206730168810566)
(9.280652090476122, 35.64359526915892)
(9.365795687636453, 36.080767605802215)
(9.450939284796785, 36.521178379067806)
(9.536082881957116, 36.95935546143238)
(9.621226479117448, 37.3980556758667)
(9.706370076277778, 37.83925529907876)
(9.79151367343811, 38.28019750809775)
(9.876657270598441, 38.722227499674496)
(9.961800867758773, 39.163676233395954)
(10.046944464919104, 39.60388771825402)
(10.132088062079436, 40.038560646119585)
(10.217231659239767, 40.47785872577649)
(10.302375256400099, 40.91323746675205)
(10.387518853560431, 41.34745369201704)
(10.472662450720762, 41.7825501077486)
(10.557806047881094, 42.21599409043442)
(10.642949645041424, 42.646764286985935)
(10.728093242201757, 43.07437078006797)
(10.813236839362087, 43.498257222876184)
(10.89838043652242, 43.91869763697092)
(10.98352403368275, 44.33547612657737)
(11.068667630843082, 44.748360188553406)
(11.153811228003413, 45.15861198281337)
(11.238954825163745, 45.56912949495003)
(11.324098422324075, 45.97072054716625)
(11.409242019484408, 46.3707422031732)
(11.494385616644738, 46.77262388431706)
(11.57952921380507, 47.16709867964787)
(11.664672810965401, 47.56183088917173)
(11.749816408125733, 47.95055123173522)
(11.834960005286064, 48.33828343594472)
(11.920103602446396, 48.72429677763931)
(12.005247199606726, 49.11169683450293)
(12.090390796767059, 49.49893912137727)
(12.17553439392739, 49.88755151605335)
(12.260677991087721, 50.27705240487964)
(12.345821588248052, 50.66016776098146)
(12.430965185408384, 51.052716101706174)
(12.516108782568715, 51.44366183148704)
(12.601252379729047, 51.83633472746646)
(12.686395976889377, 52.23695424869599)
(12.77153957404971, 52.64595218672527)
(12.85668317121004, 53.05578049311923)
(12.941826768370372, 53.472866219020624)
(13.026970365530703, 53.89520817667051)
(13.112113962691035, 54.32900091406949)
(13.197257559851366, 54.774634704349)
(13.282401157011698, 55.23339661847431)
(13.367544754172028, 55.703484757094)
(13.45268835133236, 56.19313637438586)
(13.537831948492691, 56.70205253773858)
(13.622975545653023, 57.23467571790327)
(13.708119142813356, 57.78257767597831)
(13.793262739973686, 58.35878689160571)
(13.878406337134019, 58.96124405124104)
(13.963549934294349, 59.58829672183855)
(14.048693531454681, 60.260828667770284)
(14.133837128615012, 60.97835827538469)
(14.218980725775344, 61.752693382827715)
(14.304124322935674, 62.59927884168264)
(14.389267920096007, 63.54679557526591)
(14.474411517256337, 64.63686164601596)
(14.55955511441667, 65.99609162218107)
(14.644698711577, 67.90240149174016)
(14.729842308737332, 71.19859023380516)
(14.814985905897663, 79.14542307600328)
(14.900129503057995, 92.20966668349546)
(14.985273100218325, 98.79774285949637)
(15.070416697378658, 99.80456450168597)
(15.155560294538988, 99.9010616093469)
(15.24070389169932, 99.95728585132022)
(15.325847488859651, 99.98284458958545)
(15.410991086019983, 99.99237721841212)
(15.496134683180314, 99.99550770714701)
(15.581278280340646, 99.99690272599969)
(15.666421877500976, 99.99764175384426)
(15.751565474661309, 99.99830604853602)
(15.83670907182164, 99.99875444745297)
(15.921852668981971, 99.99911980953343)
(16.006996266142302, 99.99937722372648)
(16.092139863302634, 99.99955160108307)
(16.177283460462967, 99.99967615633777)
(16.262427057623295, 99.99975088949058)
(16.347570654783627, 99.99982562264341)
(16.43271425194396, 99.999858837378)
(16.517857849104292, 99.99992526684719)
(16.60300144626462, 99.99995017789813)
(16.688145043424953, 99.99997508894906)
(16.773288640585285, 99.99997508894906)
(16.858432237745617, 99.99998339263271)
(16.943575834905946, 99.99998339263271)
};
\addplot[solid, blue, thick, mark = none] coordinates{
(0.0, 0.3720592570533261)
(0.075, 0.3720592570533261)
(0.15, 0.3720592570533261)
(0.225, 0.3720592570533261)
(0.3, 0.3720592570533261)
(0.375, 0.3720592570533261)
(0.45, 0.3720592570533261)
(0.525, 0.3720592570533261)
(0.6, 0.3720592570533261)
(0.675, 0.3720592570533261)
(0.75, 0.3720592570533261)
(0.8250000000000001, 0.3720592570533261)
(0.9, 0.3720592570533261)
(0.975, 0.3720592570533261)
(1.05, 0.3720592570533261)
(1.125, 0.3720592570533261)
(1.2, 0.3720592570533261)
(1.2750000000000001, 0.3720592570533261)
(1.35, 0.3720592570533261)
(1.425, 0.3720592570533261)
(1.5, 0.3720592570533261)
(1.575, 0.3720592570533261)
(1.6500000000000001, 0.3720592570533261)
(1.725, 0.3720592570533261)
(1.8, 0.3720592570533261)
(1.875, 0.3720592570533261)
(1.95, 0.3720592570533261)
(2.025, 2.114295148147641)
(2.1, 2.1937115249980885)
(2.1750000000000003, 2.2760241165376693)
(2.25, 2.3633445720930433)
(2.325, 2.457792887430896)
(2.4, 2.5534347436925118)
(2.475, 2.6553698157339745)
(2.5500000000000003, 2.765183927160284)
(2.625, 2.8811910970861243)
(2.7, 3.0048602989561273)
(2.775, 3.1344387803647664)
(2.85, 3.271161814435936)
(2.9250000000000003, 3.4161645170132164)
(3.0, 3.5696305097771863)
(3.075, 3.732285933010137)
(3.15, 3.9026951990275394)
(3.225, 4.083979876399239)
(3.3000000000000003, 4.276490515606341)
(3.375, 4.481554200613029)
(3.45, 4.700214236422596)
(3.525, 4.93253739455525)
(3.6, 5.178047927929492)
(3.6750000000000003, 5.44652786425617)
(3.75, 5.740105545741997)
(3.825, 6.062879074439896)
(3.9, 6.4268172453476105)
(3.975, 6.799769571483753)
(4.05, 7.117660432766254)
(4.125, 7.452527953062292)
(4.2, 7.804180164251262)
(4.275, 8.174127771977929)
(4.3500000000000005, 8.559724954753948)
(4.425, 8.955446369281896)
(4.5, 9.363754215369536)
(4.575, 9.785499829899551)
(4.65, 10.20939882595636)
(4.7250000000000005, 10.641243632918226)
(4.8, 11.074757727885357)
(4.875, 11.503965059798904)
(4.95, 11.927354923014107)
(5.025, 12.348140696941098)
(5.1000000000000005, 12.760746959642292)
(5.175, 13.169906142612616)
(5.25, 13.571703765479725)
(5.325, 13.96953682933433)
(5.4, 14.367995876190912)
(5.4750000000000005, 14.767080906049465)
(5.55, 15.163703736100256)
(5.625, 15.565000572565785)
(5.7, 15.966656305952448)
(5.775, 16.361234258196788)
(5.8500000000000005, 16.751605604667862)
(5.925, 17.12811351425522)
(6.0, 17.49191814212251)
(6.075, 17.857500561715415)
(6.15, 18.220295270339523)
(6.2250000000000005, 18.578157232908076)
(6.3, 18.935551794835156)
(6.375, 19.29363911128442)
(6.45, 19.647302814519733)
(6.525, 20.003036434881576)
(6.6000000000000005, 20.359846746006813)
(6.675, 20.71204982223752)
(6.75, 21.06820076460068)
(6.825, 21.421422106514594)
(6.9, 21.775344549390727)
(6.9750000000000005, 22.132989504518598)
(7.05, 22.49276280185318)
(7.125, 22.855156881356024)
(7.2, 23.2167997812565)
(7.275, 23.575788513228606)
(7.3500000000000005, 23.937247791448506)
(7.425, 24.2982313225869)
(7.5, 24.6584219419228)
(7.575, 25.019555708981674)
(7.65, 25.379354045636333)
(7.7250000000000005, 25.734219636235434)
(7.8, 26.08638932670604)
(7.875, 26.43821681313556)
(7.95, 26.78978555992427)
(8.025, 27.138157620182895)
(8.1, 27.48806542540636)
(8.175, 27.841820939481966)
(8.25, 28.194816927515177)
(8.325, 28.551760781680834)
(8.4, 28.913361949381176)
(8.475, 29.27674090880713)
(8.55, 29.64019498619332)
(8.625, 30.005501973265353)
(8.700000000000001, 30.376175721274308)
(8.775, 30.75380205382519)
(8.85, 31.1282984713662)
(8.925, 31.508887790126426)
(9.0, 31.889911123768023)
(9.075000000000001, 32.27526625978328)
(9.15, 32.65502093454087)
(9.225, 33.03737969858668)
(9.3, 33.42172491535875)
(9.375, 33.805552652849194)
(9.450000000000001, 34.18784464537479)
(9.525, 34.569761048099195)
(9.6, 34.94928202253605)
(9.675, 35.32884472917304)
(9.75, 35.7064293295238)
(9.825000000000001, 36.08131802974604)
(9.9, 36.459561998858874)
(9.975, 36.832864875476126)
(10.05, 37.20588397313247)
(10.125, 37.579362124990276)
(10.200000000000001, 37.95359145645045)
(10.275, 38.3245489834203)
(10.35, 38.69860303963992)
(10.425, 39.06778277488416)
(10.5, 39.43561038684414)
(10.575000000000001, 39.80004099771341)
(10.65, 40.15890453308512)
(10.725, 40.51516397916862)
(10.8, 40.86583965687451)
(10.875, 41.21497124317553)
(10.950000000000001, 41.55496347764773)
(11.025, 41.894246264717694)
(11.1, 42.22616749168444)
(11.175, 42.55337298003632)
(11.25, 42.87501139289064)
(11.325000000000001, 43.19444634557801)
(11.4, 43.5097665033324)
(11.475, 43.82094682683374)
(11.55, 44.13049124808992)
(11.625, 44.43834968846078)
(11.700000000000001, 44.74773552735646)
(11.775, 45.059416637259375)
(11.85, 45.36825995755334)
(11.925, 45.68169381986179)
(12.0, 45.99704736337629)
(12.075000000000001, 46.31162468796834)
(12.15, 46.63223648869942)
(12.225, 46.957196784684214)
(12.3, 47.28946856213207)
(12.375, 47.62642269243469)
(12.450000000000001, 47.96820106507252)
(12.525, 48.316422889410674)
(12.6, 48.67506107090167)
(12.675, 49.045092143028604)
(12.75, 49.4213913916153)
(12.825000000000001, 49.80961770299961)
(12.9, 50.21127343638627)
(12.975, 50.62342064488602)
(13.05, 51.04922262926883)
(13.125, 51.487928209932335)
(13.200000000000001, 51.94147376096263)
(13.275, 52.41070227280239)
(13.35, 52.893043041923505)
(13.425, 53.39021543497139)
(13.5, 53.8991646548964)
(13.575000000000001, 54.42033306301997)
(13.65, 54.95175089949584)
(13.725, 55.49119801127704)
(13.8, 56.03532747591301)
(13.875, 56.58007457711093)
(13.950000000000001, 57.12537254335057)
(14.025, 57.66658075397733)
(14.1, 58.20770550020382)
(14.175, 58.7459757639413)
(14.25, 59.285781772643645)
(14.325000000000001, 59.8263890395885)
(14.4, 60.36879079113901)
(14.475, 60.91369647469743)
(14.55, 61.46604718275933)
(14.625, 62.0304084180191)
(14.700000000000001, 62.60944269484514)
(14.775, 63.21374164563086)
(14.85, 63.84166936813109)
(14.925, 64.50338347985787)
};
\addplot[solid, red, thick, mark = none] coordinates{
(0.0008405942394446342,0.38817229944278964)
(0.08490001818390805,0.3944914026980993)
(0.16895944212837147,0.40272865687584863)
(0.25301886607283486,0.4139967555847255)
(0.3370782900172983,0.4281877509373198)
(0.4211377139617617,0.4477346222421806)
(0.5051971379062252,0.4851510207552233)
(0.5892565618506886,0.5548355339202156)
(0.6733159857951521,0.6224192151225357)
(0.7573754097396155,0.6839910293644825)
(0.8414348336840789,0.7413362686301446)
(0.9254942576285423,0.8005000146144833)
(1.0095536815730055,0.8613909267973822)
(1.093613105517469,0.9267824355169143)
(1.1776725294619323,0.9950719298292231)
(1.2617319534063958,1.0704693773432996)
(1.3457913773508592,1.1520613728579816)
(1.4298508012953228,1.2425632209258142)
(1.5139102252397862,1.3416925963028015)
(1.5979696491842497,1.4473154522916838)
(1.682029073128713,1.560453141981033)
(1.7660884970731765,1.6830570310278765)
(1.85014792101764,1.8232315146716125)
(1.9342073449621033,1.9749730296355148)
(2.0182667689065665,2.1427240466706876)
(2.10232619285103,2.333658948448075)
(2.1863856167954934,2.5059686878054097)
(2.270445040739957,2.6406461328748816)
(2.35450446468442,2.766222740667324)
(2.4385638886288836,2.8949962666638323)
(2.522623312573347,3.0294495122748373)
(2.6066827365178105,3.1679217407709537)
(2.690742160462274,3.3122231551872114)
(2.7748015844067373,3.4653347779528563)
(2.8588610083512007,3.6234036998557153)
(2.942920432295664,3.7892033512338608)
(3.0269798562401276,3.9617788084678973)
(3.111039280184591,4.144418330282006)
(3.1950987041290544,4.340634374858837)
(3.279158128073518,4.549762647506636)
(3.3632175520179812,4.768523193184867)
(3.4472769759624446,5.004322897706589)
(3.531336399906908,5.2525947350659905)
(3.6153958238513715,5.5208203242289535)
(3.699455247795835,5.810278432477102)
(3.7835146717402983,6.121492191880193)
(3.8675740956847617,6.458737999516393)
(3.951633519629225,6.816576942596968)
(4.035692943573689,7.199260507149139)
(4.119752367518152,7.608823095666407)
(4.203811791462615,8.036720217676084)
(4.287871215407079,8.47483087057148)
(4.371930639351542,8.915341288040835)
(4.4559900632960066,9.364695128594166)
(4.54004948724047,9.825275549438139)
(4.624108911184933,10.300428935082467)
(4.708168335129397,10.783869397006422)
(4.79222775907386,11.272914845392053)
(4.876287183018324,11.759992320753364)
(4.960346606962787,12.245317718865172)
(5.0444060309072505,12.726092698338466)
(5.128465454851714,13.199535525151527)
(5.212524878796177,13.665571466151526)
(5.296584302740641,14.119475725343374)
(5.380643726685104,14.564860405113475)
(5.464703150629568,15.0053126967973)
(5.548762574574031,15.44608883214336)
(5.632821998518494,15.887404706926468)
(5.716881422462958,16.325042049853987)
(5.800940846407421,16.761599913907407)
(5.885000270351885,17.197950185869654)
(5.969059694296348,17.63351991156909)
(6.0531191182408115,18.06354277659238)
(6.137178542185275,18.490202649738666)
(6.221237966129738,18.912104512155263)
(6.305297390074202,19.325569831986584)
(6.389356814018665,19.732533367522368)
(6.473416237963129,20.132073409877798)
(6.557475661907592,20.531123534898057)
(6.641535085852055,20.926295839655204)
(6.725594509796519,21.320222591865313)
(6.809653933740982,21.713734159893075)
(6.893713357685446,22.107478231062952)
(6.977772781629909,22.50235160320881)
(7.0618322055743725,22.898553564738176)
(7.145891629518836,23.29173298542006)
(7.229951053463299,23.68795155431672)
(7.314010477407763,24.08603014835029)
(7.398069901352226,24.481991303053896)
(7.48212932529669,24.88029409654593)
(7.566188749241153,25.278522156885145)
(7.6502481731856165,25.67768022979282)
(7.73430759713008,26.07557614278616)
(7.818367021074543,26.472525435843746)
(7.902426445019007,26.87116037668166)
(7.98648586896347,27.268358780248658)
(8.070545292907934,27.665856116426944)
(8.154604716852397,28.058562227140953)
(8.23866414079686,28.45126833785497)
(8.322723564741324,28.842097816064772)
(8.406782988685787,29.233292656355044)
(8.49084241263025,29.628224154286425)
(8.574901836574714,30.024907729467316)
(8.658961260519177,30.42784397843434)
(8.743020684463641,30.829617711690787)
(8.827080108408104,31.23732857875479)
(8.911139532352568,31.645346682113733)
(8.995198956297031,32.05966728136069)
(9.079258380241495,32.47267589859143)
(9.163317804185958,32.88860741246589)
(9.247377228130421,33.30310238906943)
(9.331436652074885,33.720096774450695)
(9.415496076019348,34.137838491360185)
(9.499555499963812,34.5542931373044)
(9.583614923908275,34.9694358012324)
(9.667674347852738,35.38109091802869)
(9.751733771797202,35.79693109138303)
(9.835793195741665,36.208179327680625)
(9.919852619686129,36.61819861879847)
(10.003912043630592,37.02985373559477)
(10.087971467575056,37.43510671229928)
(10.172030891519519,37.841912477845774)
(10.256090315463982,38.2450978373222)
(10.340149739408446,38.64830810784957)
(10.42420916335291,39.04764886179748)
(10.508268587297373,39.44613433632975)
(10.592328011241836,39.839861800132326)
(10.6763874351863,40.233165776068915)
(10.760446859130763,40.621446023399116)
(10.844506283075226,41.00477727527575)
(10.92856570701969,41.38031967189156)
(11.012625130964153,41.753644984973654)
(11.096684554908617,42.11723838082155)
(11.18074397885308,42.47565027807376)
(11.264803402797543,42.827369406306545)
(11.348862826742007,43.17724511676972)
(11.43292225068647,43.522047276524624)
(11.516981674630934,43.86349474808617)
(11.601041098575397,44.20075716308966)
(11.68510052251986,44.53514650355132)
(11.769159946464324,44.87038281974496)
(11.853219370408787,45.20703906584223)
(11.93727879435325,45.54355414931751)
(12.021338218297714,45.88084147537194)
(12.105397642242178,46.22220591009702)
(12.189457066186641,46.57153357743949)
(12.273516490131104,46.92453147295391)
(12.357575914075568,47.28773459567039)
(12.441635338020031,47.66109312348707)
(12.525694761964495,48.0405299477333)
(12.609754185908958,48.43139264067769)
(12.693813609853422,48.83388049072778)
(12.777873033797885,49.24987013038776)
(12.861932457742348,49.68053237905187)
(12.945991881686812,50.12981148645237)
(13.030051305631275,50.588515274792144)
(13.114110729575739,51.06837684906428)
(13.198170153520202,51.561922893986534)
(13.282229577464665,52.07651047327011)
(13.366289001409129,52.608759987670695)
(13.450348425353592,53.15774142461982)
(13.534407849298056,53.72085573113602)
(13.61846727324252,54.2991657787261)
(13.702526697186983,54.888868480279754)
(13.786586121131446,55.493617456601626)
(13.87064554507591,56.10252657843061)
(13.954704969020373,56.70955076407176)
(14.038764392964836,57.32219654354186)
(14.1228238169093,57.93311515681341)
(14.206883240853763,58.54772890930783)
(14.290942664798227,59.16769853775452)
(14.37500208874269,59.80248193782734)
(14.459061512687153,60.45610639609501)
(14.543120936631617,61.164942046931095)
(14.62718036057608,62.05749669845538)
(14.711239784520544,63.27984044970093)
(14.795299208465007,65.28990484642834)
(14.87935863240947,70.19900110007201)
(14.963418056353934,94.36003011912132)
(15.047477480298397,98.9960680397195)
(15.13153690424286,99.78597255400051)
(15.215596328187324,99.95465358360414)
(15.299655752131788,99.98883154549489)
(15.383715176076251,99.99593119501301)
(15.467774600020714,99.99795729382286)
(15.551834023965178,99.99900355796237)
(15.635893447909641,99.99948517161388)
(15.719952871854105,99.99968446002143)
(15.804012295798568,99.99978410422517)
(15.888071719743031,99.99983392632707)
(15.972131143687495,99.999858837378)
(16.05619056763196,99.9998920521126)
(16.14024999157642,99.99990035579623)
(16.224309415520885,99.99991696316353)
(16.30836883946535,99.99991696316353)
(16.392428263409812,99.99995848158176)
(16.476487687354275,99.99997508894906)
(16.56054711129874,99.99997508894906)
(16.644606535243202,99.99997508894906)
(16.728665959187666,99.99998339263271)
};
\addplot[dashed, magenta, thick, mark = none] coordinates{
(0.0, 0.5978301732190421)
(0.075, 0.6133760916944118)
(0.15, 0.6302307014301745)
(0.225, 0.6474937562089899)
(0.3, 0.6658404406938631)
(0.375, 0.6855625013441176)
(0.45, 0.7072100886259058)
(0.525, 0.729924634387505)
(0.6, 0.7542562890950675)
(0.675, 0.7787713272913476)
(0.75, 0.8055703234834727)
(0.8250000000000001, 0.8346949557370608)
(0.9, 0.8651199436379183)
(0.975, 0.8980706223152032)
(1.05, 0.9571367769084845)
(1.125, 1.0989005493002337)
(1.2, 1.1451548665226605)
(1.2750000000000001, 1.1934430733472272)
(1.35, 1.2504586671121218)
(1.425, 1.3082328016712572)
(1.5, 1.3678491067306908)
(1.575, 1.431733245709368)
(1.6500000000000001, 1.5001519582272418)
(1.725, 1.5731302511236822)
(1.8, 1.6536022602181697)
(1.875, 1.7413345883432452)
(1.95, 1.8342933458967696)
(2.025, 2.4780944254920385)
(2.1, 2.60748814800848)
(2.1750000000000003, 2.7090742651448503)
(2.25, 2.8046754120585313)
(2.325, 2.9040109136515504)
(2.4, 3.005847099181626)
(2.475, 3.113043083950127)
(2.5500000000000003, 3.2260573266788466)
(2.625, 3.3446564302003265)
(2.7, 3.4692071614920015)
(2.775, 3.6020601634547047)
(2.85, 3.7420984639298847)
(2.9250000000000003, 3.8896138093768644)
(3.0, 4.044789583284362)
(3.075, 4.211743578535397)
(3.15, 4.3851493383440365)
(3.225, 4.567940998529765)
(3.3000000000000003, 4.762994345620194)
(3.375, 4.968975681515561)
(3.45, 5.1898861005151575)
(3.525, 5.4273593827911935)
(3.6, 5.676210776980837)
(3.6750000000000003, 5.947368271889028)
(3.75, 6.237430937361369)
(3.825, 6.549357916056708)
(3.9, 6.891509827937941)
(3.975, 7.275306462984293)
(4.05, 7.7634899811765194)
(4.125, 8.116119758754019)
(4.2, 8.48711289204264)
(4.275, 8.87052608888531)
(4.3500000000000005, 9.27121067611992)
(4.425, 9.682389800277043)
(4.5, 10.10815624740033)
(4.575, 10.5434836427763)
(4.65, 10.981970235526083)
(4.7250000000000005, 11.424399573283294)
(4.8, 11.862452714150654)
(4.875, 12.295629521340754)
(4.95, 12.727806054956032)
(5.025, 13.160140965220654)
(5.1000000000000005, 13.587757918457367)
(5.175, 14.010456859951196)
(5.25, 14.423828250359808)
(5.325, 14.839166845465568)
(5.4, 15.251346243197514)
(5.4750000000000005, 15.66676819443451)
(5.55, 16.075063196450895)
(5.625, 16.484250109071496)
(5.7, 16.894520651398157)
(5.775, 17.309109041322802)
(5.8500000000000005, 17.720679939296733)
(5.925, 18.130767098134672)
(6.0, 18.538695333173624)
(6.075, 18.95191668254601)
(6.15, 19.333304325399663)
(6.2250000000000005, 19.705797869050517)
(6.3, 20.07650759149294)
(6.375, 20.44800086156897)
(6.45, 20.81621823568746)
(6.525, 21.186994643034872)
(6.6000000000000005, 21.553469874010542)
(6.675, 21.92303761745504)
(6.75, 22.287362260244844)
(6.825, 22.653379032498723)
(6.9, 23.022079872178374)
(6.9750000000000005, 23.391764314206604)
(7.05, 23.76241568735716)
(7.125, 24.13397564233818)
(7.2, 24.505969049201624)
(7.275, 24.879329496617324)
(7.3500000000000005, 25.253565183411)
(7.425, 25.62804260298525)
(7.5, 26.006062658137)
(7.575, 26.38009829021571)
(7.65, 26.755175873934856)
(7.7250000000000005, 27.127711095651325)
(7.8, 27.496295236747248)
(7.875, 27.869213896667404)
(7.95, 28.23931511935181)
(8.025, 28.617751955159736)
(8.1, 28.98364369321676)
(8.175, 29.34897694519451)
(8.25, 29.720561907014904)
(8.325, 30.09275536859331)
(8.4, 30.46615749407463)
(8.475, 30.84332731668778)
(8.55, 31.21890503719434)
(8.625, 31.598592214970793)
(8.700000000000001, 31.97865449533781)
(8.775, 32.36687734095275)
(8.85, 32.75448335119655)
(8.925, 33.146215489936495)
(9.0, 33.53790595061083)
(9.075000000000001, 33.9300381987807)
(9.15, 34.32471280895325)
(9.225, 34.71945410403078)
(9.3, 35.11671275427163)
(9.375, 35.51023704983313)
(9.450000000000001, 35.905778563770525)
(9.525, 36.295701874462665)
(9.6, 36.69002638888403)
(9.675, 37.08318391746809)
(9.75, 37.47364070740014)
(9.825000000000001, 37.86537284614009)
(9.9, 38.250669891548675)
(9.975, 38.637117251568306)
(10.05, 39.027840781120304)
(10.125, 39.411112272539874)
(10.200000000000001, 39.790757772250714)
(10.275, 40.16463502768007)
(10.35, 40.53541143502748)
(10.425, 40.90880522489568)
(10.5, 41.273504970276036)
(10.575000000000001, 41.638121359525165)
(10.65, 41.998494921694416)
(10.725, 42.358118278682554)
(10.8, 42.71624122530845)
(10.875, 43.066195271073305)
(10.950000000000001, 43.41125631193465)
(11.025, 43.754591880879424)
(11.1, 44.08891665203766)
(11.175, 44.42049900647827)
(11.25, 44.75122279276715)
(11.325000000000001, 45.072352288350864)
(11.4, 45.39109779858125)
(11.475, 45.70932650079797)
(11.55, 46.02420428653903)
(11.625, 46.337431620881645)
(11.700000000000001, 46.65159254389409)
(11.775, 46.966295281759564)
(11.85, 47.28467402501251)
(11.925, 47.59957681759294)
(12.0, 47.9187391084795)
(12.075000000000001, 48.24137735003857)
(12.15, 48.56677467954152)
(12.225, 48.8958313432057)
(12.3, 49.22941424479595)
(12.375, 49.56739835011542)
(12.450000000000001, 49.914426595673916)
(12.525, 50.266964681507055)
(12.6, 50.62702149037762)
(12.675, 50.99723941164576)
(12.75, 51.37682656206473)
(12.825000000000001, 51.76616637983822)
(12.9, 52.16448365294575)
(12.975, 52.573937305186305)
(13.05, 52.996636246680126)
(13.125, 53.435272880466144)
(13.200000000000001, 53.89191443859895)
(13.275, 54.3584170270569)
(13.35, 54.83736468590826)
(13.425, 55.33235006440928)
(13.5, 55.835370973961375)
(13.575000000000001, 56.34455190161176)
(13.65, 56.86528598905134)
(13.725, 57.39508088795618)
(13.8, 57.92813501159234)
(13.875, 58.46749085874987)
(13.950000000000001, 59.008280431364646)
(14.025, 59.609169774600026)
(14.1, 60.313295686370225)
(14.175, 61.02494865679097)
(14.25, 61.75203918271648)
(14.325000000000001, 62.49846833108855)
(14.4, 63.252357853206185)
(14.475, 64.02990384536838)
(14.55, 64.82927247268795)
(14.625, 65.65083883775546)
(14.700000000000001, 66.52143527921554)
(14.775, 70.33132728467902)
(14.85, 79.65141799615529)
(14.925, 89.58084202696104)
};
\addplot[dashed, black, thick, mark = none] coordinates{
(0.0, 0.4969173404829157)
(0.075, 0.5062340735347652)
(0.15, 0.5163977823186011)
(0.225, 0.5269434605501954)
(0.3, 0.53835272188107)
(0.375, 0.550268507914407)
(0.45, 0.562831981272204)
(0.525, 0.5761012677399898)
(0.6, 0.5904915515001102)
(0.675, 0.6063432835820896)
(0.75, 0.6221950156640689)
(0.8250000000000001, 0.6391677450383829)
(0.9, 0.6574524564289111)
(0.975, 0.6764180698784872)
(1.05, 0.7090598502945483)
(1.125, 0.7954098565389183)
(1.2, 0.8221975399838976)
(1.2750000000000001, 0.8511690922280178)
(1.35, 0.8842177531427782)
(1.425, 0.9161703278161446)
(1.5, 0.9497006023824264)
(1.575, 0.9857551967773736)
(1.6500000000000001, 1.02340409843253)
(1.725, 1.0635690162327052)
(1.8, 1.1058513733628457)
(1.875, 1.1509735903002347)
(1.95, 1.1987446823209924)
(2.025, 1.7221922920558328)
(2.1, 1.7916692131296517)
(2.1750000000000003, 1.843243392260701)
(2.25, 1.8896692875306573)
(2.325, 1.9366432259213102)
(2.4, 1.9850370942155877)
(2.475, 2.0365116291428738)
(2.5500000000000003, 2.0894891308102537)
(2.625, 2.143712185024672)
(2.7, 2.2025603910304272)
(2.775, 2.2620978027788774)
(2.85, 2.3243173043452843)
(2.9250000000000003, 2.3913861571614956)
(3.0, 2.462689888637638)
(3.075, 2.5398061986666276)
(3.15, 2.6193803990551072)
(3.225, 2.7038454691116254)
(3.3000000000000003, 2.7930602462141843)
(3.375, 2.890636832749197)
(3.45, 2.9943913599175214)
(3.525, 3.1081933442986243)
(3.6, 3.229892131827953)
(3.6750000000000003, 3.3595624556583292)
(3.75, 3.497171101055166)
(3.825, 3.6439885316164413)
(3.9, 3.796552111261389)
(3.975, 3.9640457141035075)
(4.05, 4.160718461280919)
(4.125, 4.3076438397296055)
(4.2, 4.464525334870954)
(4.275, 4.632600195568357)
(4.3500000000000005, 4.812590842299097)
(4.425, 5.005867382864917)
(4.5, 5.2136587624455615)
(4.575, 5.438995825572157)
(4.65, 5.677577264115598)
(4.7250000000000005, 5.928796909169658)
(4.8, 6.202577662692413)
(4.875, 6.492376221970085)
(4.95, 6.800127345292409)
(5.025, 7.128961521394276)
(5.1000000000000005, 7.478231062951222)
(5.175, 7.847404534209848)
(5.25, 8.235319419459582)
(5.325, 8.641660178721844)
(5.4, 9.071799295316191)
(5.4750000000000005, 9.520206515933772)
(5.55, 9.991232970805578)
(5.625, 10.479414836091928)
(5.7, 10.992316767595174)
(5.775, 11.52684979499866)
(5.8500000000000005, 12.083105258822497)
(5.925, 12.66119941063775)
(6.0, 13.257935332240347)
(6.075, 13.880611961555939)
(6.15, 14.515802242127442)
(6.2250000000000005, 15.172058968111198)
(6.3, 15.844051174605875)
(6.375, 16.53359736833015)
(6.45, 17.238314392077356)
(6.525, 17.967560497317578)
(6.6000000000000005, 18.71260020885425)
(6.675, 19.468443012815573)
(6.75, 20.24003790465511)
(6.825, 21.023714656200926)
(6.9, 21.815313121945906)
(6.9750000000000005, 22.6223979576924)
(7.05, 23.43845077177757)
(7.125, 24.258979271348437)
(7.2, 25.086009555214844)
(7.275, 25.916651941467666)
(7.3500000000000005, 26.750399905404436)
(7.425, 27.58905534637654)
(7.5, 28.4297036714239)
(7.575, 29.272876316299936)
(7.65, 30.108550734842787)
(7.7250000000000005, 30.937416132795164)
(7.8, 31.767742979069403)
(7.875, 32.594872907139575)
(7.95, 33.41305146423836)
(8.025, 34.22857284257013)
(8.1, 35.029454826632374)
(8.175, 35.81735815315447)
(8.25, 36.594126239906046)
(8.325, 37.364309505525604)
(8.4, 38.123291101905465)
(8.475, 38.86482665894314)
(8.55, 39.598083443384816)
(8.625, 40.31560474731559)
(8.700000000000001, 41.01306435155538)
(8.775, 41.69369238904286)
(8.85, 42.367876768020324)
(8.925, 43.02274677883504)
(9.0, 43.66313516536952)
(9.075000000000001, 44.28660064463157)
(9.15, 44.893168127672126)
(9.225, 45.47962408891983)
(9.3, 46.04844302610147)
(9.375, 46.60949801907323)
(9.450000000000001, 47.1497439808258)
(9.525, 47.67525090410508)
(9.6, 48.182755441237816)
(9.675, 48.677671593961826)
(9.75, 49.15570635783163)
(9.825000000000001, 49.61625356394102)
(9.9, 50.06293361836004)
(9.975, 50.49758993885831)
(10.05, 50.9185866997574)
(10.125, 51.322594123914875)
(10.200000000000001, 51.71207010169023)
(10.275, 52.08970502658508)
(10.35, 52.45745856794007)
(10.425, 52.810713877647544)
(10.5, 53.1511898182224)
(10.575000000000001, 53.48158508684989)
(10.65, 53.80176682459166)
(10.725, 54.11220003773194)
(10.8, 54.412245342629916)
(10.875, 54.70402017861555)
(10.950000000000001, 54.98860402456296)
(11.025, 55.26488418686344)
(11.1, 55.53651428632163)
(11.175, 55.799417214266924)
(11.25, 56.05691444415805)
(11.325000000000001, 56.305900398311096)
(11.4, 56.552320514217236)
(11.475, 56.793368146803815)
(11.55, 57.027374255657804)
(11.625, 57.25936256938559)
(11.700000000000001, 57.491035343134776)
(11.775, 57.718307164551106)
(11.85, 57.93951729690519)
(11.925, 58.15959812828327)
(12.0, 58.37749509086223)
(12.075000000000001, 58.59598991866376)
(12.15, 58.80997584624501)
(12.225, 59.02287399126851)
(12.3, 59.232583521771595)
(12.375, 59.44123848445152)
(12.450000000000001, 59.65192784962494)
(12.525, 59.85984378446029)
(12.6, 60.06953670759607)
(12.675, 60.27927945283375)
(12.75, 60.49015980273105)
(12.825000000000001, 60.70515877971723)
(12.9, 60.916769853775456)
(12.975, 61.13025756033789)
(13.05, 61.34844515184448)
(13.125, 61.564581733490286)
(13.200000000000001, 61.78546802218213)
(13.275, 62.0060055561608)
(13.35, 62.22949920151778)
(13.425, 62.45551716670342)
(13.5, 62.687380925176505)
(13.575000000000001, 62.92040719936015)
(13.65, 63.160151153614166)
(13.725, 63.40534232434055)
(13.8, 63.65456908531936)
(13.875, 63.91151827208979)
(13.950000000000001, 64.17222902755229)
(14.025, 64.49729333127846)
(14.1, 64.92511572013531)
(14.175, 65.37155496772856)
(14.25, 65.84285544416072)
(14.325000000000001, 66.34035404249892)
(14.4, 66.85715040163257)
(14.475, 67.40418877660832)
(14.55, 67.96977758085131)
(14.625, 68.57305680516768)
(14.700000000000001, 69.21068006504774)
(14.775, 72.6176897690646)
(14.85, 81.23674732089951)
(14.925, 90.38879341497959)
};
